# Supplementary material for: Solving Continual Offline Reinforcement Learning with Decision Transformer
Source: arXiv:2401.08478 source file (2024-04-07)
Supplement: Supplementary file 1 [file appendix.tex]

\appendix
\section{ADDITIONAL ALGORITHM DESCRIPTIONS} \label{sec:pseudo-code}
\subsection{PSEUDO-CODE}
We present the algorithms for MH-DT training in Sec.\ref{sec:mhdt_train} and for LoRA-DT in Sec.\ref{sec:lora_train}
\subsubsection{MH-DT}\label{sec:mhdt_train}
\begin{algorithm}[htbp]
    \caption{MH-DT training}
    \label{alg:MH-DT}
    \textbf{Input}: Number of task N; Number of select task K; Number of select frequency T; Dataset $D_i$ of each task $T_i$, $i \in [1, \dots, N]$; Initial the policy $\pi$.
    \begin{algorithmic}[1] %[1] enables line numbers
        \FOR{Tasks $T_n$ in $[1, \dots, N]$}
            \STATE Get dataset $D_n$; Get replay buffers for previous task $B_1, \dots, B_{n-1}$; Initial the replay buffer $B_n = \emptyset$; Initial new head $h_n$ for $\pi$; Initial DT policy $\mu_n$; Initial select set $S=[1, \dots, N-1]$.
            \FOR{step $i$ in $range(max\_steps)$}
                \STATE Update $\mu_n$ via minimizing mean-squared loss.
                \STATE Copy the parameters in head of $\mu_n$ to head $h_n$.
                \IF{$i \mod T ==0 $}
                    \STATE Select $K$ tasks and add them to $S$ via Eq.(\ref{eq:select}).
                \ENDIF
                \STATE Sample a batch from $D_n$.
                \STATE Calculate $\mathcal{L}_{\text {predict }}$ with mean-squared loss.
                \STATE Calculate $\mathcal{L}_{\text {distillation }}$ via Eq.(\ref{eq:loss_distill}).
                \FOR{$j$ in $S$}
                    \STATE Sample a batch from $B_{j}$.
                    \STATE Calculate $\mathcal{L}_{\text {rehearsal }}$ with corresponding $\pi_j$ as in Eq.(\ref{eq:loss_rehearsal}).
                \ENDFOR
                \STATE Update $\pi$ with $\mathcal{L}_{\text {total }}$ in Eq.(\ref{eq:loss}).
            \ENDFOR
            \STATE Randomly select trajectories in $D_n$ and add them to $B_n$.
        \ENDFOR
    \end{algorithmic}
    \textbf{Output}: Policy $\pi$.
\end{algorithm}

\subsubsection{LoRA-DT}\label{sec:lora_train}

\begin{algorithm}[htbp]
    \caption{LoRA-DT training}
    \label{alg:lora-DT}
    \textbf{Input}: Number of task N; Number of blocks k; Dataset $D_i$ of each task $T_i$, $i \in [1, \dots, N]$; Initial the policy $\pi$.
    \begin{algorithmic}[1] %[1] enables line numbers
        \FOR{Tasks $T_n$ in $[1, \dots, N]$}
            \STATE Get dataset $D_n$; Get replay buffers for previous task $B_1, \dots, B_{n-1}$; Initial the replay buffer $B_n = \emptyset$; Initial DT policy $\mu_n$; Initial update matrices $\mA \mB$; Initial $ \sM_n= \emptyset$.
            \IF{n == 1 }
                \STATE Update $\pi$ via minimizing mean-squared loss.
            \ELSE
                \STATE Update $\mu_n$ via minimizing mean-squared loss.
                \STATE Merge the parameters in $\mu_n$ to  $\pi$ except for the MLP layers of each block as in Eq.(\ref{eq:merge}).
                \STATE Update matrices $\mA \mB$ with LoRA as in Eq.(\ref{eq:fine-tune})
            \ENDIF
            \STATE Randomly select trajectories in $D_n$ and add them to $B_n$.
            \STATE Save $ \sM_n = k * [\mA_0,\mB_0,\mA_1,\mB_1] $ for $T_n$
        \ENDFOR
    \end{algorithmic}
    \textbf{Output}: Policy $\pi$.
\end{algorithm}

\subsection{Hyperparameters}
We show the common hyperparameters of DT in Table.\ref{tab:common_hyp} and specific hyperparameters of our MH-DT and LoRA-DT in Table.\ref{tab:MHDT_hyp} and Table.\ref{tab:lora_hyp}.
\begin{table}[h!]
\centering
\caption{Common Hyperparameters of all Decision Transformer}

\begin{tabular}{cc}
\hline Hyperparameters & Value \\
\hline$K$ (length of context $\tau$ ) & 20 \\
number of evaluation episodes for each task & 10 \\
learning rate & $1 \mathrm{e}-4$ \\
learning rate decay weight & $1 \mathrm{e}-4$ \\
number of layers & 3 \\
number of attention heads & 1 \\
embedding dimension & 128 \\
activation & ReLU \\
\hline
\end{tabular}
\label{tab:common_hyp}
\end{table}

\begin{table}[h!]
\centering
\caption{Specific Hyperparameters of MH-DT}

\begin{tabular}{cc}
\hline Hyperparameters & Value \\
\hline
number of select task K & 2 \\
select frequency T &  10 \\
replay buffer size & 1K \\
weight of distillation $\lambda_1$ & 0.5 \\
weight of distillation $\lambda_2$ &  1.0 \\
\hline
\end{tabular}
\label{tab:MHDT_hyp}

\end{table}

\begin{table}[h!]
\centering
\caption{Specific Hyperparameters of LoRA-DT}

\begin{tabular}{cc}
\hline Hyperparameters & Value \\
\hline
rank $r$ & 4 \\
inner dim of the MLP layer &  128 \\
weight of merge $\lambda$ & 0.2 \\
\hline
\end{tabular}
\label{tab:lora_hyp}

\end{table}

\section{EXPERIMENT DETAILS}\label{sec:detail}
We present the detail of offline sequential datasets  in Sec.\ref{sec:dataset}, details of metrics in Sec.\ref{sec:metric} and implement details in Sec.\ref{sec:imple}.

\subsection{offline sequential datasets}\label{sec:dataset}
We consider four sets of tasks from widely-used continuous control environments as in \citet{gai2023offline} and \citet{mitchell2021offline}:
\begin{itemize}[leftmargin=*]
    \item Ant-2D Direction (Ant-Dir): train a simulated ant with 8 articulated joints to run in a 2D direction
    \item Walker-2D Params (Walker-Par): train a simulated agent to move forward, where different tasks have different parameters. Specifically, different tasks require the agent to move at different speeds
    \item Half-Cheetah Velocity (Cheetah-Vel): train a cheetah to run at a random velocity. Cheetah-vel is unique in that as the 'vel' number increases the task becomes more challenging.
    % Cheetah-vel is special because the larger the vel number, the greater the target speed and the more difficult the task.
    \item Meta-World reach-v2. Tasks are to control a Sawyer robot's end-effector to reach different target positions in 3D space. The agent directly controls the XYZ location of the end-effector.
\end{itemize}
For Ant-Dir, Walker-Par and Meta-World reach-v2, we randomly sample six tasks to form sequential tasks $T_1$ to $T_6$. For Cheetah-Vel, we fixedly select the six tasks of vel={3, 6, 9, 12, 15, 18} and train them in order. The difficulty of the six tasks increases in sequence.

To consider different data quality, we selected different time periods in the online training buffer and obtained expert-quality data and middle-quality data as in \citet{mitchell2021offline}. For Meta-World reach-v2, we use the expert dataset because only expert script policies are available.

\subsection{metrics}\label{sec:metric}
use evaluation metrics to evaluate the continuous learning ability of the algorithm as in \citet{lopez2017gradient}. More specifically, we would like to measure:
\begin{itemize}[leftmargin=*]
    \item \textit{Average Performance} (PER), which measures average performance on all tasks after training.
    \begin{equation}
    \mathrm{PER}=\frac{1}{N} \sum_{n=1}^N a_{N, n}
    \label{eq:per}
    \end{equation}
    \item \textit{Backward transfer} (BWT), which is the influence that learning a task $t$ has on the performance on a previous task $k \prec t$. On the one hand, there exists positive backward transfer when learning about some task $t$ increases the performance on some preceding task $k$. On the other hand, there exists negative backward transfer when learning about some task $t$ decreases the performance on some preceding task $k$. Large negative backward transfer is also known as catastrophic forgetting.
    \begin{equation}
    \mathrm{BWT}=\frac{1}{N-1} \sum_{n=1}^{N-1} a_{n, n}-a_{N, n}
    \label{eq:bwt}
    \end{equation}
    \item \textit{Forward transfer} (FWT), which is the influence that learning a task $t$ has on the performance on a future task $k \succ t$. In particular, positive forward transfer is possible when the model is able to perform "zero-shot" learning, perhaps by exploiting the structure available in the task descriptors.
    \begin{equation}
    \mathrm{FWT}=\frac{1}{N-1} \sum_{n=2}^N a_{n-1, n}-\bar{b}_n
    \label{eq:fwt}
    \end{equation}
\end{itemize} 
where $a_{i, j}$ means the final cumulative rewards of task $j$ after learning task $i$ and $\bar{b}_n$ means the test performance for each task at random initialization. For PER, higher is better; for BWT, lower is better; for FWT, higher is better. If two models have similar PER, the most preferable one is the one with lower BWT and higher FWT.

\subsection{implement detials}\label{sec:imple}

For each evaluation step, we test all strategies on the corresponding tasks 10 times and report the average.

For LoRA-DT, the MLP layer in each block in the original DT implementation is composed of two Cov1D layers plus an intermediate activation layer. In our implementation, we replace the Cov1D layer with a liner class \footnote{https://github.com/microsoft/LoRA} which contains a LoRA Layer and a Linear layer. Update the parameters of the Linear layer when training the first task $T_1$, and then only fine-tune the LoRA matrix $\mA\mB$ and save it after training each task. 

\section{ADDITIONAL RESULTS}\label{sec:exp}
We present the training curves for all environments and dataset qualities in this section.
\subsection{traing curves}
\begin{figure}[htbp]
	\centering
	\subcaptionbox{PDT}
    {\includegraphics[width=0.245\linewidth]{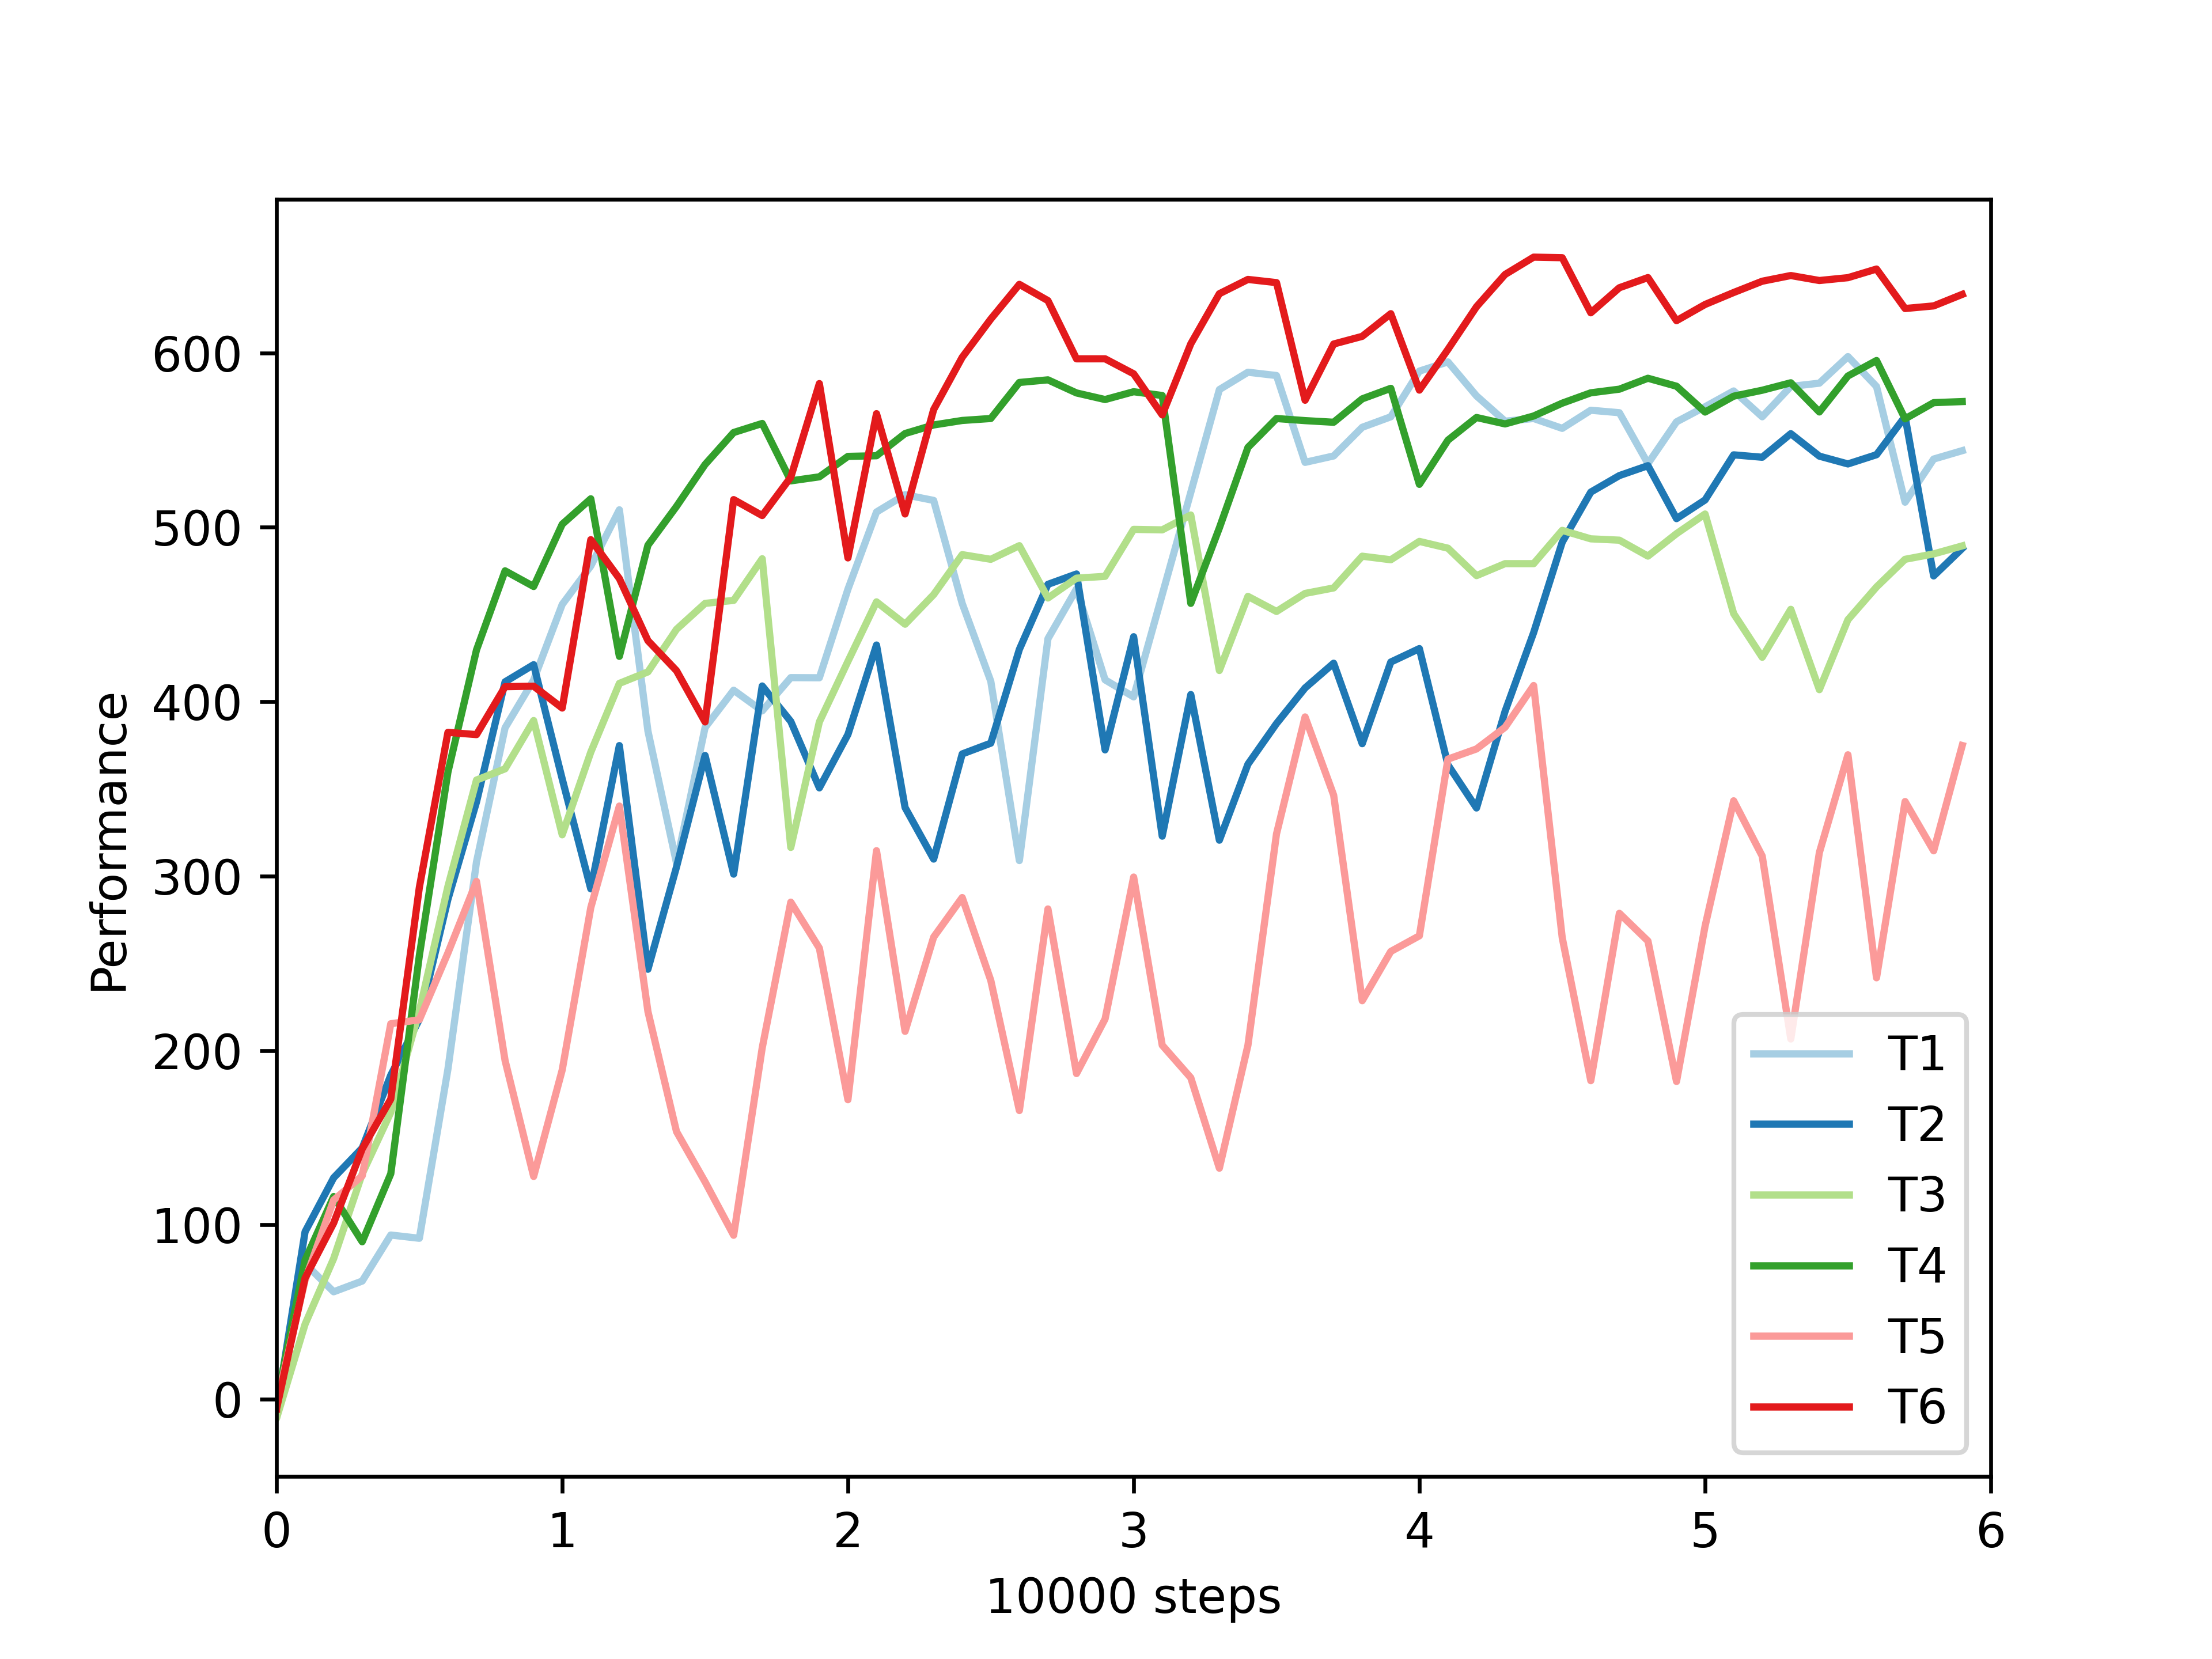}}
    \subcaptionbox{DT + EWC}
    {\includegraphics[width=0.245\linewidth]{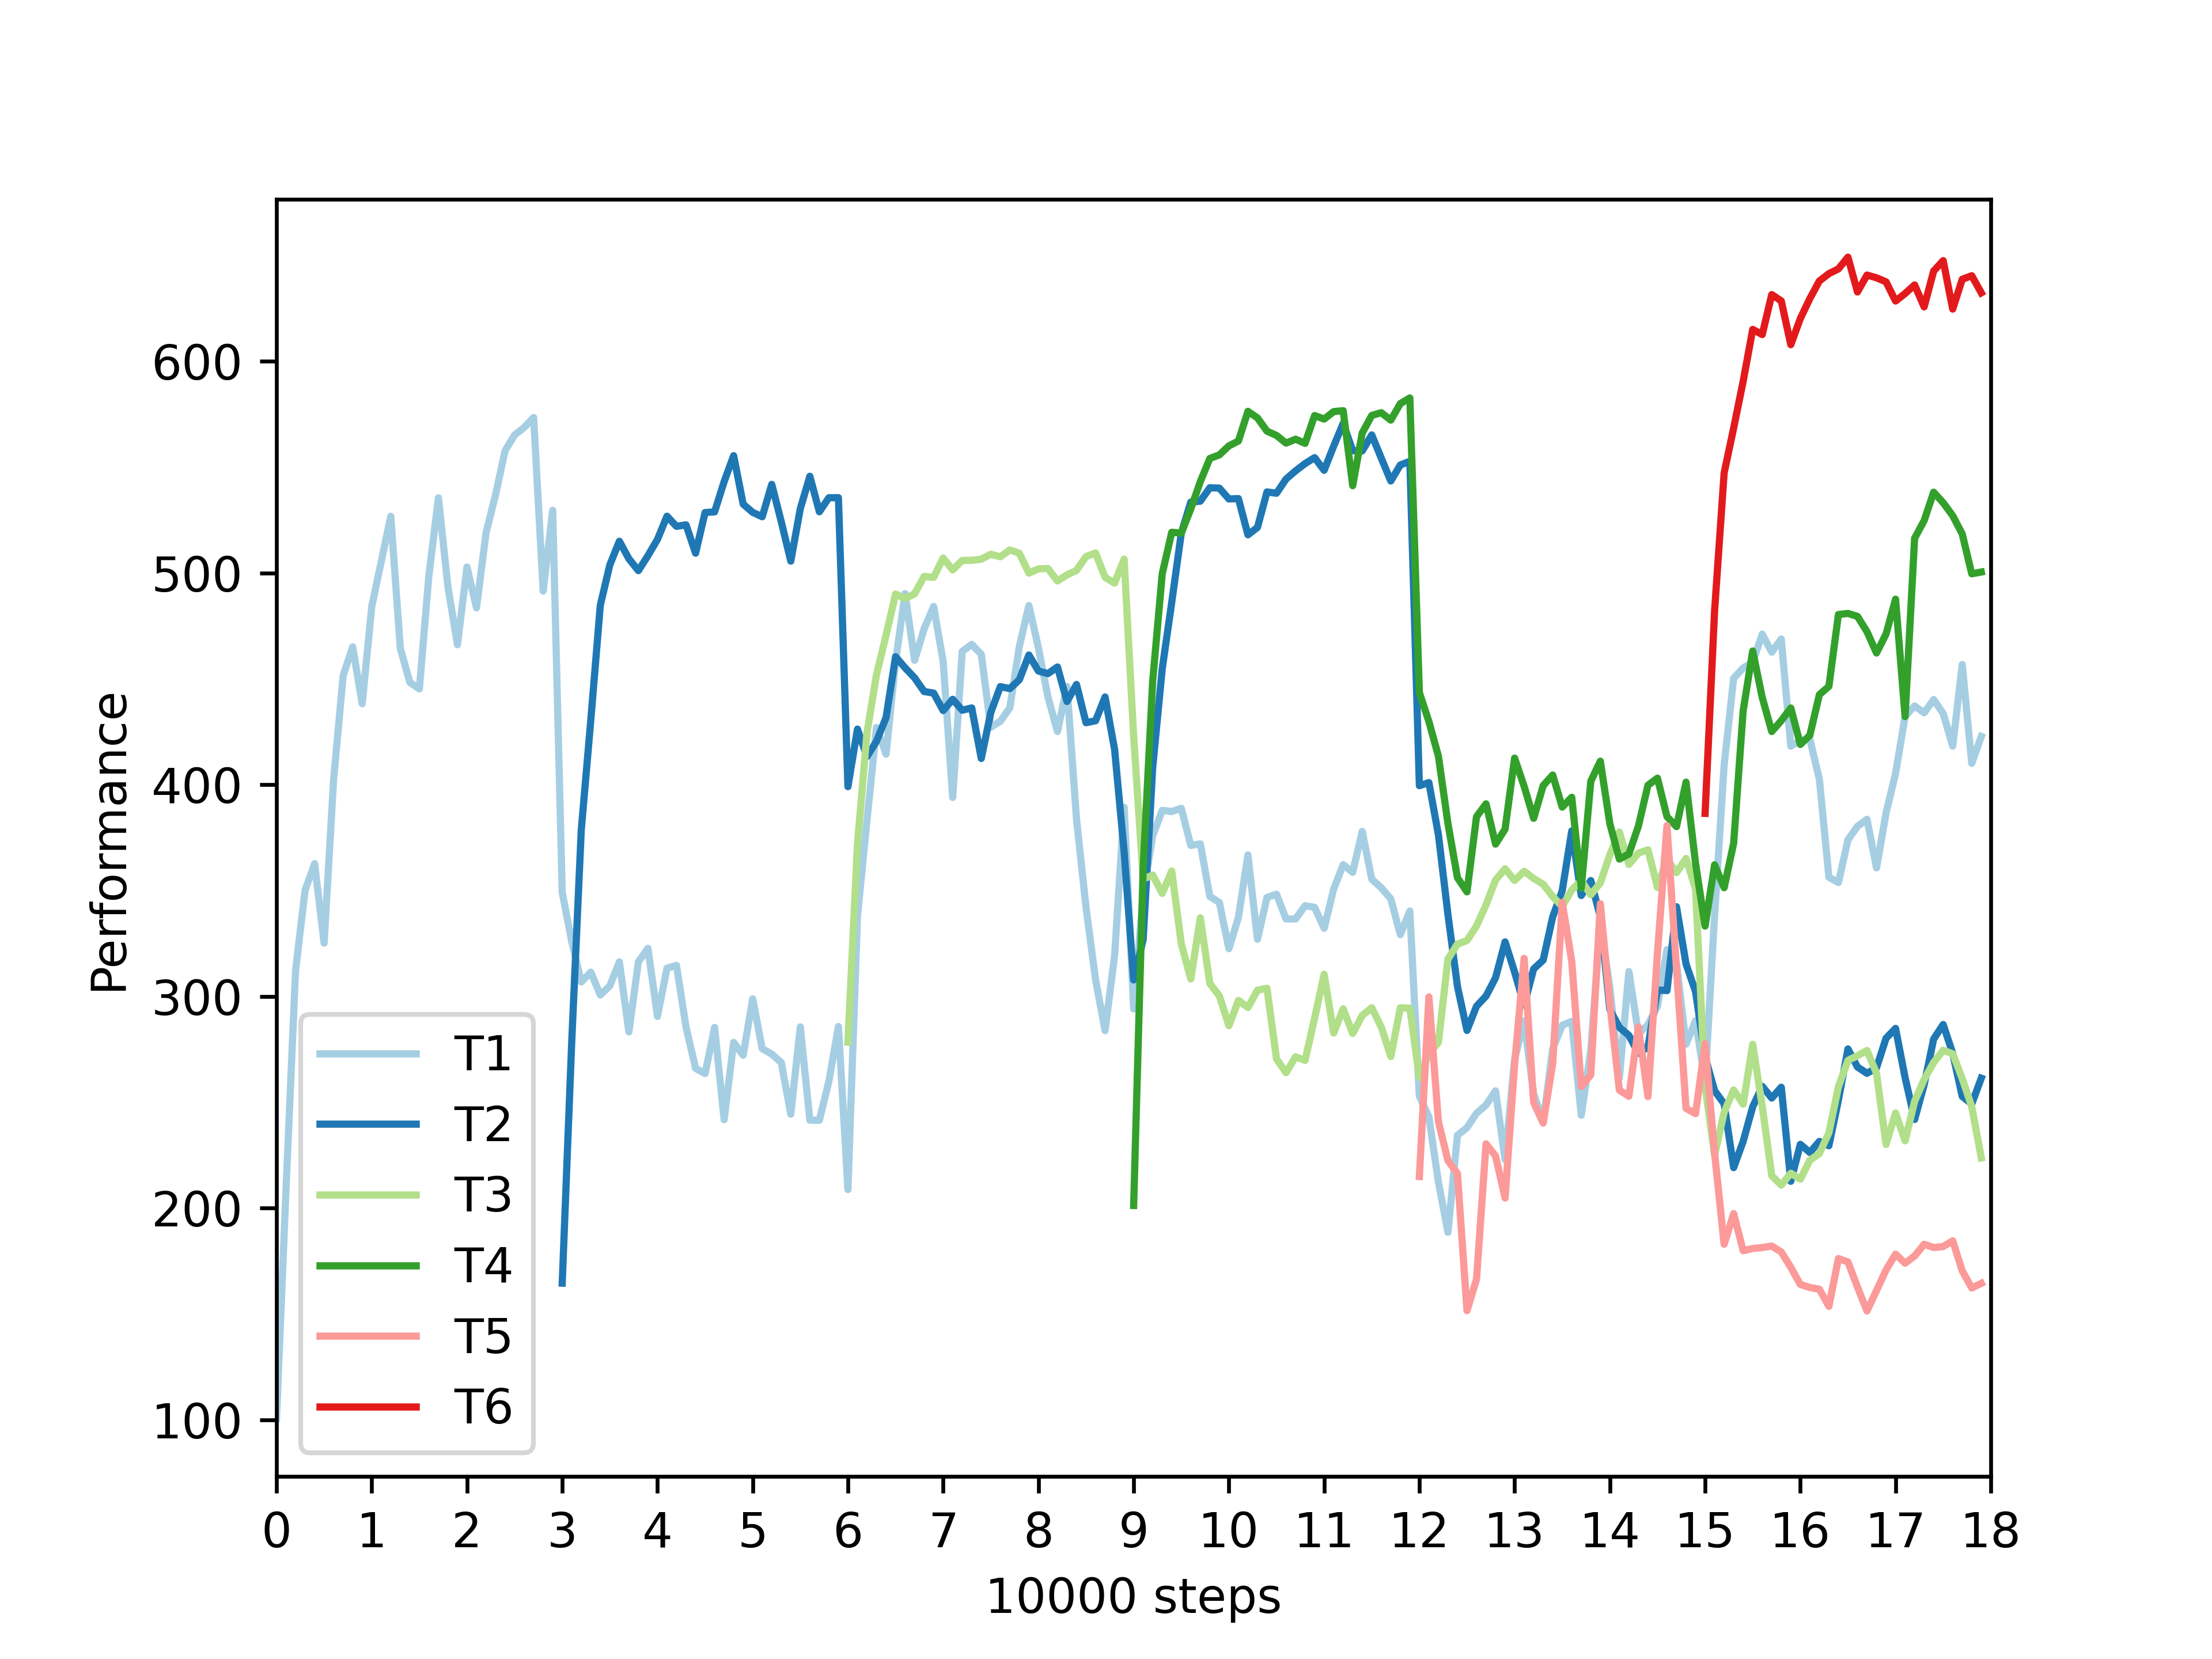}}
    \subcaptionbox{DT + SI}
    {\includegraphics[width=0.245\linewidth]{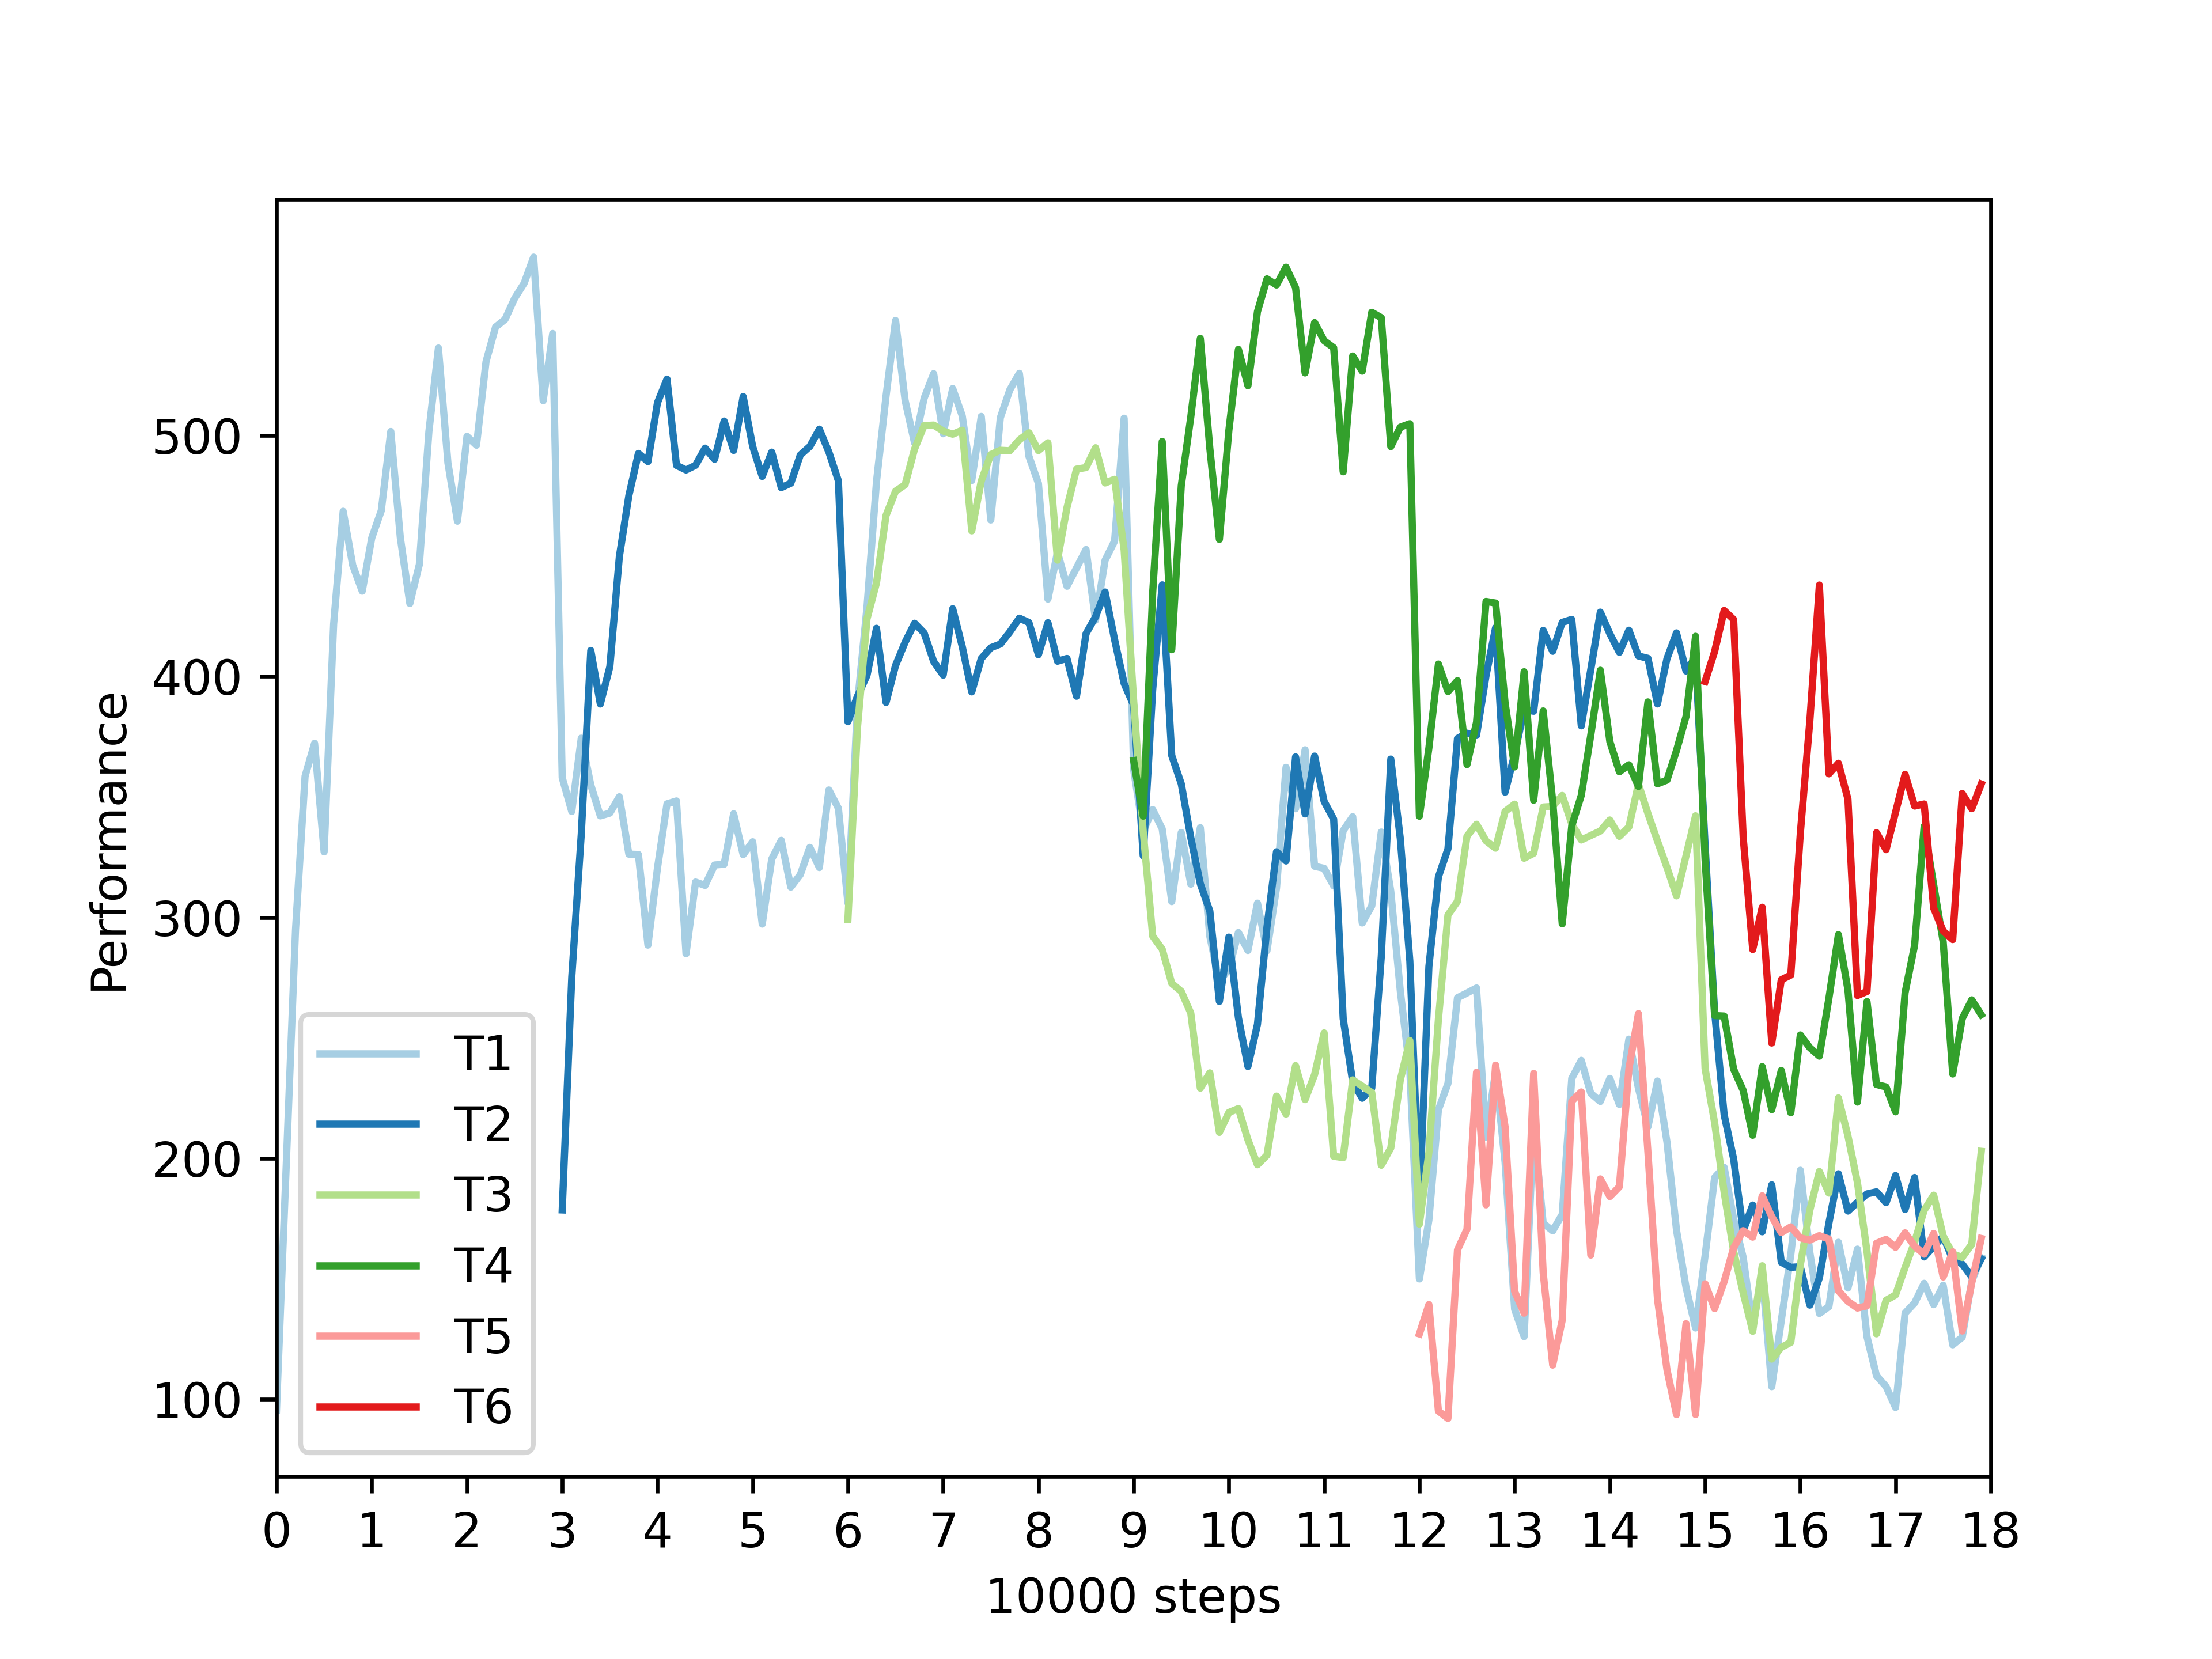}}
    \subcaptionbox{DT + GEM}
    {\includegraphics[width=0.245\linewidth]{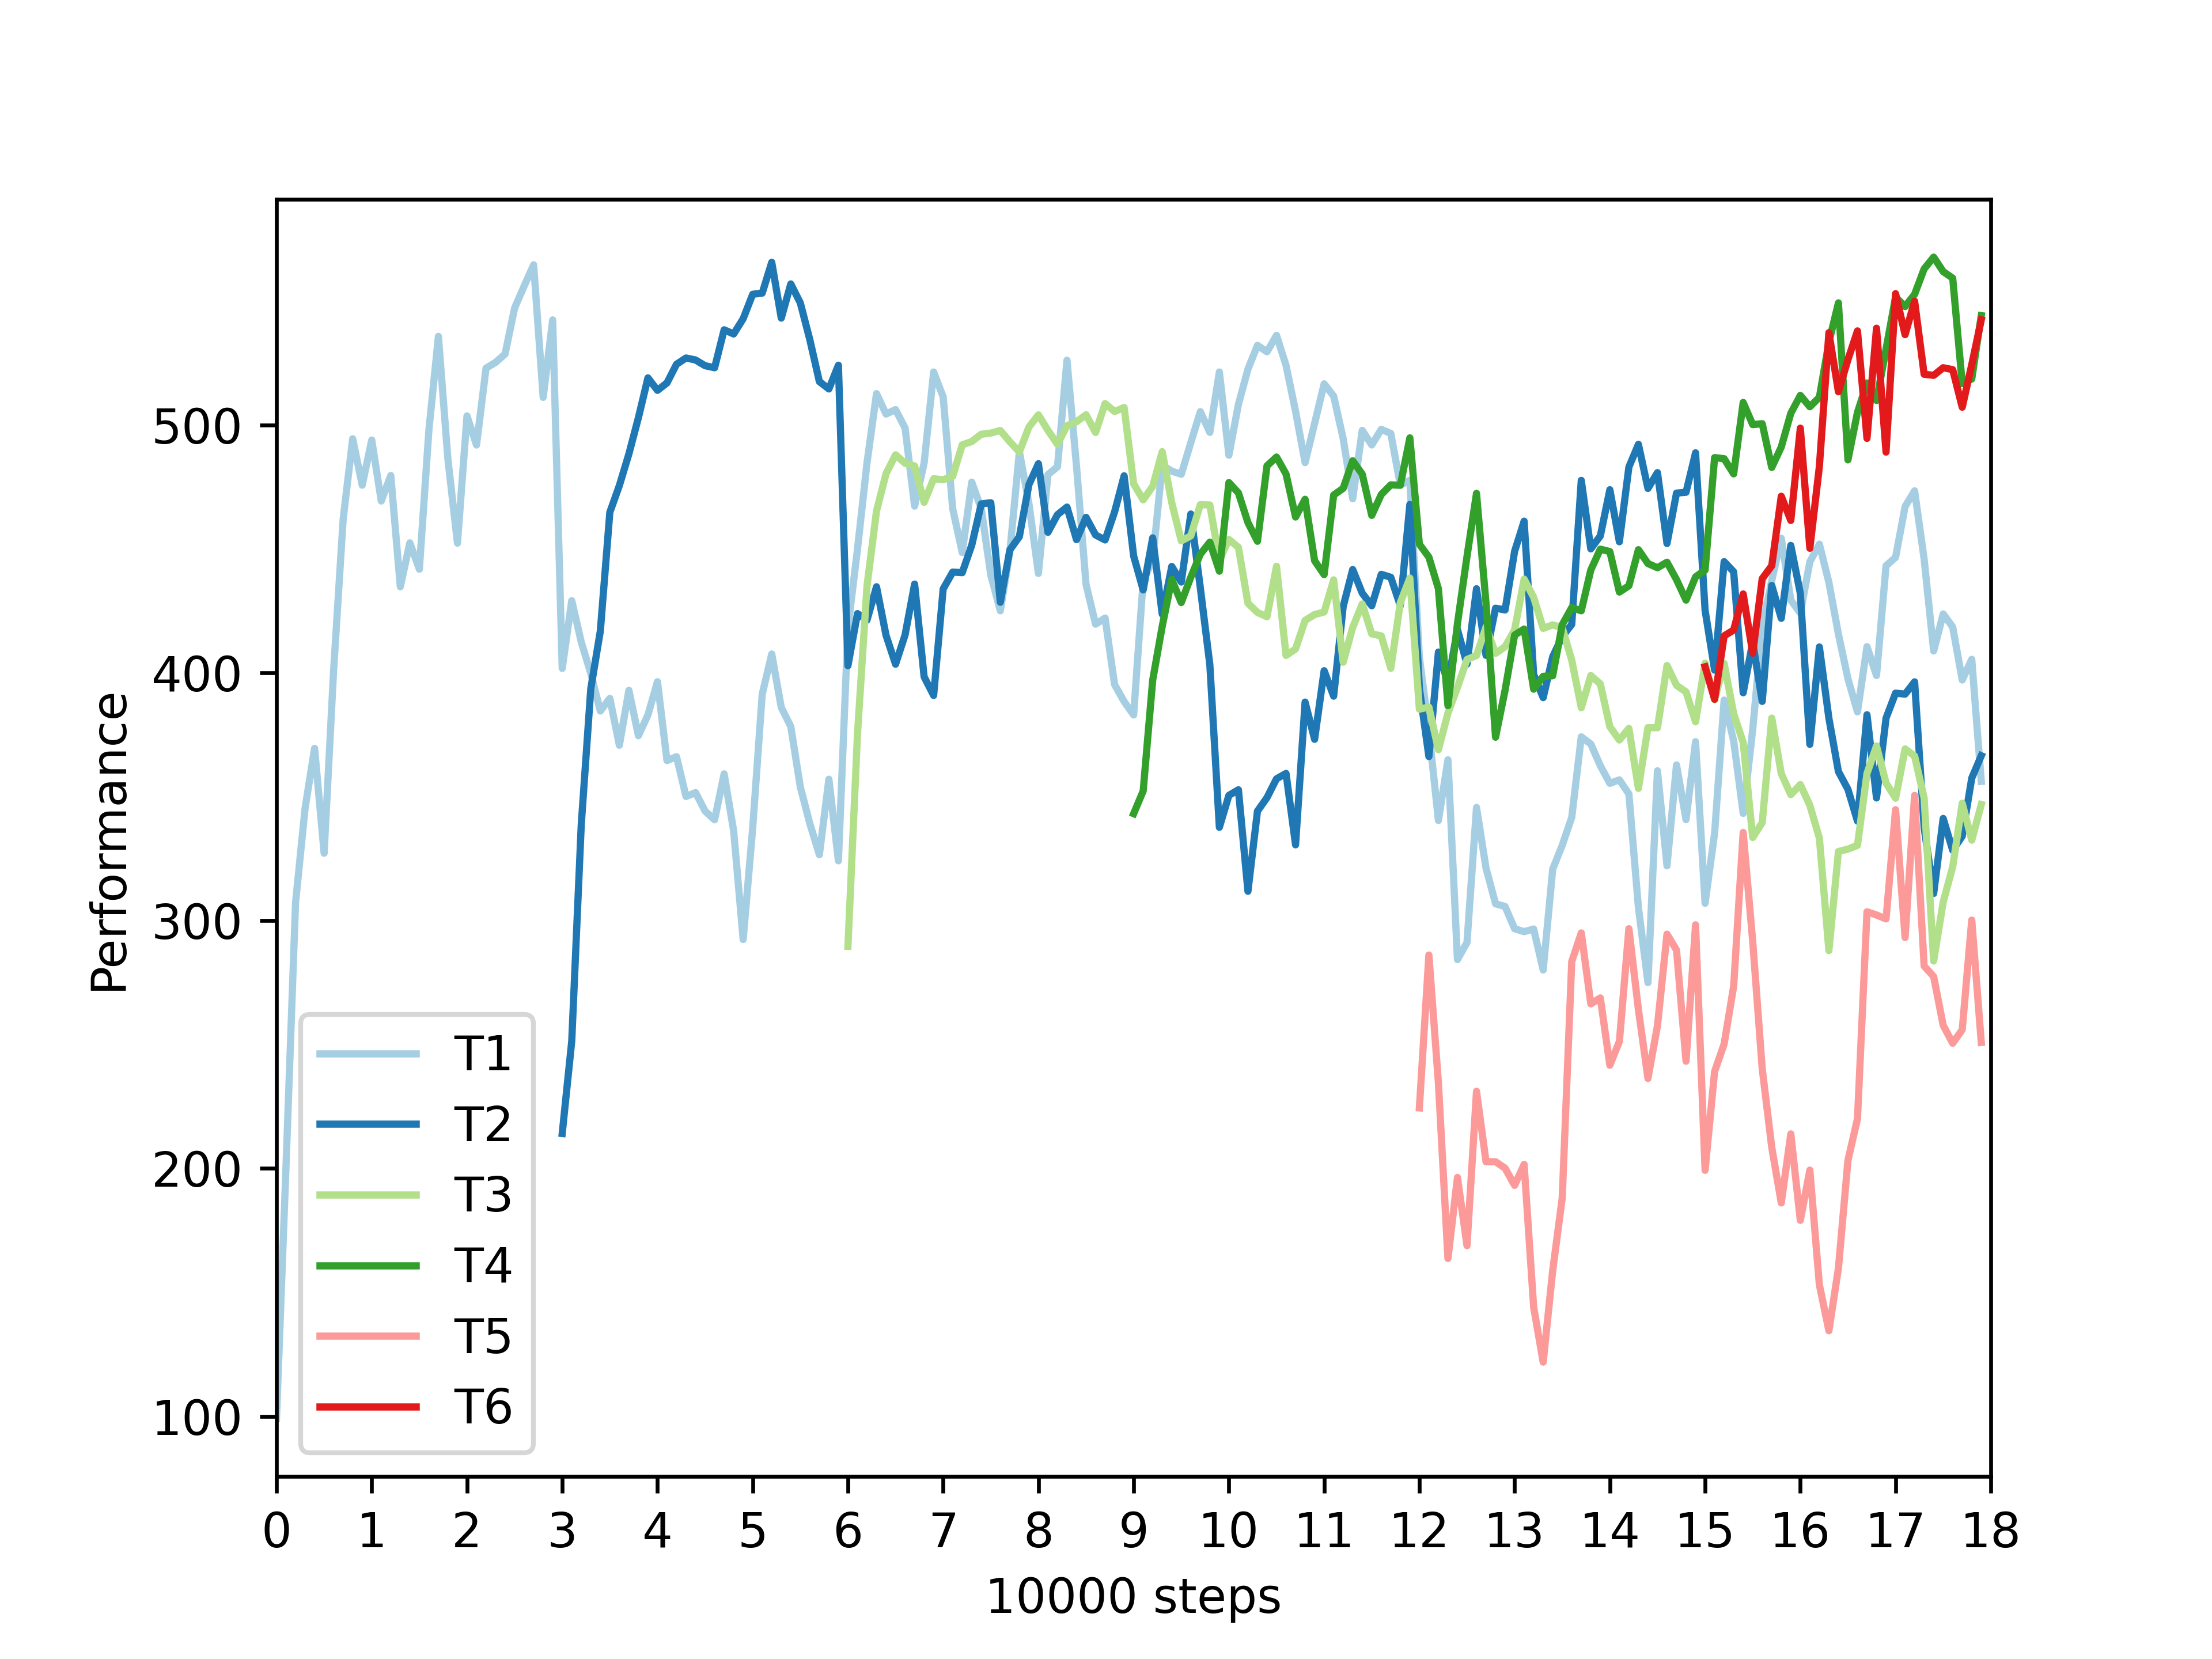}}

     \centering	
     \subcaptionbox{Vanilla DT}
    {\includegraphics[width=0.245\linewidth]{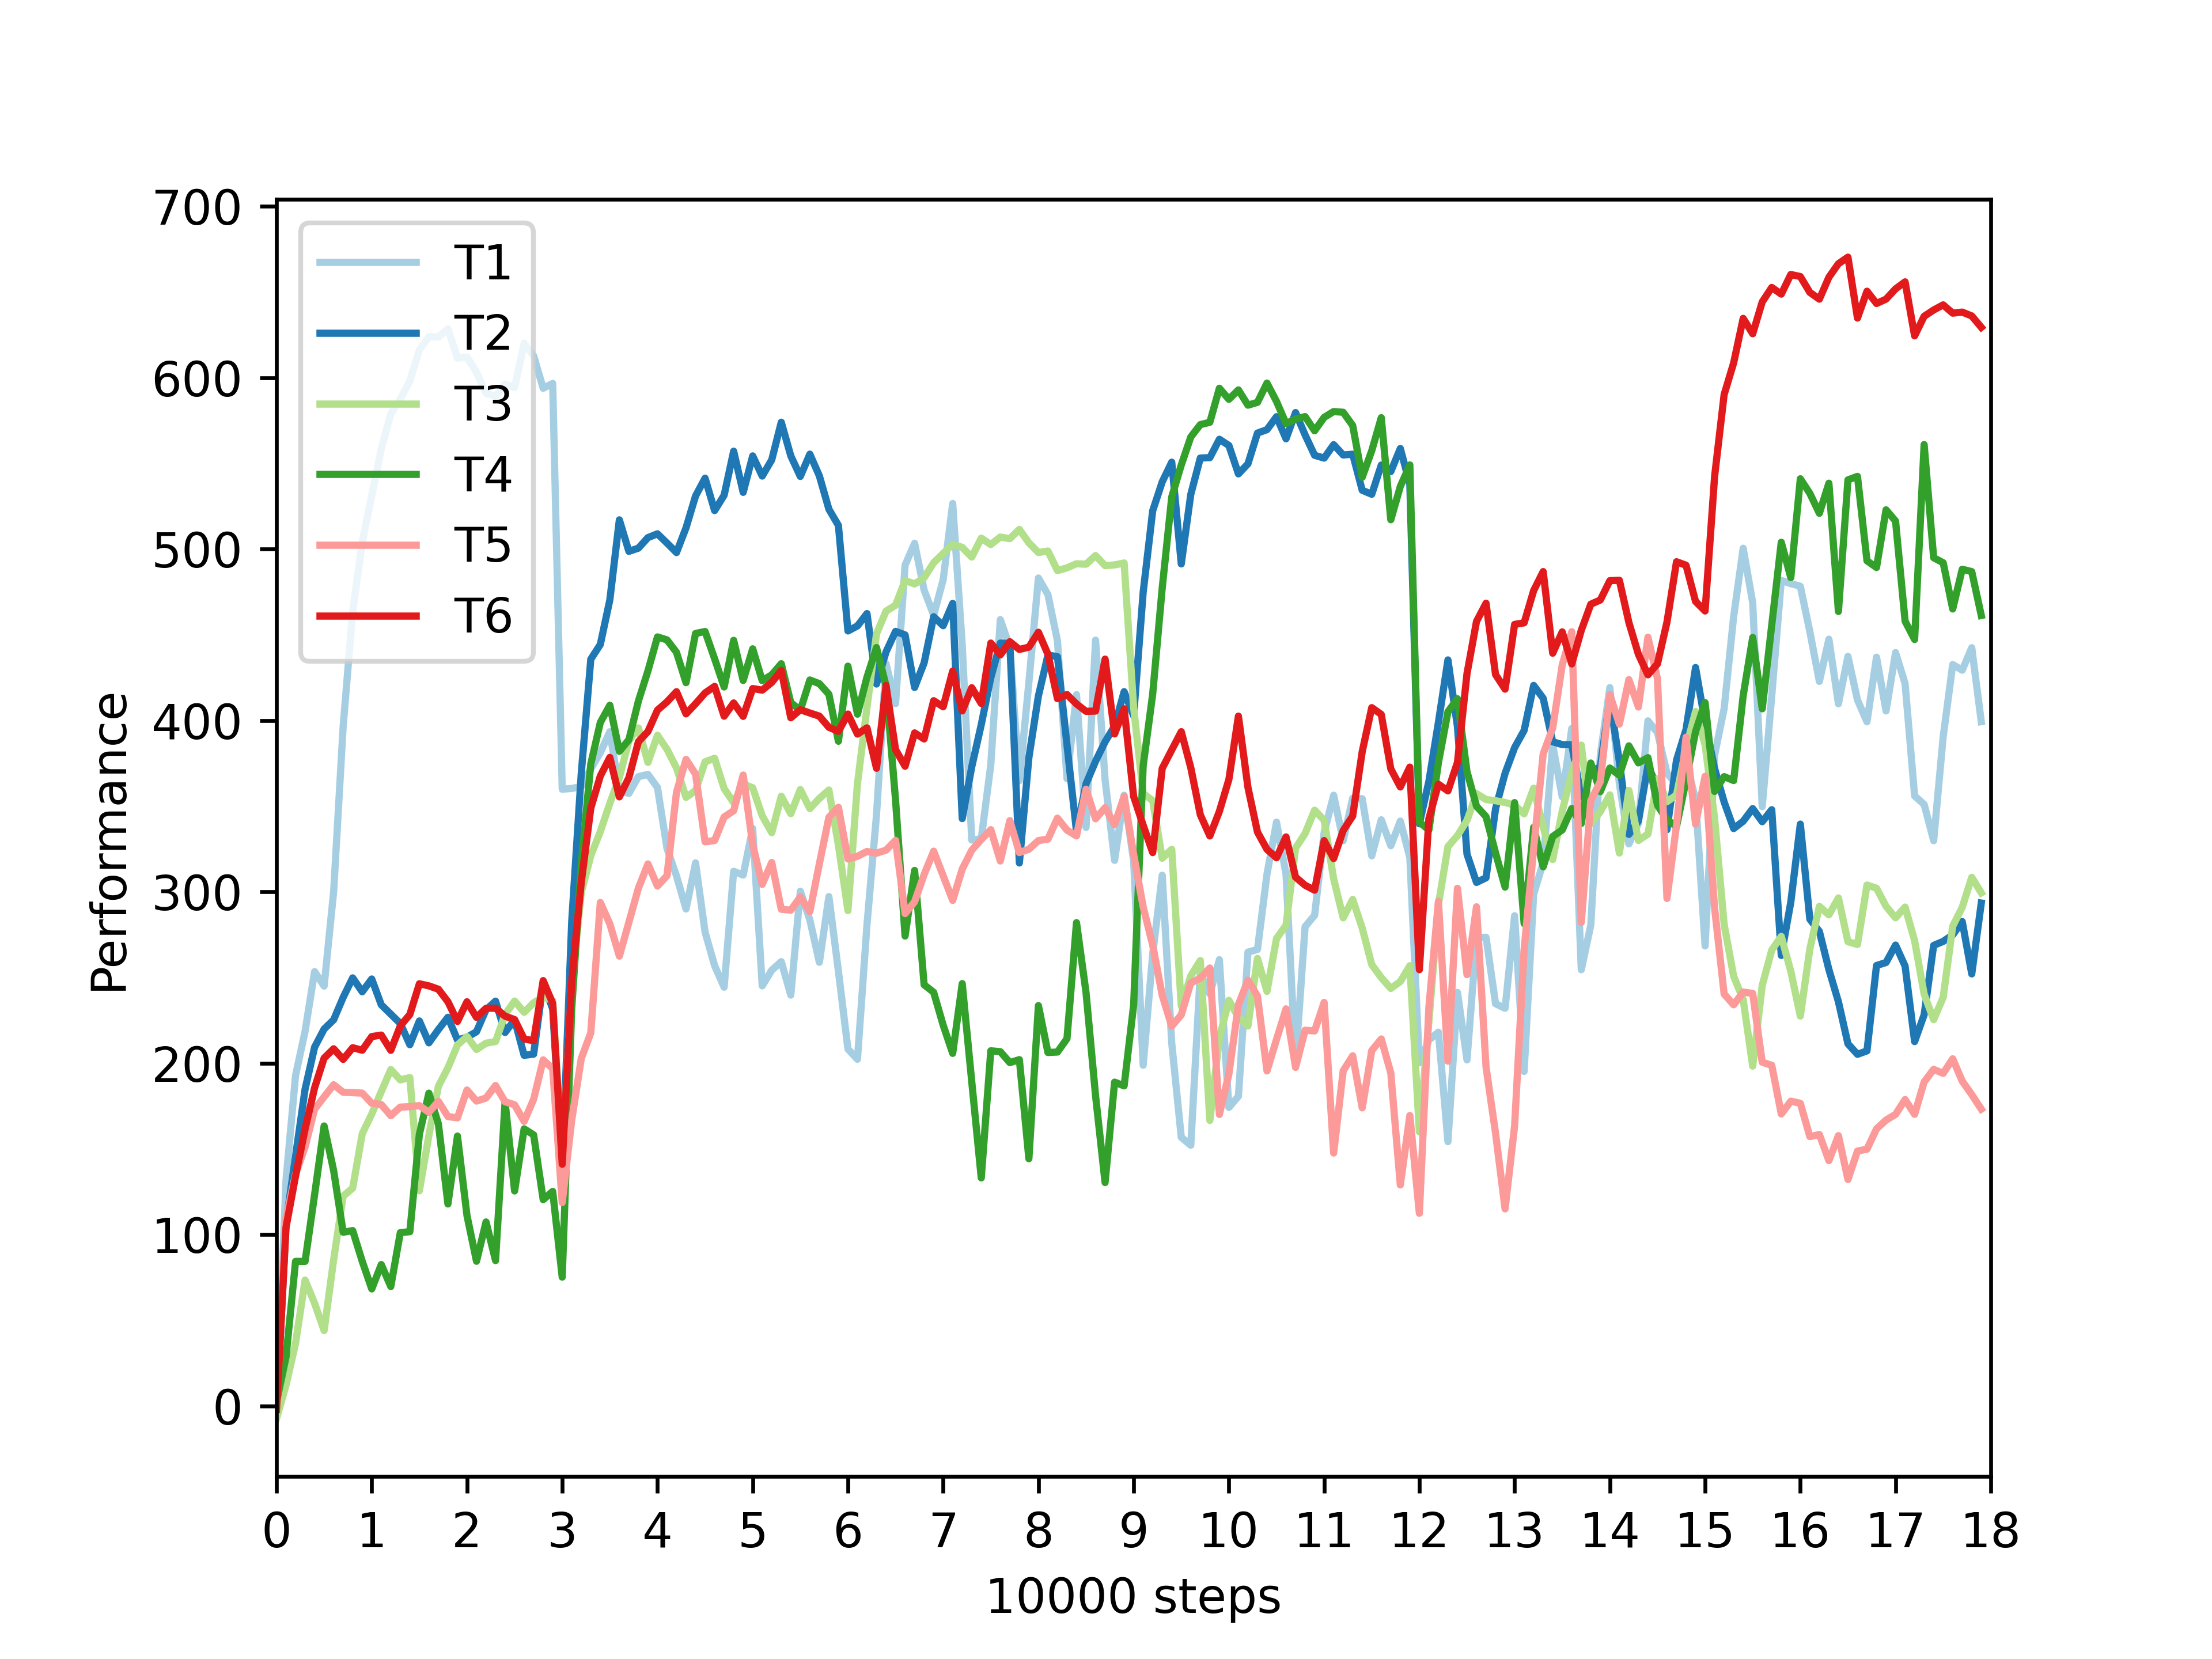}}
      \subcaptionbox{OER}
    {\includegraphics[width=0.245\linewidth]{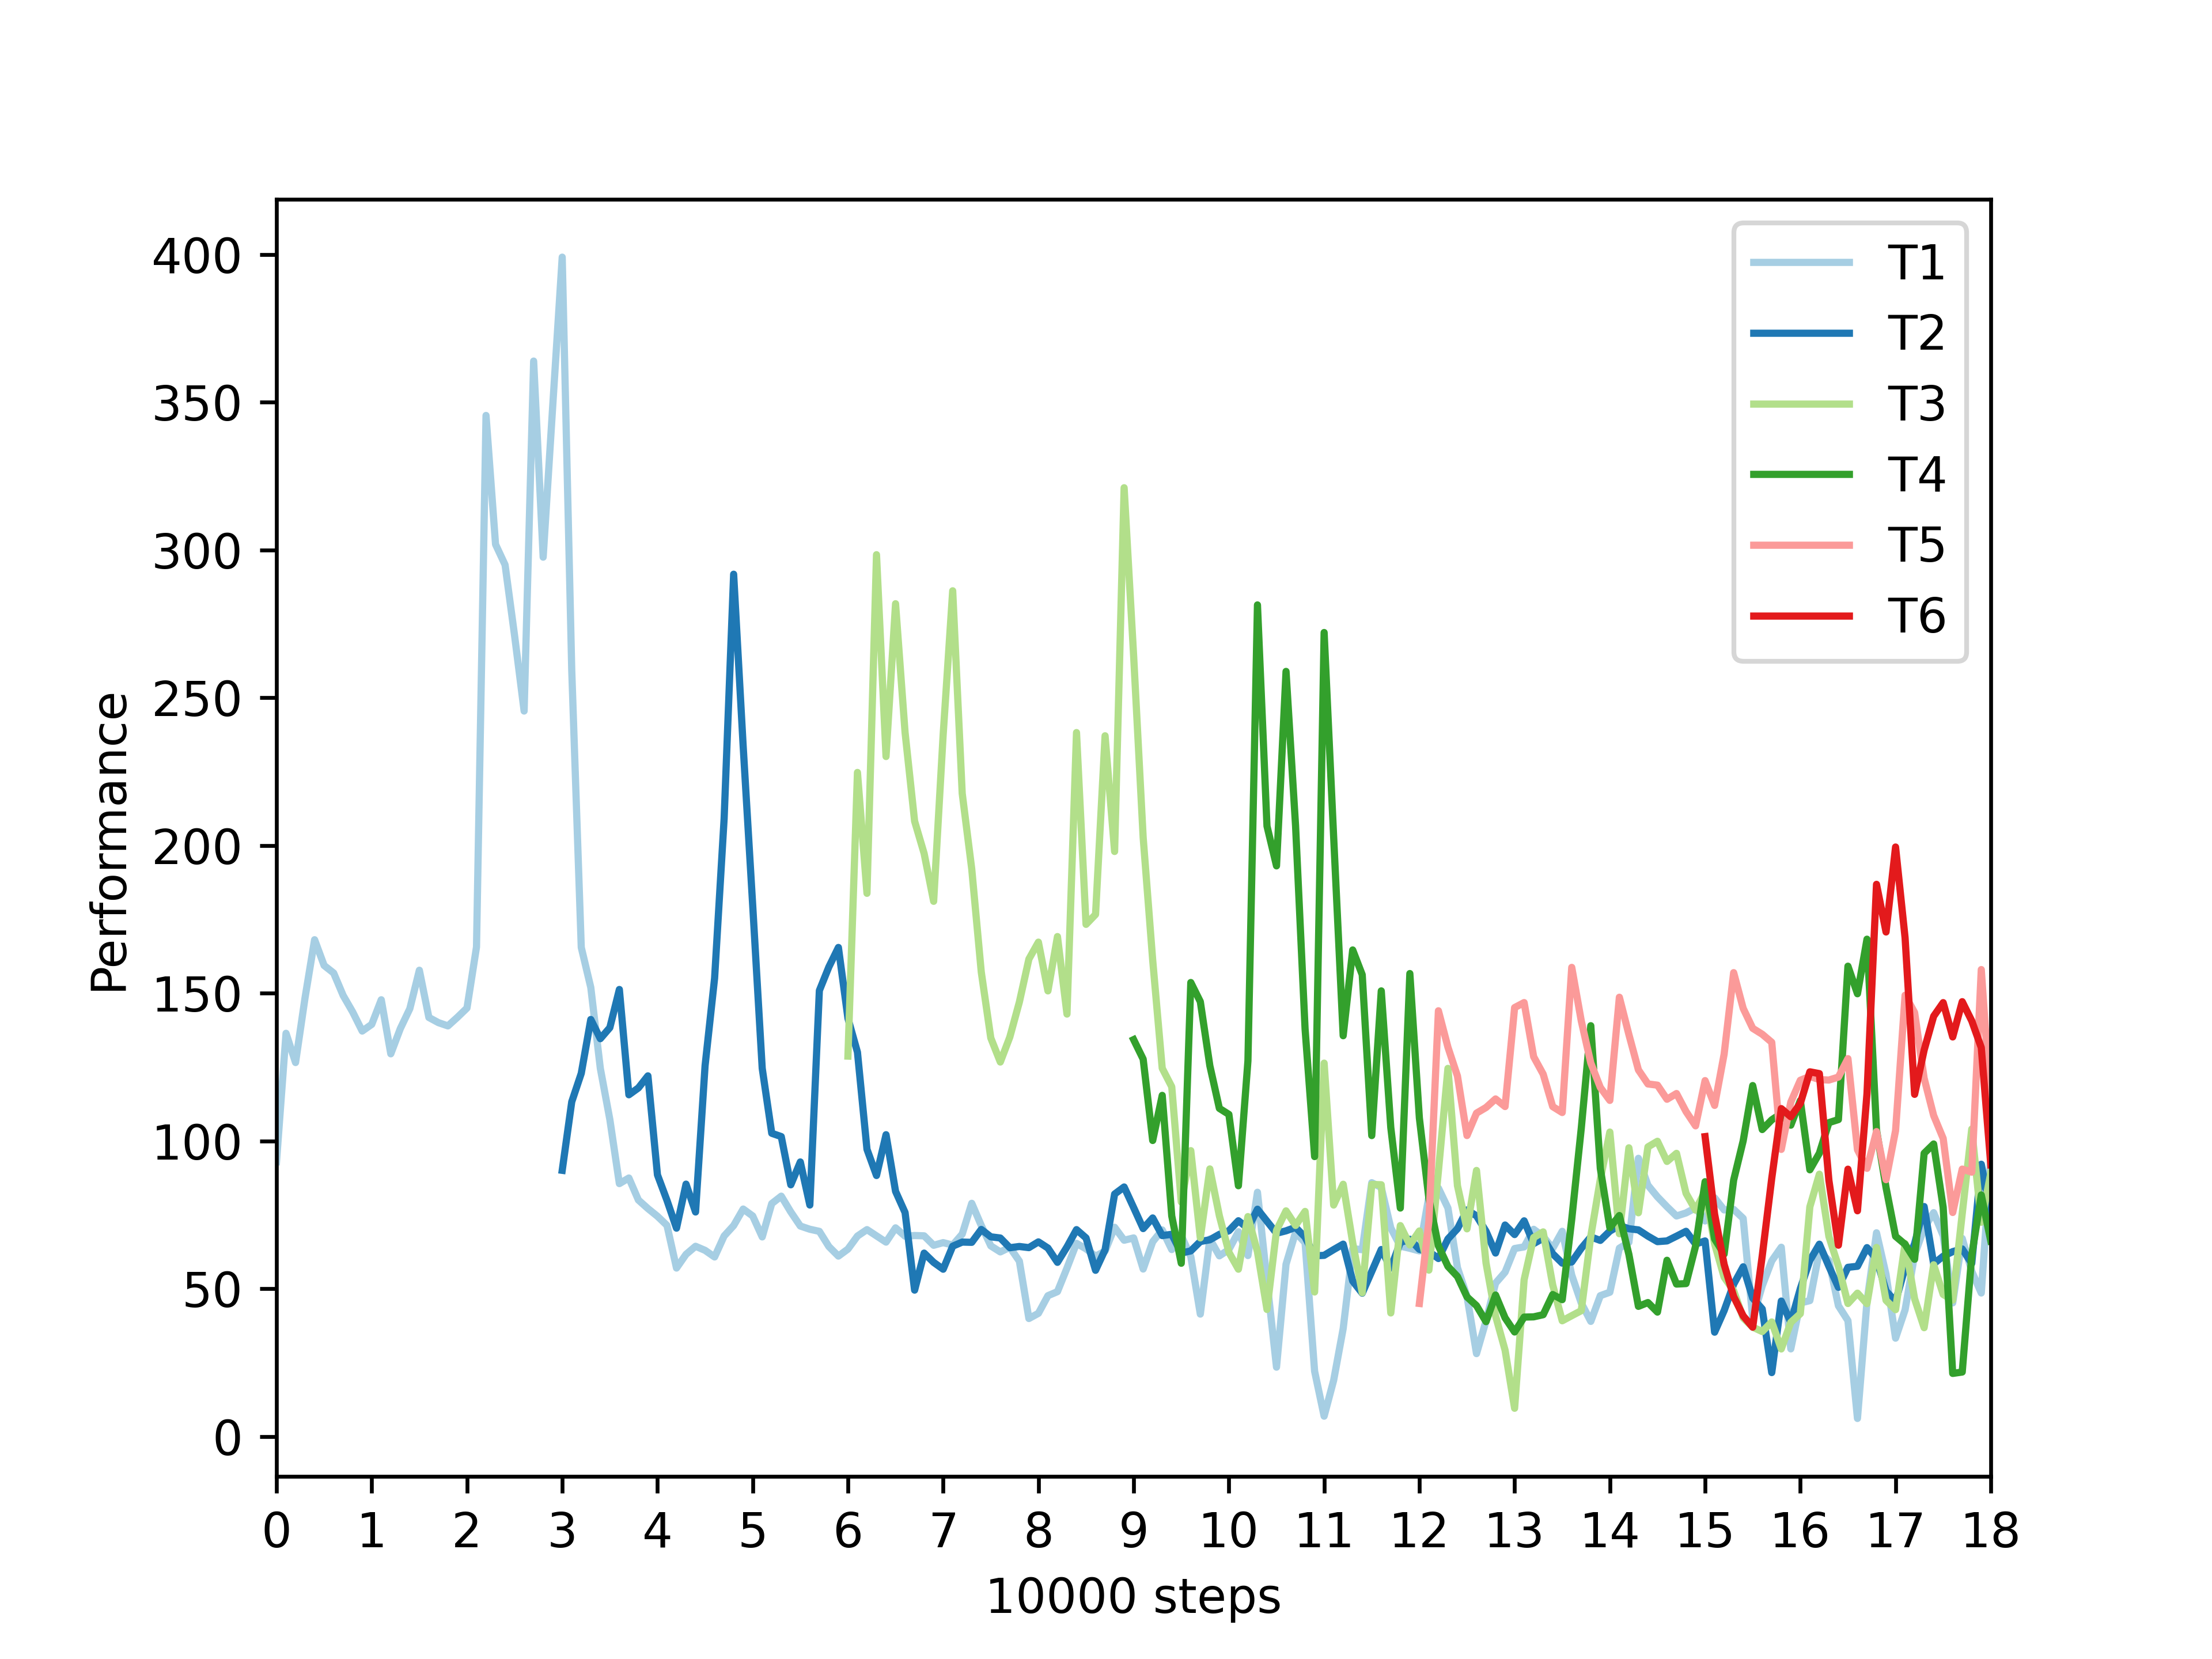}}
     \subcaptionbox{MH-DT}
    {\includegraphics[width=0.245\linewidth]{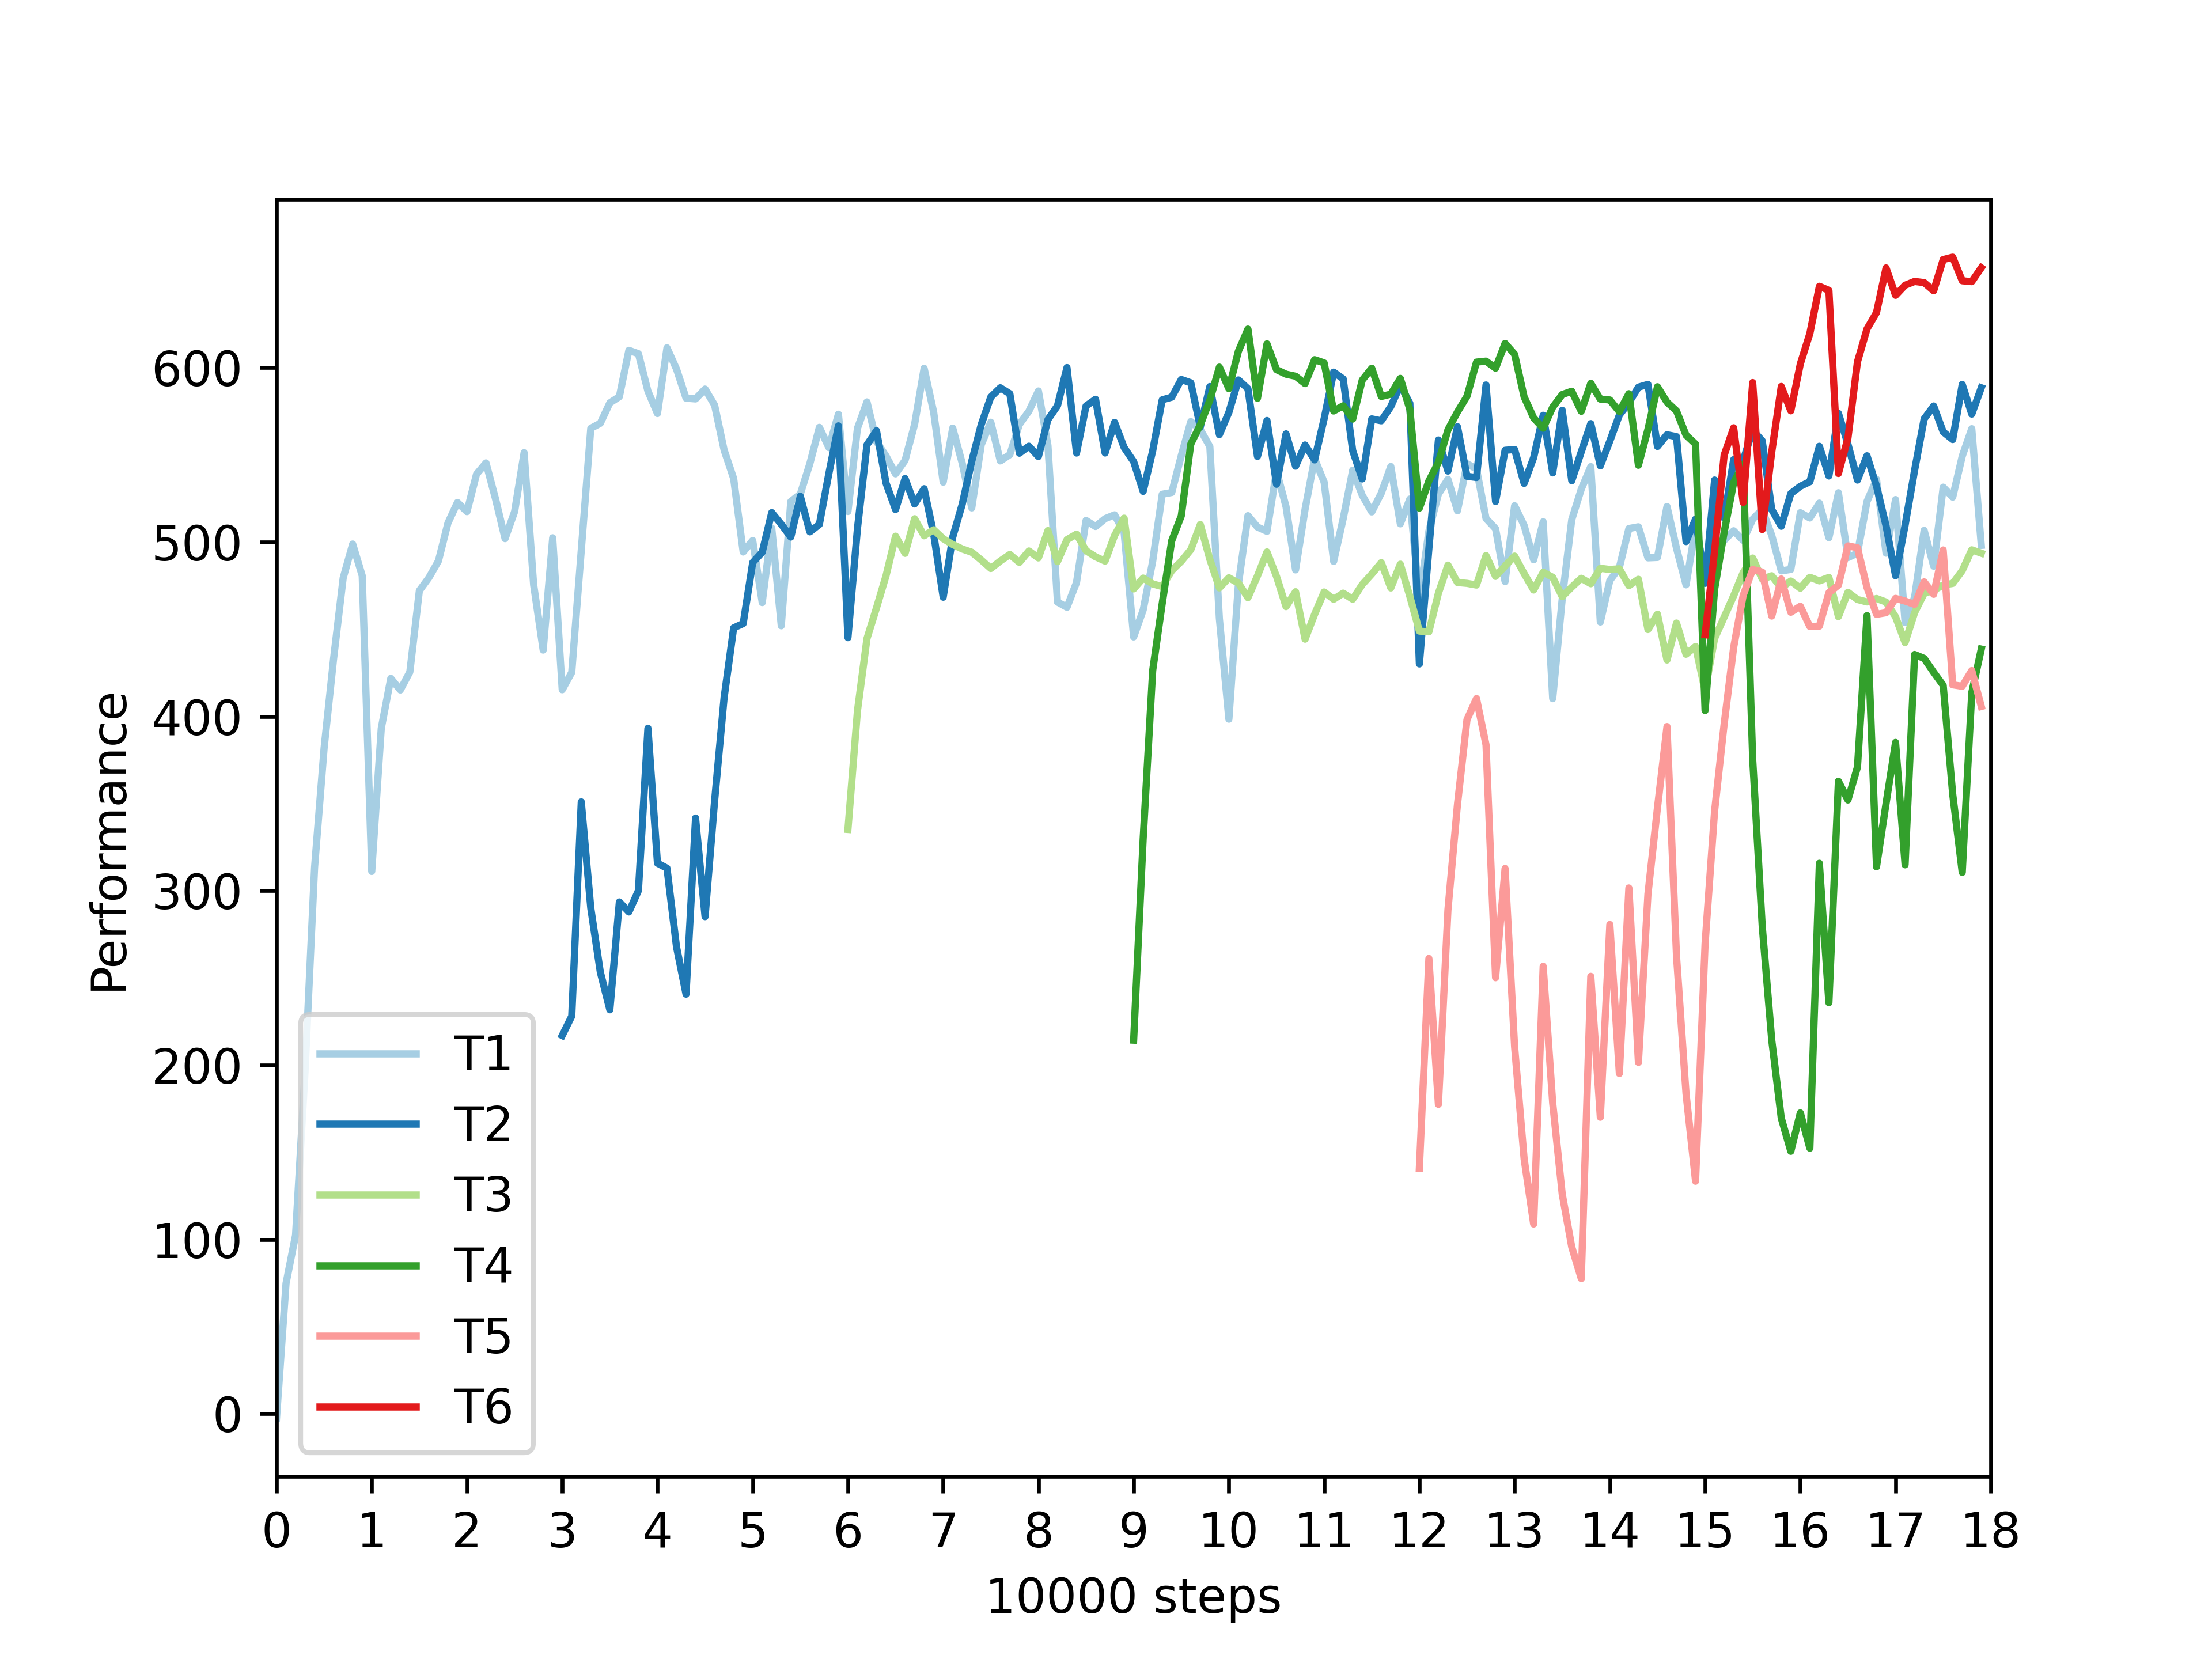}}
	\subcaptionbox{LoRA-DT}
    {\includegraphics[width=0.245\linewidth]{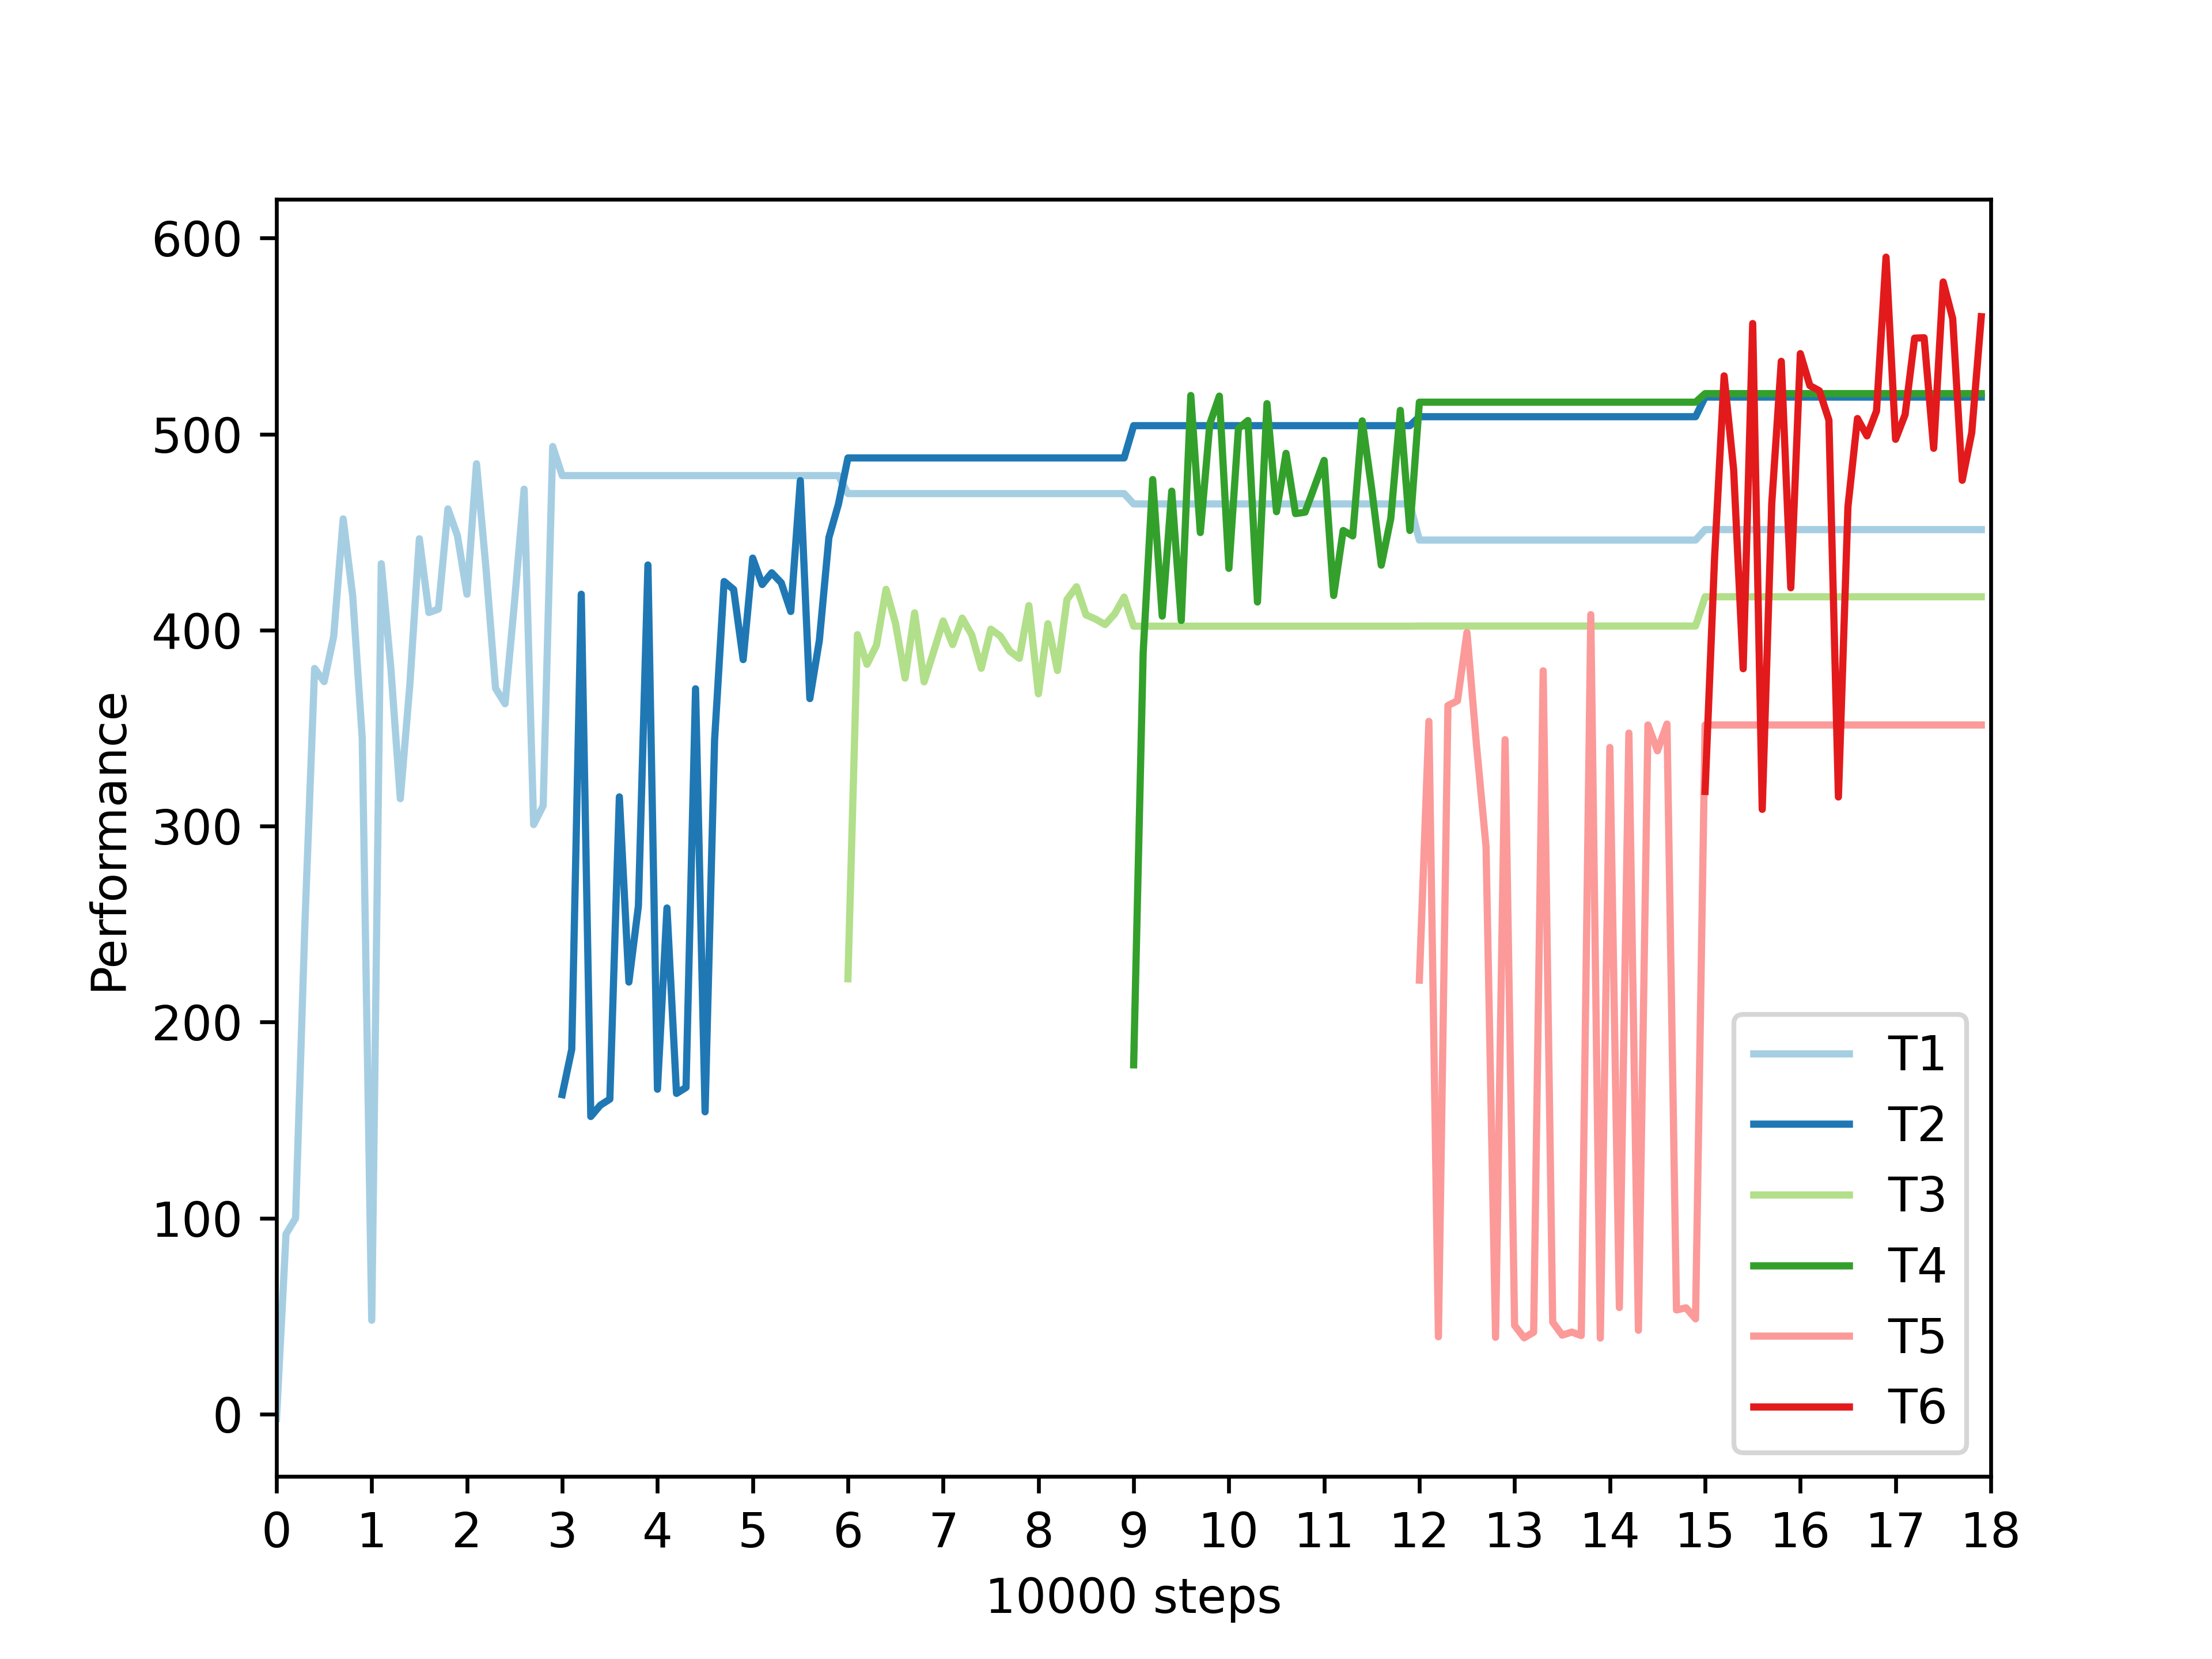}}
    \caption{Walker\_Param (middle)}
\end{figure}

\begin{figure}[htbp]
	\centering
	\subcaptionbox{PDT}
    {\includegraphics[width=0.245\linewidth]{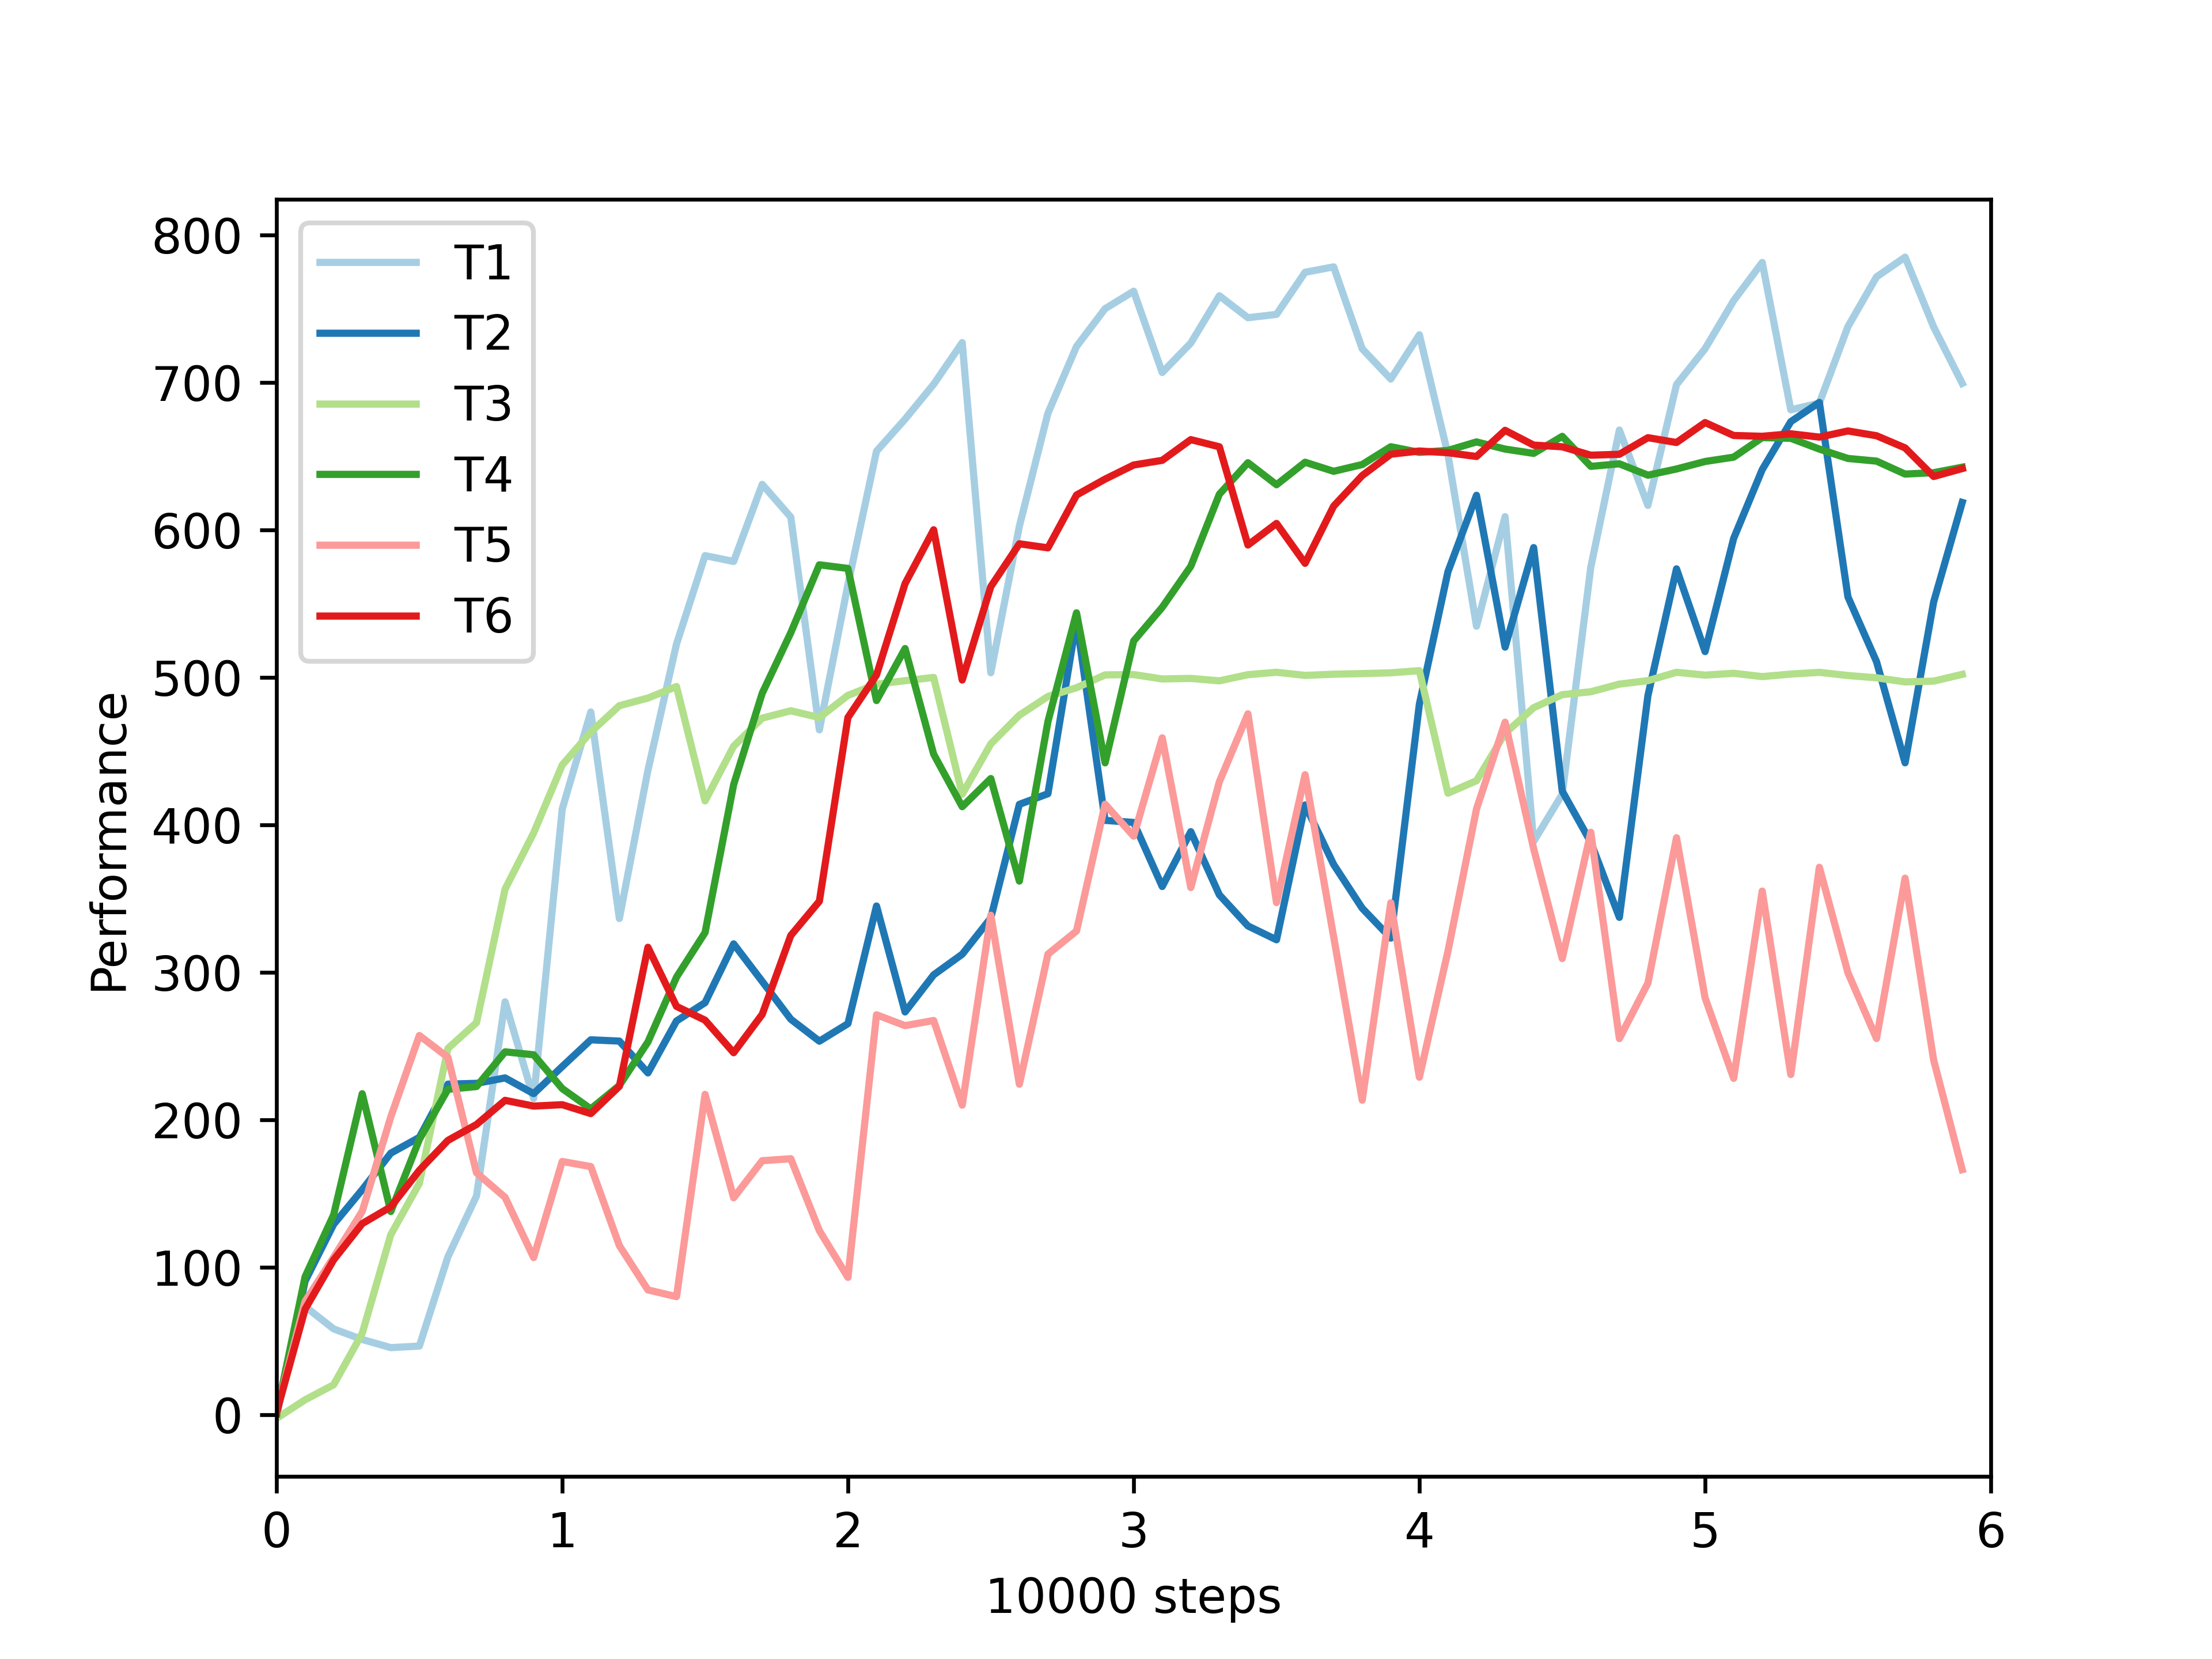}}
	\subcaptionbox{DT + EWC}
    {\includegraphics[width=0.245\linewidth]{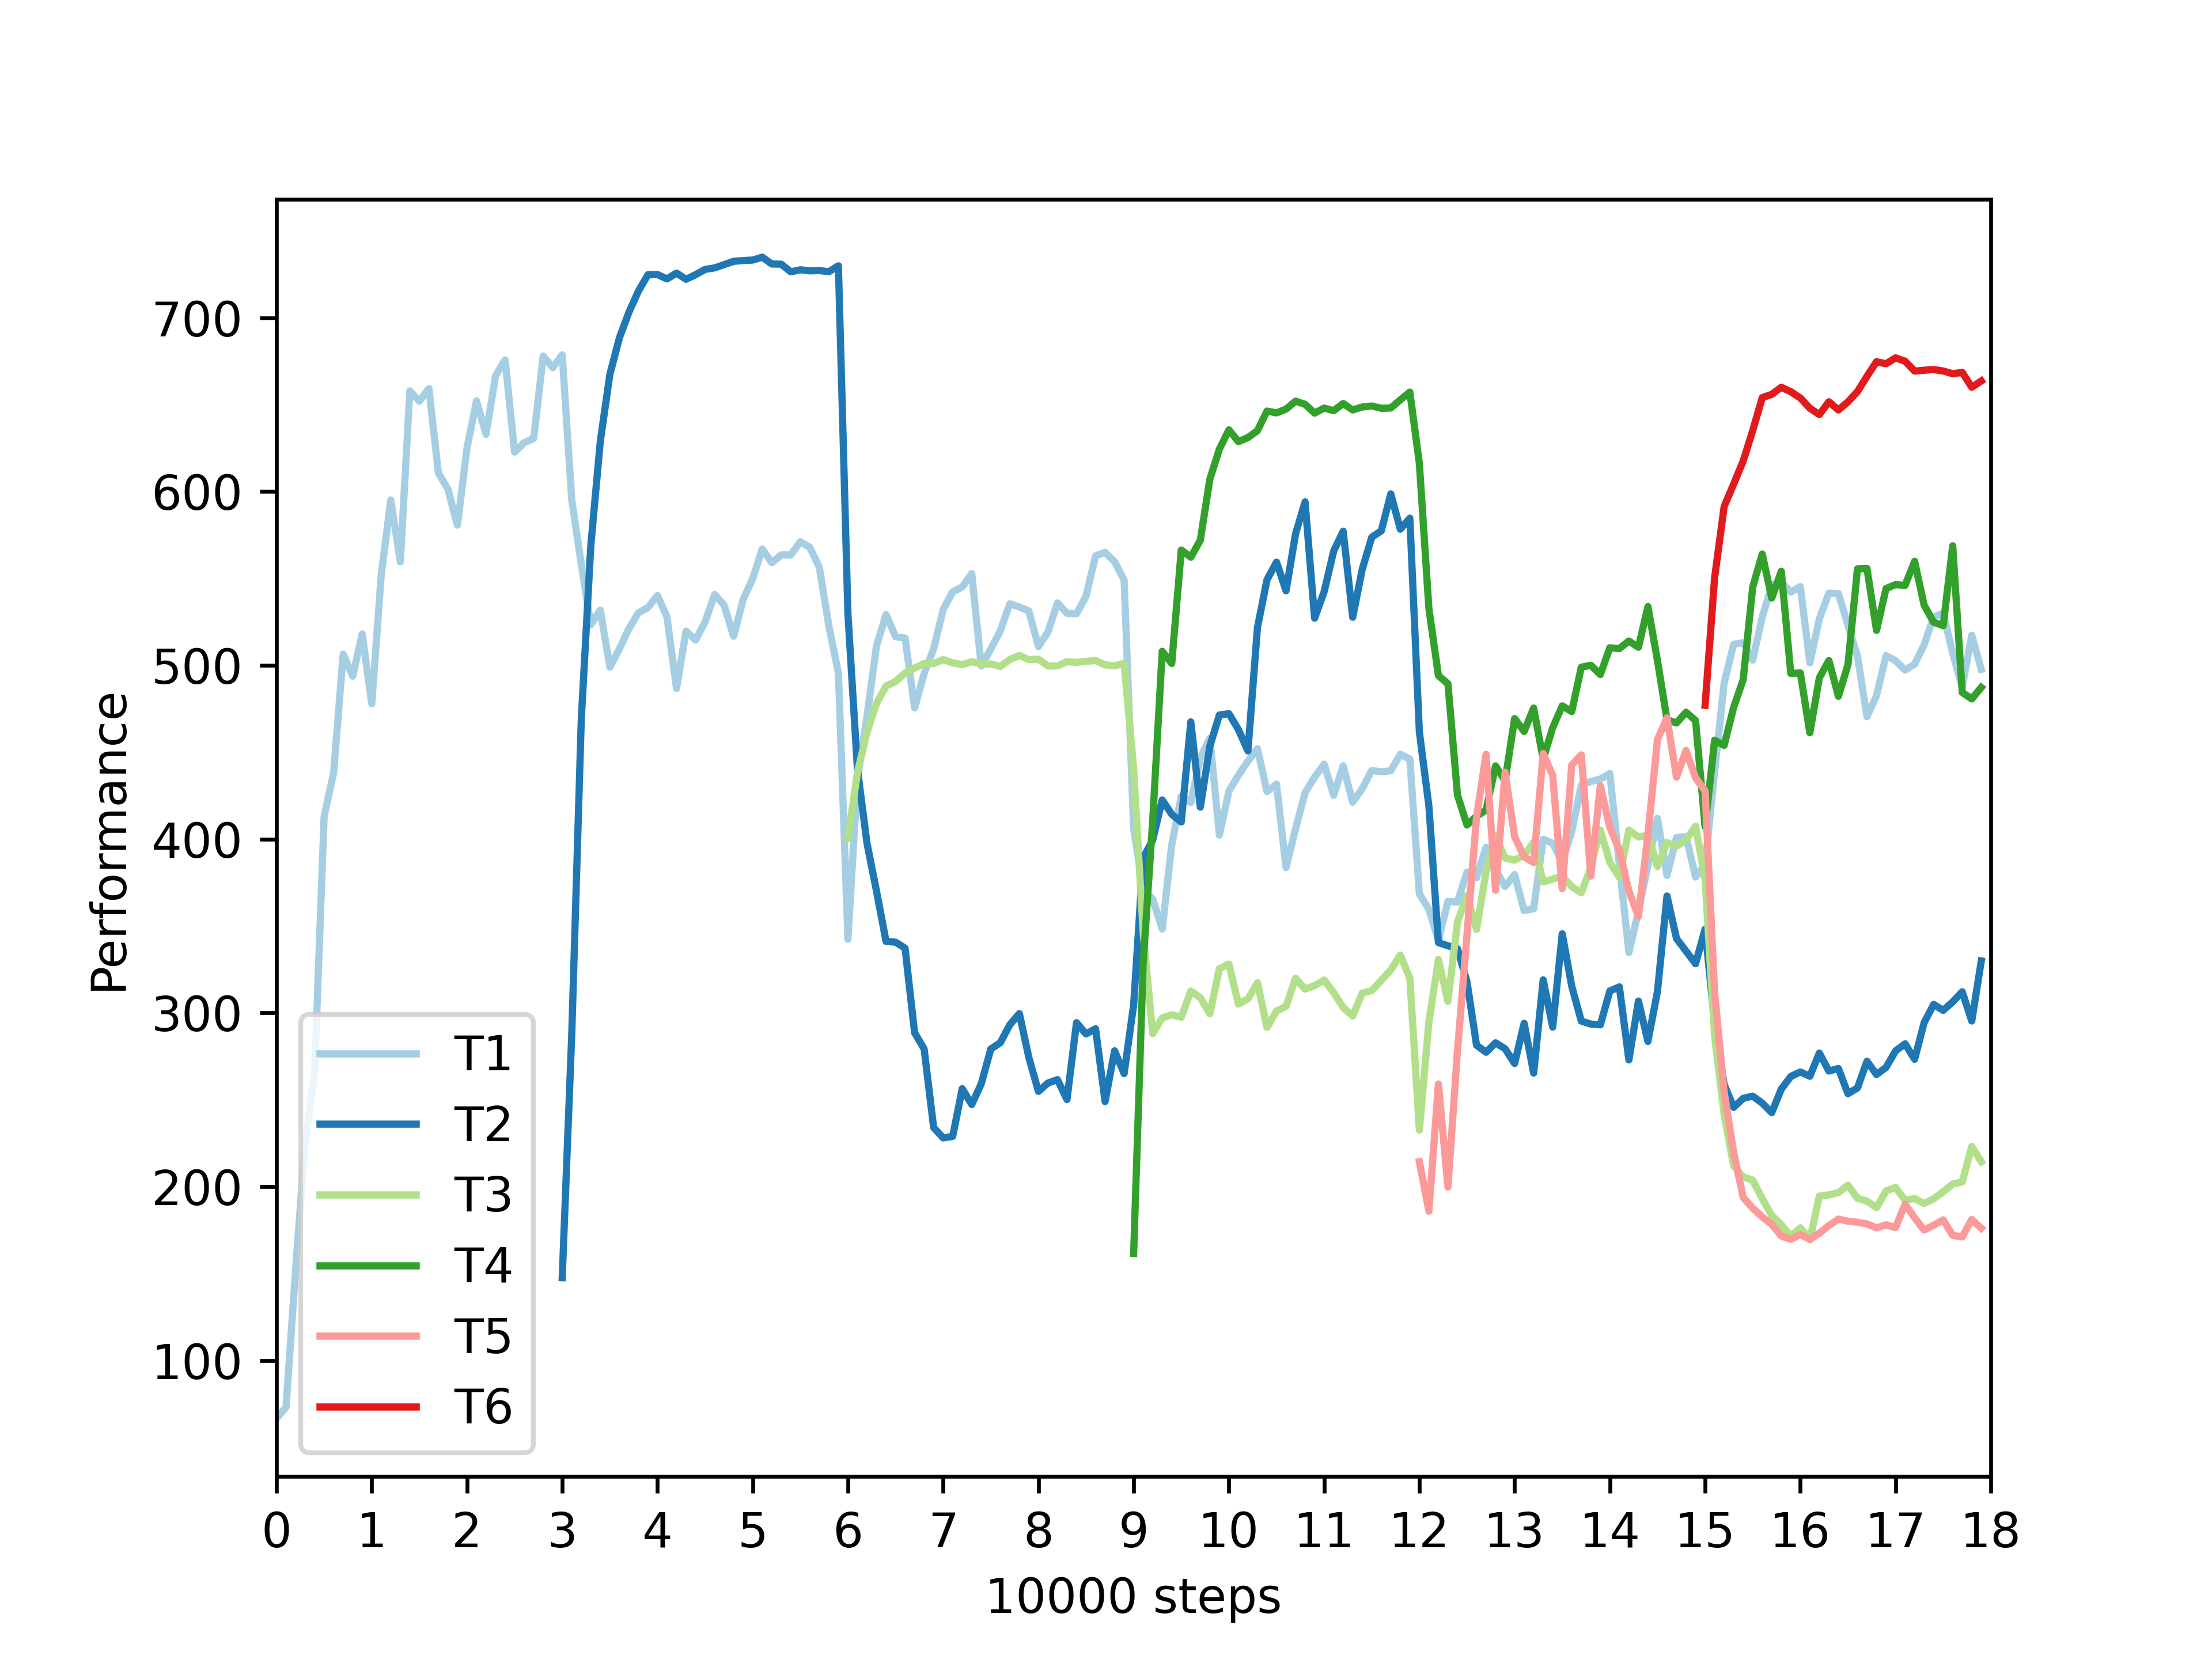}}
    \subcaptionbox{DT + SI}
    {\includegraphics[width=0.245\linewidth]{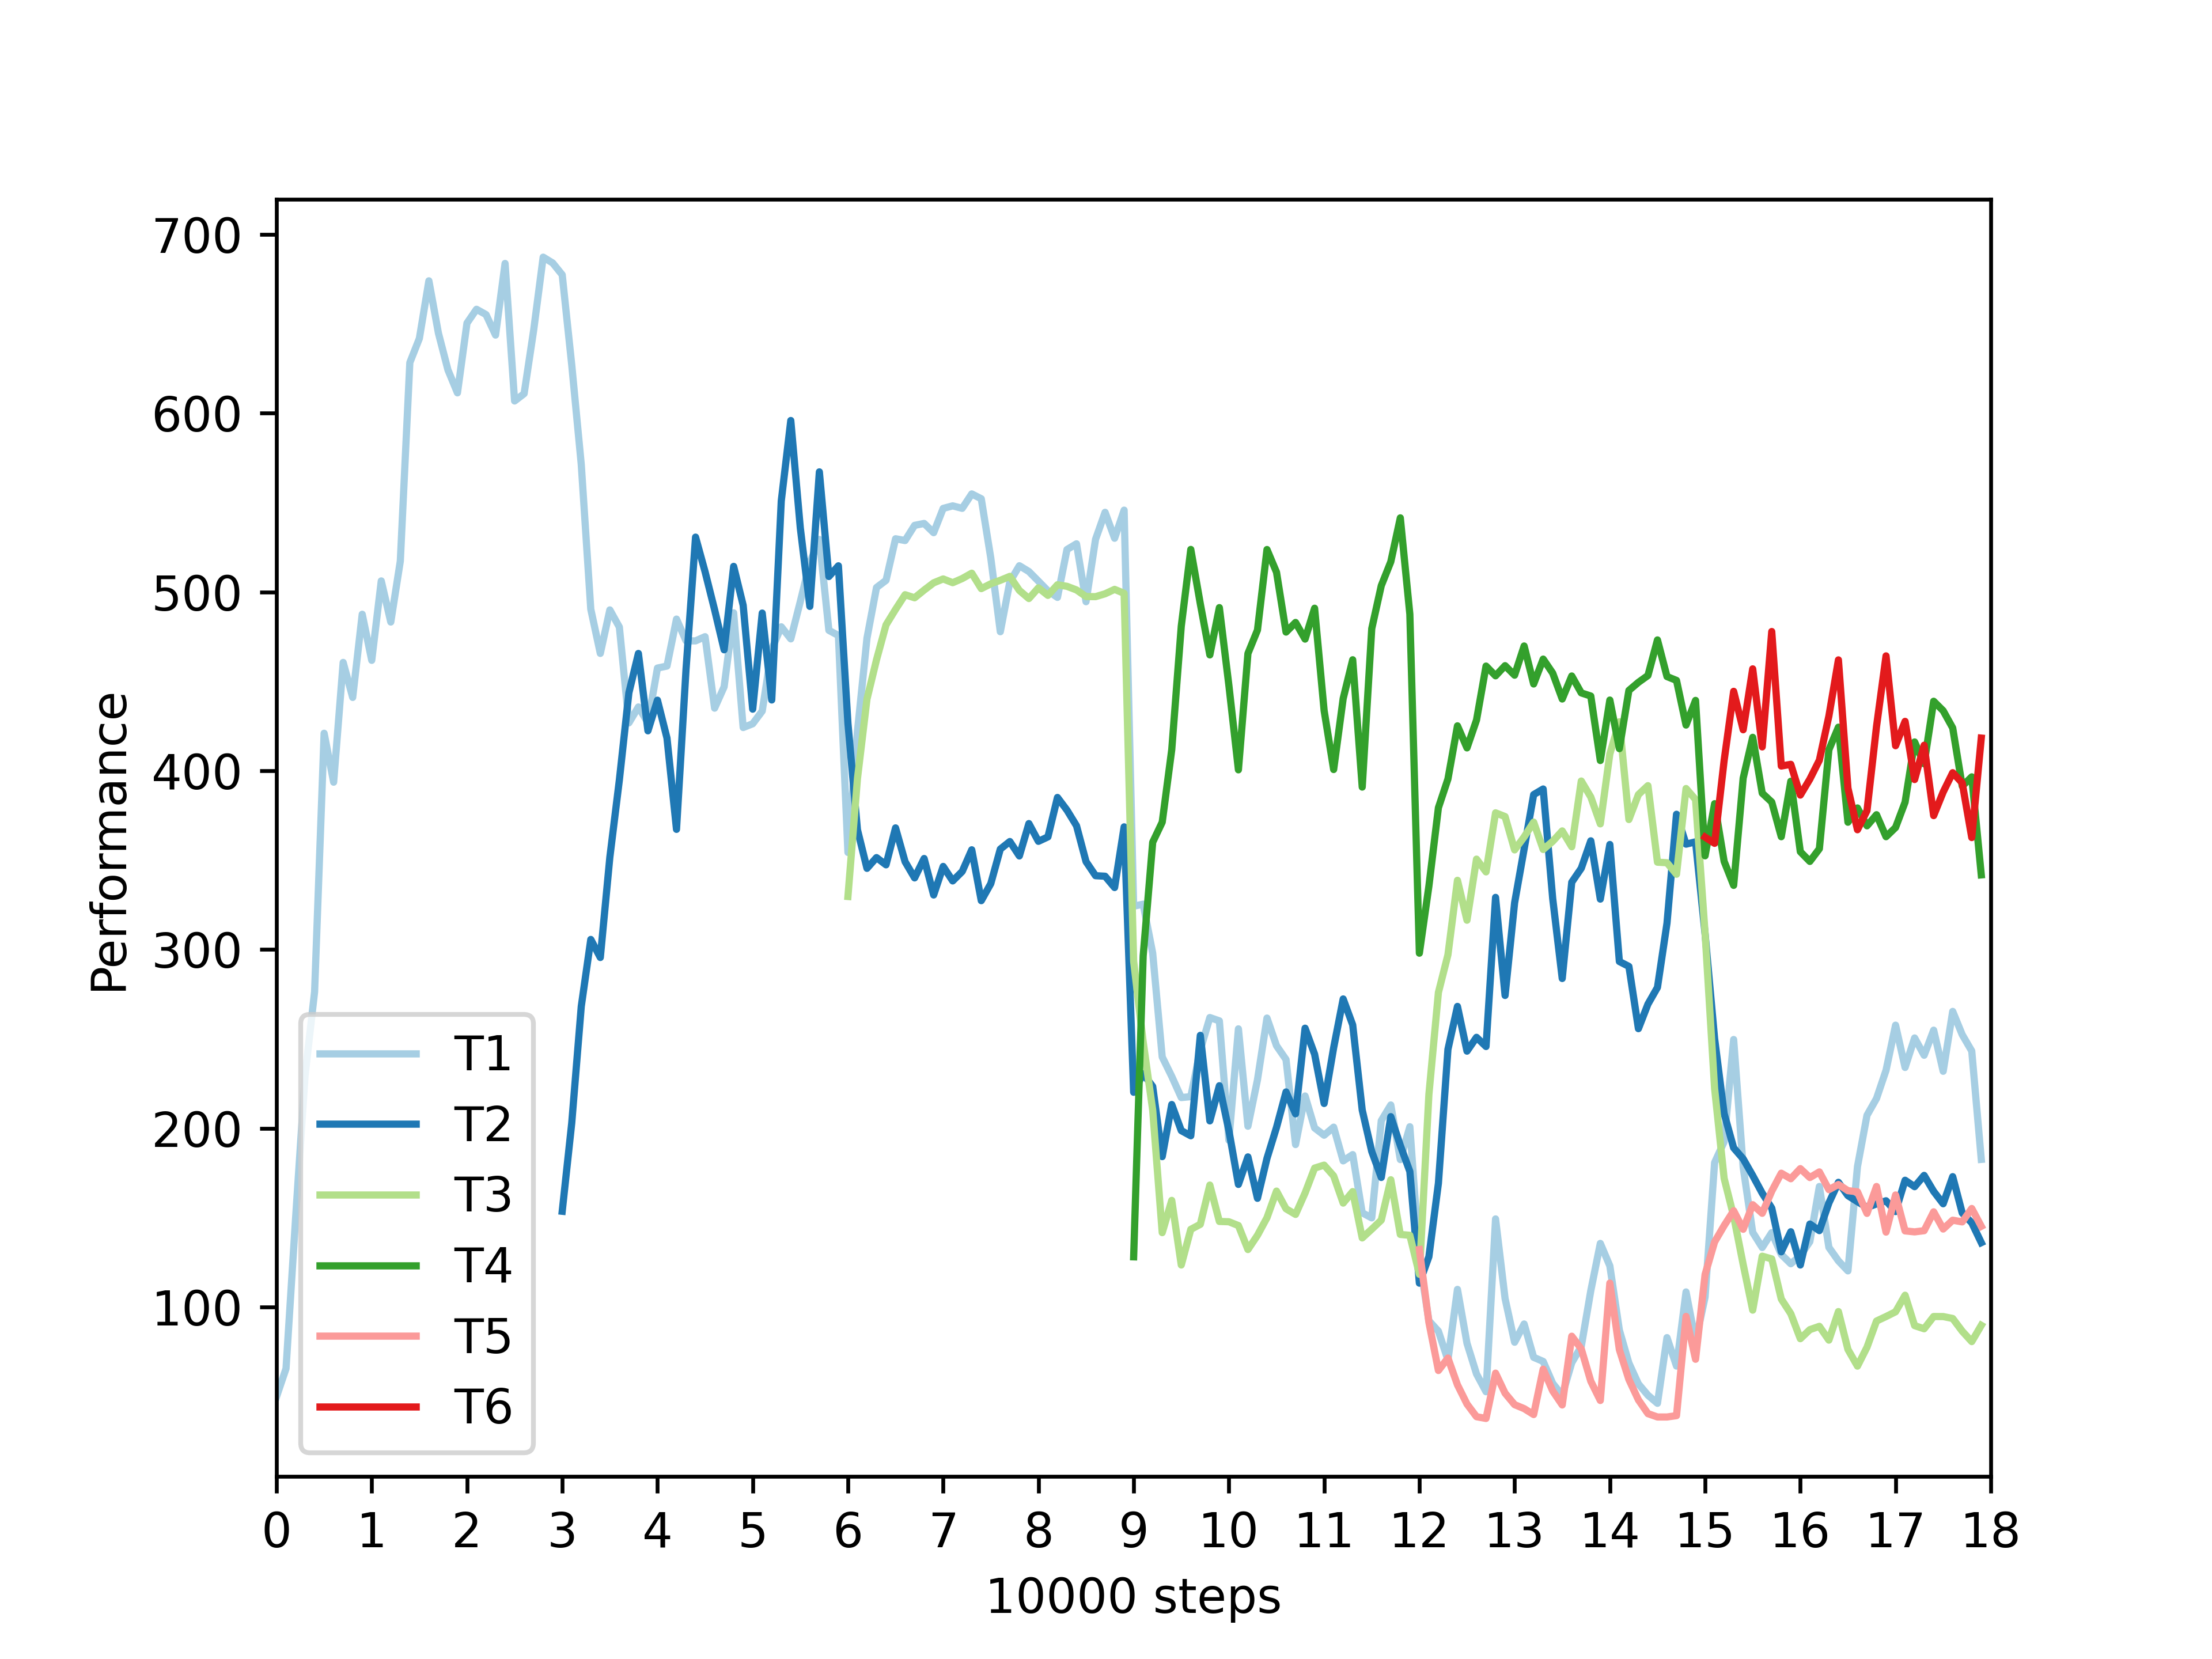}}
    \subcaptionbox{DT + GEM}
    {\includegraphics[width=0.245\linewidth]{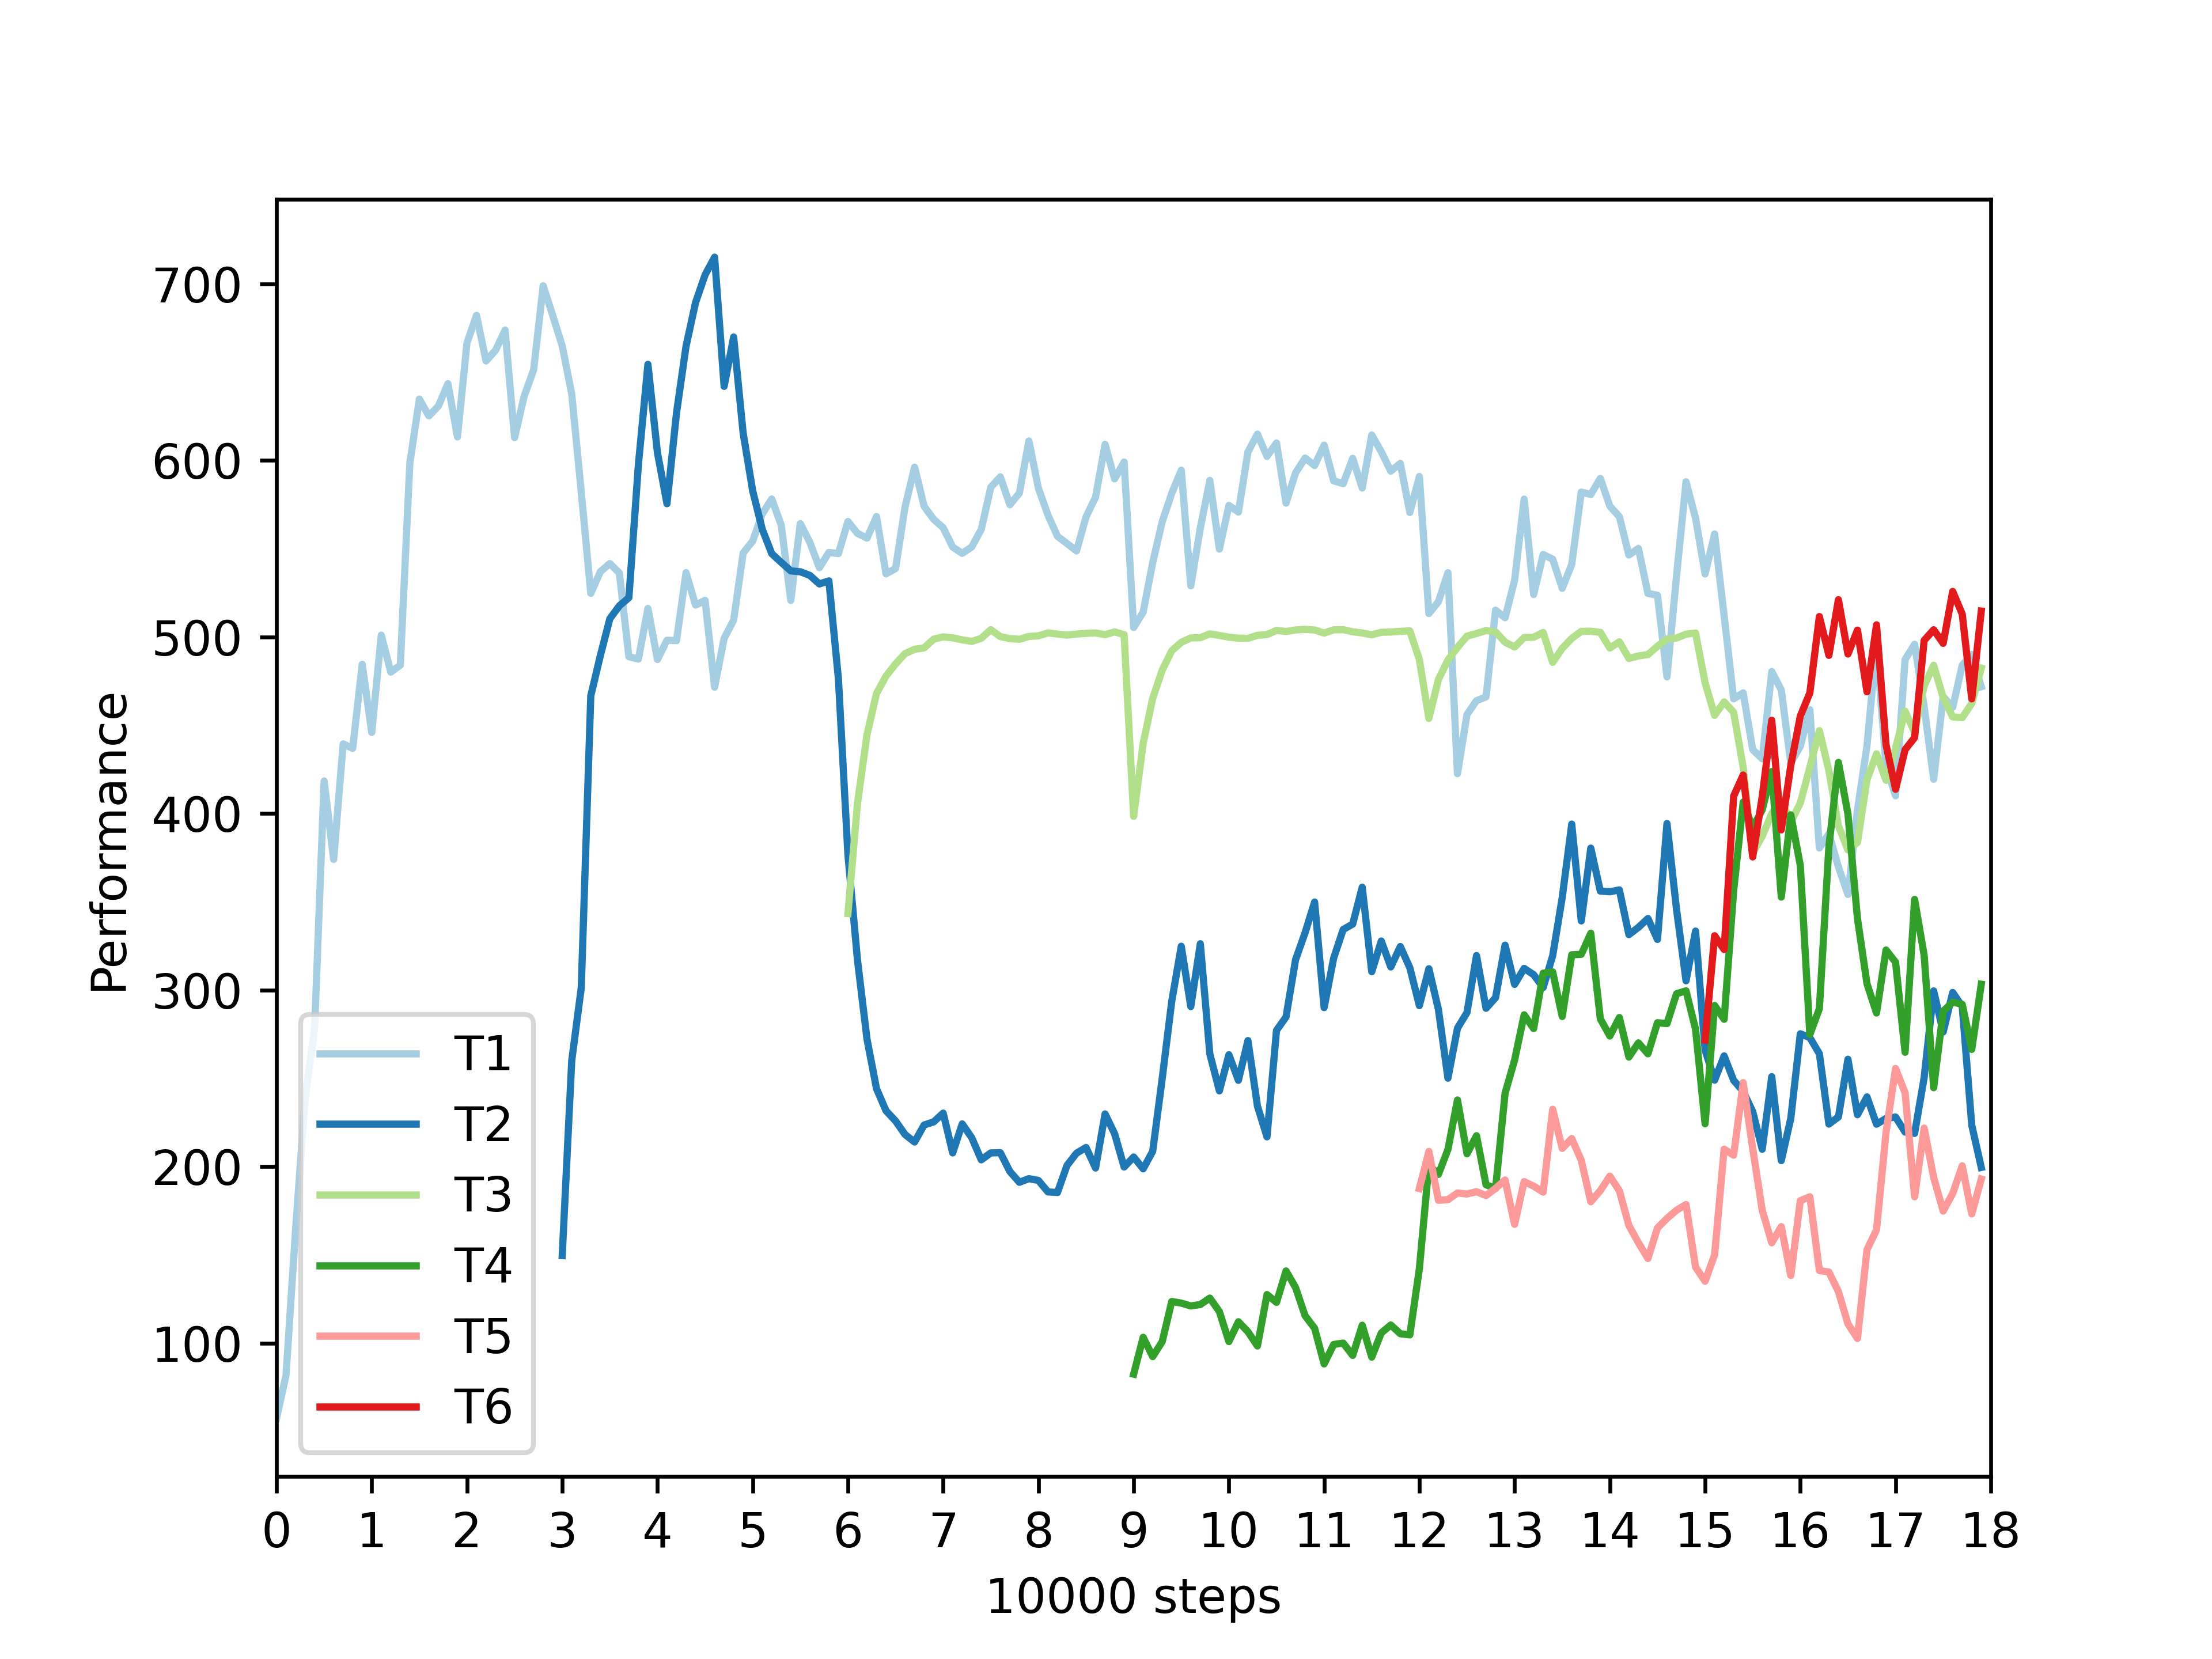}}
     \centering	
     \subcaptionbox{Vanilla DT}
    {\includegraphics[width=0.245\linewidth]{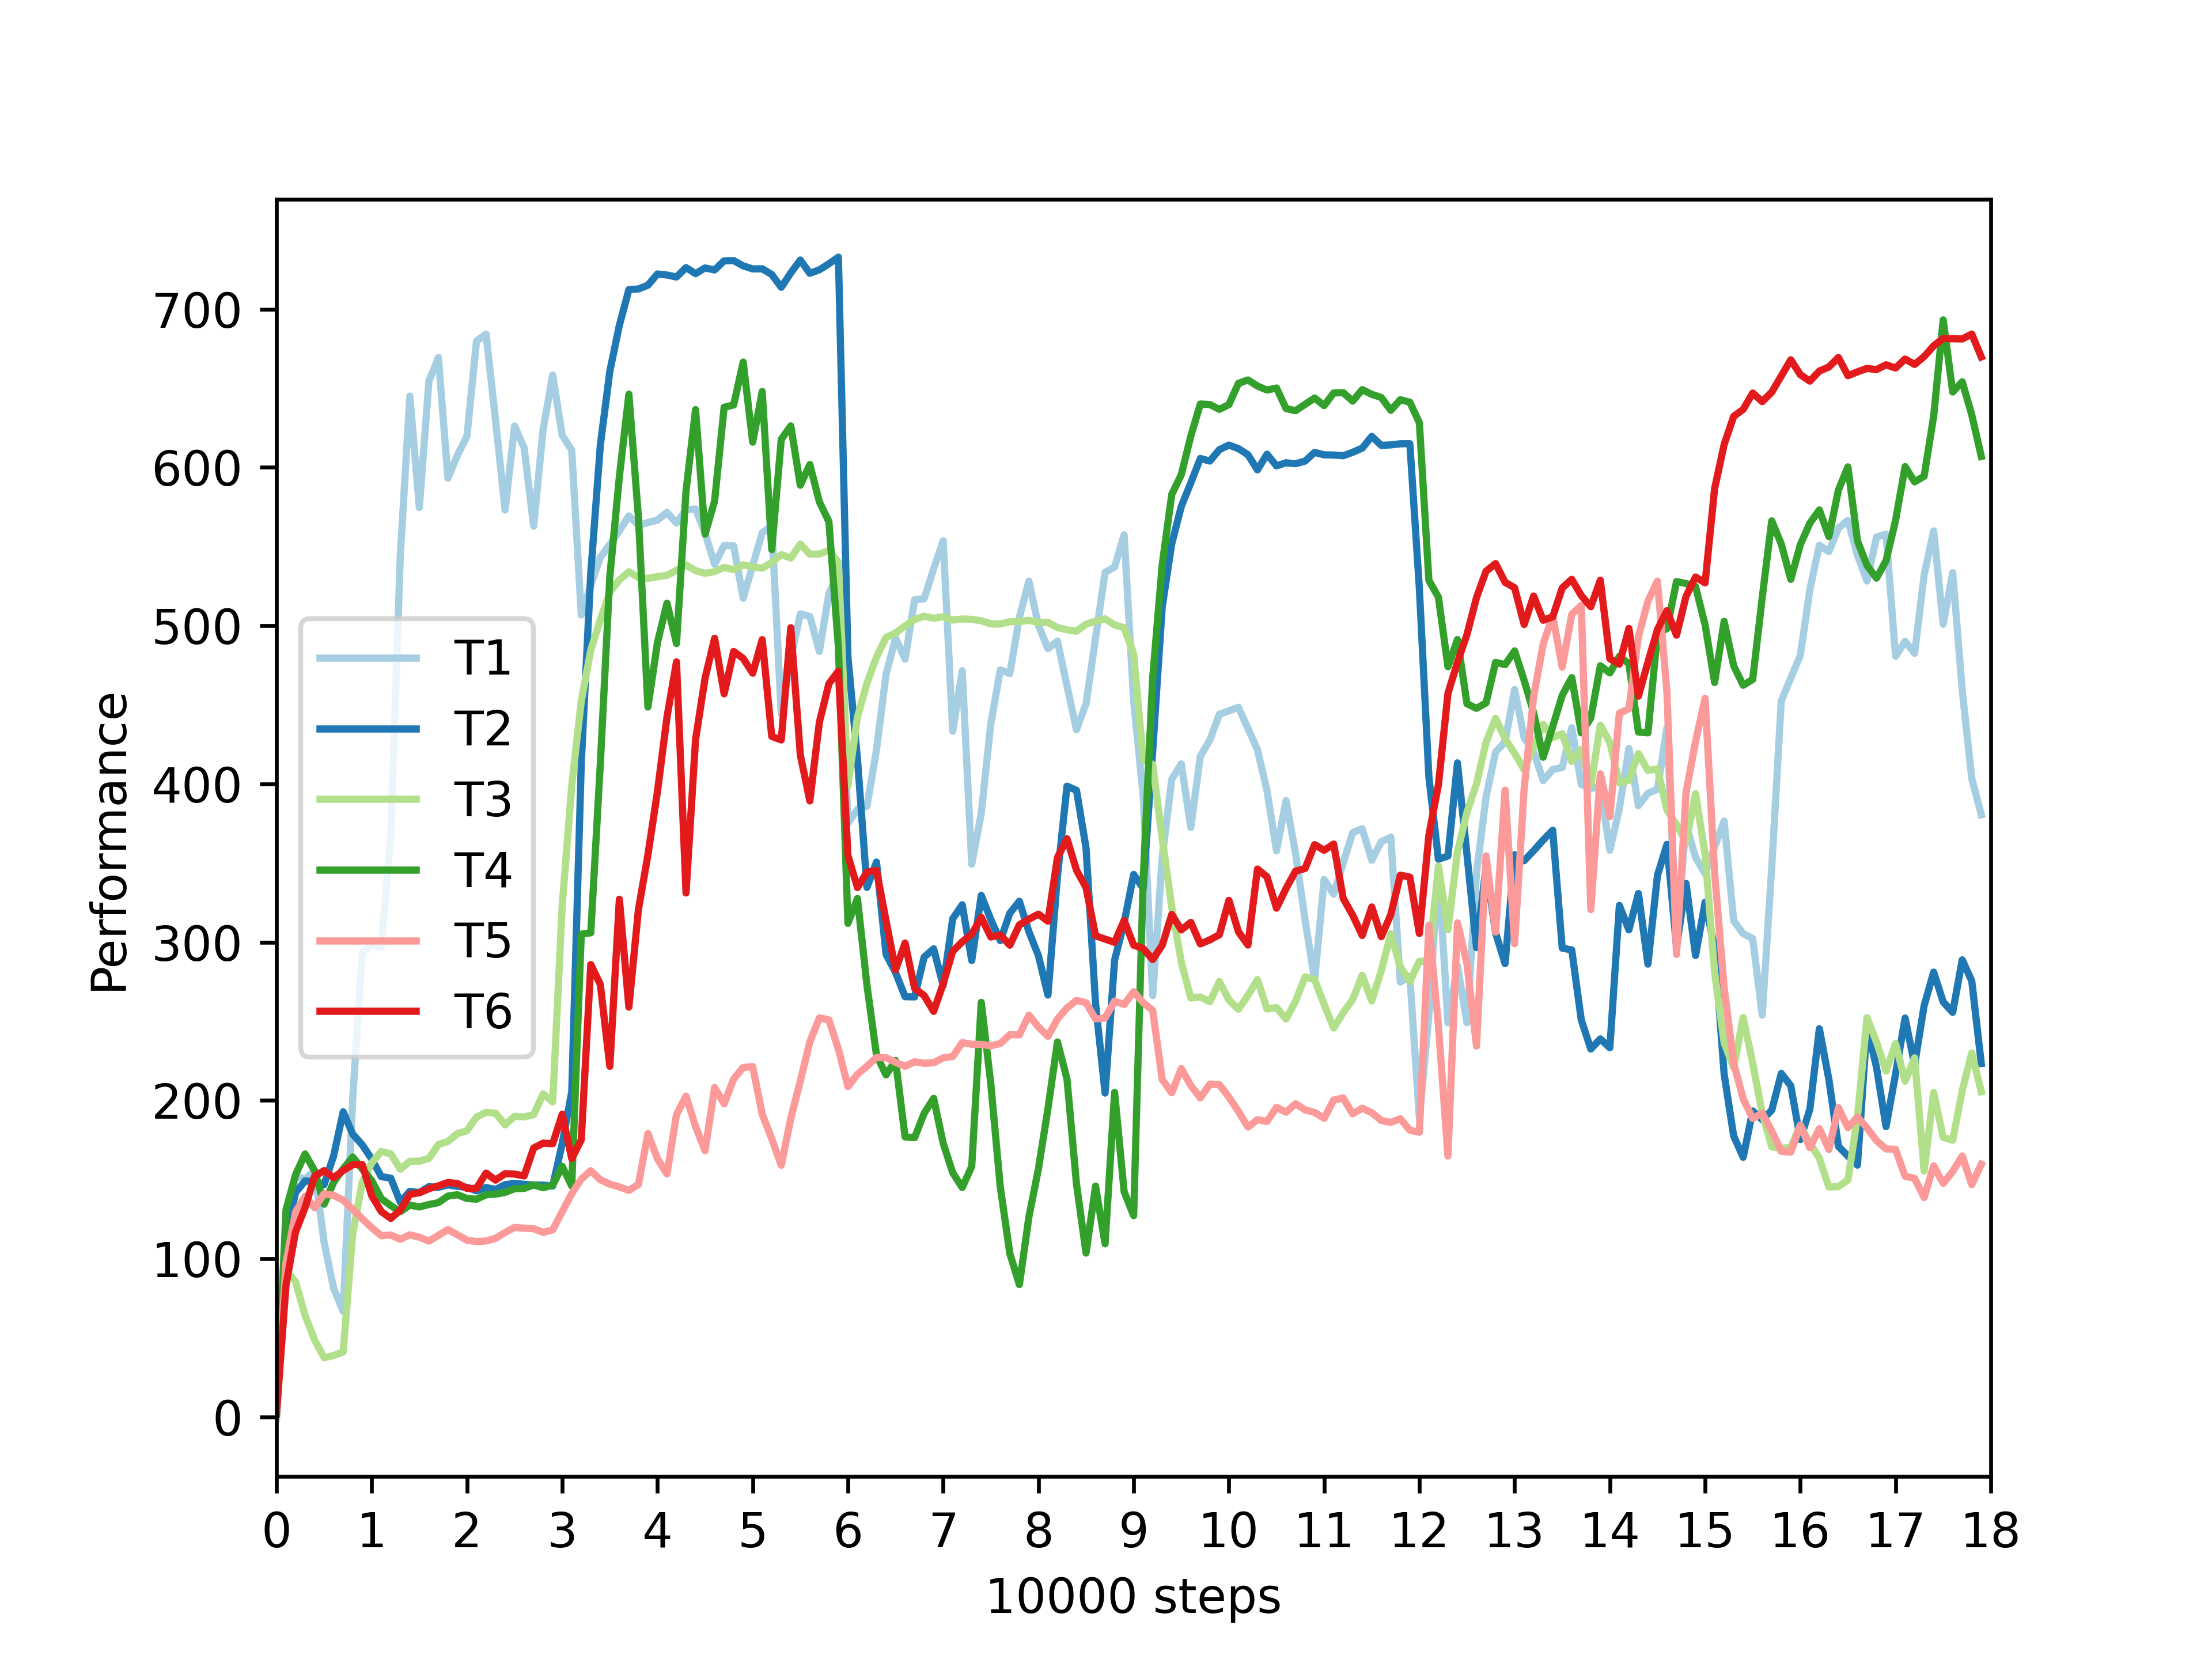}}
        \subcaptionbox{OER}
    {\includegraphics[width=0.245\linewidth]{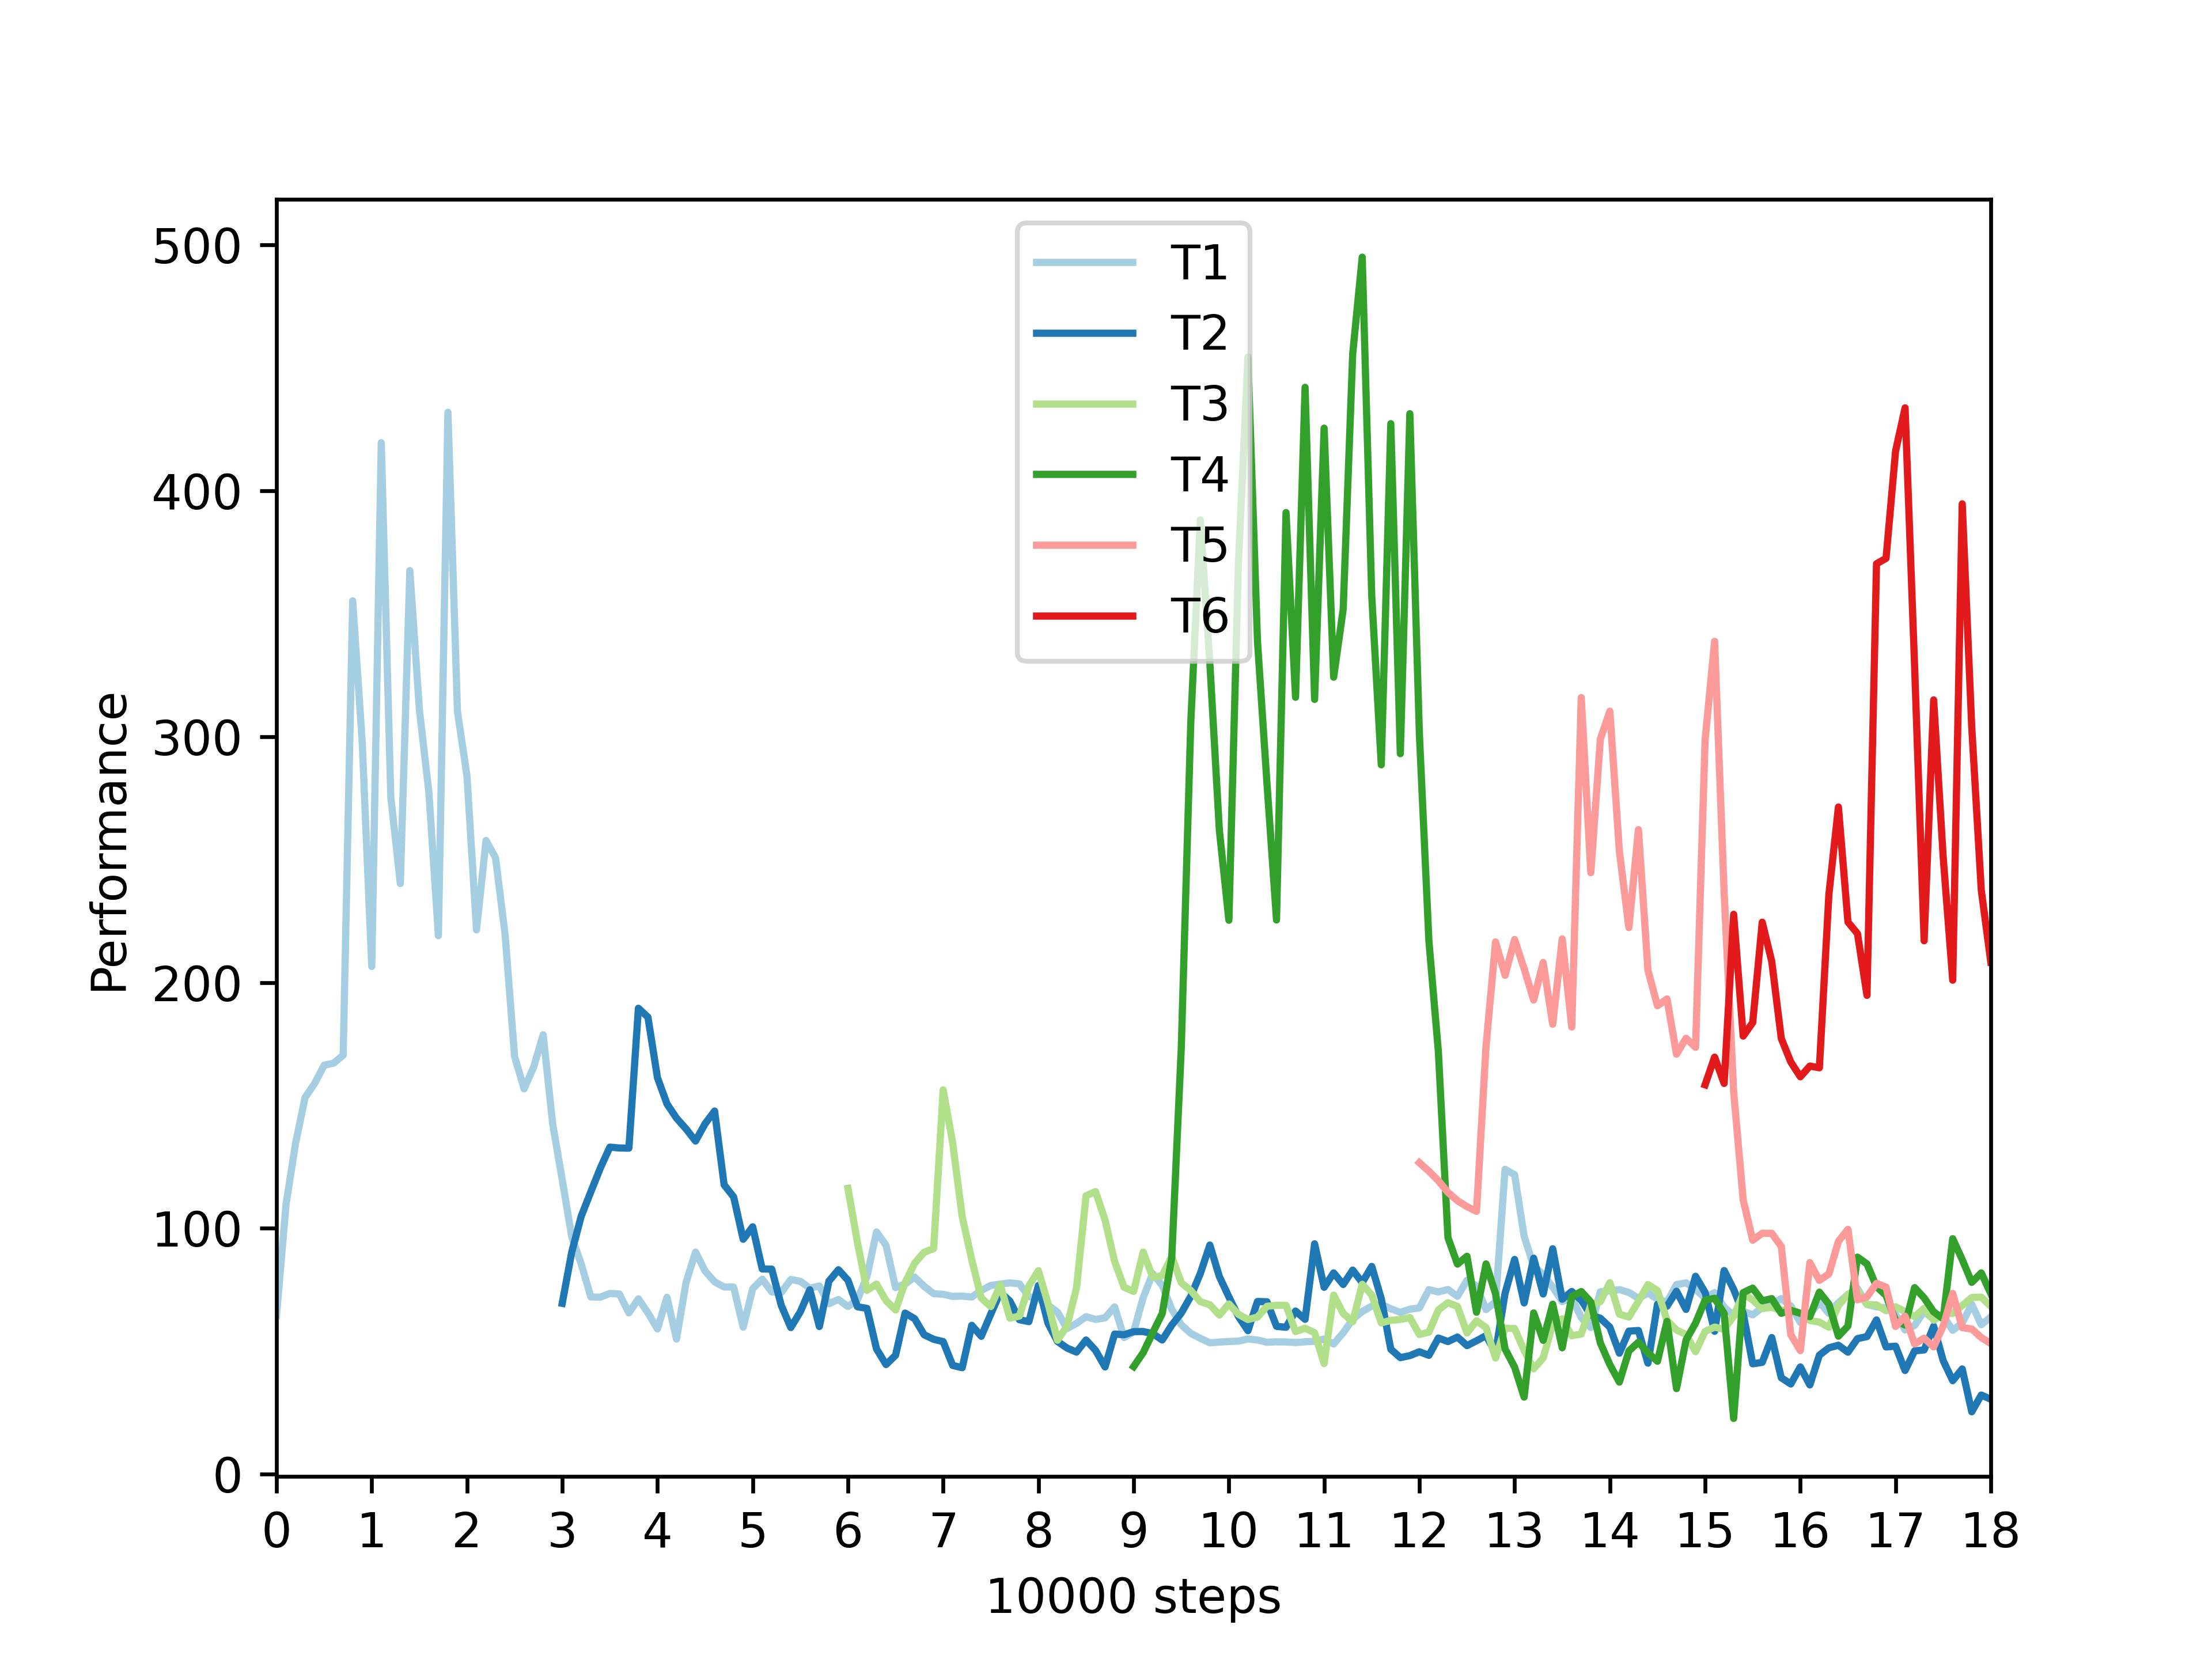}}
     \subcaptionbox{MH-DT}
    {\includegraphics[width=0.245\linewidth]{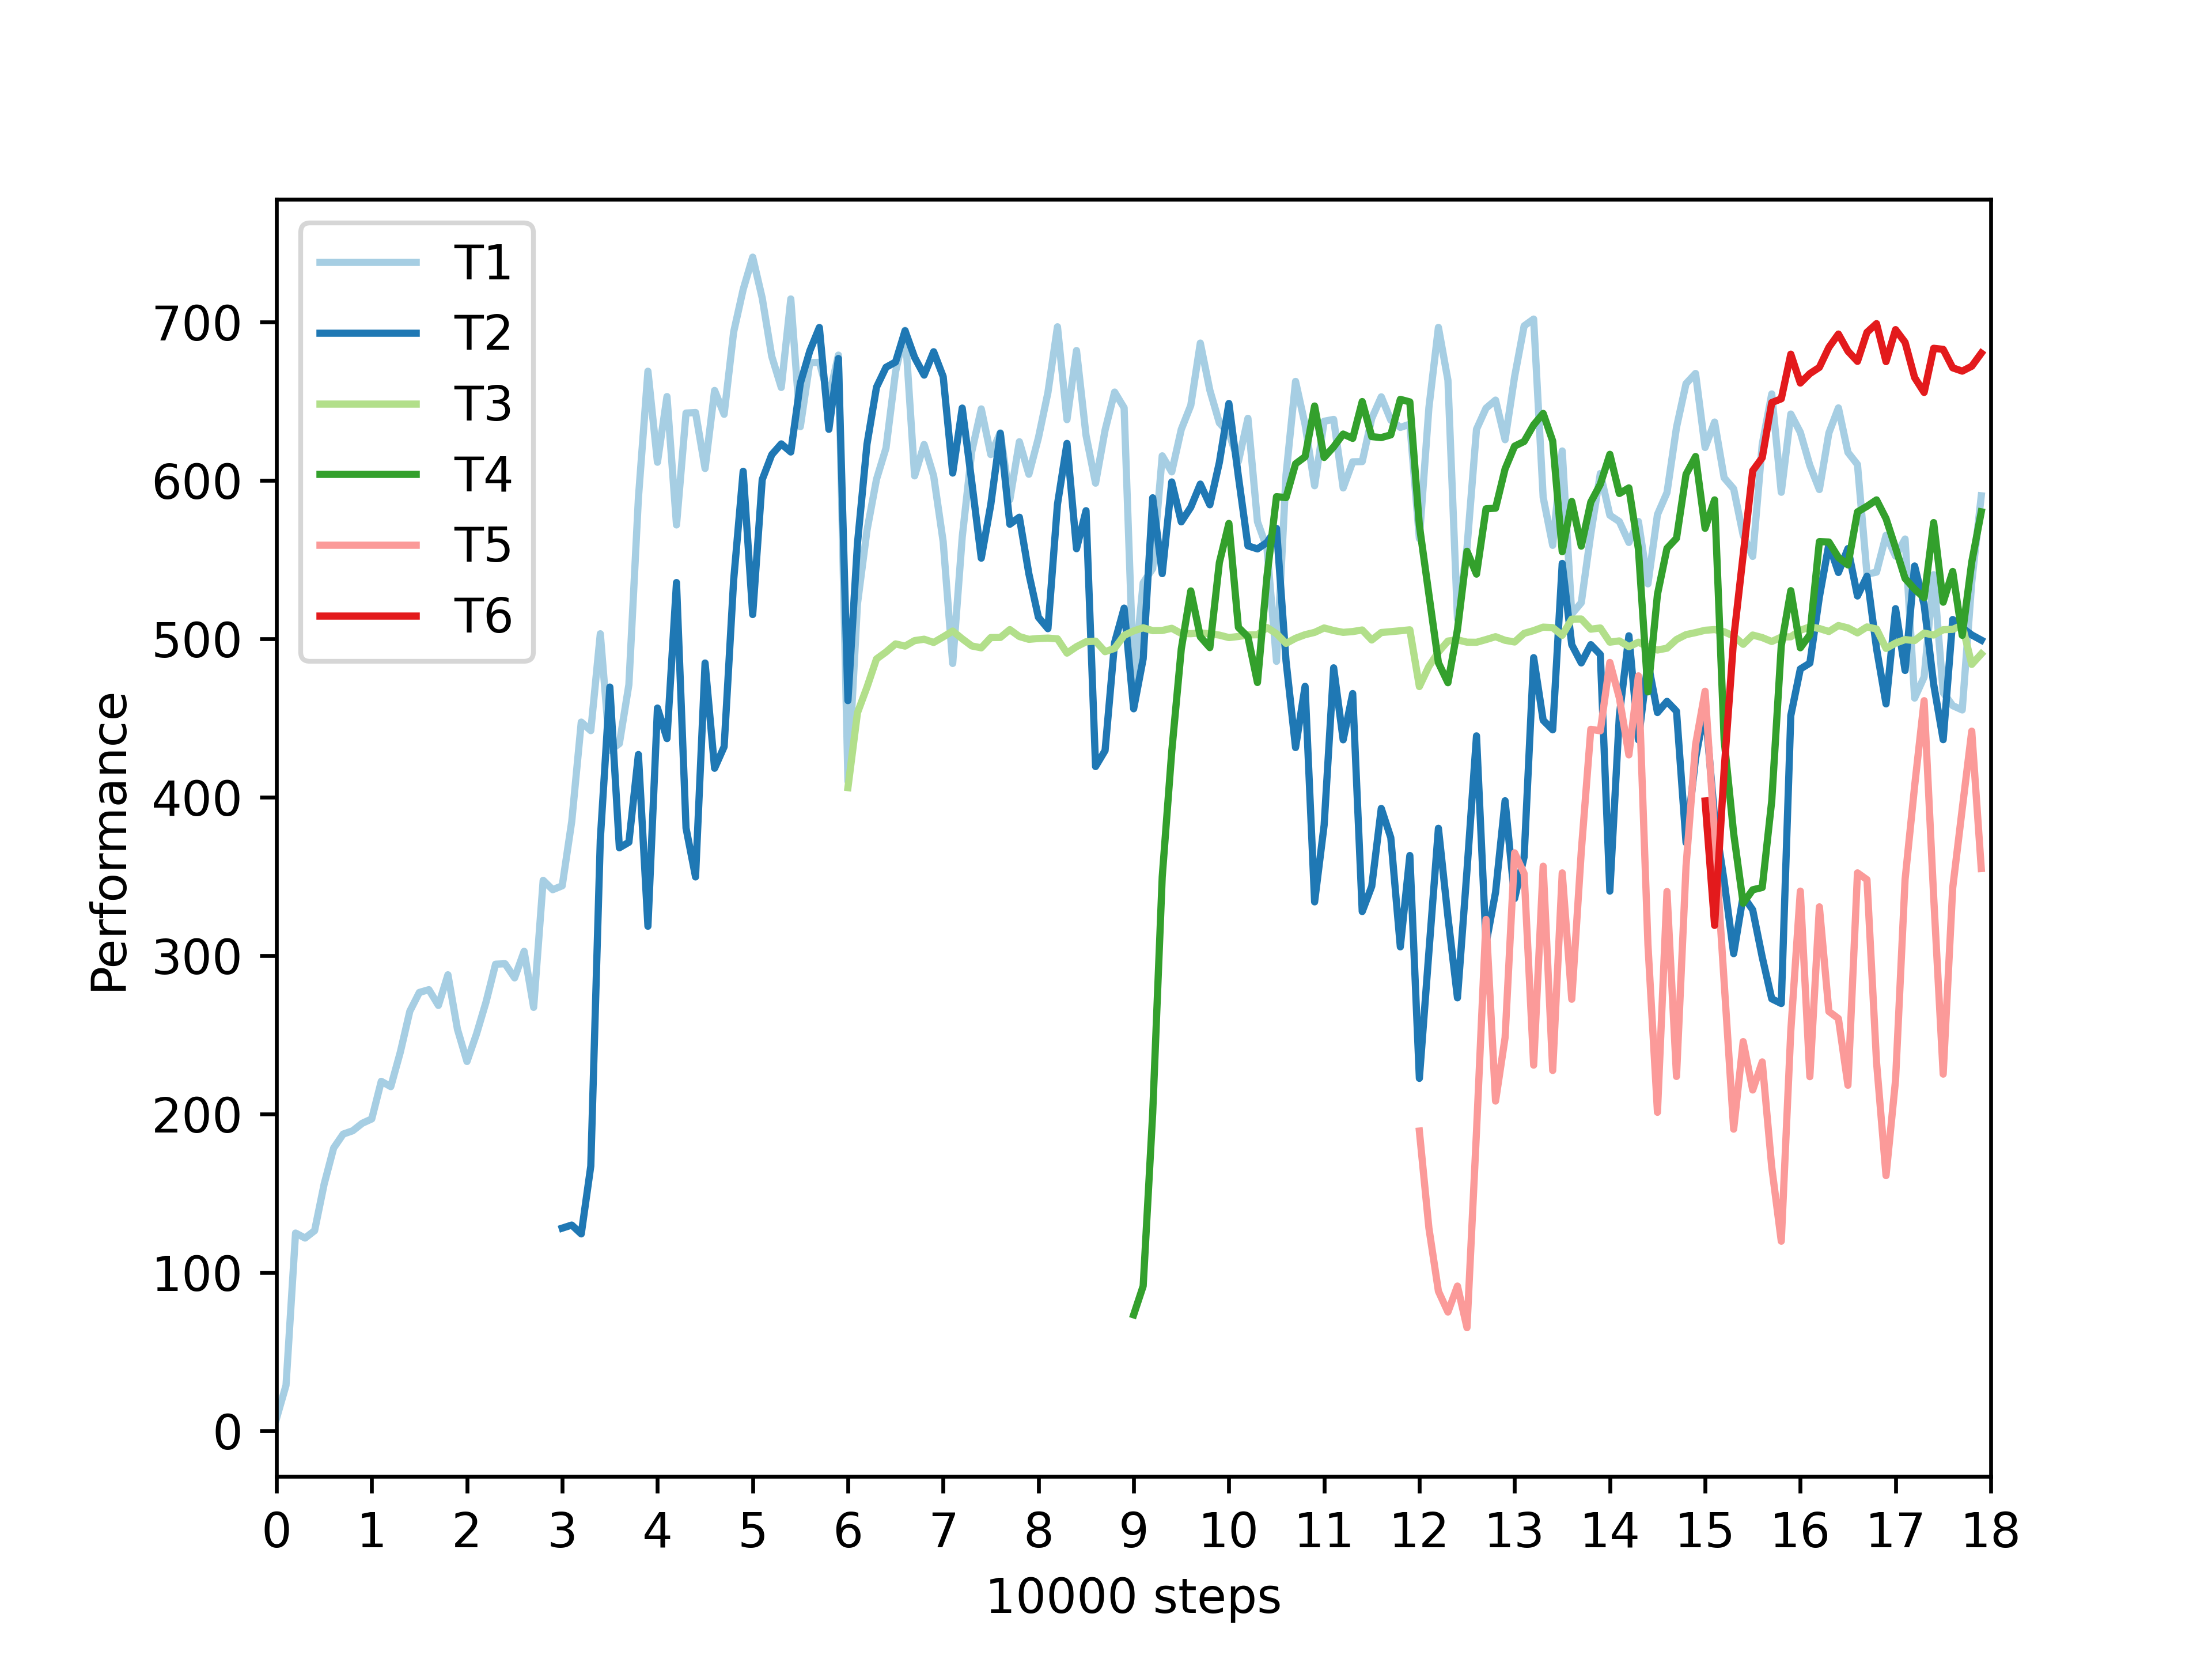}}
	\subcaptionbox{LoRA-DT}
    {\includegraphics[width=0.245\linewidth]{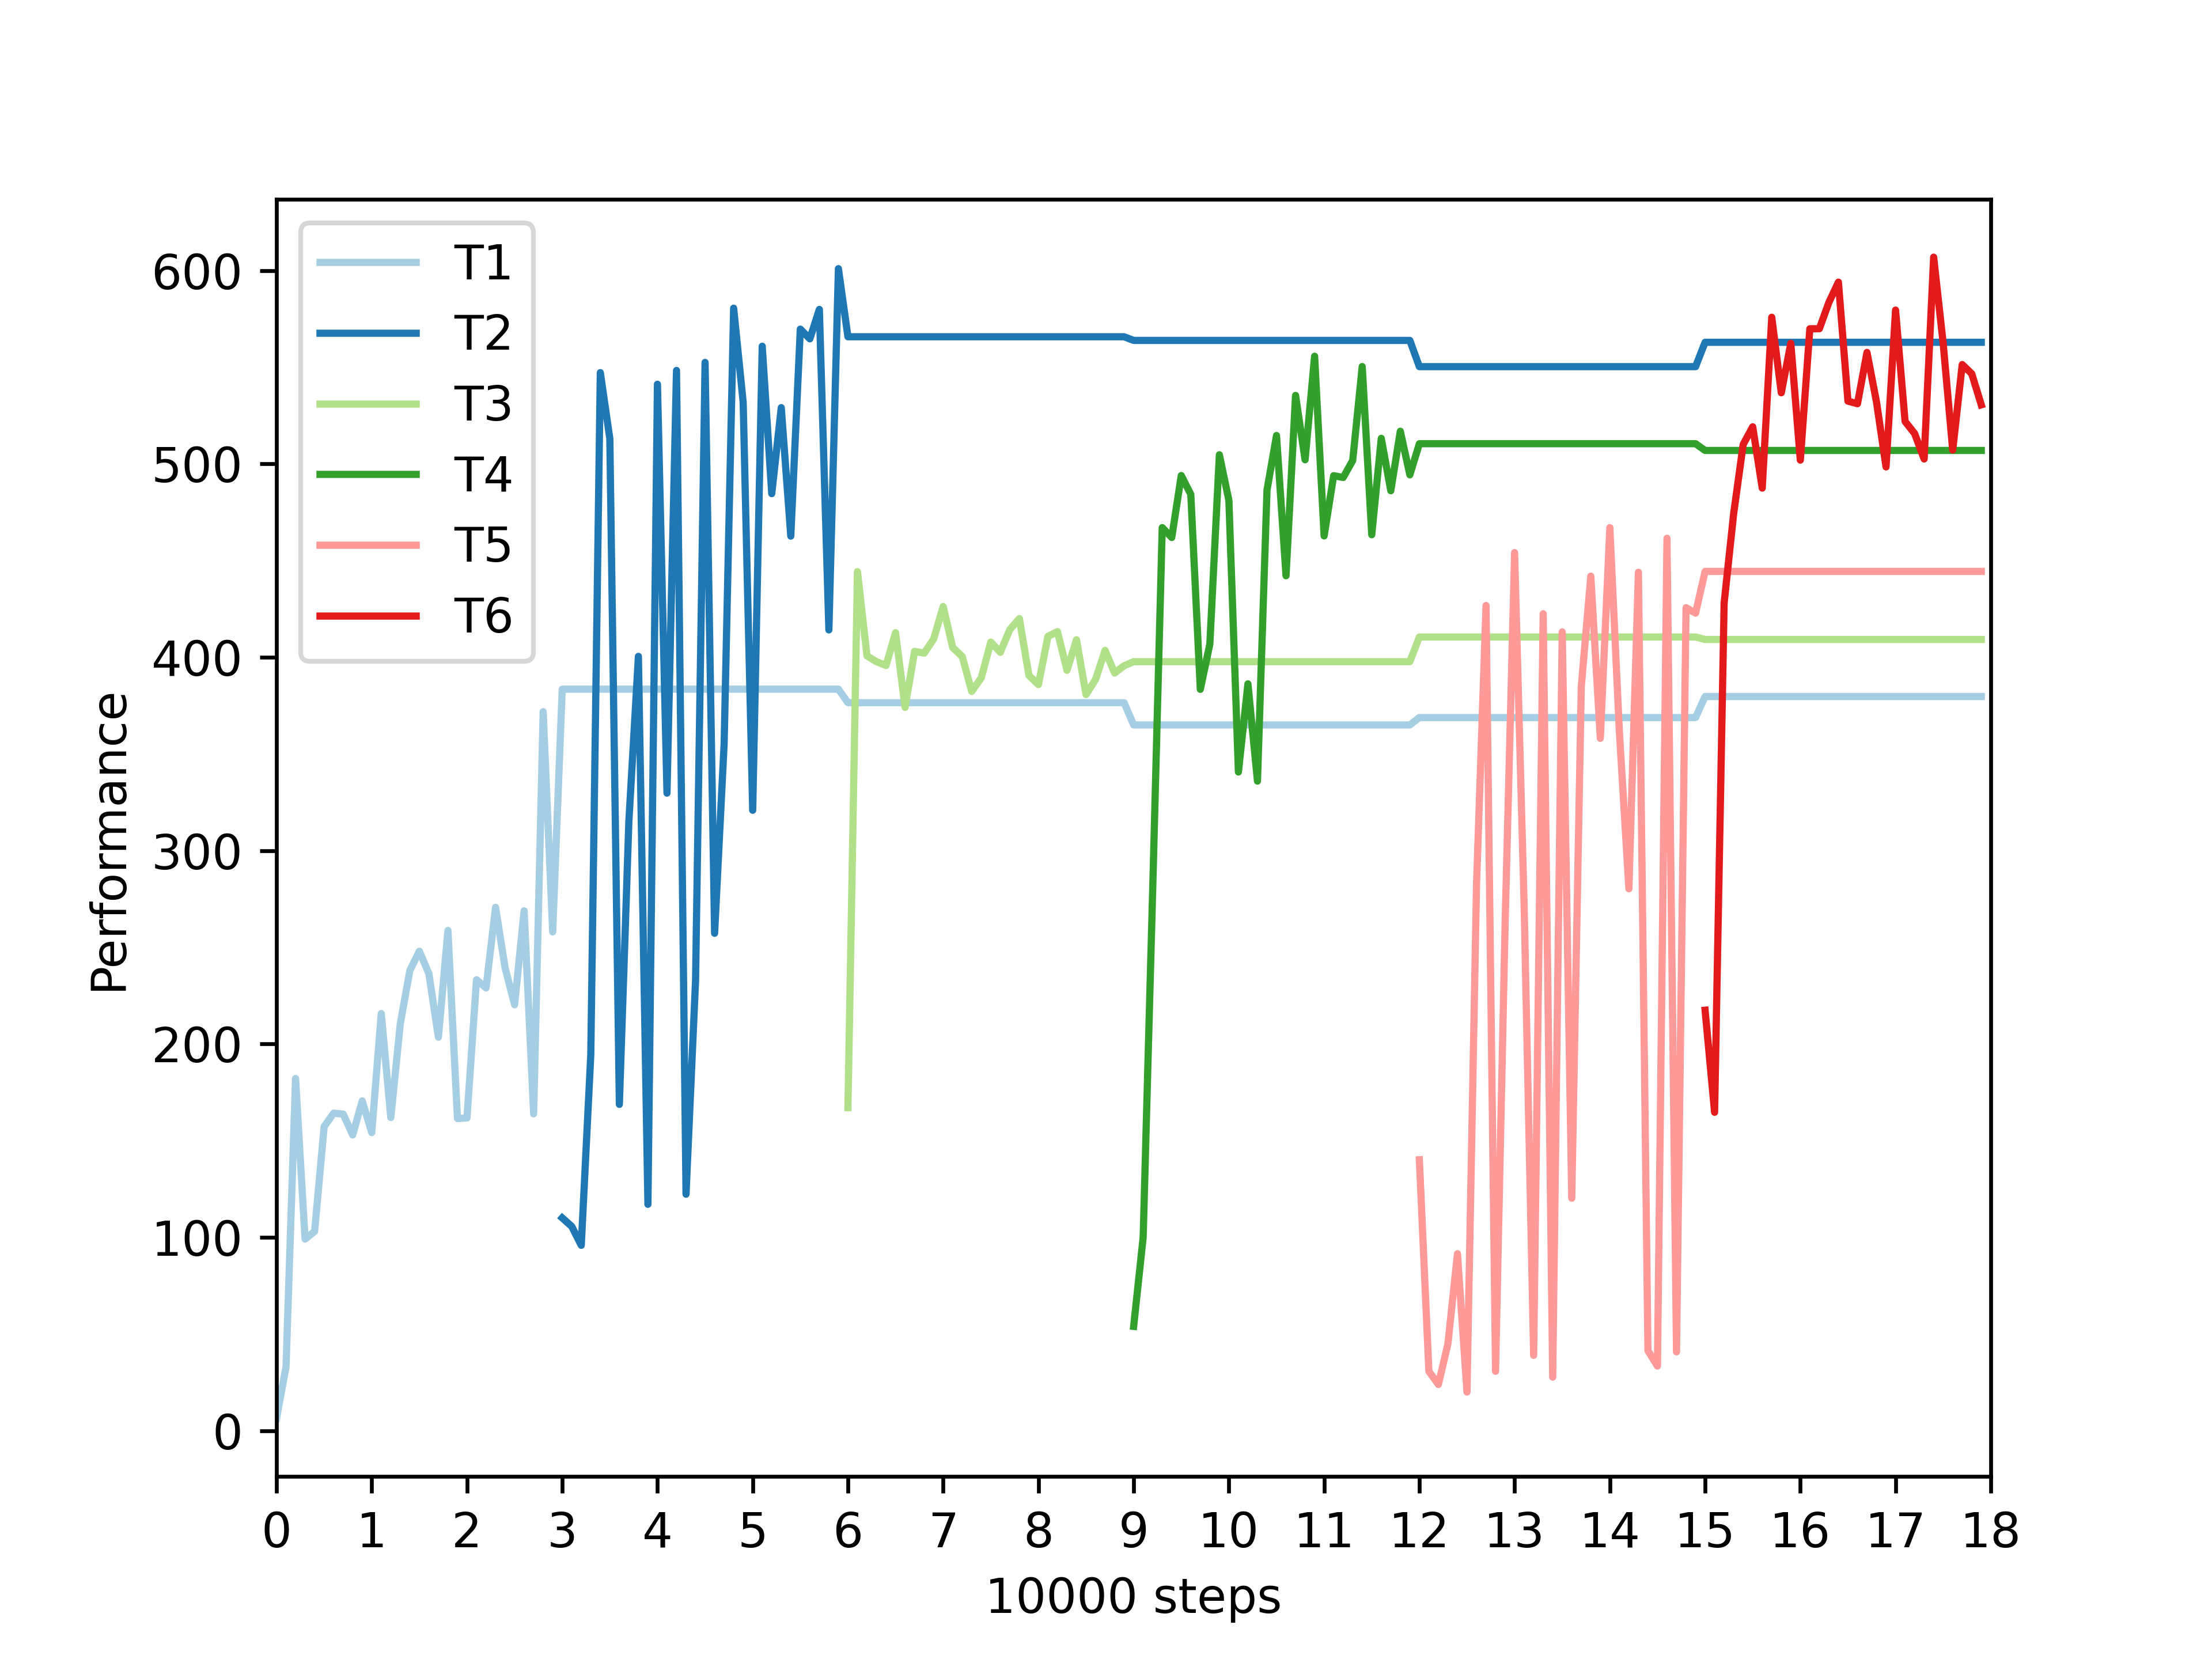}}
    \caption{Walker\_Param (expert)}
\end{figure}

\begin{figure}[htbp]
	\centering
	\subcaptionbox{PDT}
    {\includegraphics[width=0.245\linewidth]{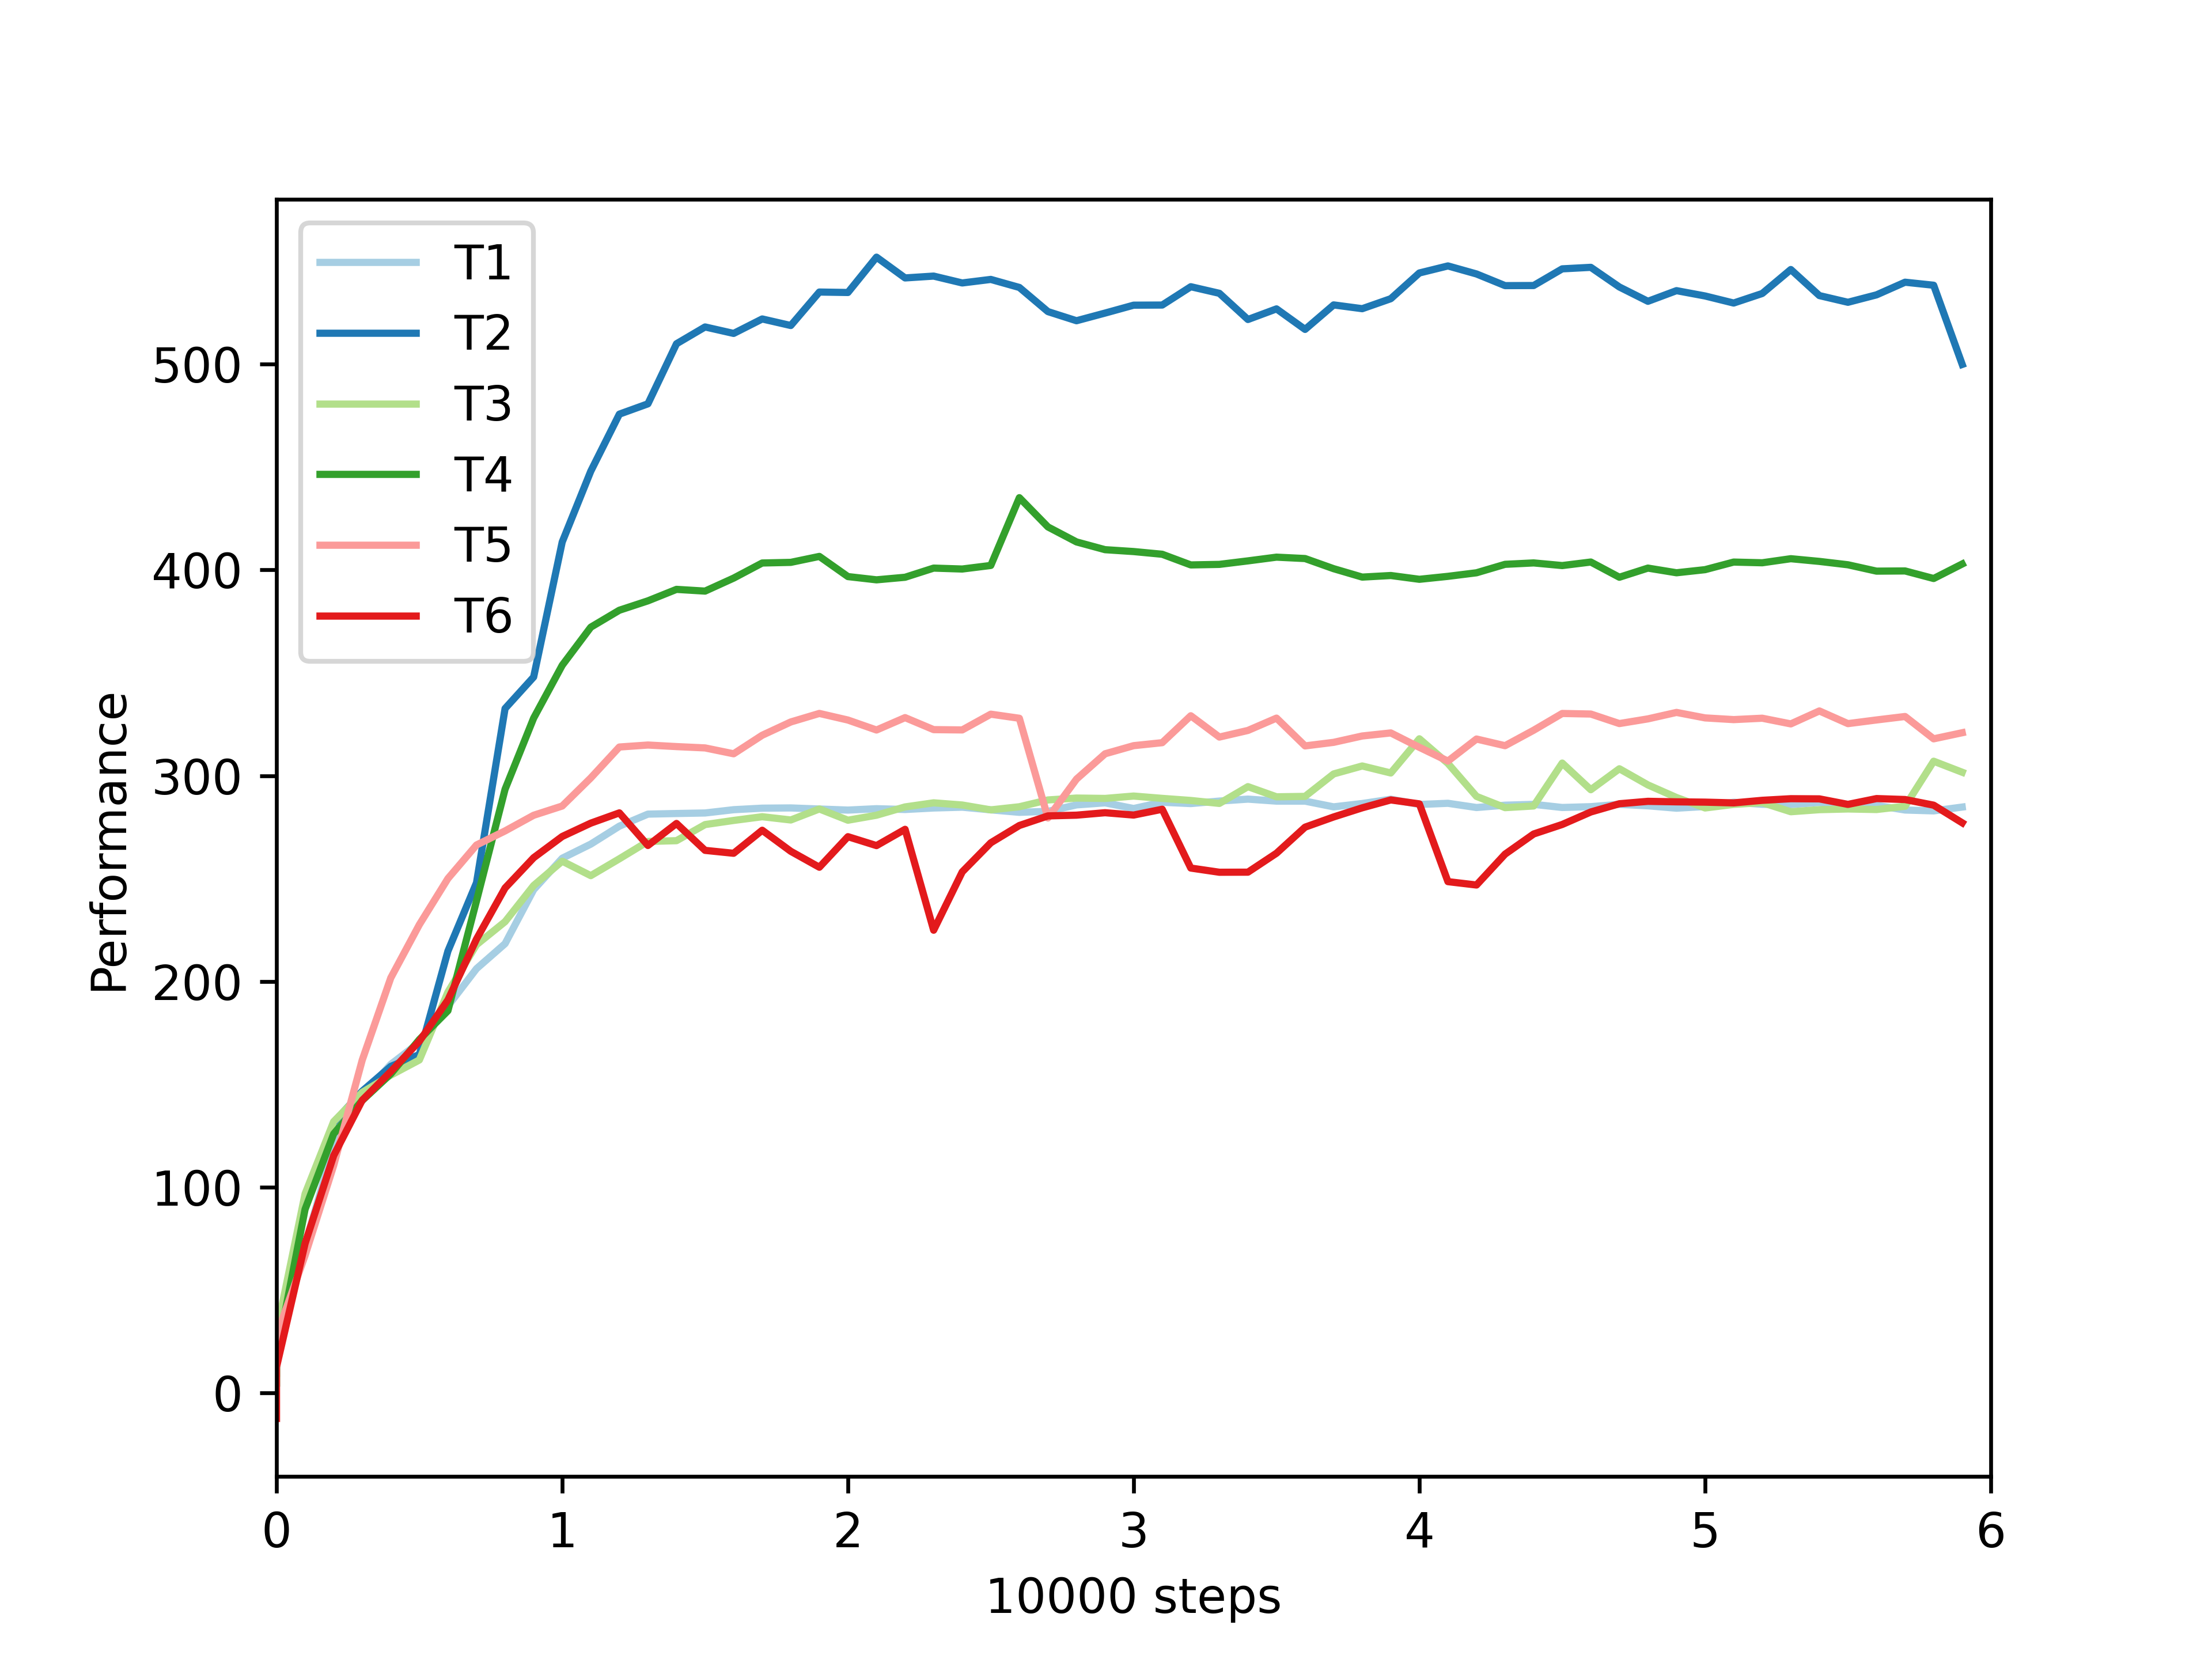}}
	\subcaptionbox{DT + EWC}
    {\includegraphics[width=0.245\linewidth]{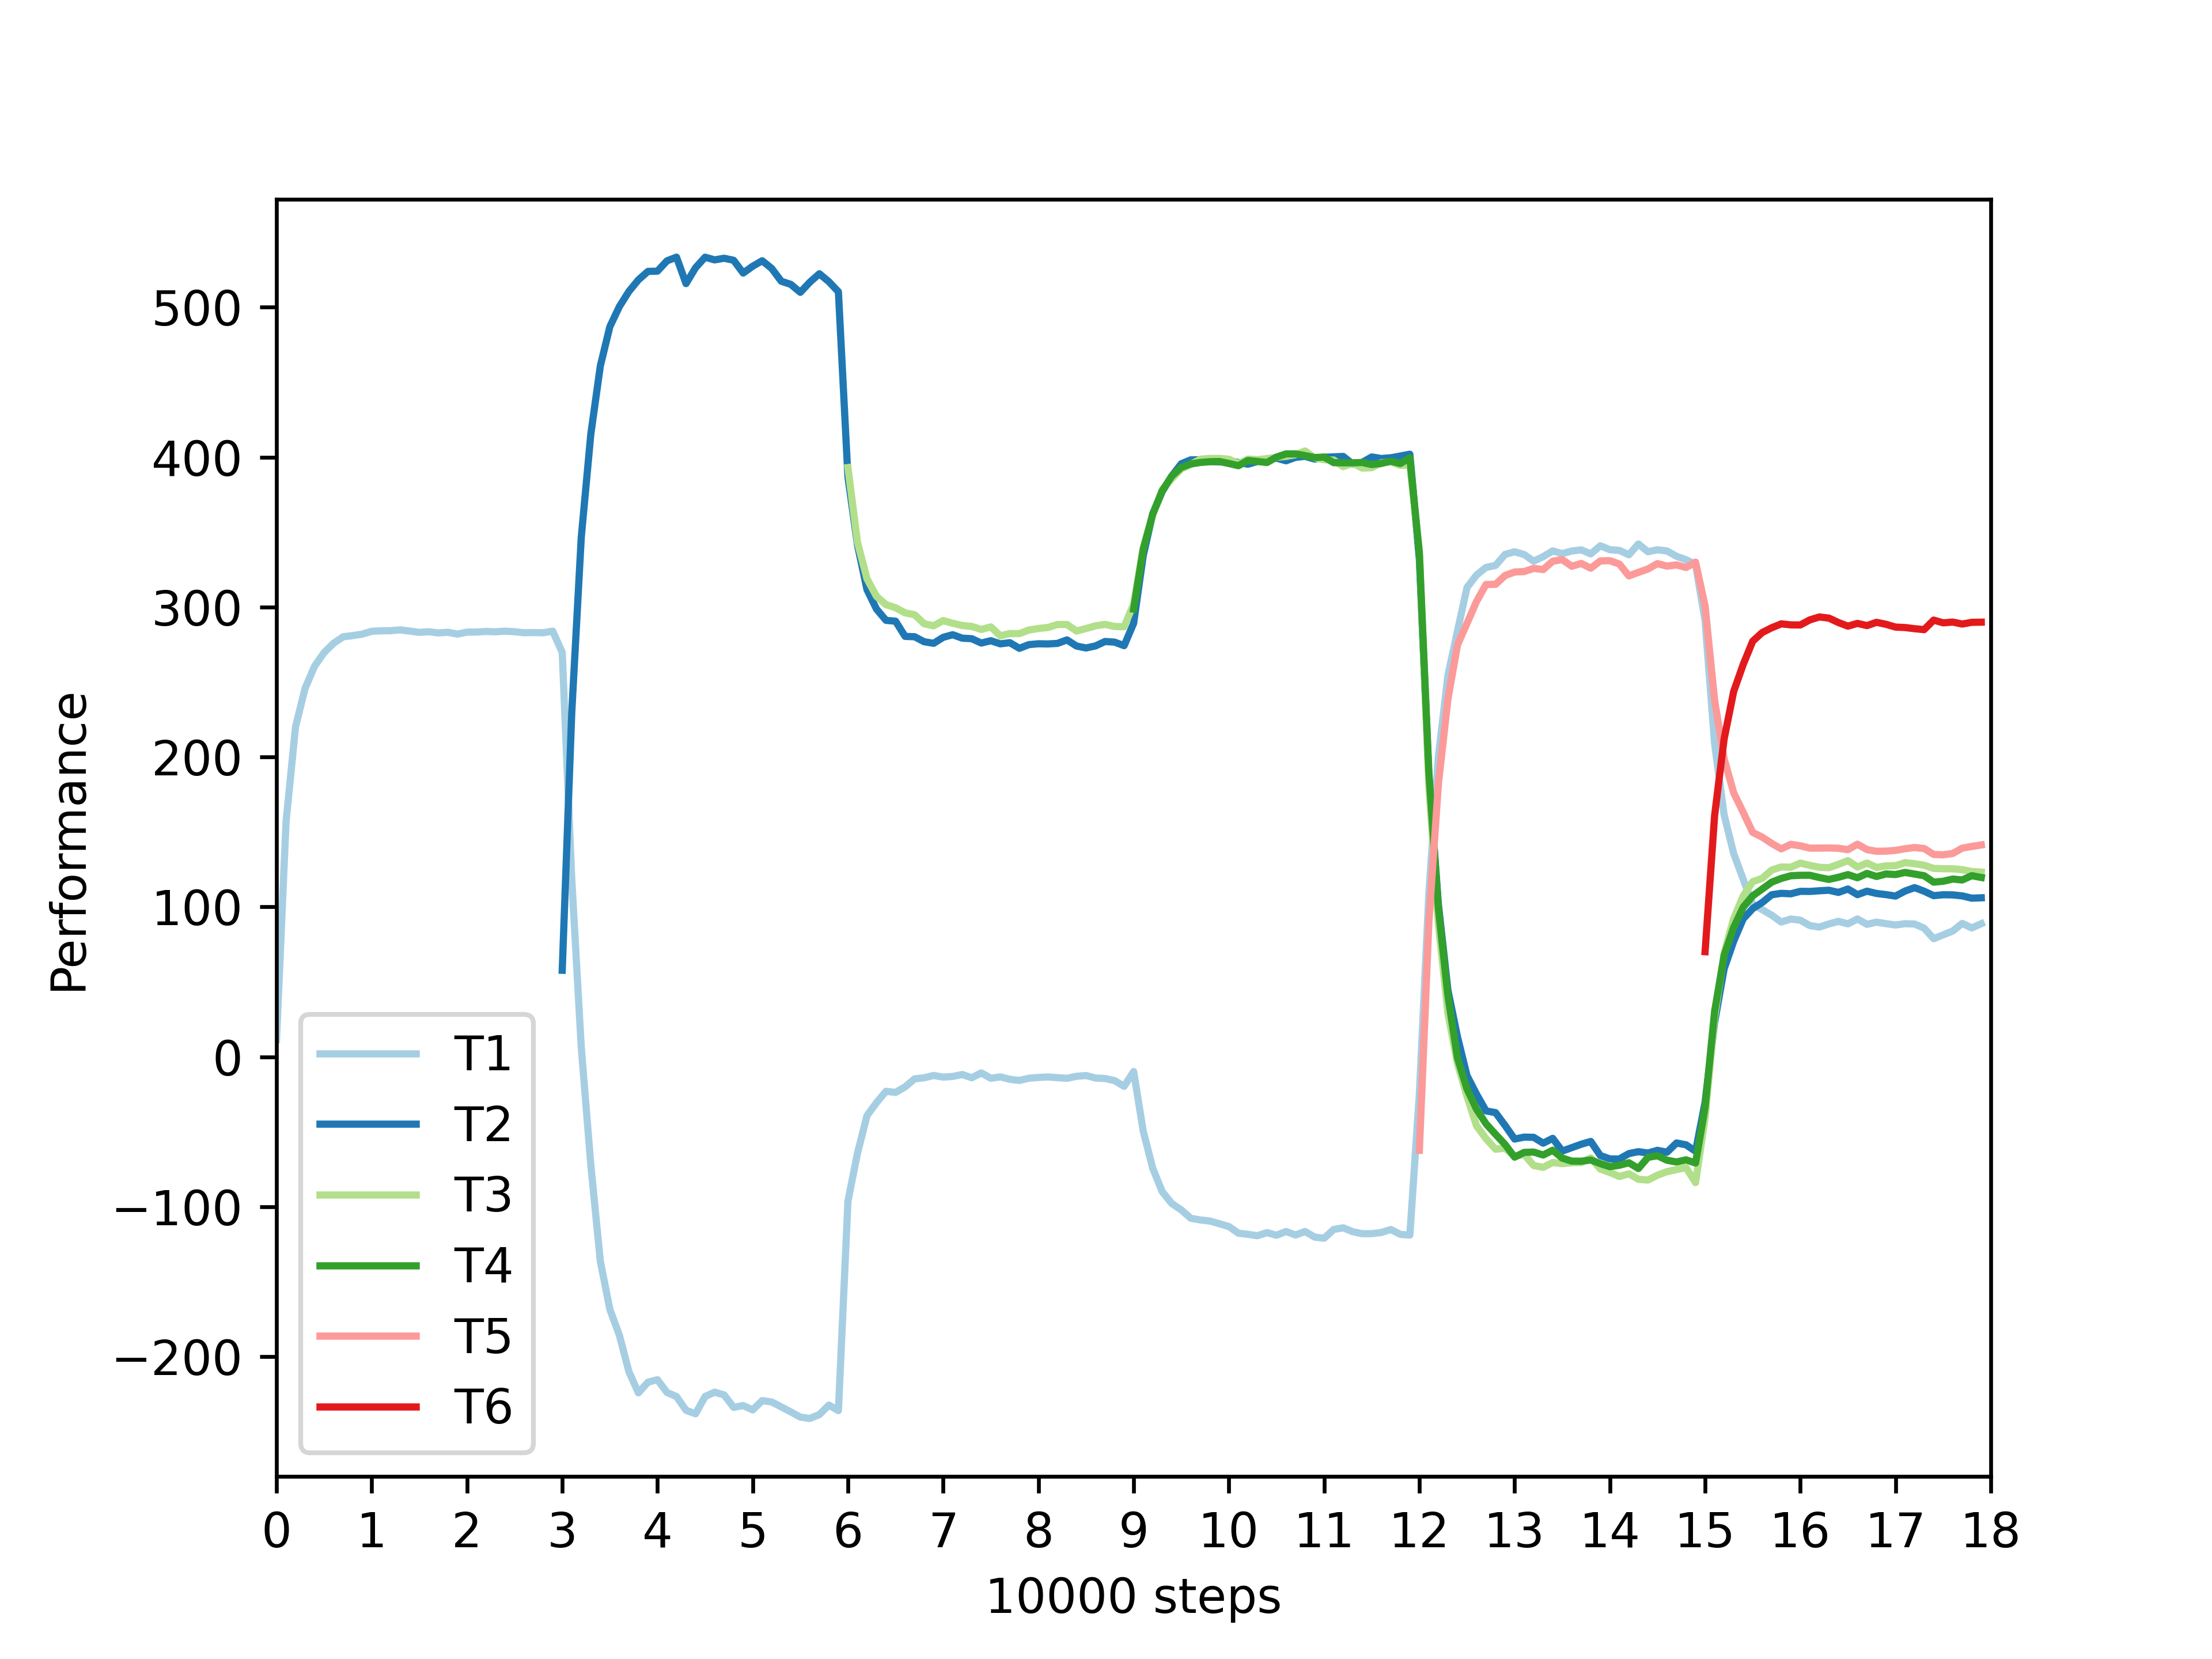}}
    \subcaptionbox{DT + SI}
    {\includegraphics[width=0.245\linewidth]{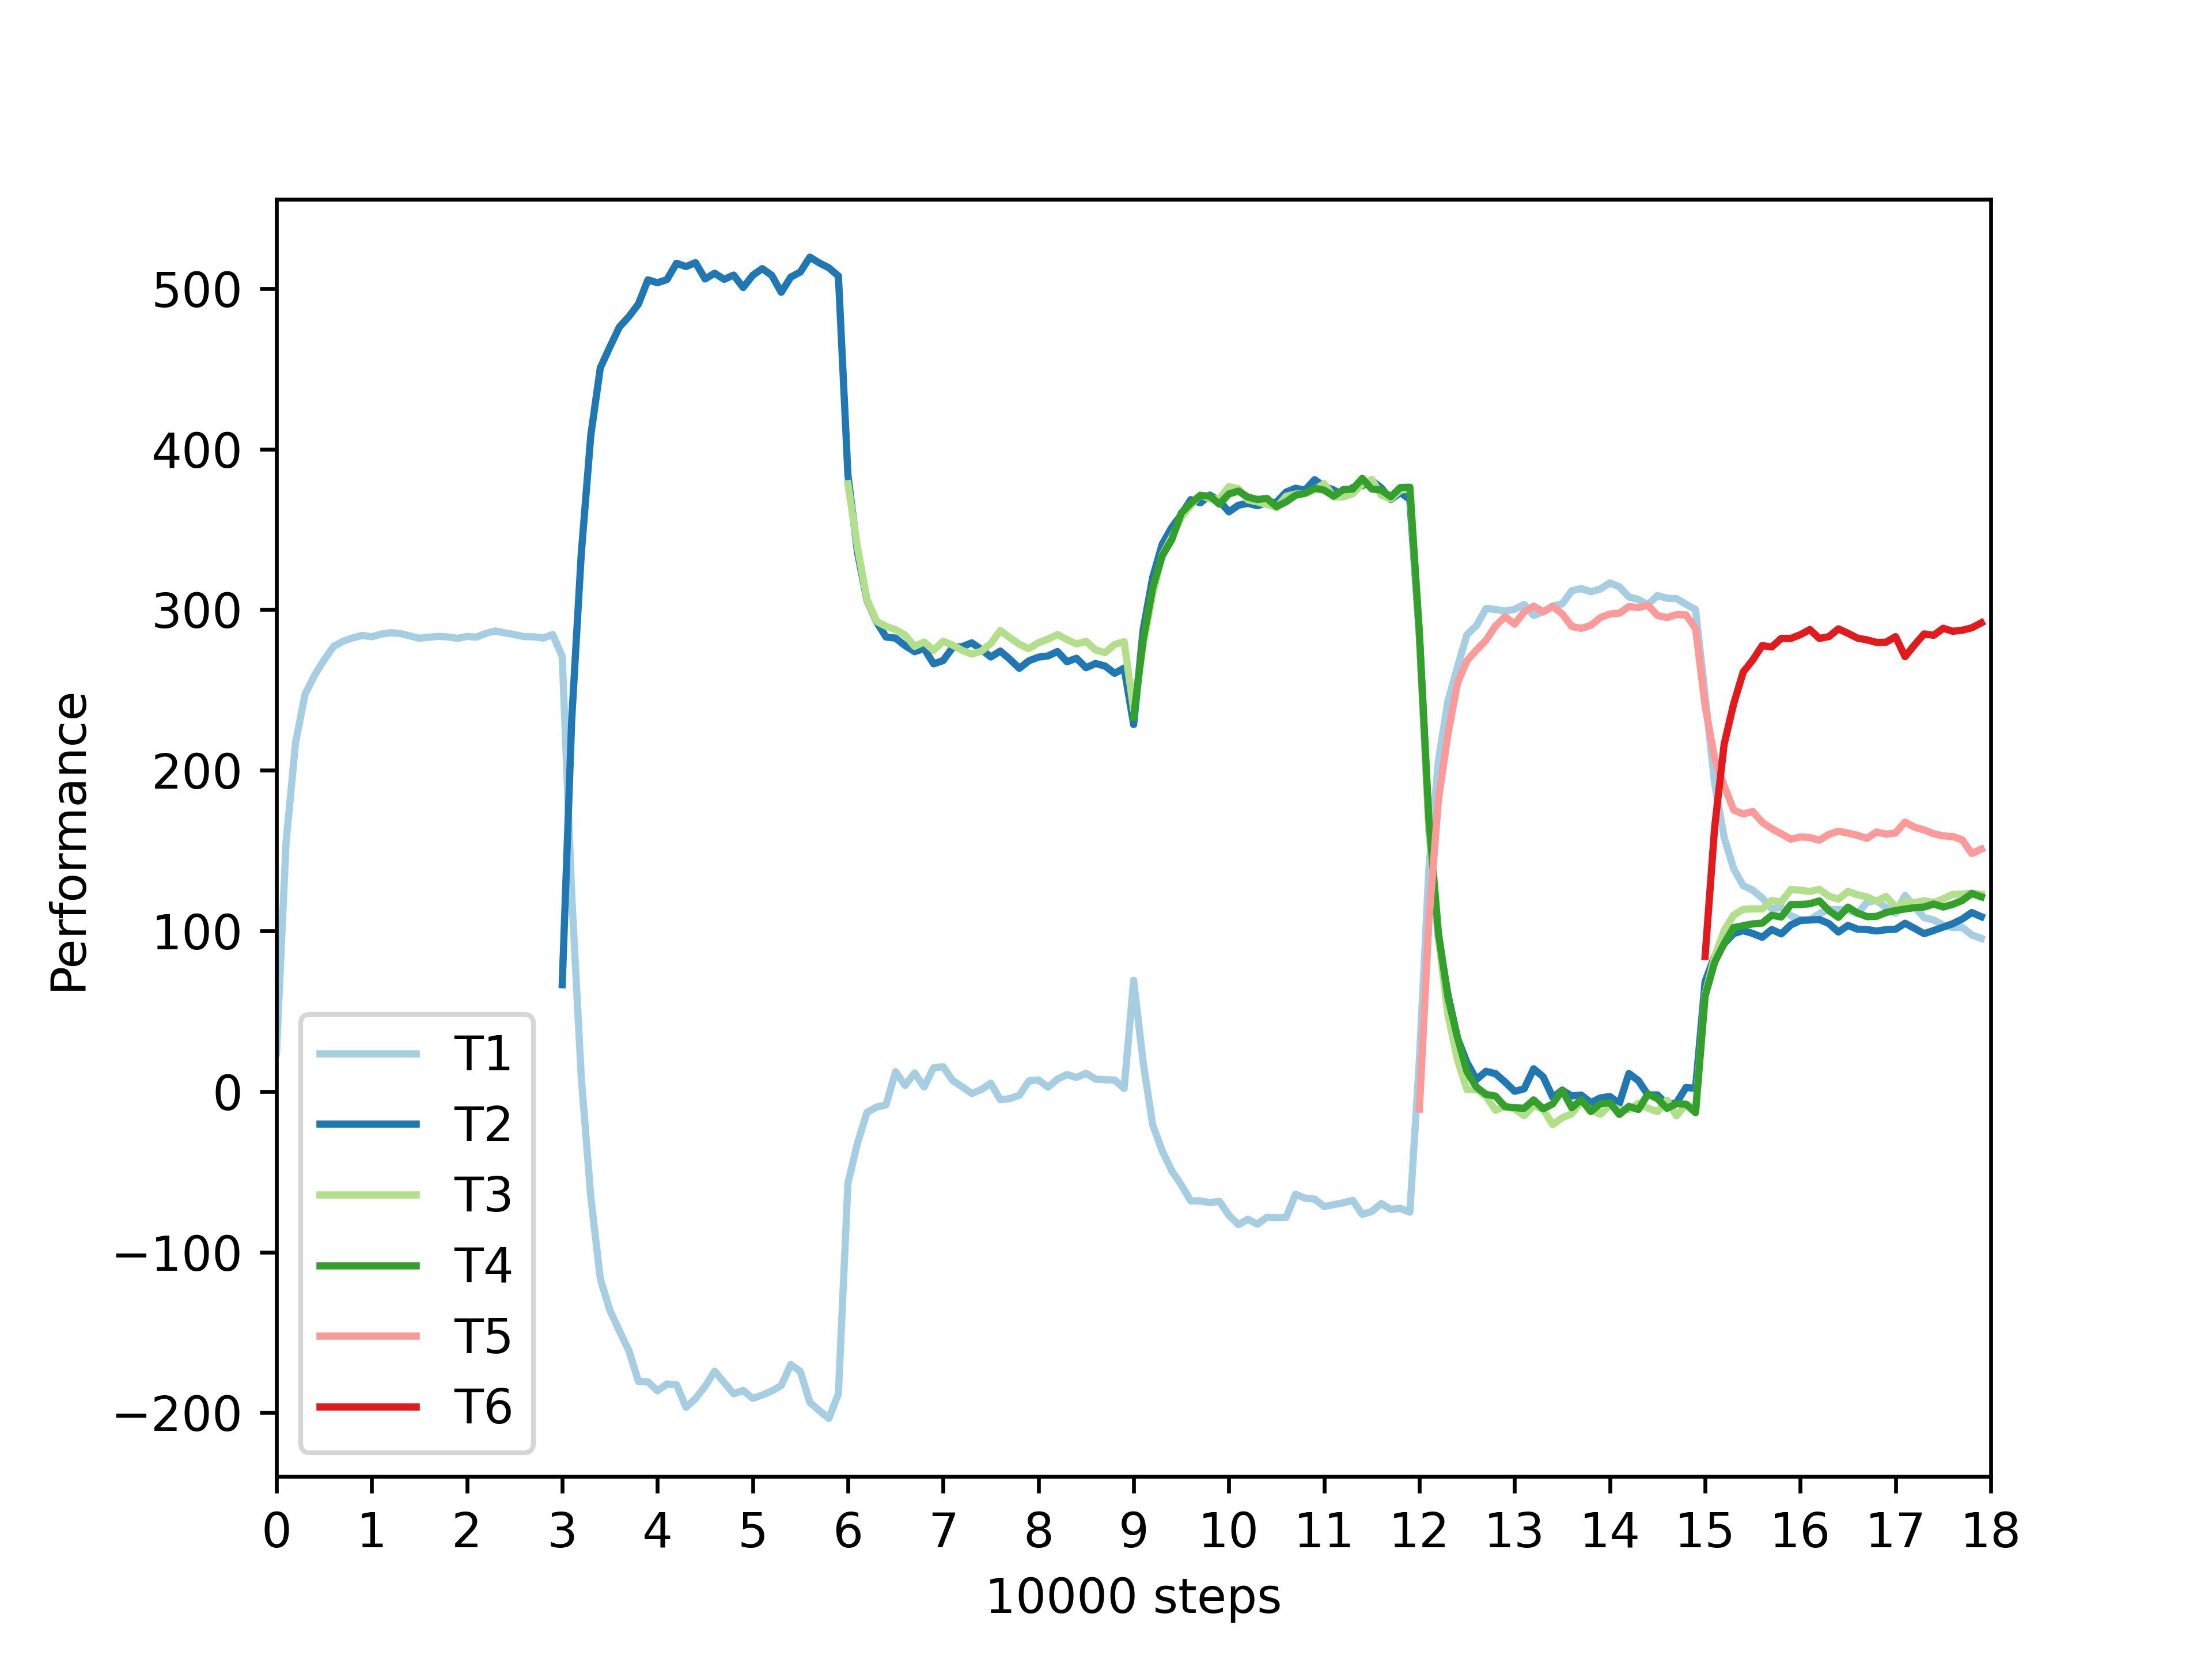}}
    \subcaptionbox{DT + GEM}
    {\includegraphics[width=0.245\linewidth]{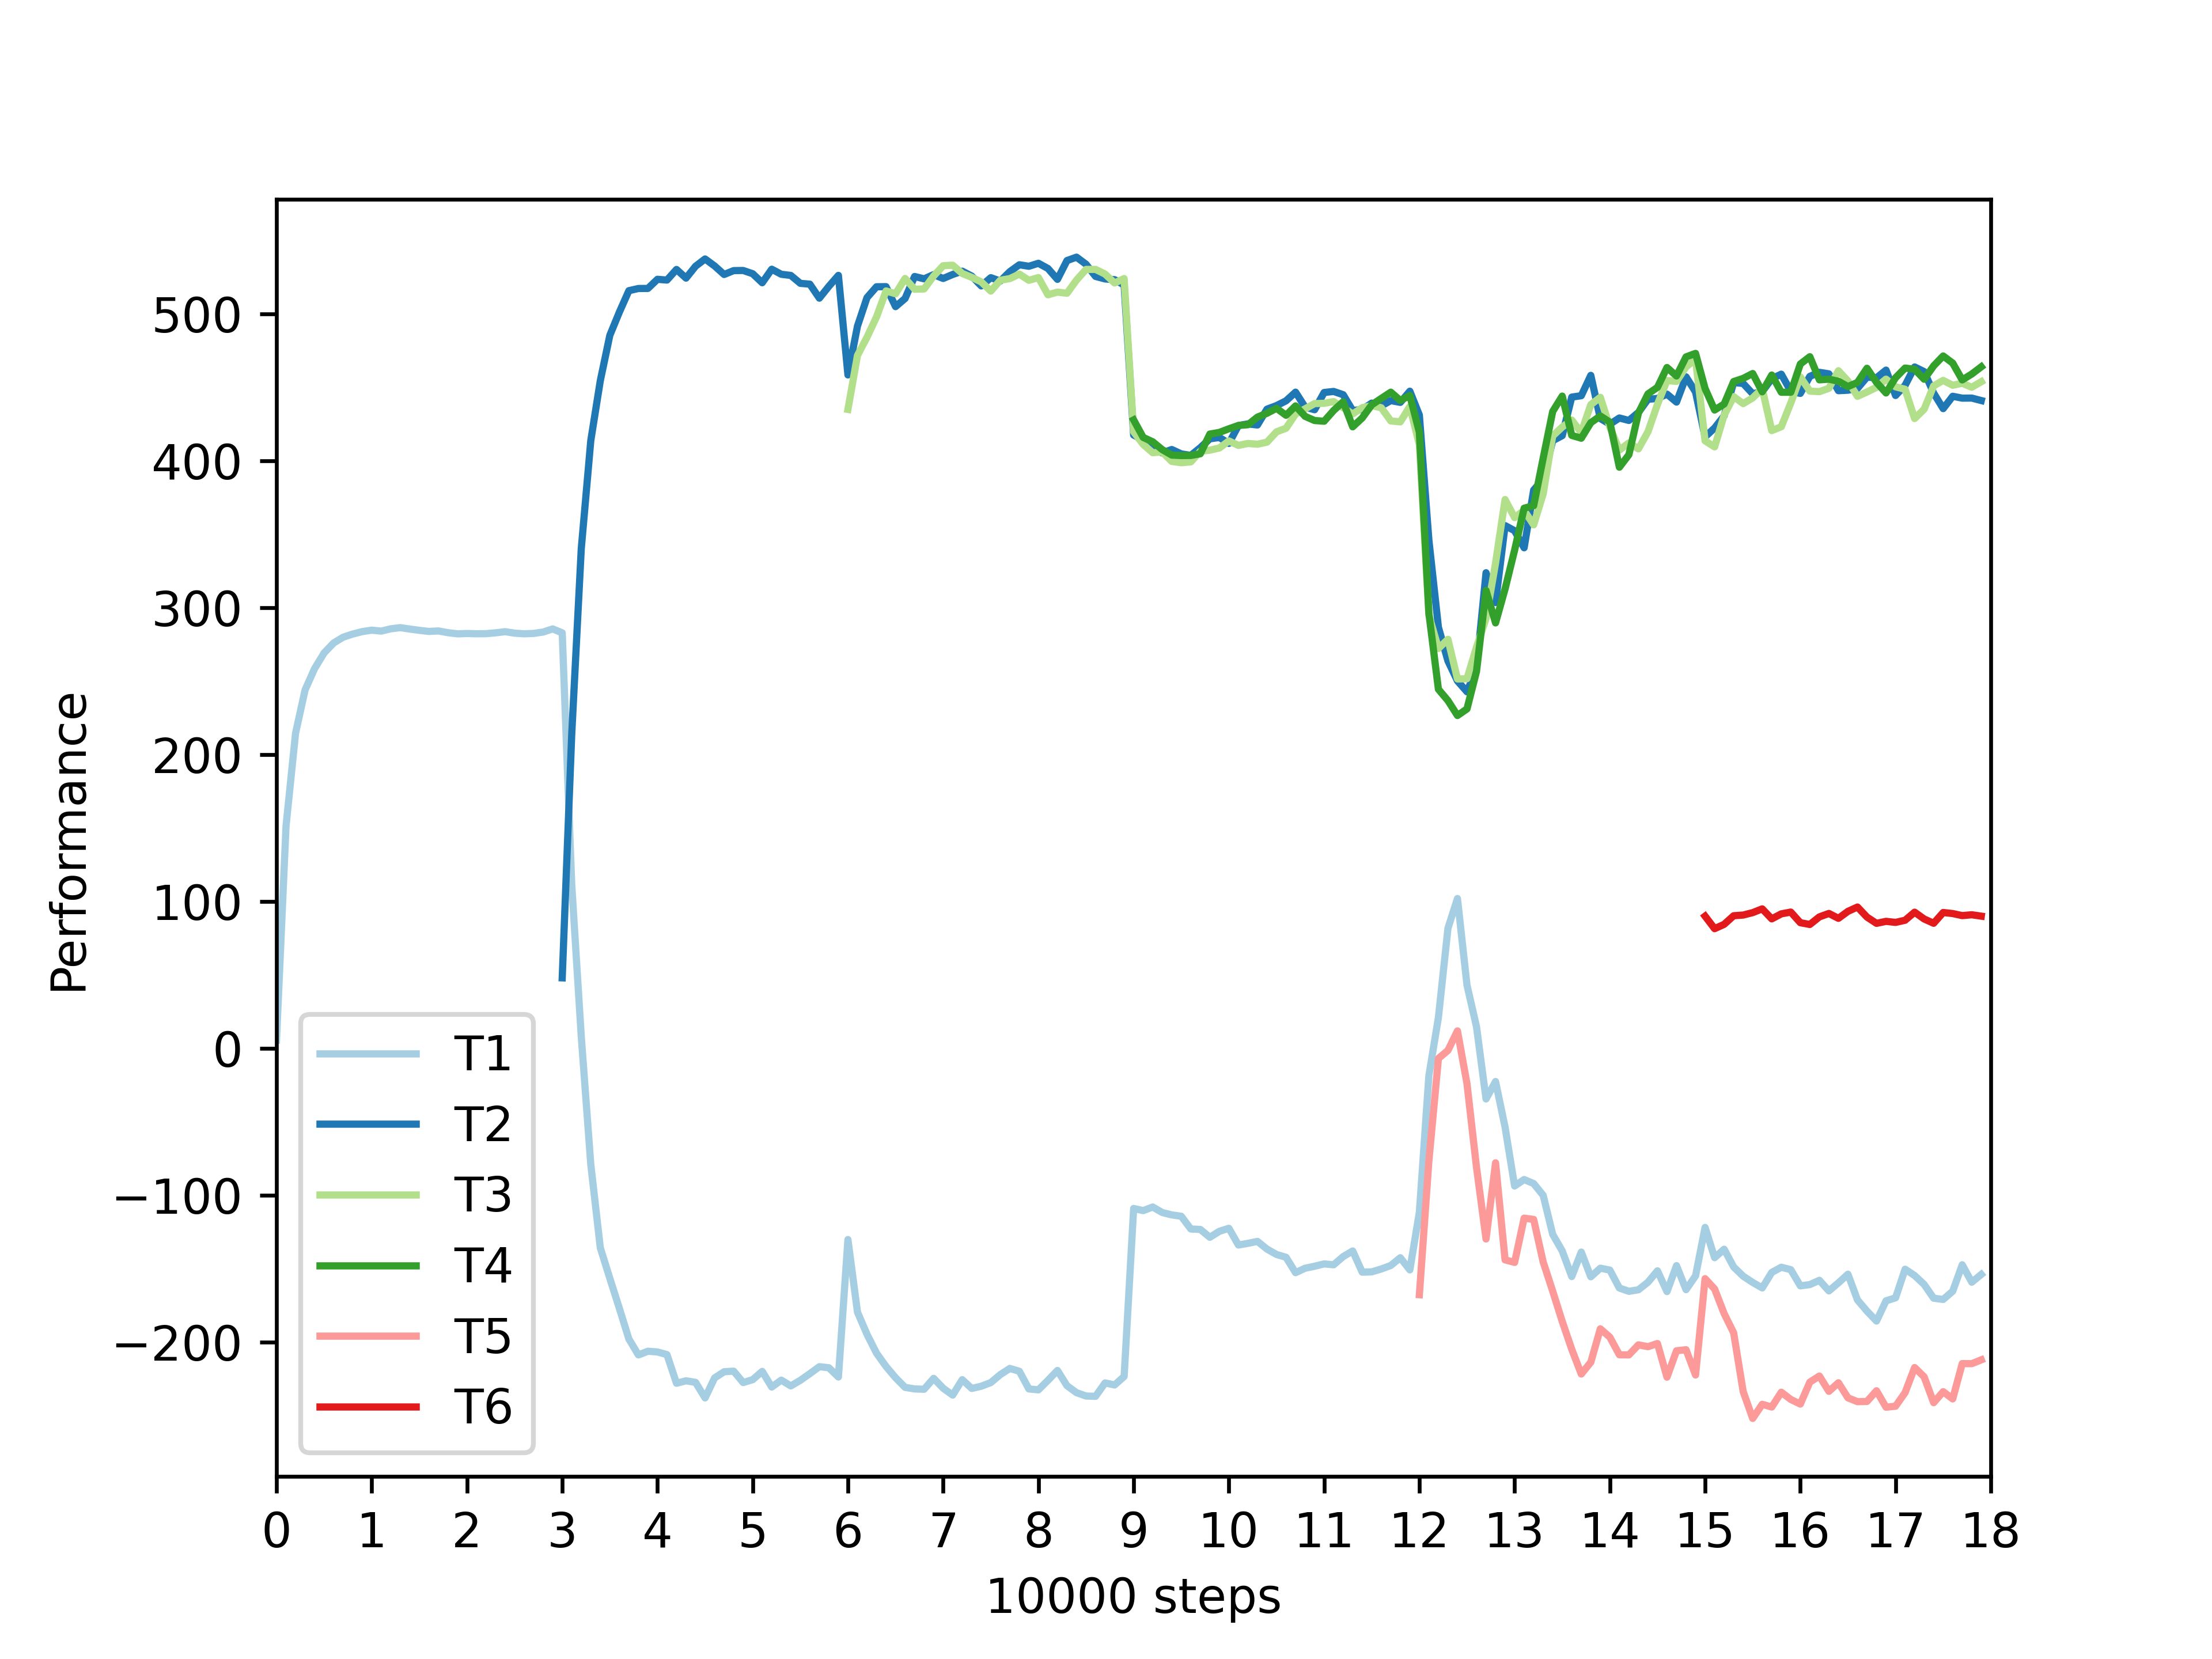}}
	
        \centering	
        \subcaptionbox{Vanilla DT}
    {\includegraphics[width=0.245\linewidth]{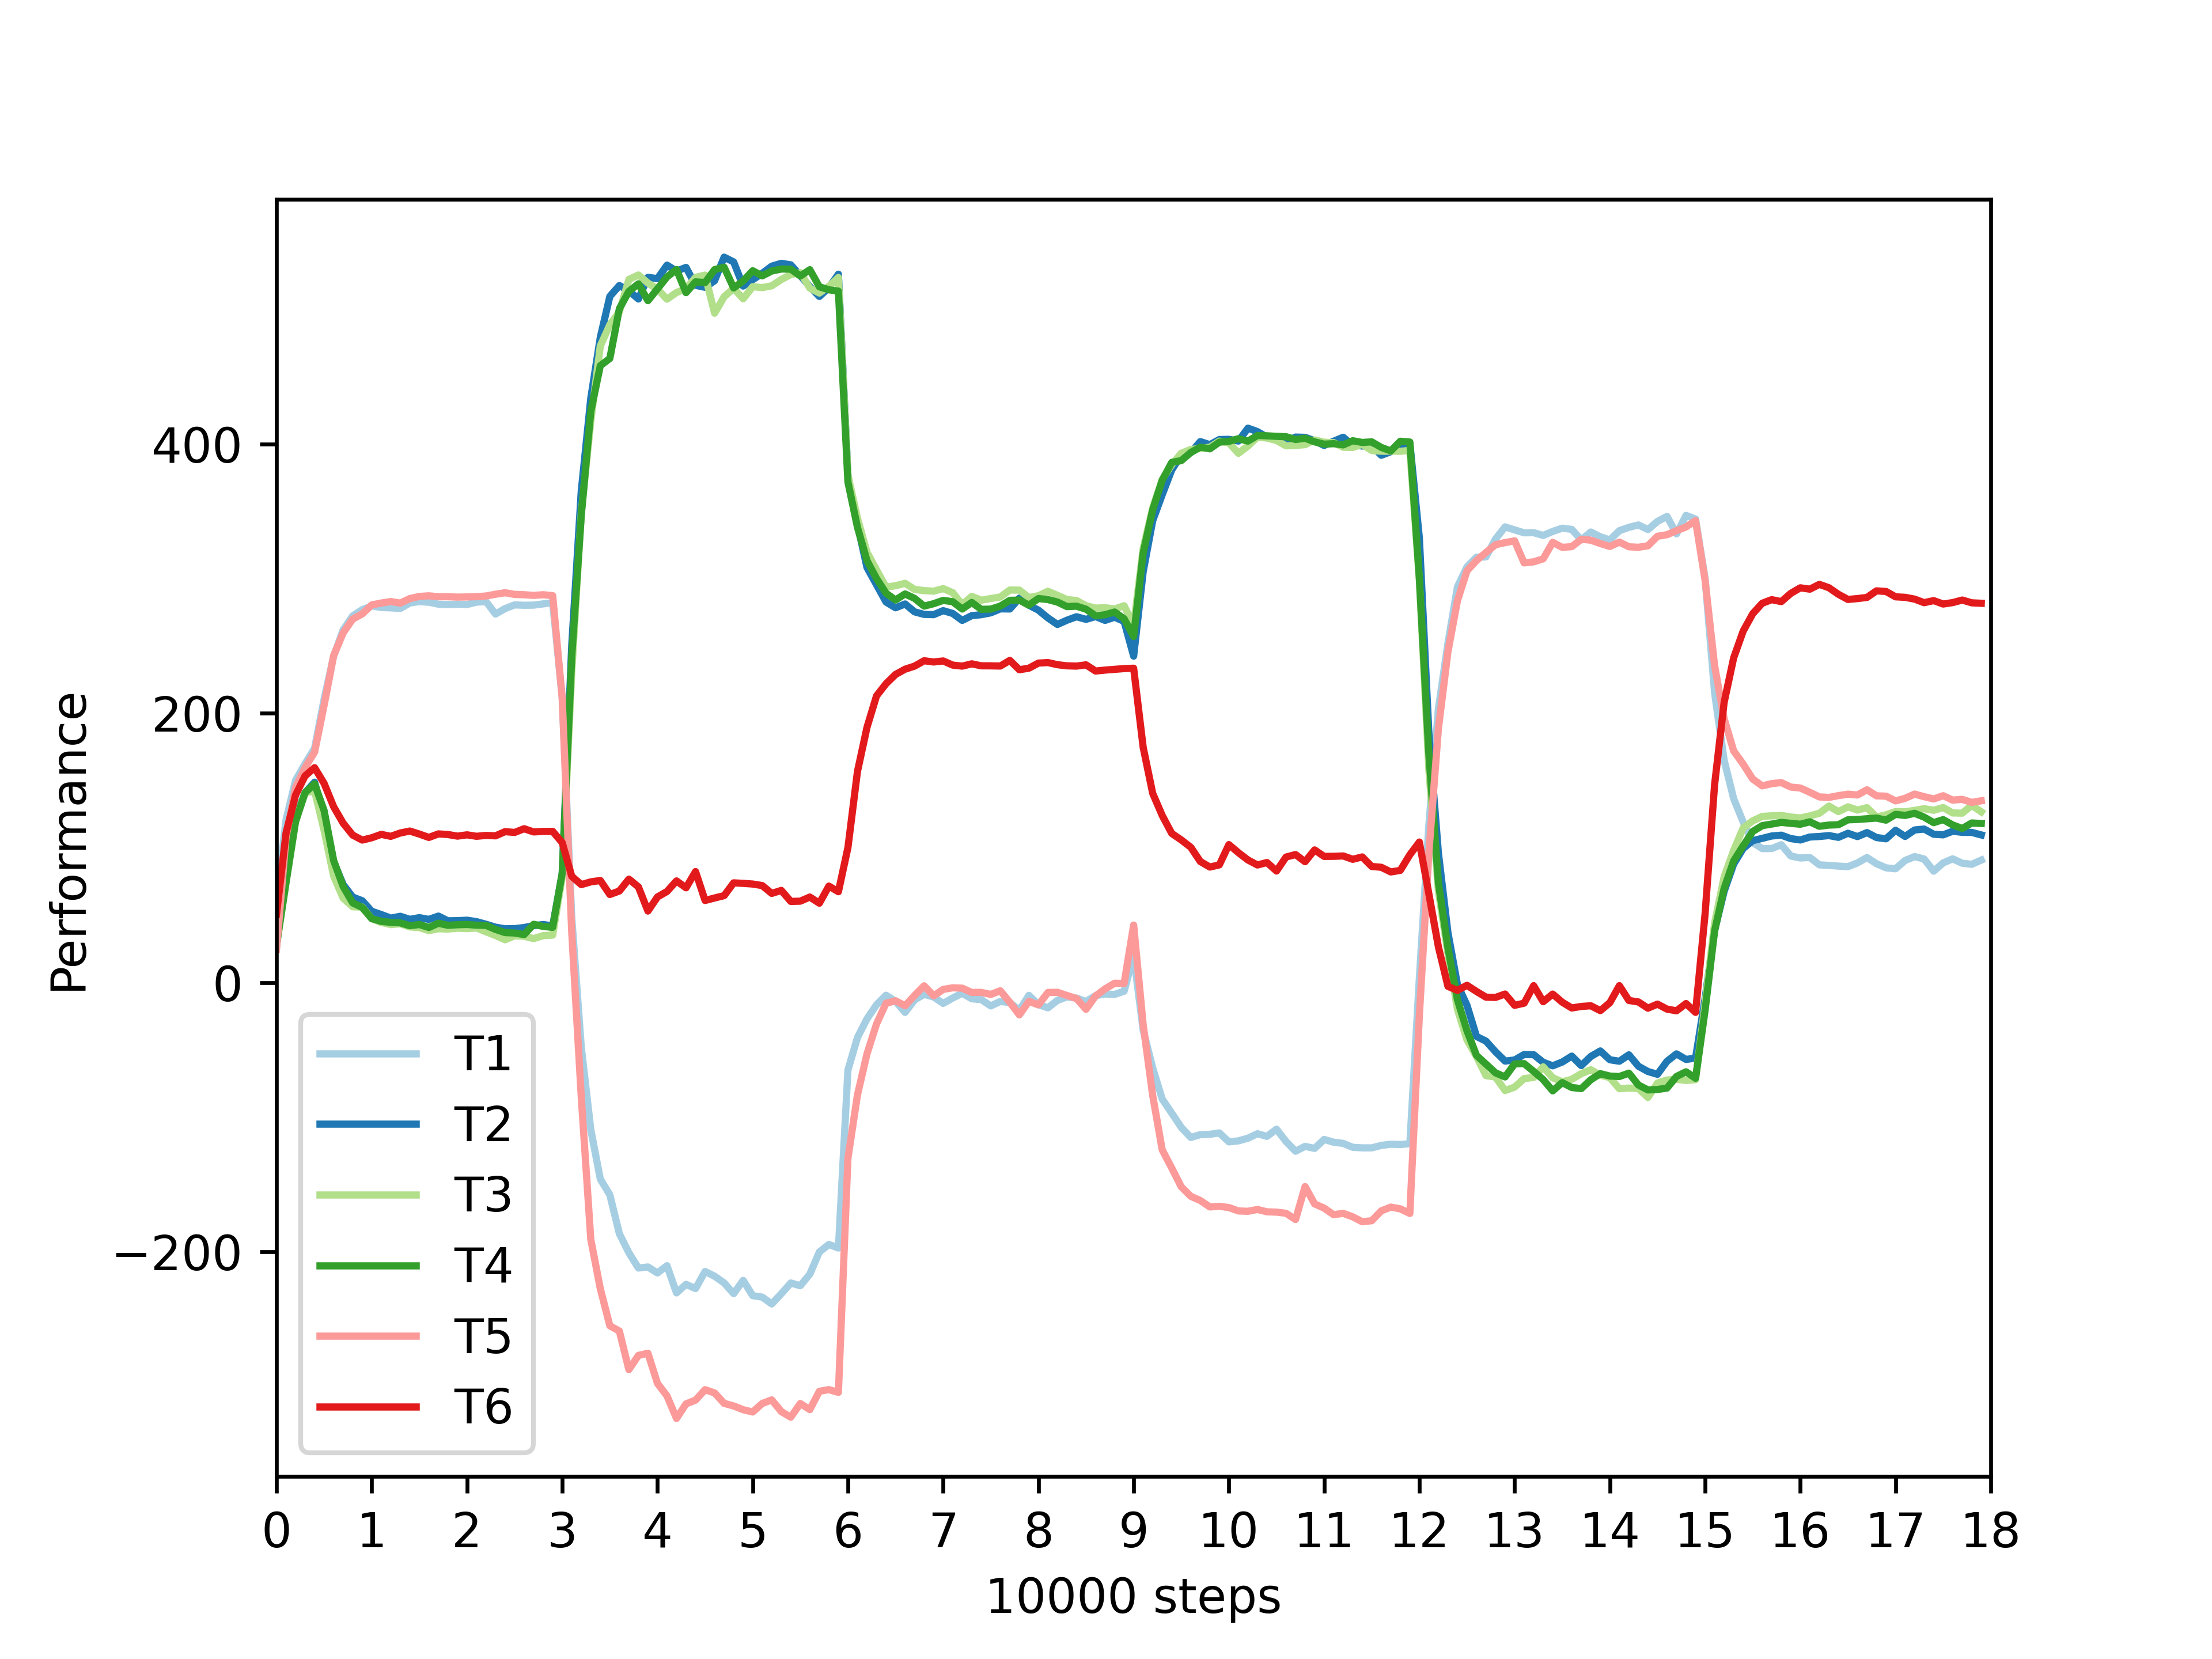}}
        \subcaptionbox{OER}
    {\includegraphics[width=0.245\linewidth]{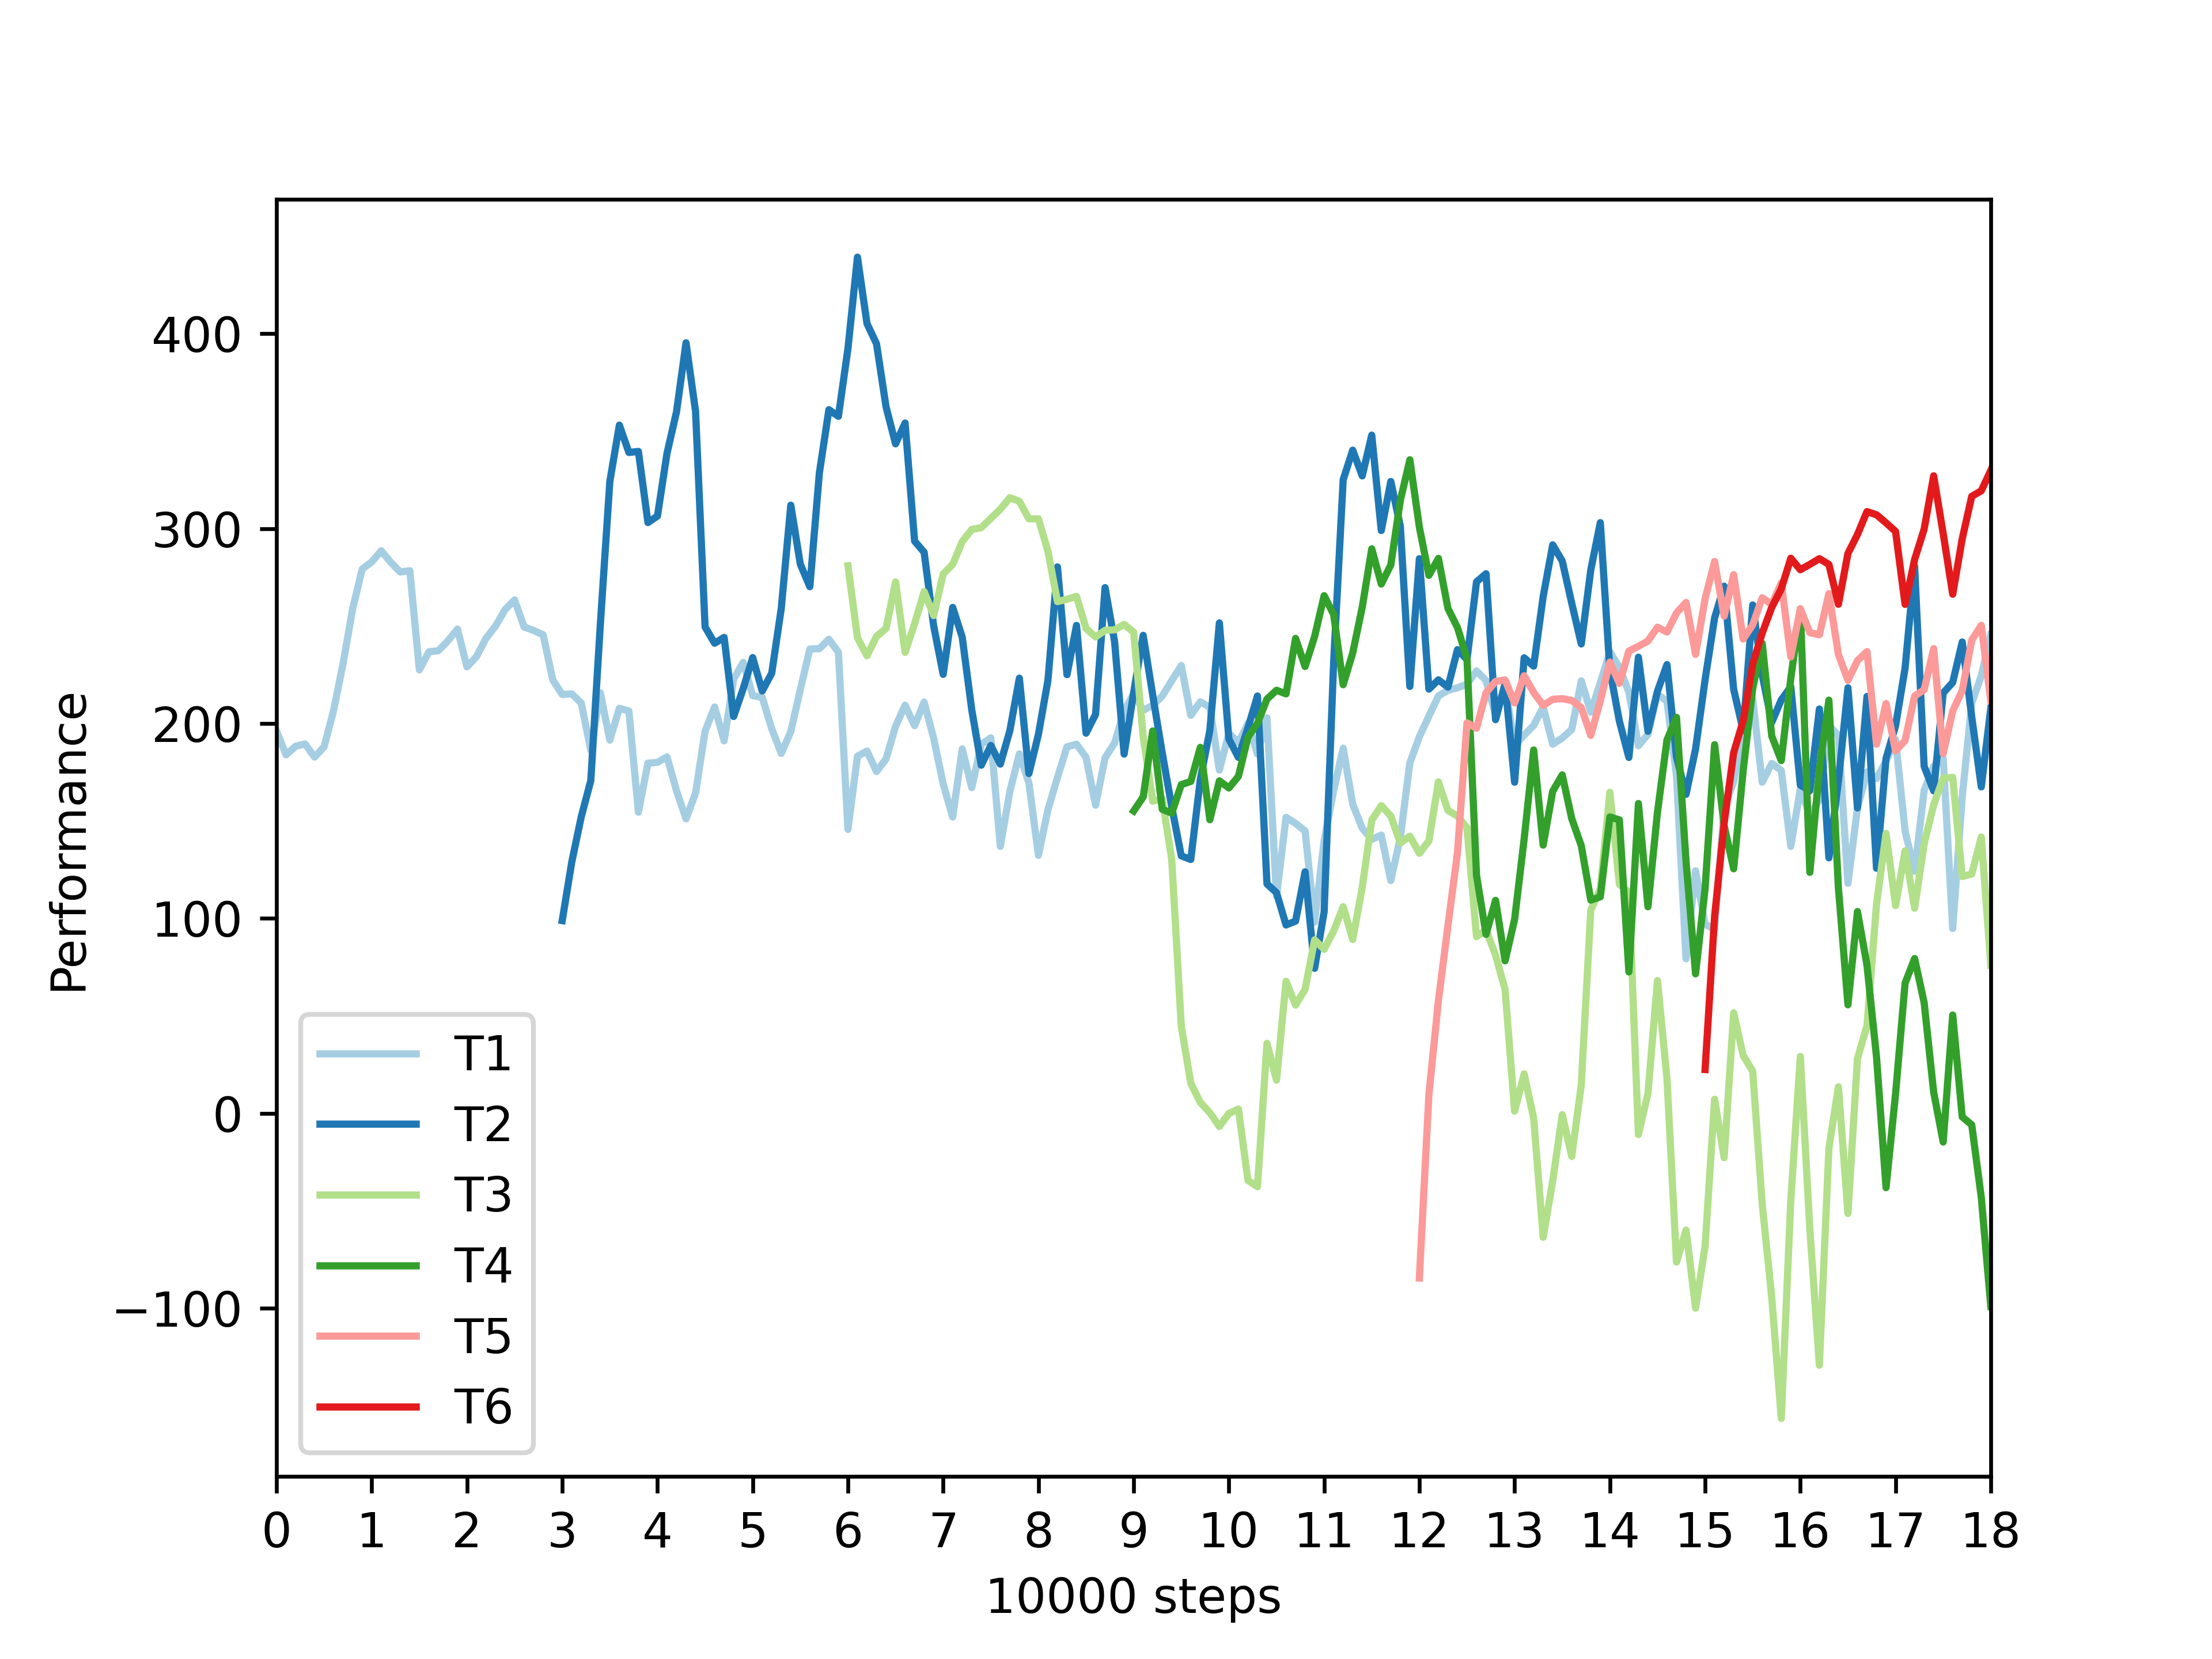}}
         \subcaptionbox{MH-DT}
    {\includegraphics[width=0.245\linewidth]{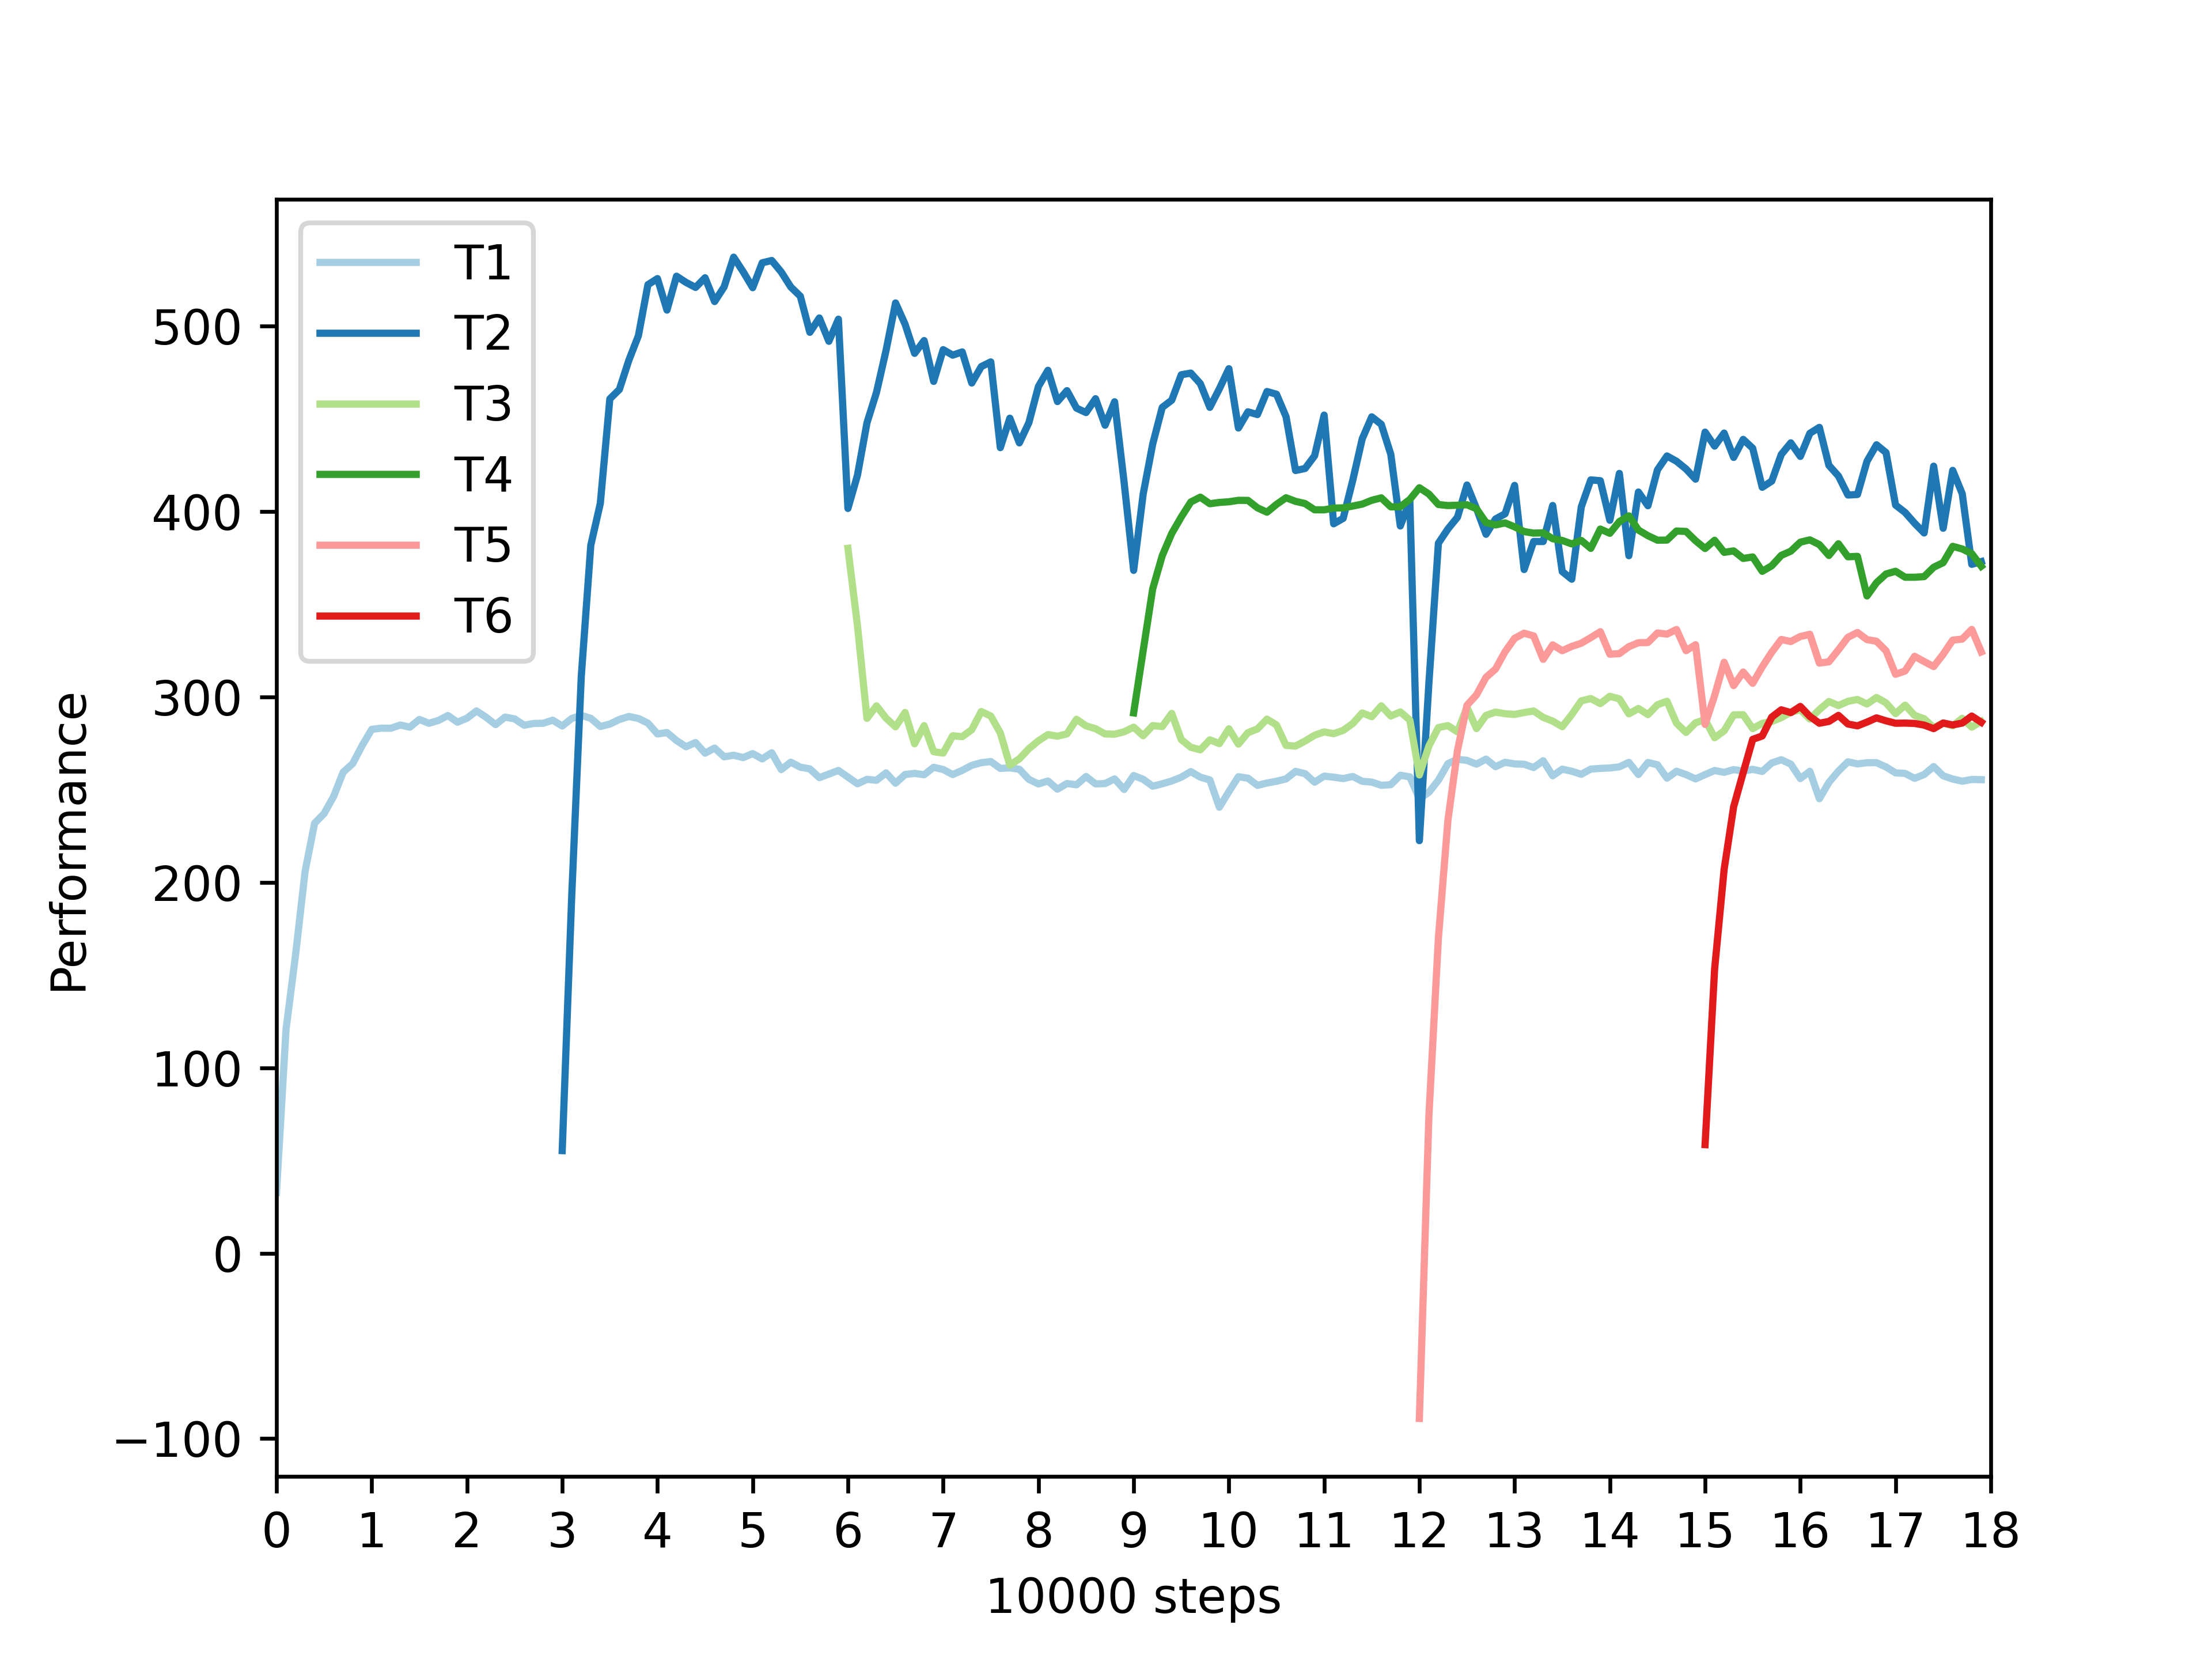}}
	\subcaptionbox{LoRA-DT}
    {\includegraphics[width=0.245\linewidth]{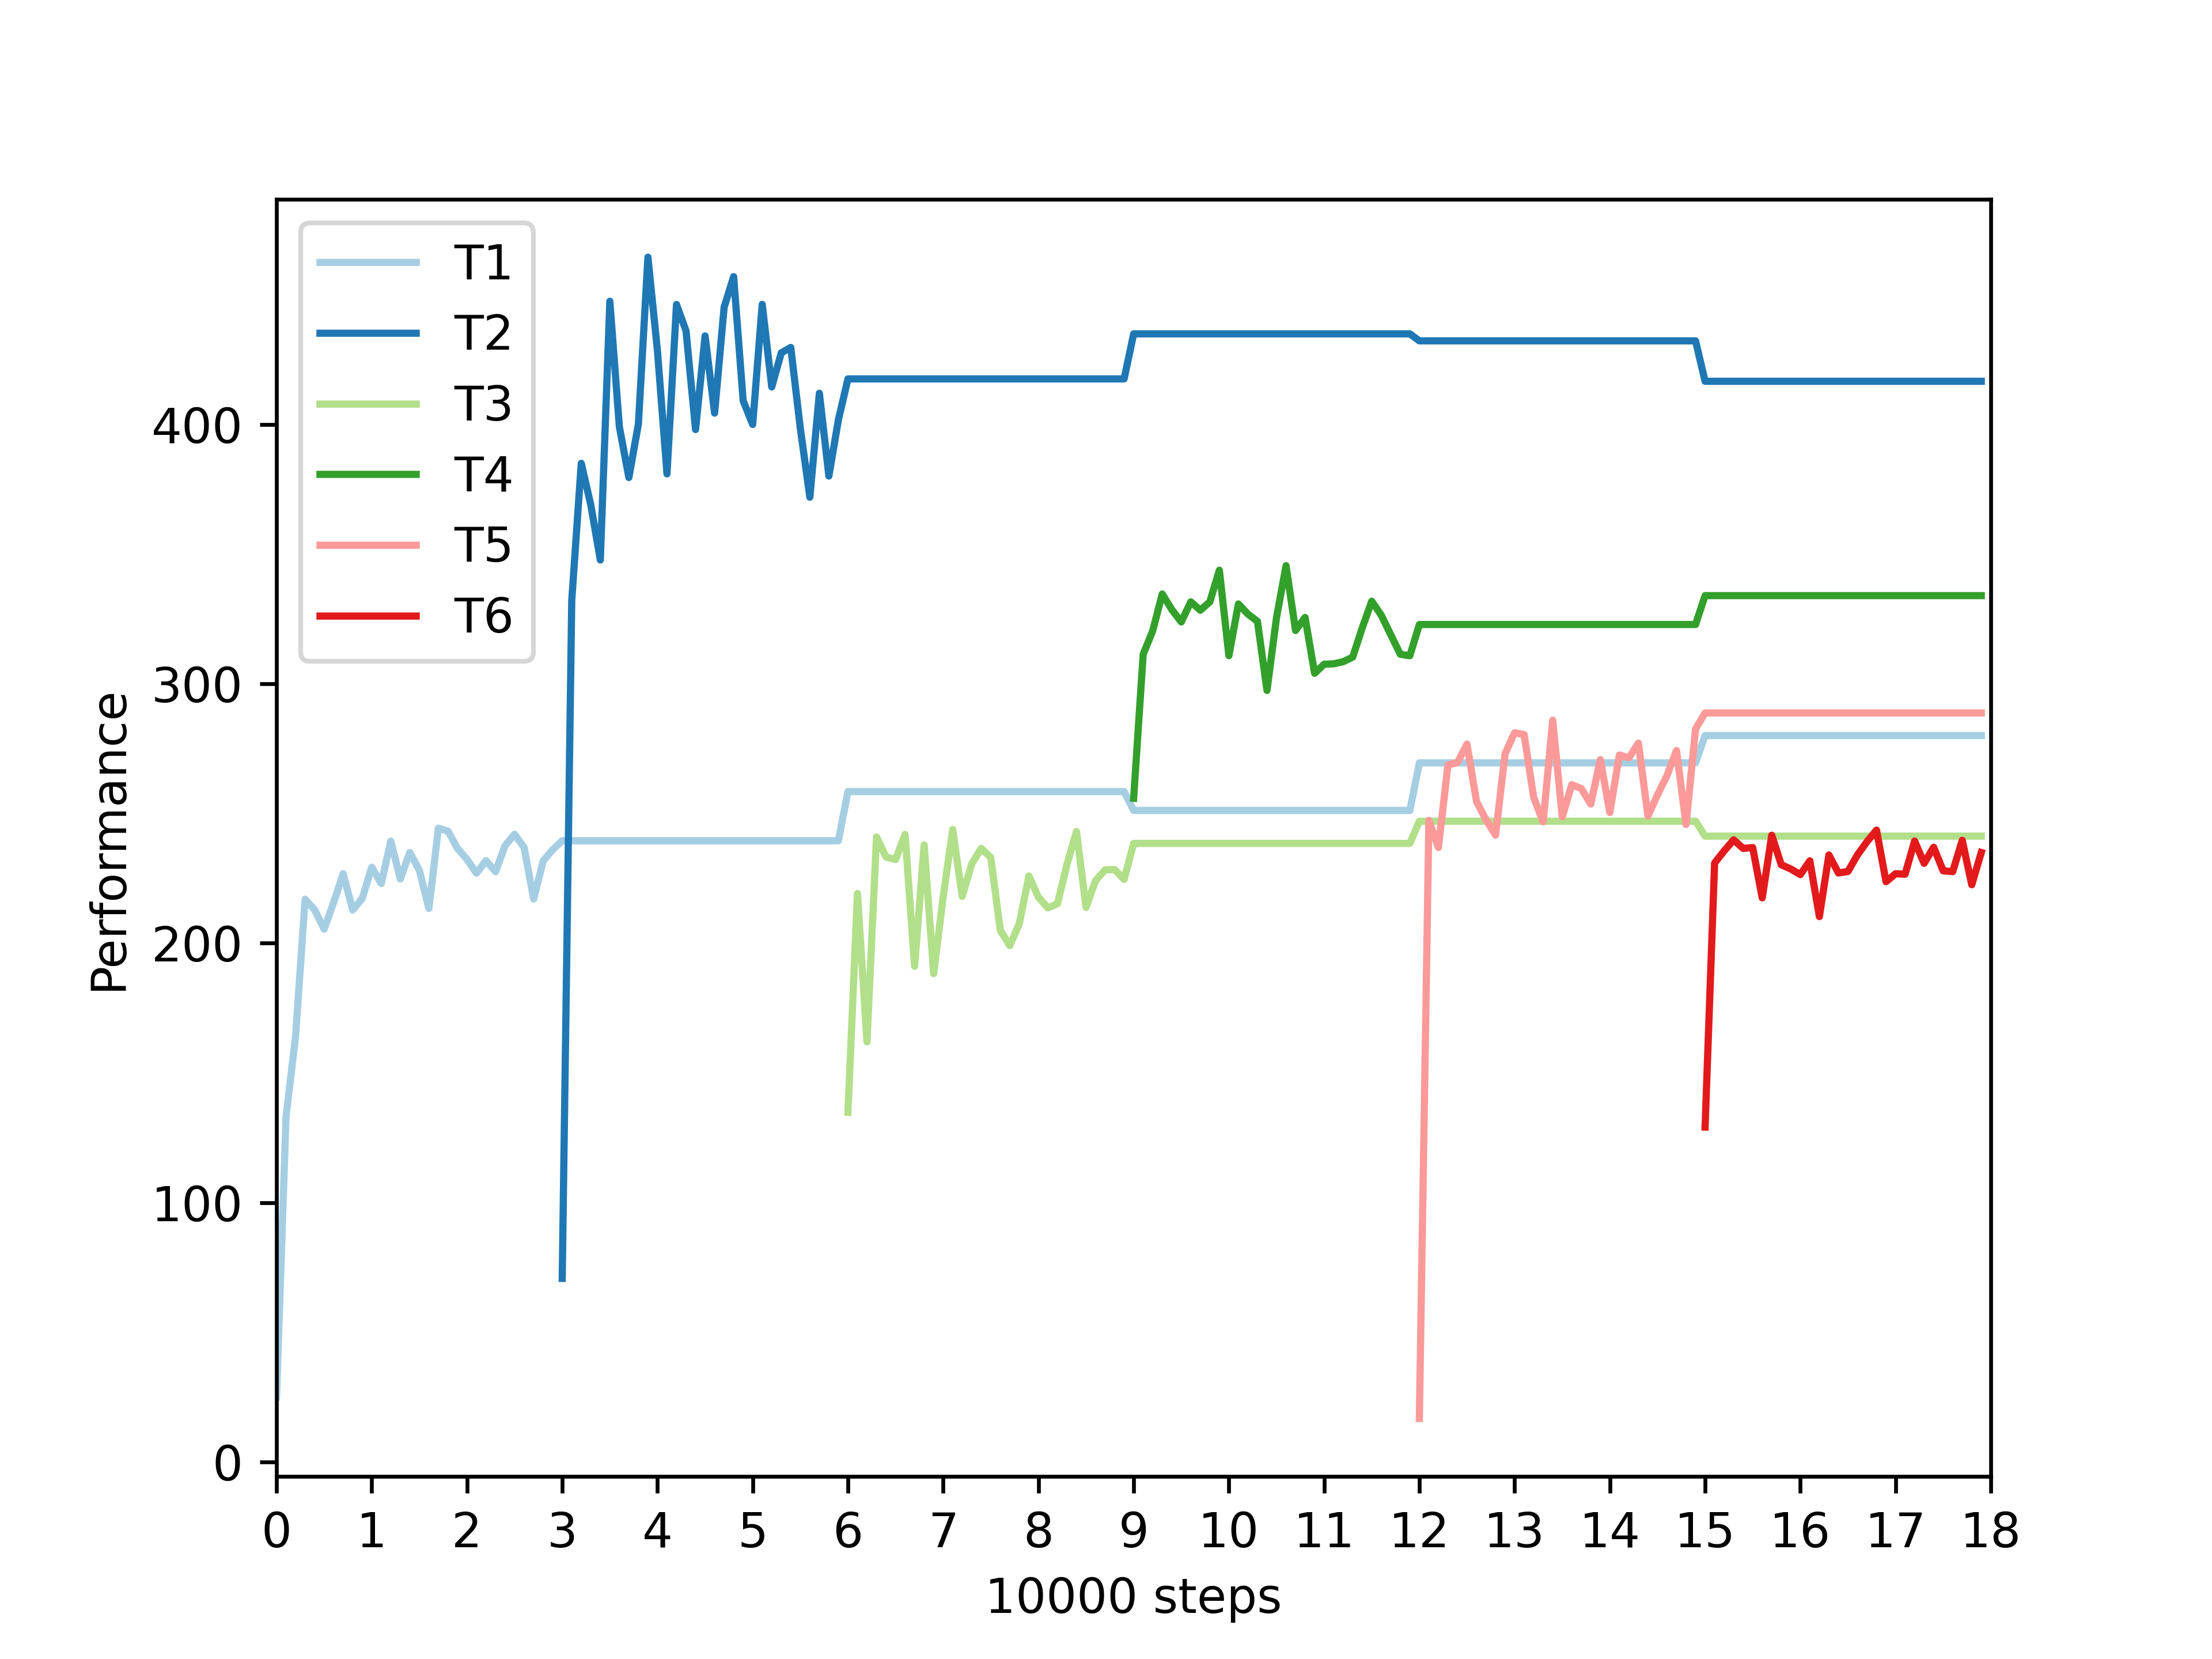}}
    \caption{Ant\_Dir (middle)}
\end{figure}

\begin{figure}[htbp]
	\centering
	\subcaptionbox{PDT}
    {\includegraphics[width=0.245\linewidth]{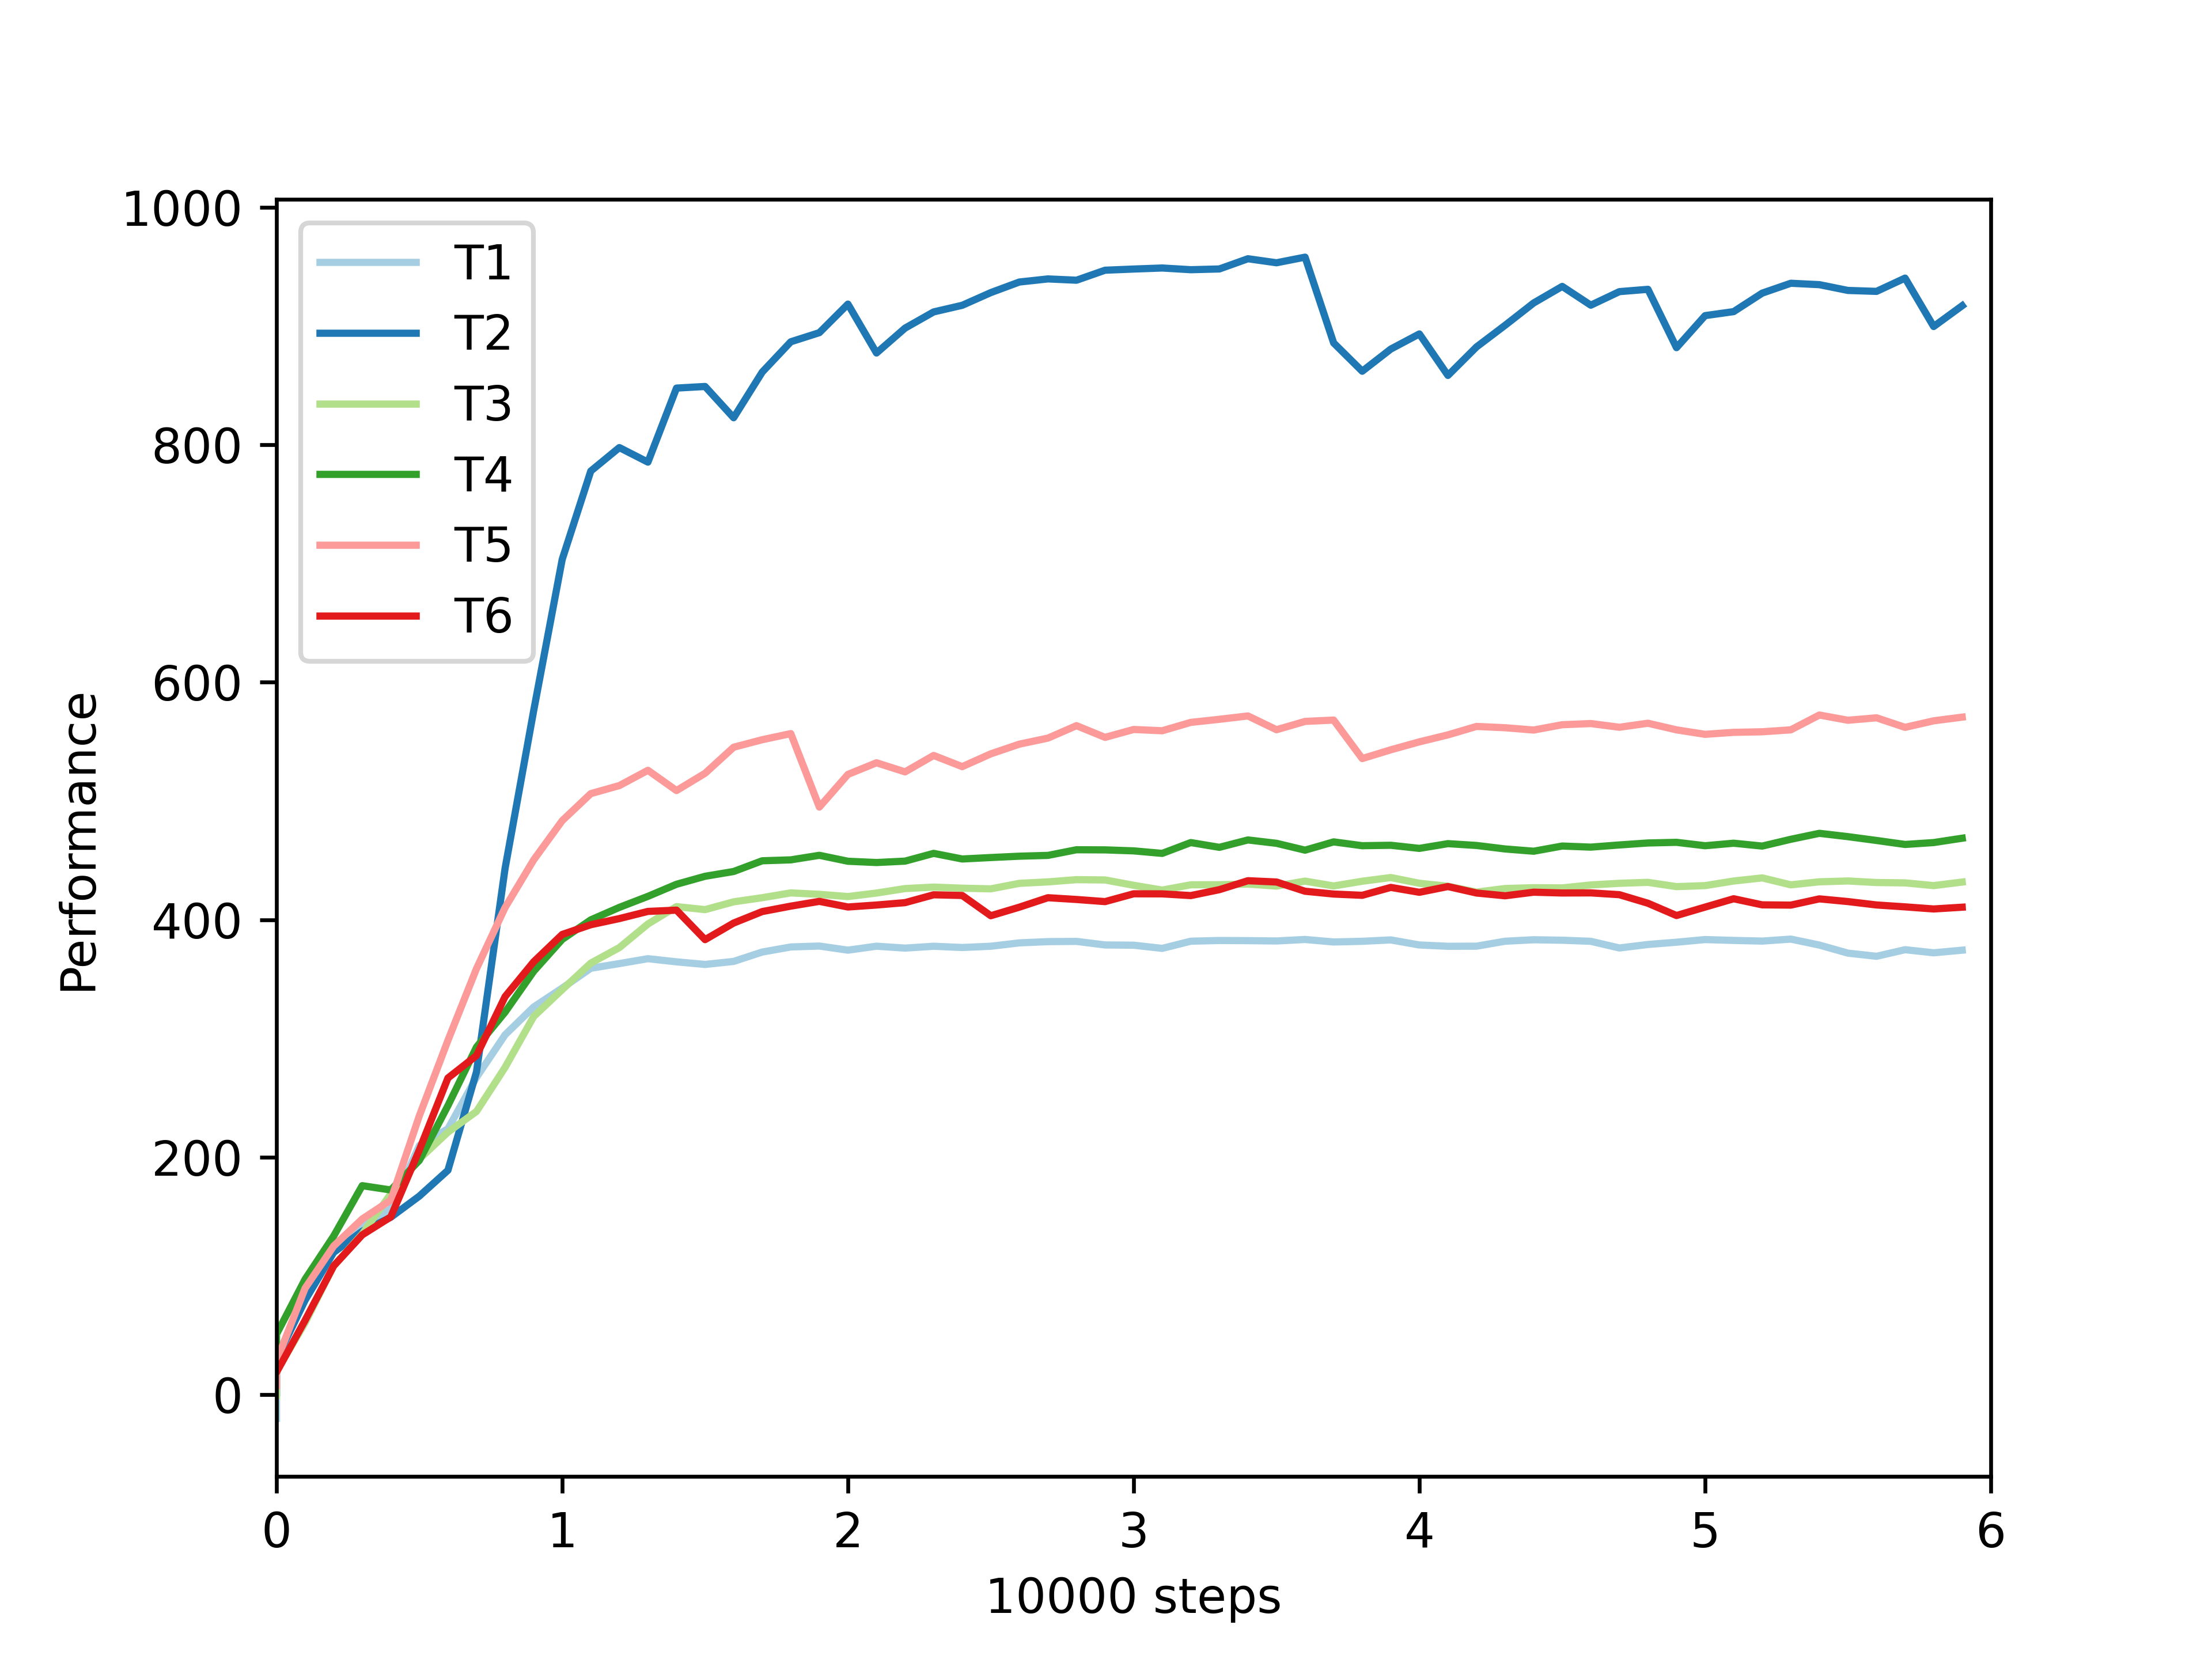}}
    \subcaptionbox{DT + EWC}
    {\includegraphics[width=0.245\linewidth]{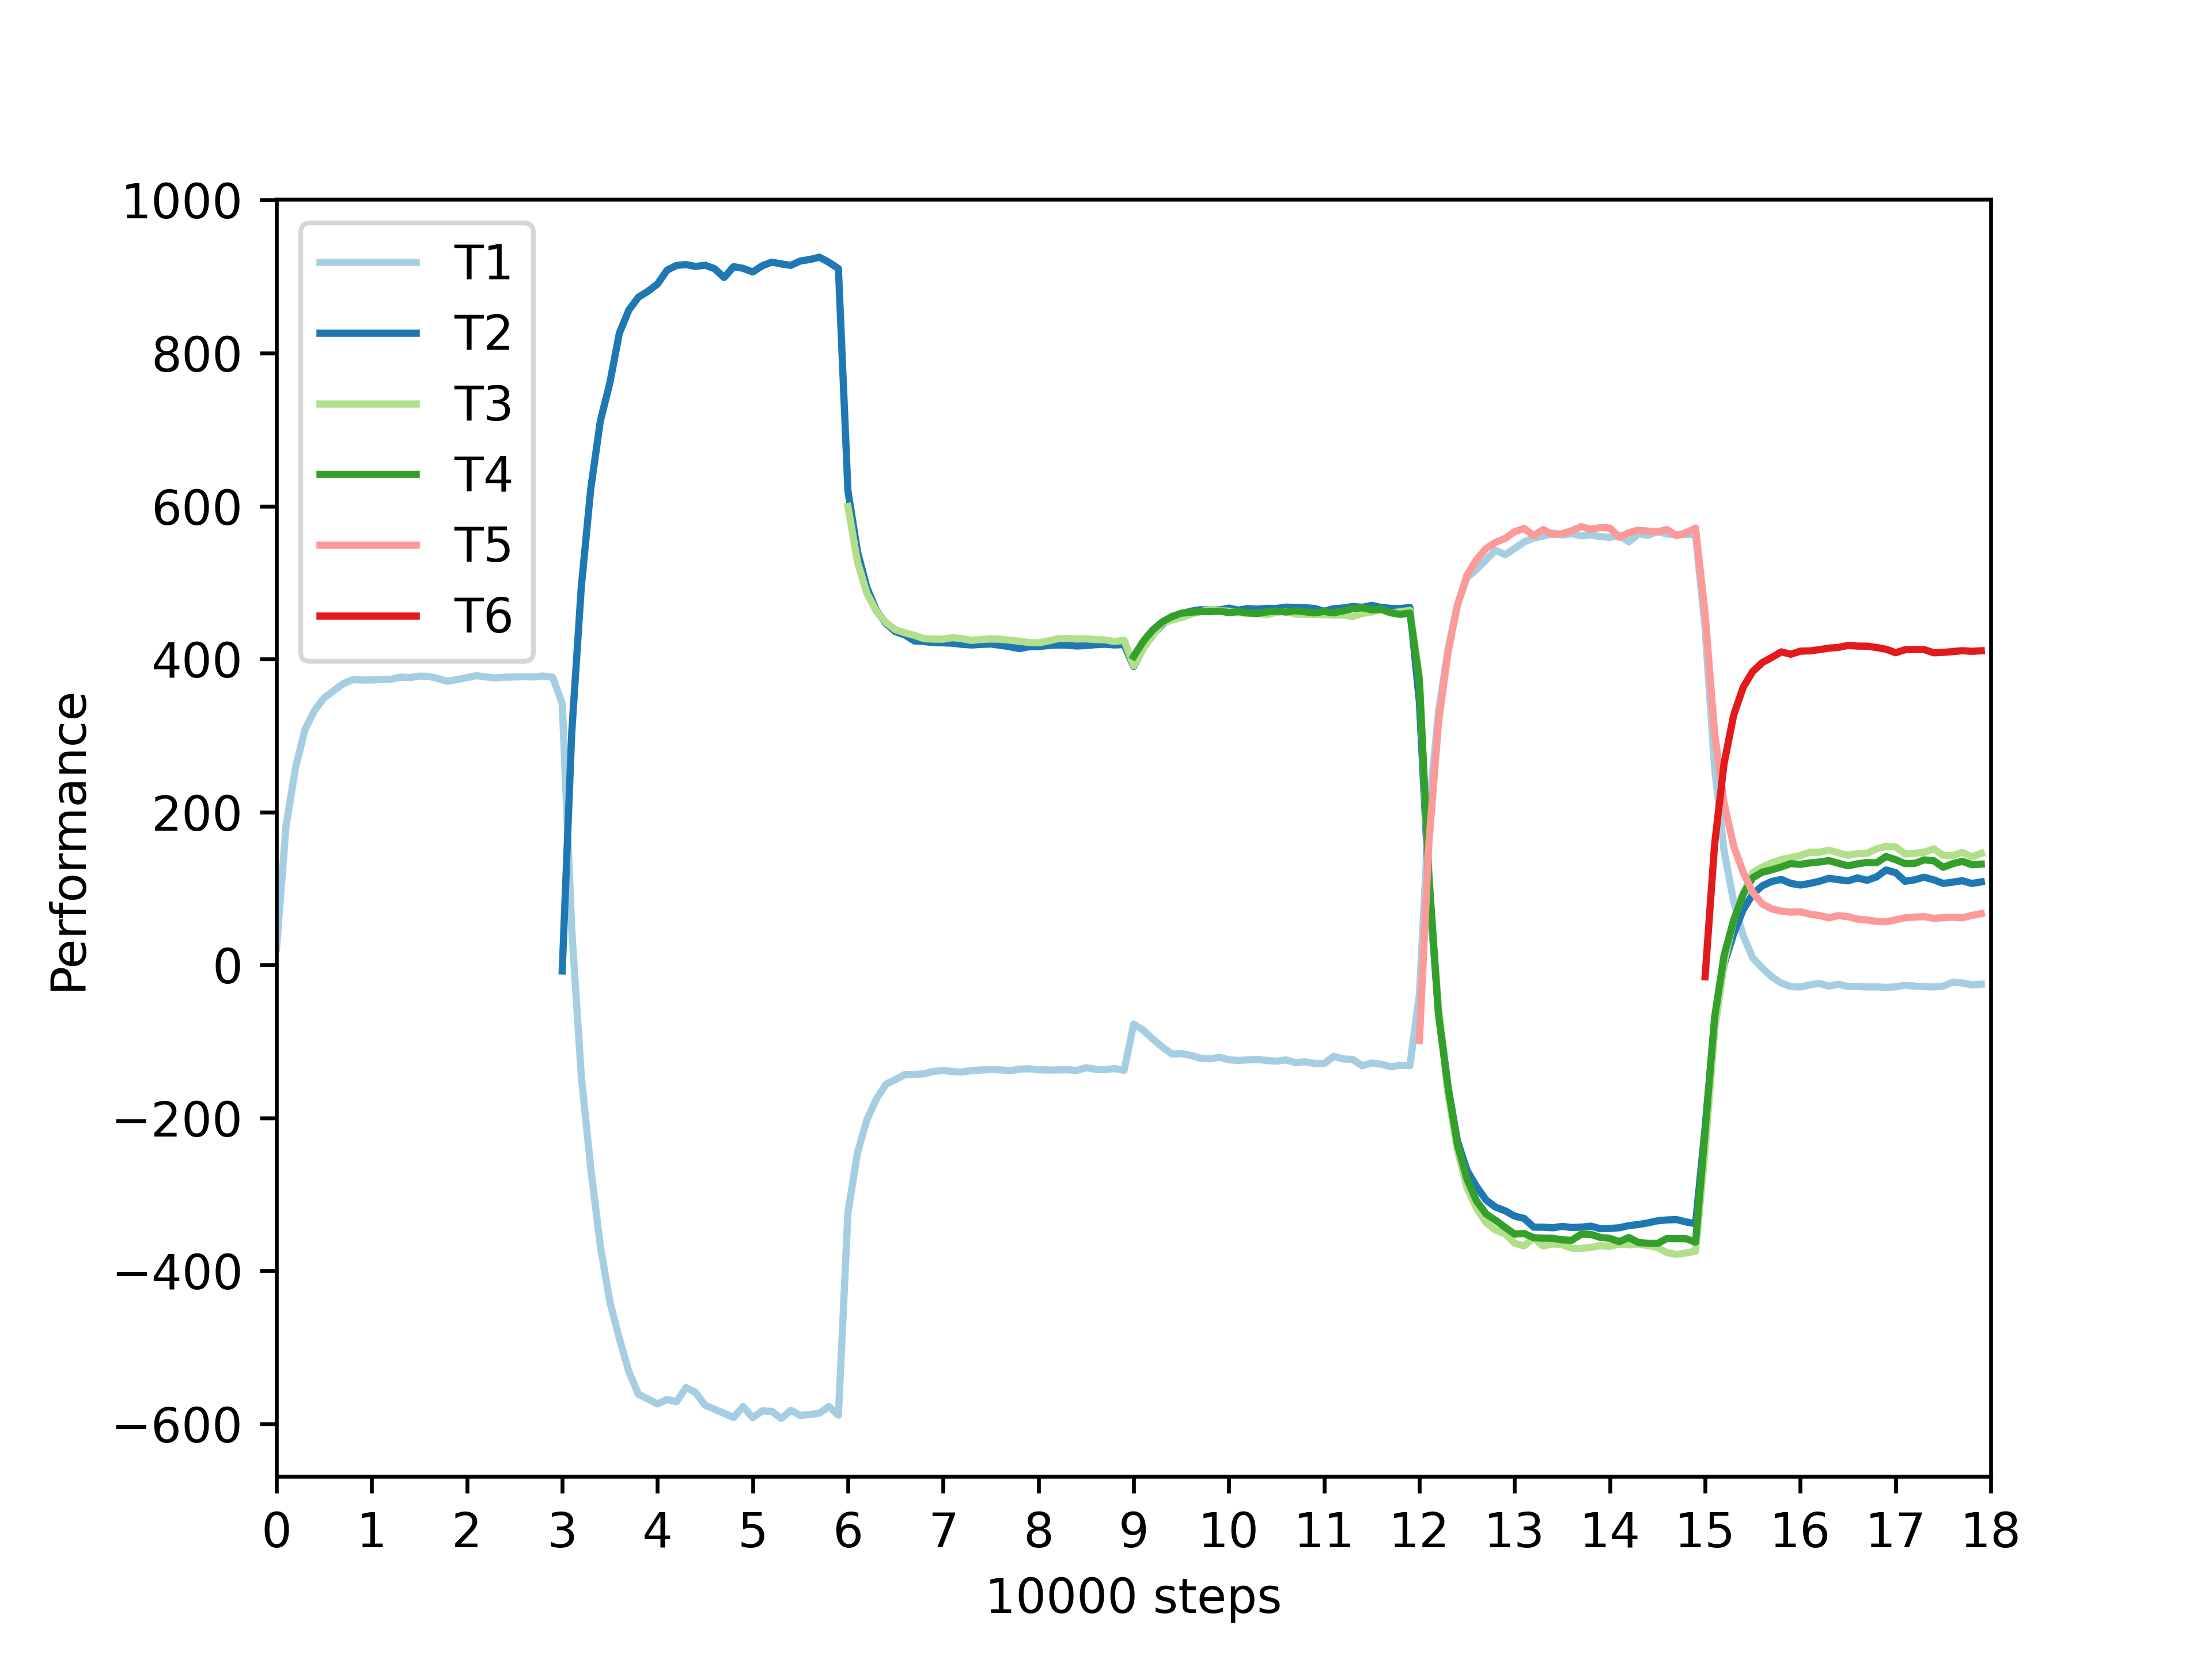}}
    \subcaptionbox{DT + SI}
    {\includegraphics[width=0.245\linewidth]{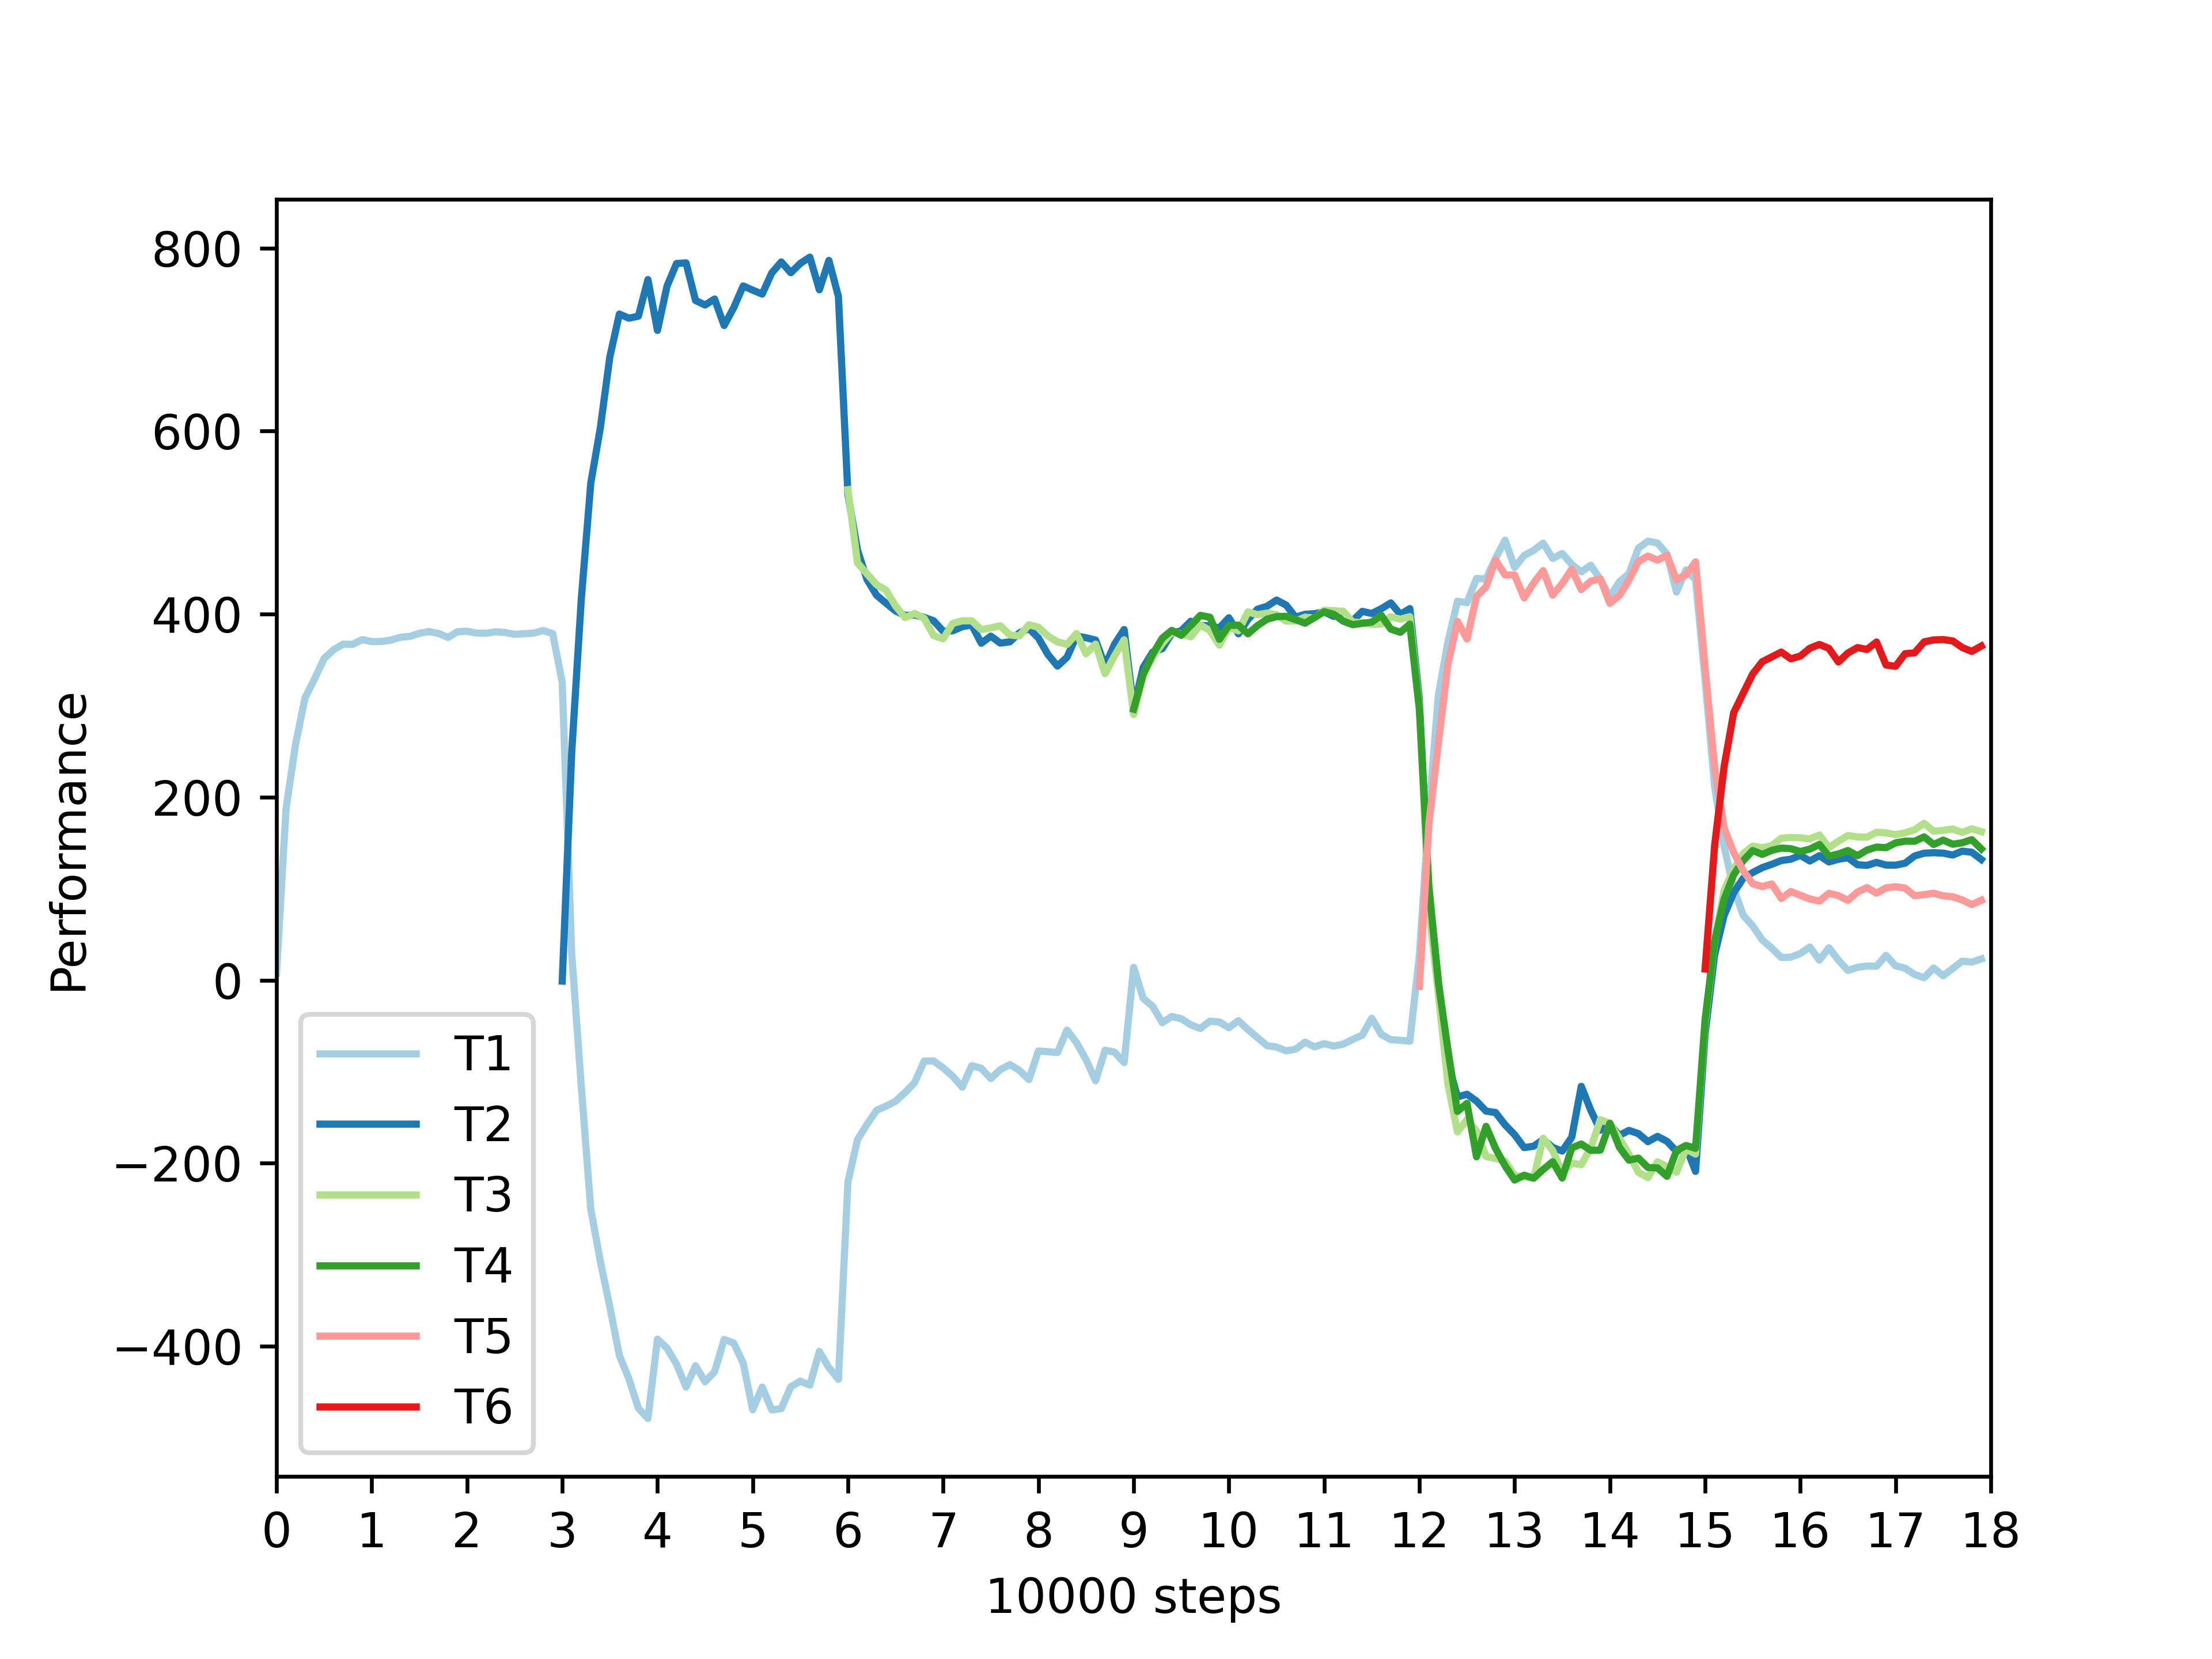}}
    \subcaptionbox{DT + GEM}
    {\includegraphics[width=0.245\linewidth]{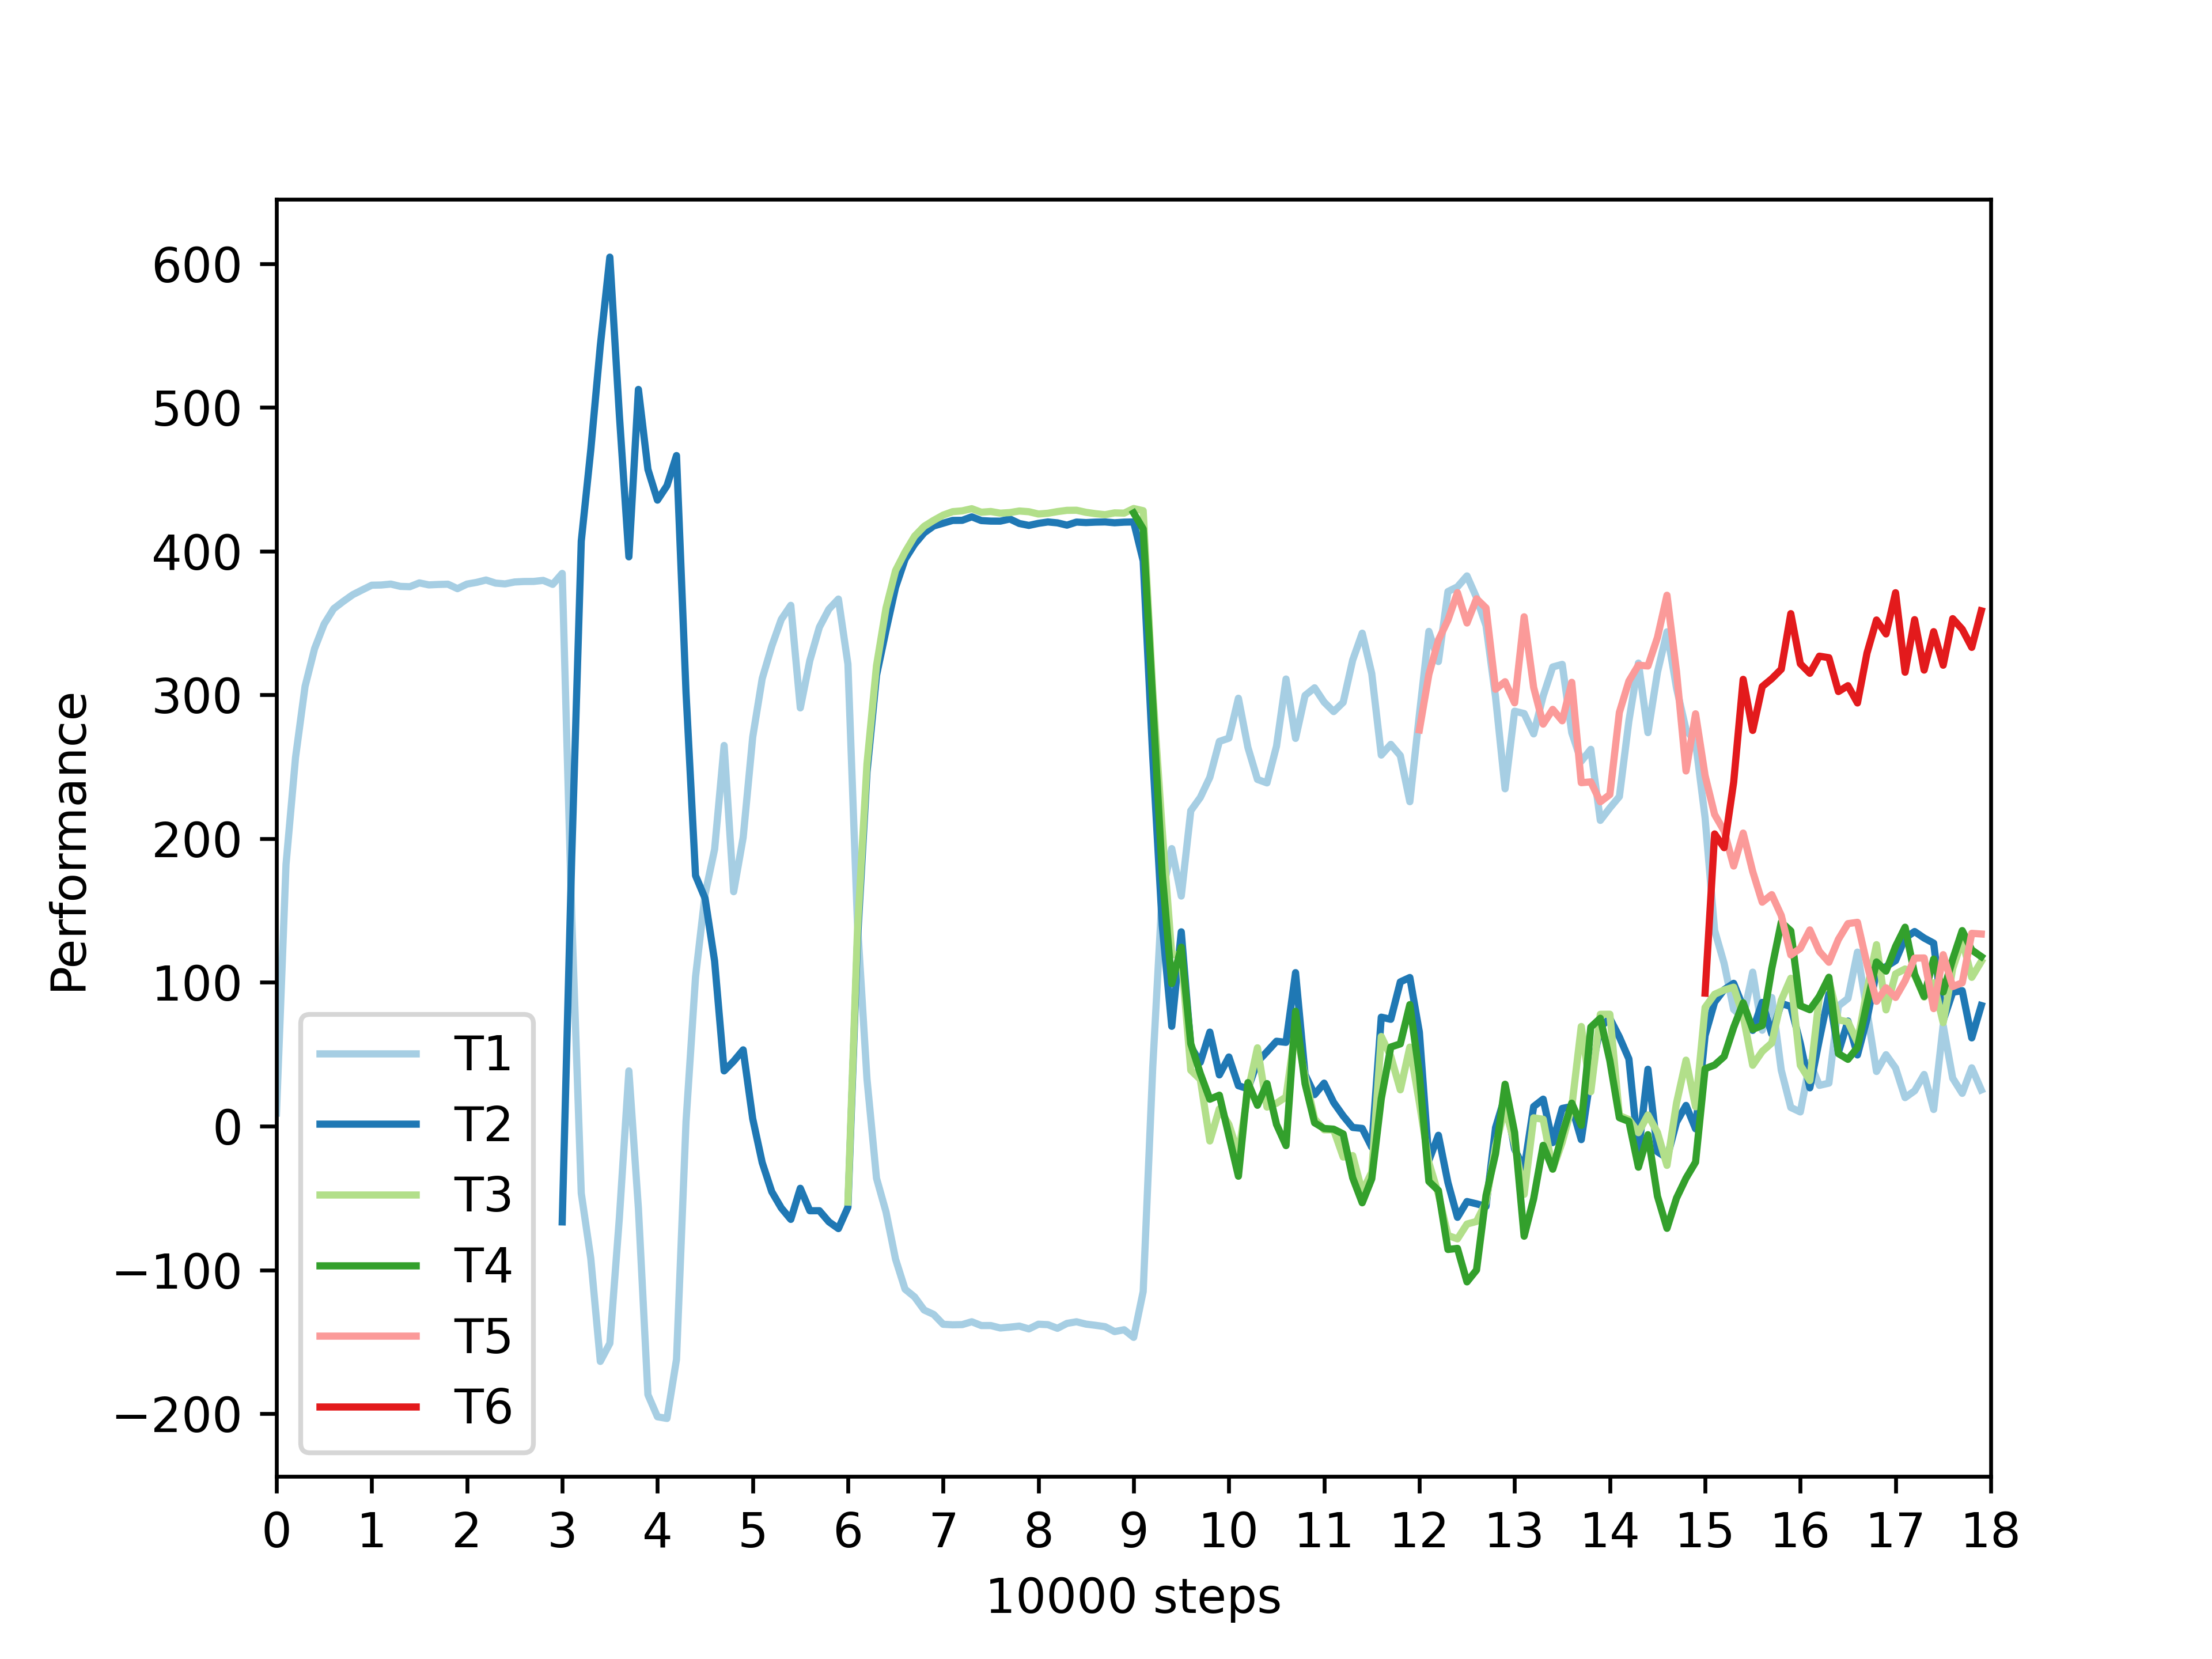}}
	
     \centering	
     \subcaptionbox{Vanilla DT}
    {\includegraphics[width=0.245\linewidth]{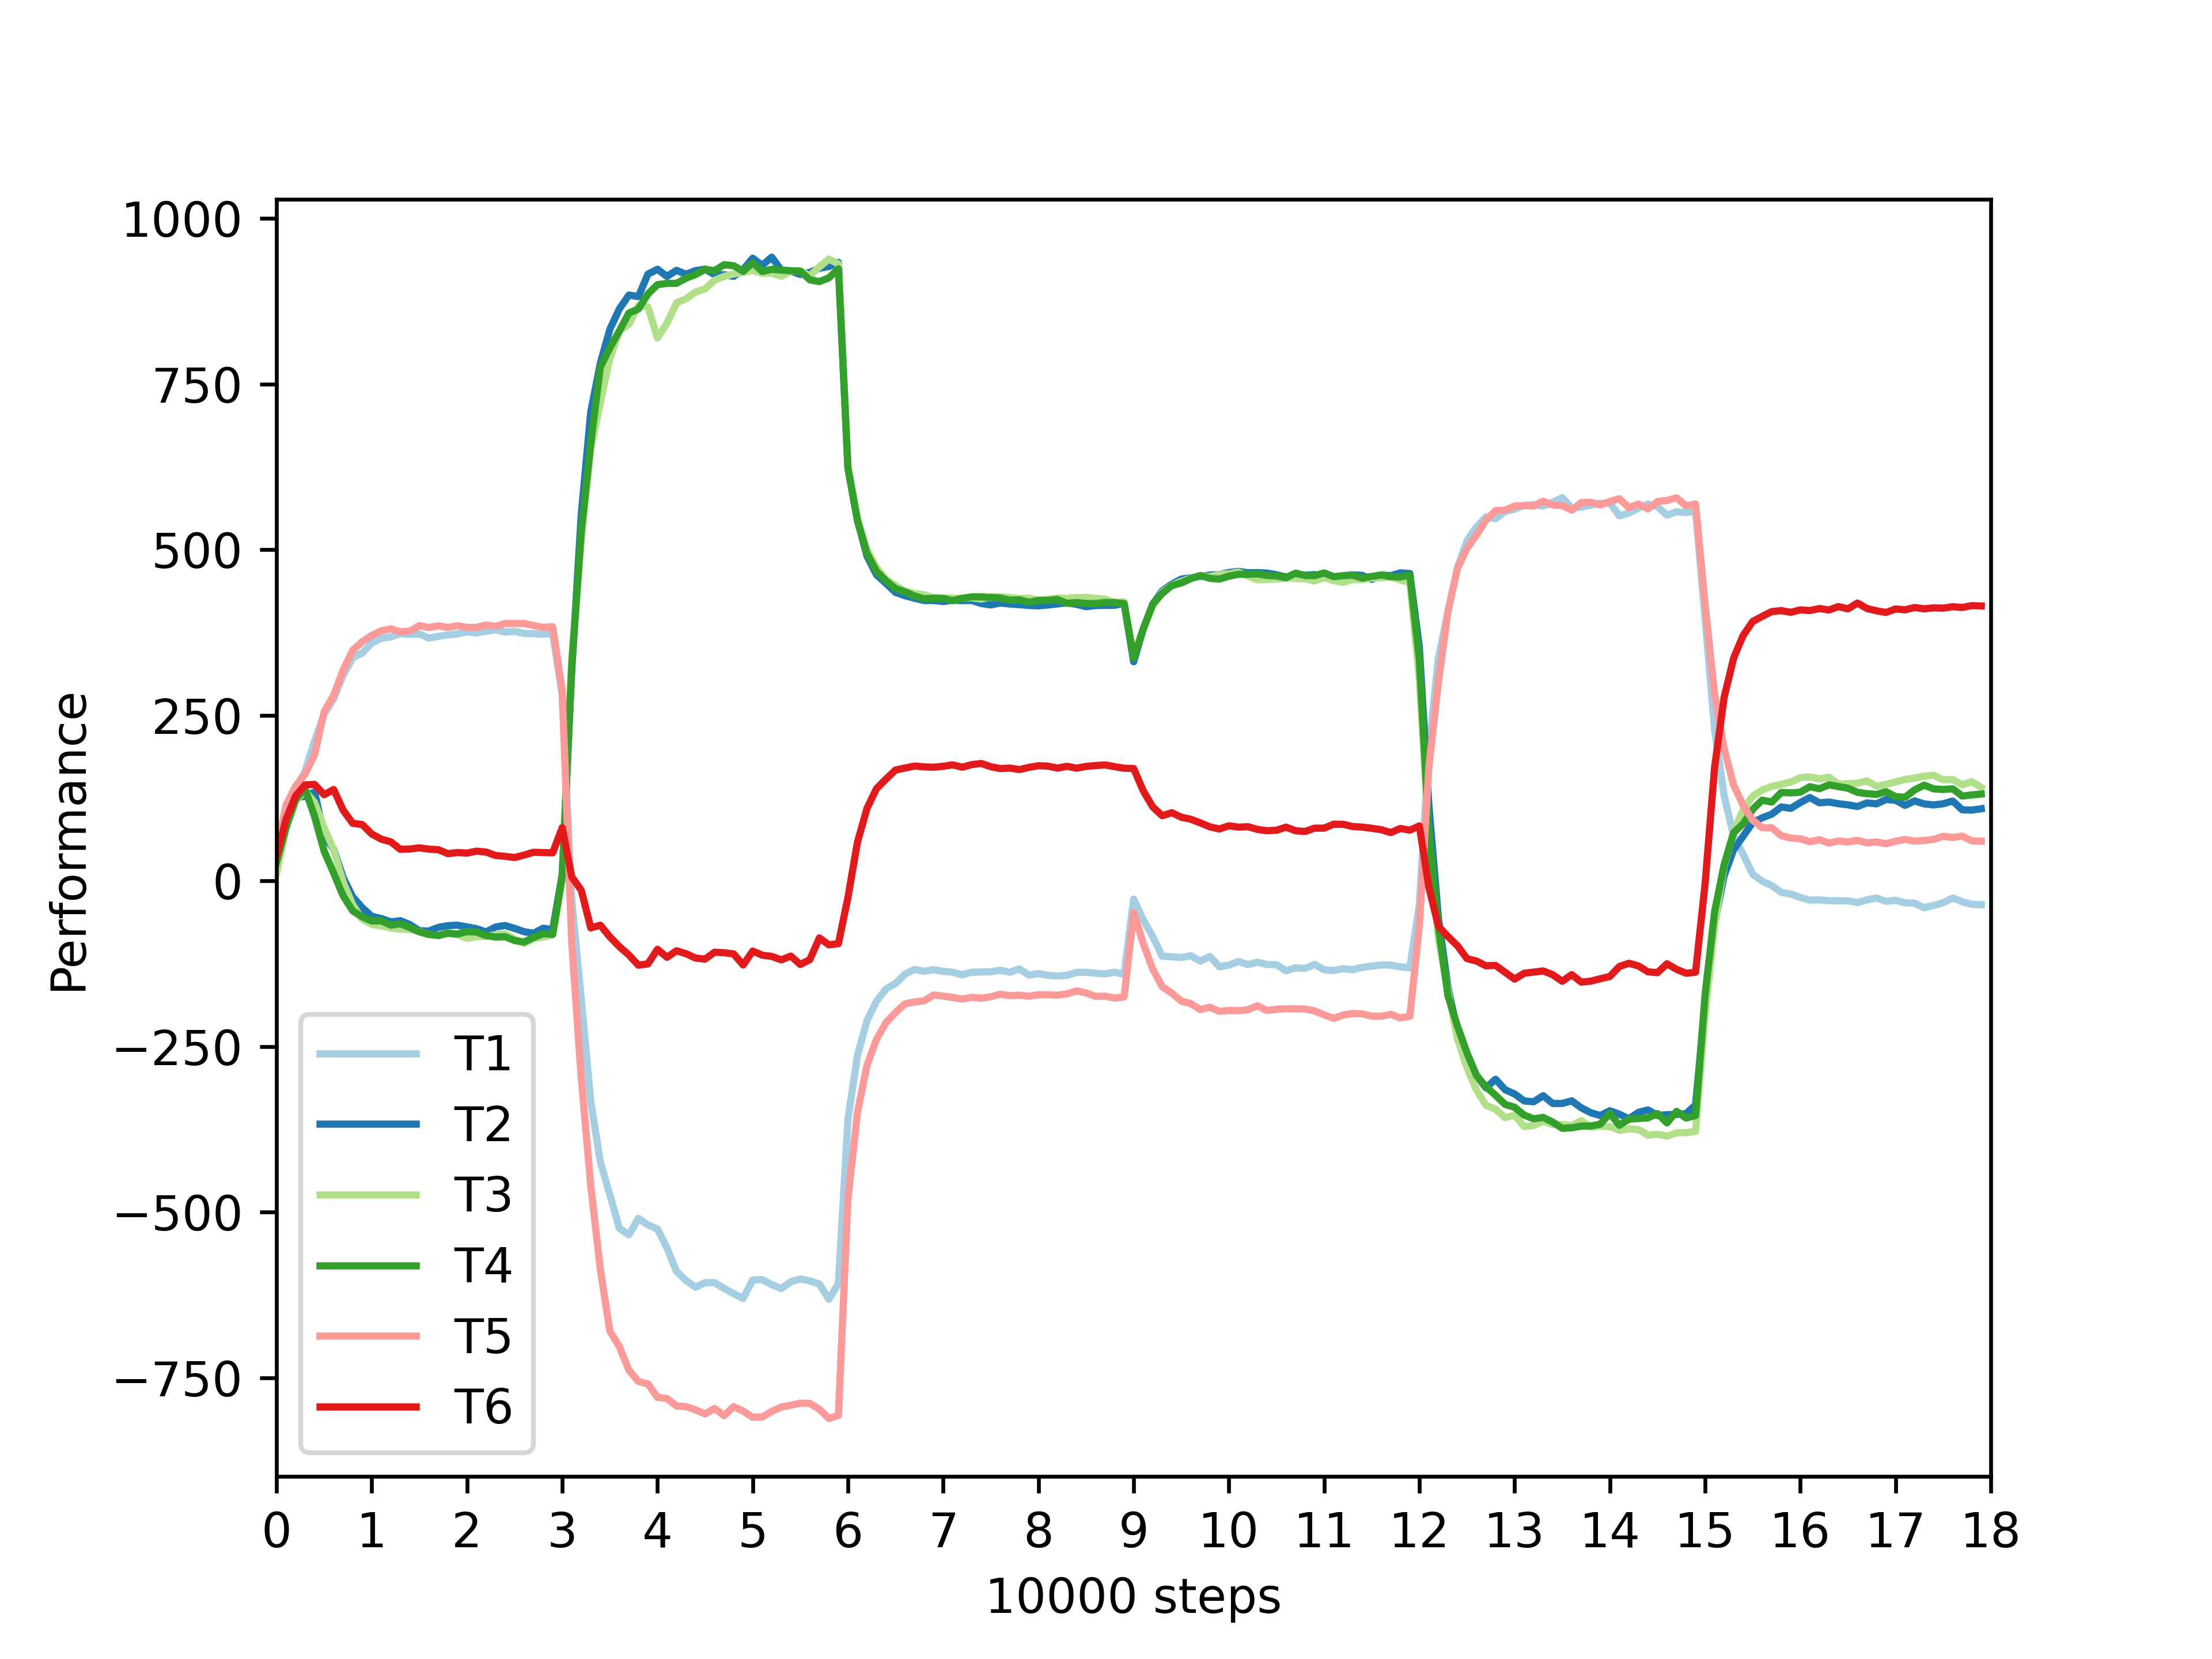}}
        \subcaptionbox{OER}
    {\includegraphics[width=0.245\linewidth]{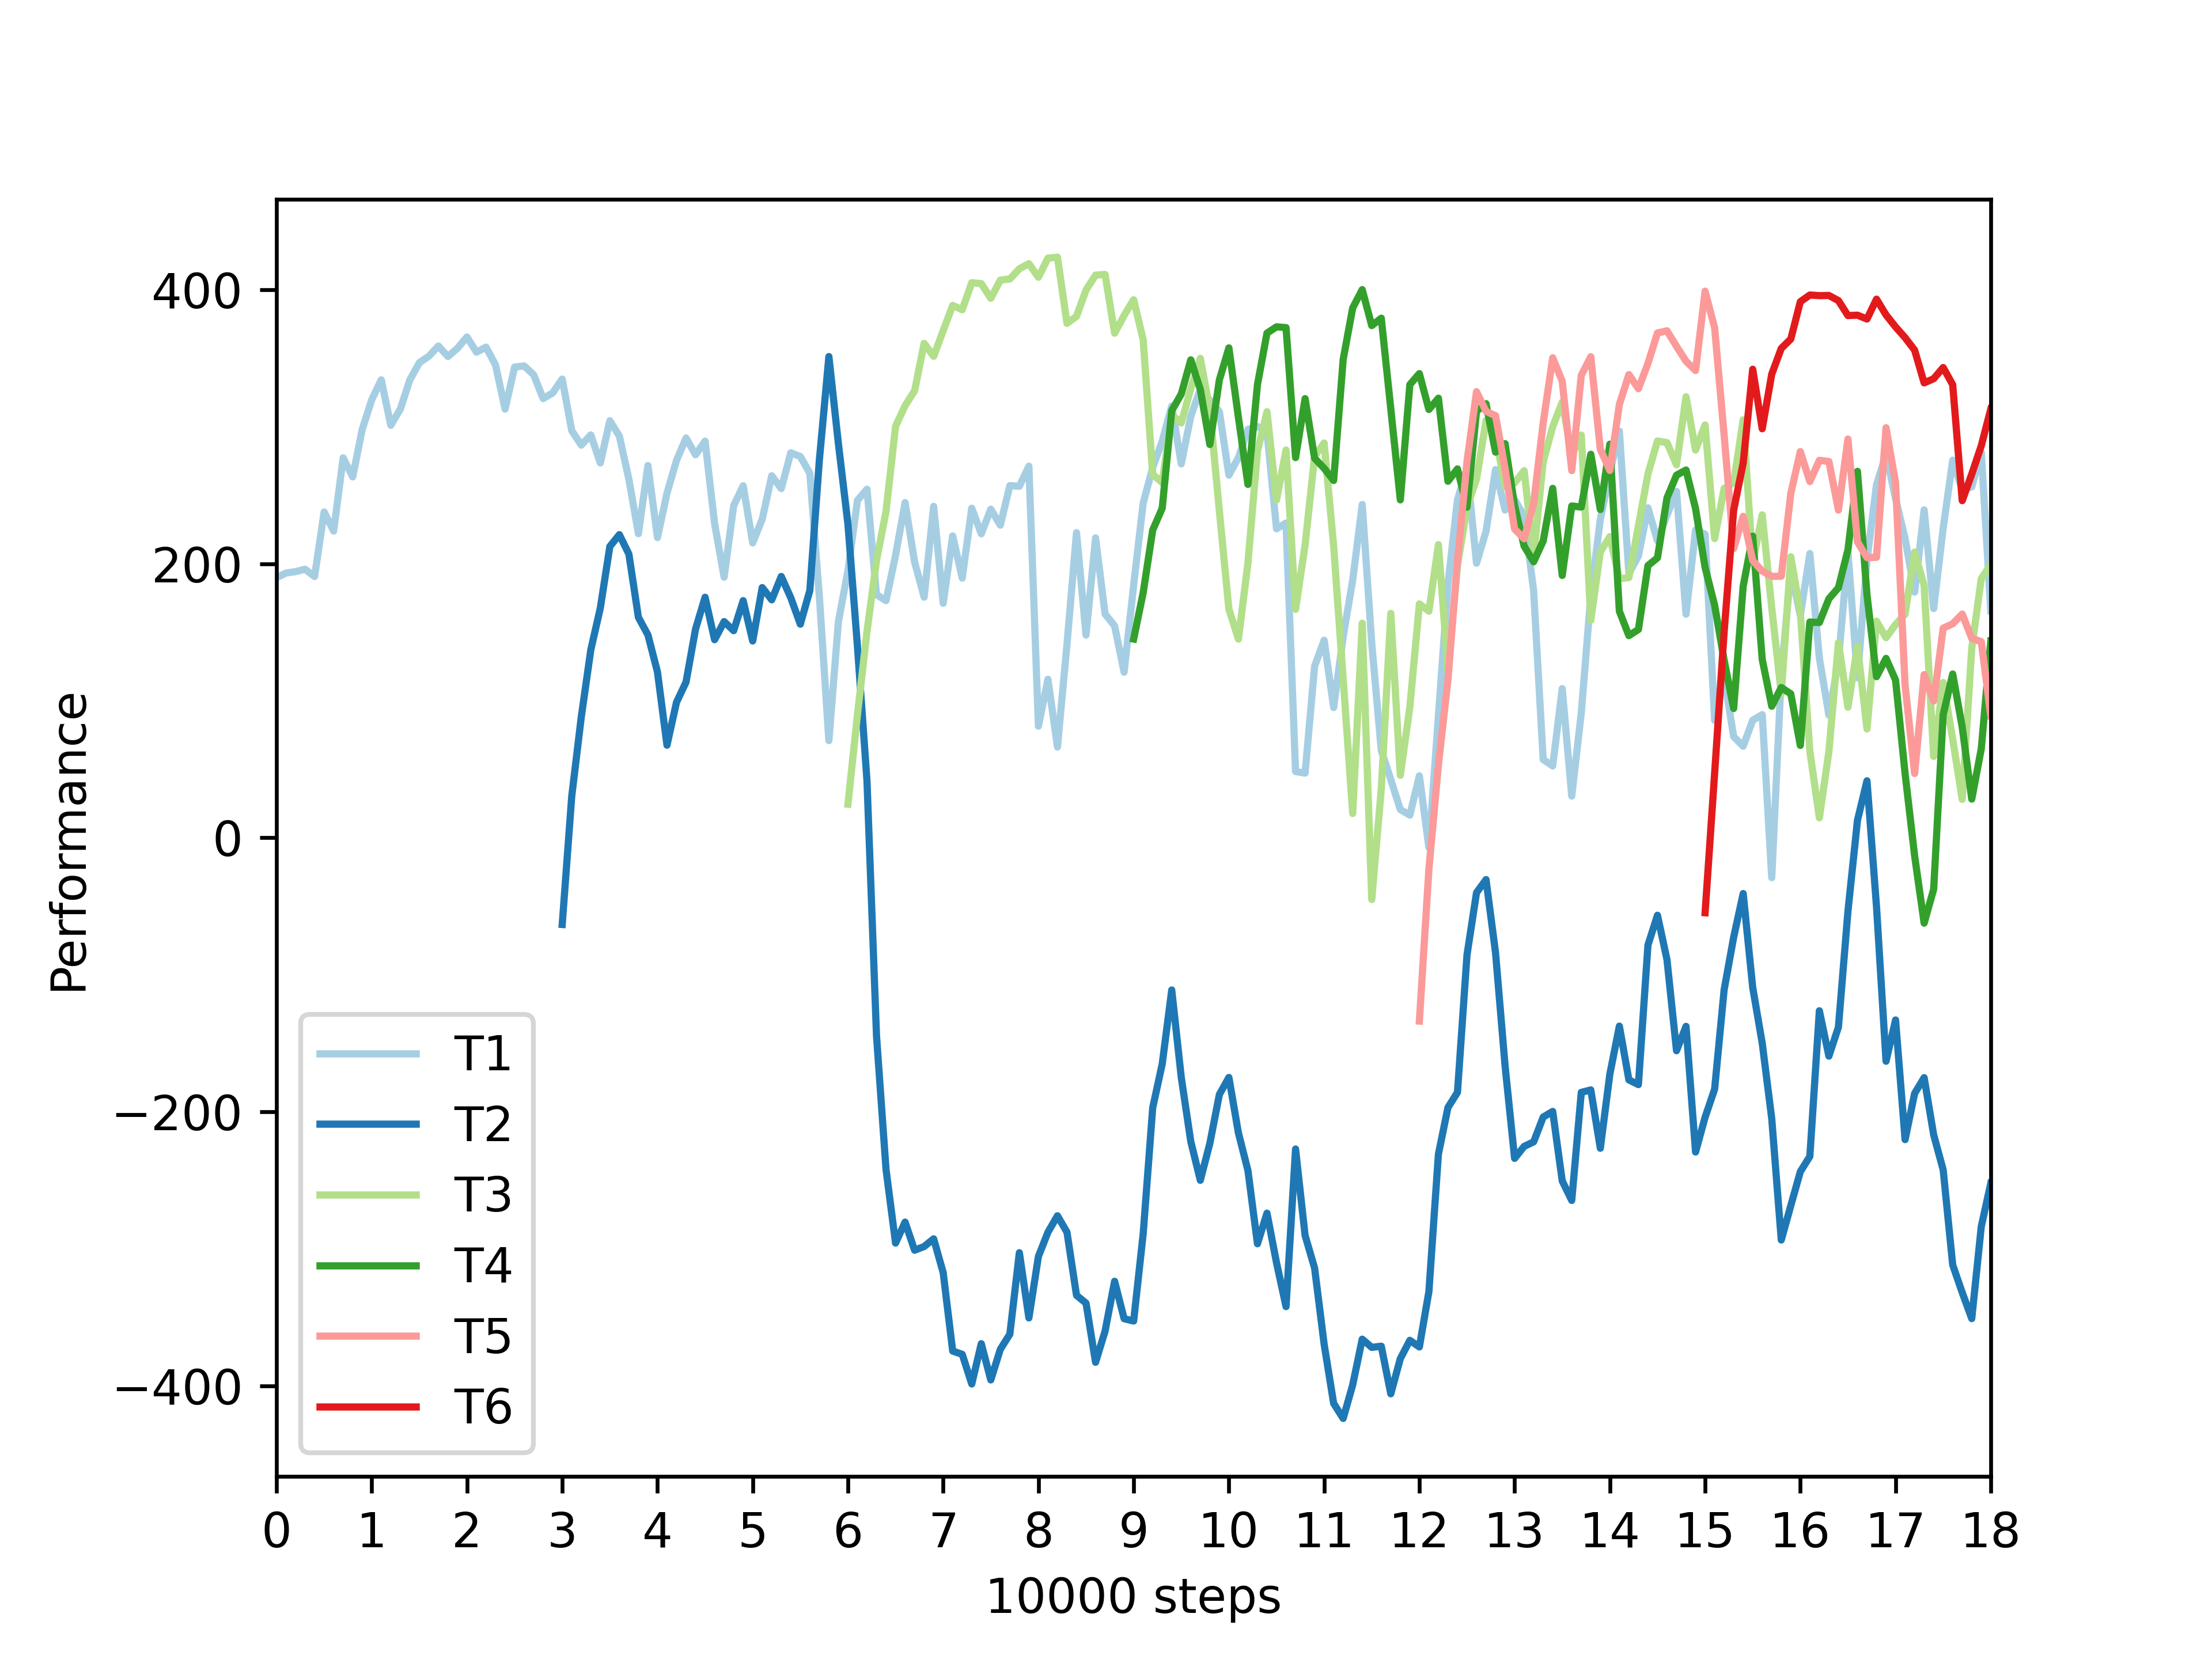}}
    \subcaptionbox{MH-DT}
    {\includegraphics[width=0.245\linewidth]{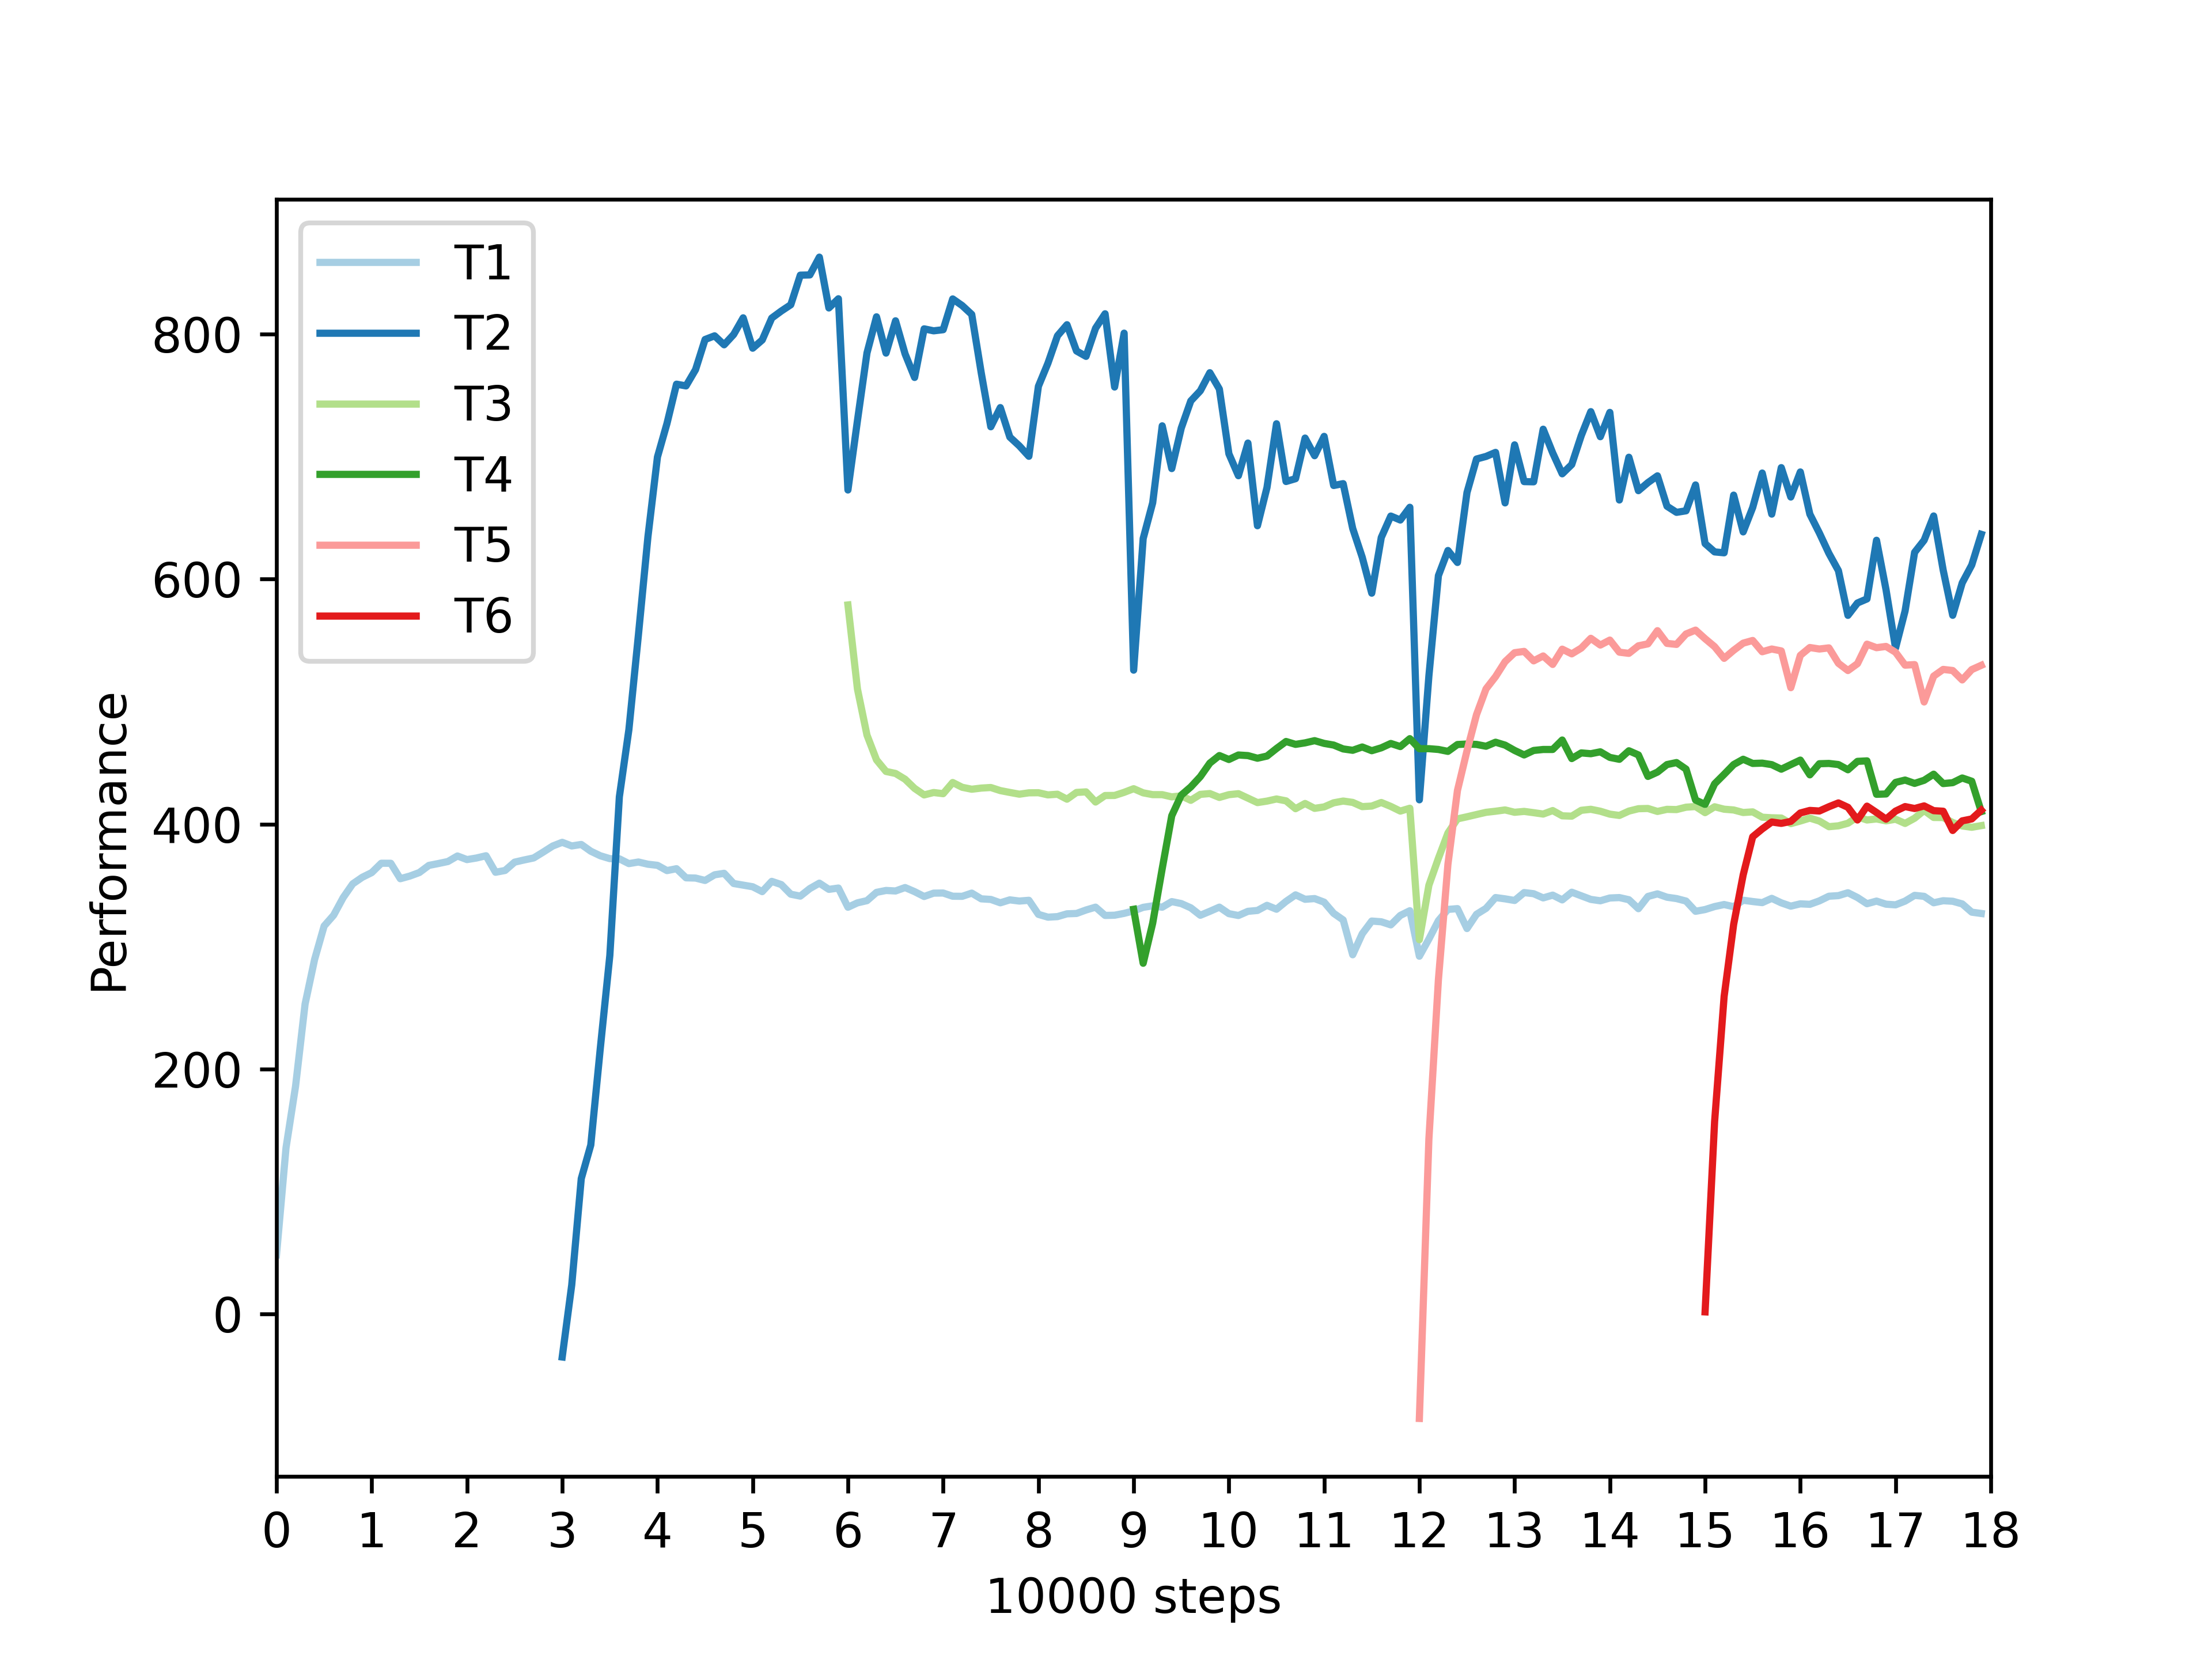}}
	\subcaptionbox{LoRA-DT}
    {\includegraphics[width=0.245\linewidth]{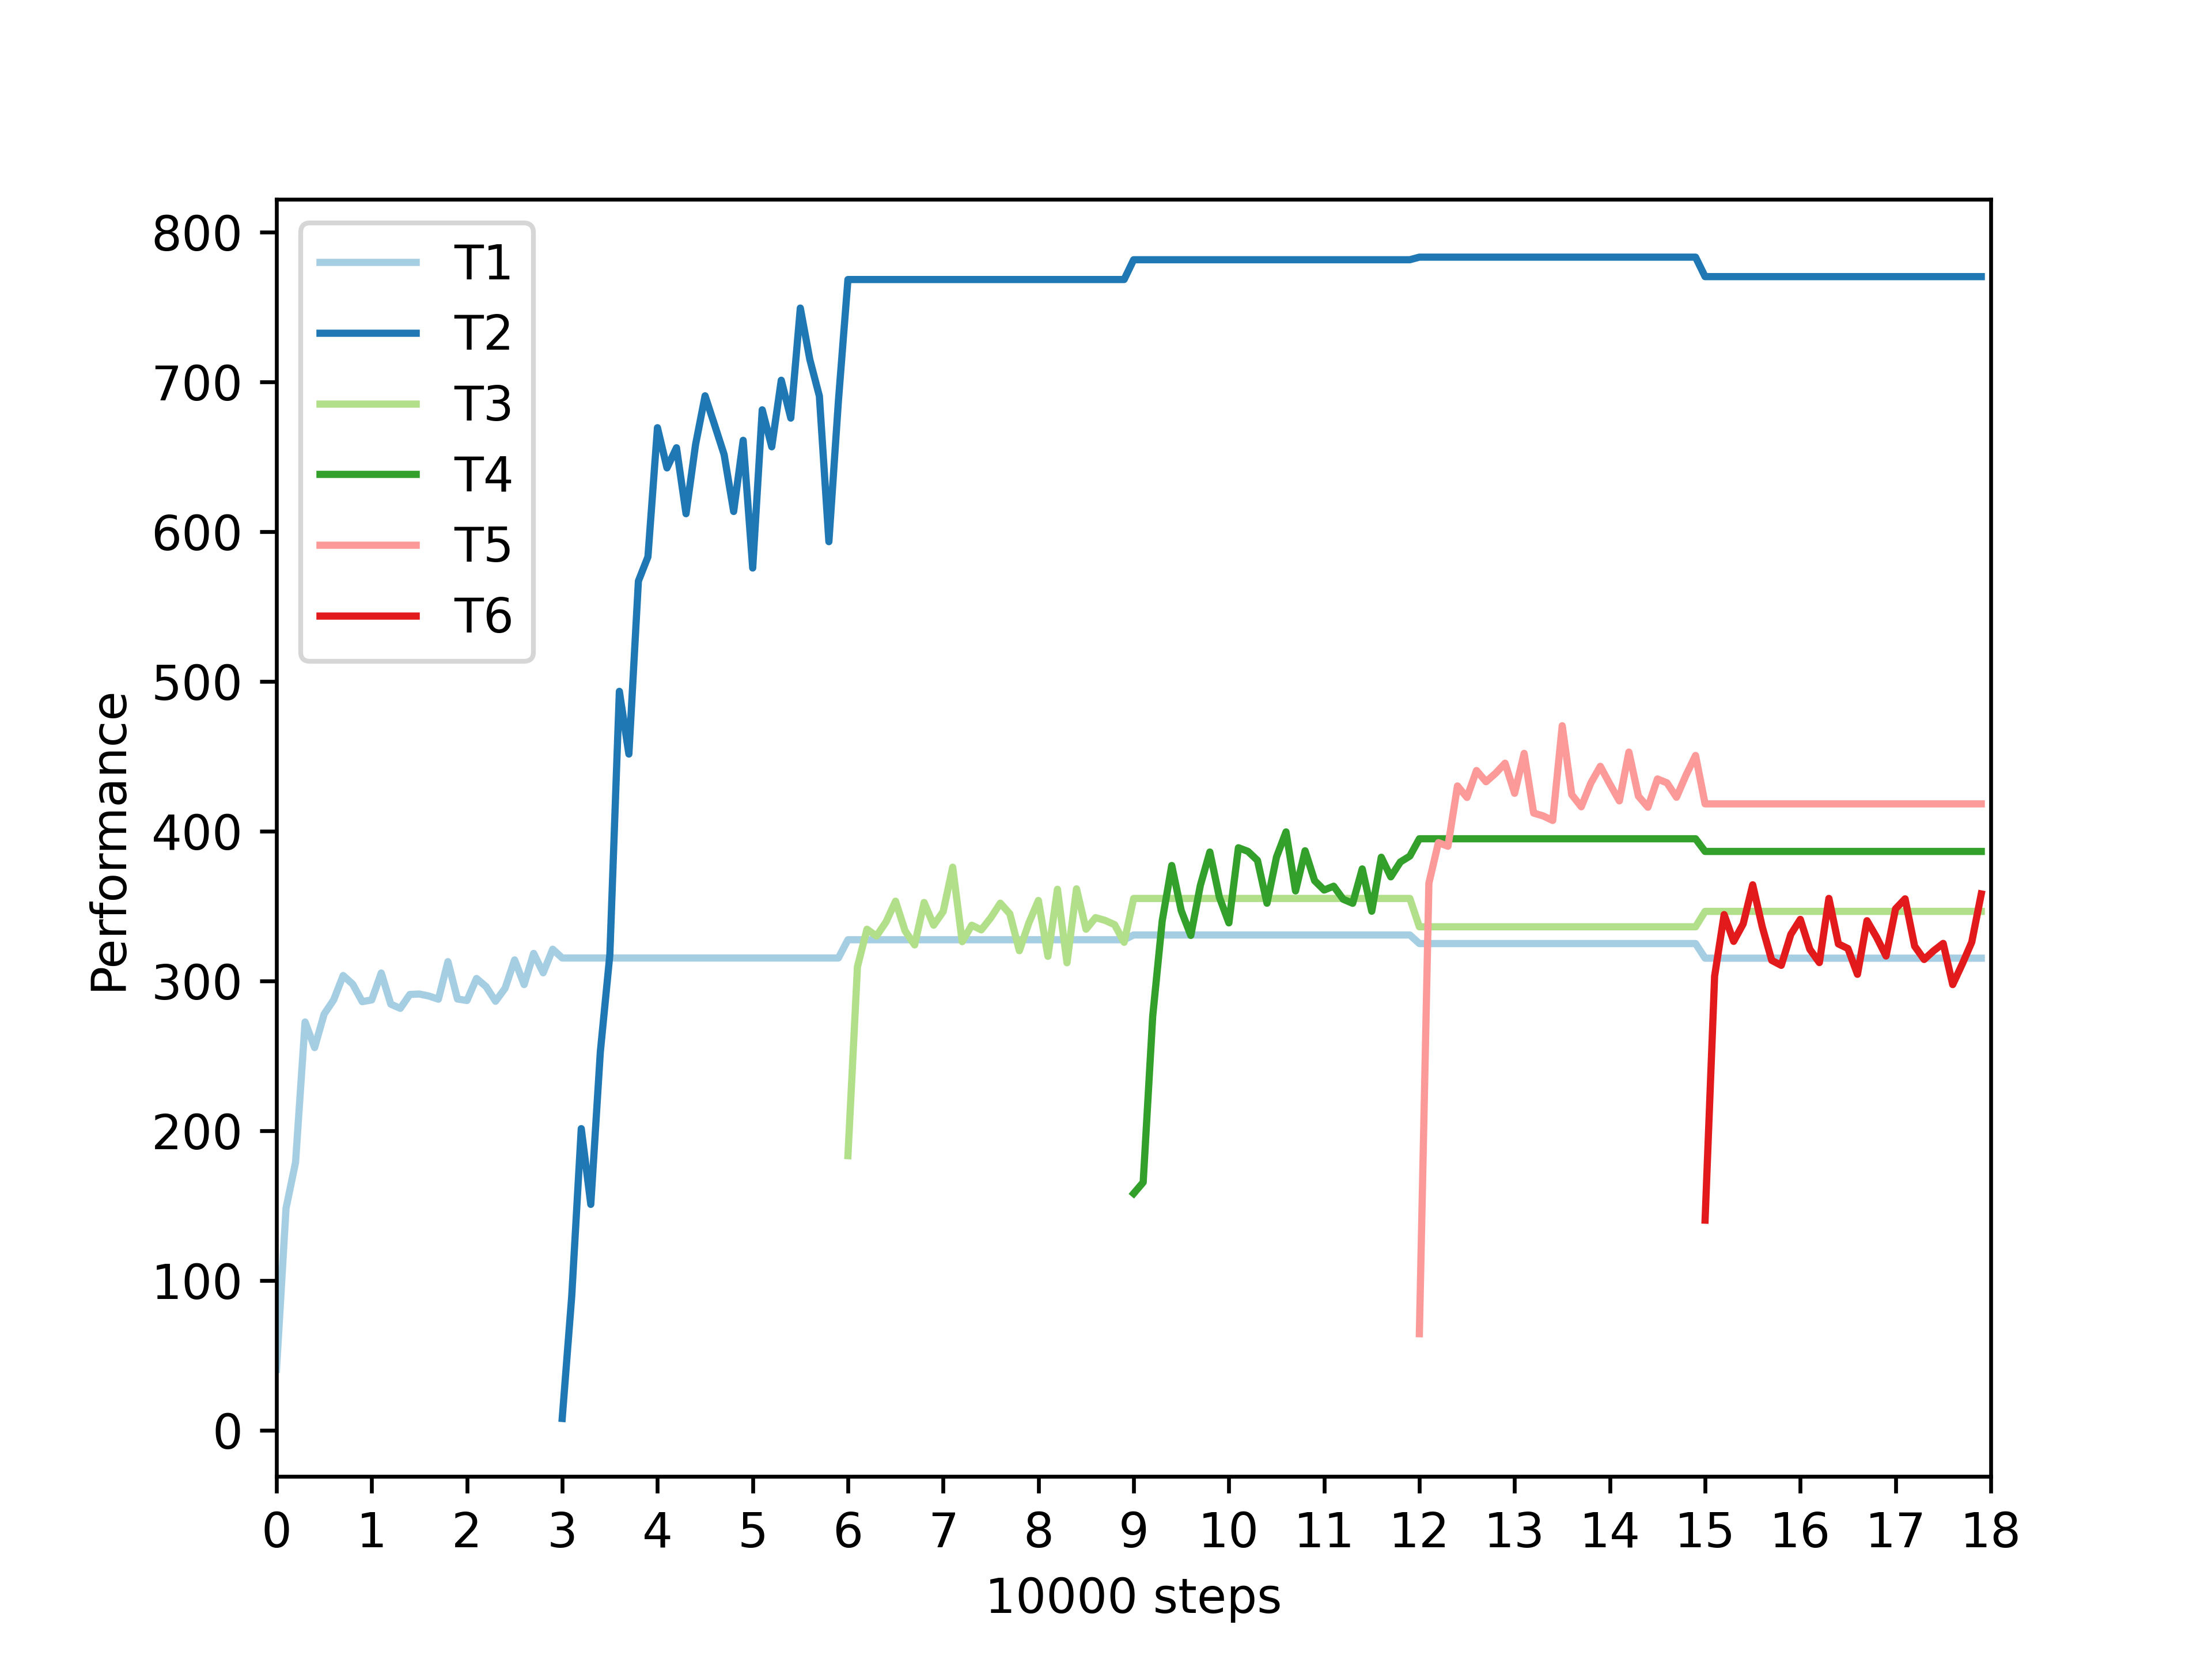}}
    \caption{Ant\_Dir (expert)}
\end{figure}

\begin{figure}[htbp]
	\centering
	\subcaptionbox{PDT}
    {\includegraphics[width=0.245\linewidth]{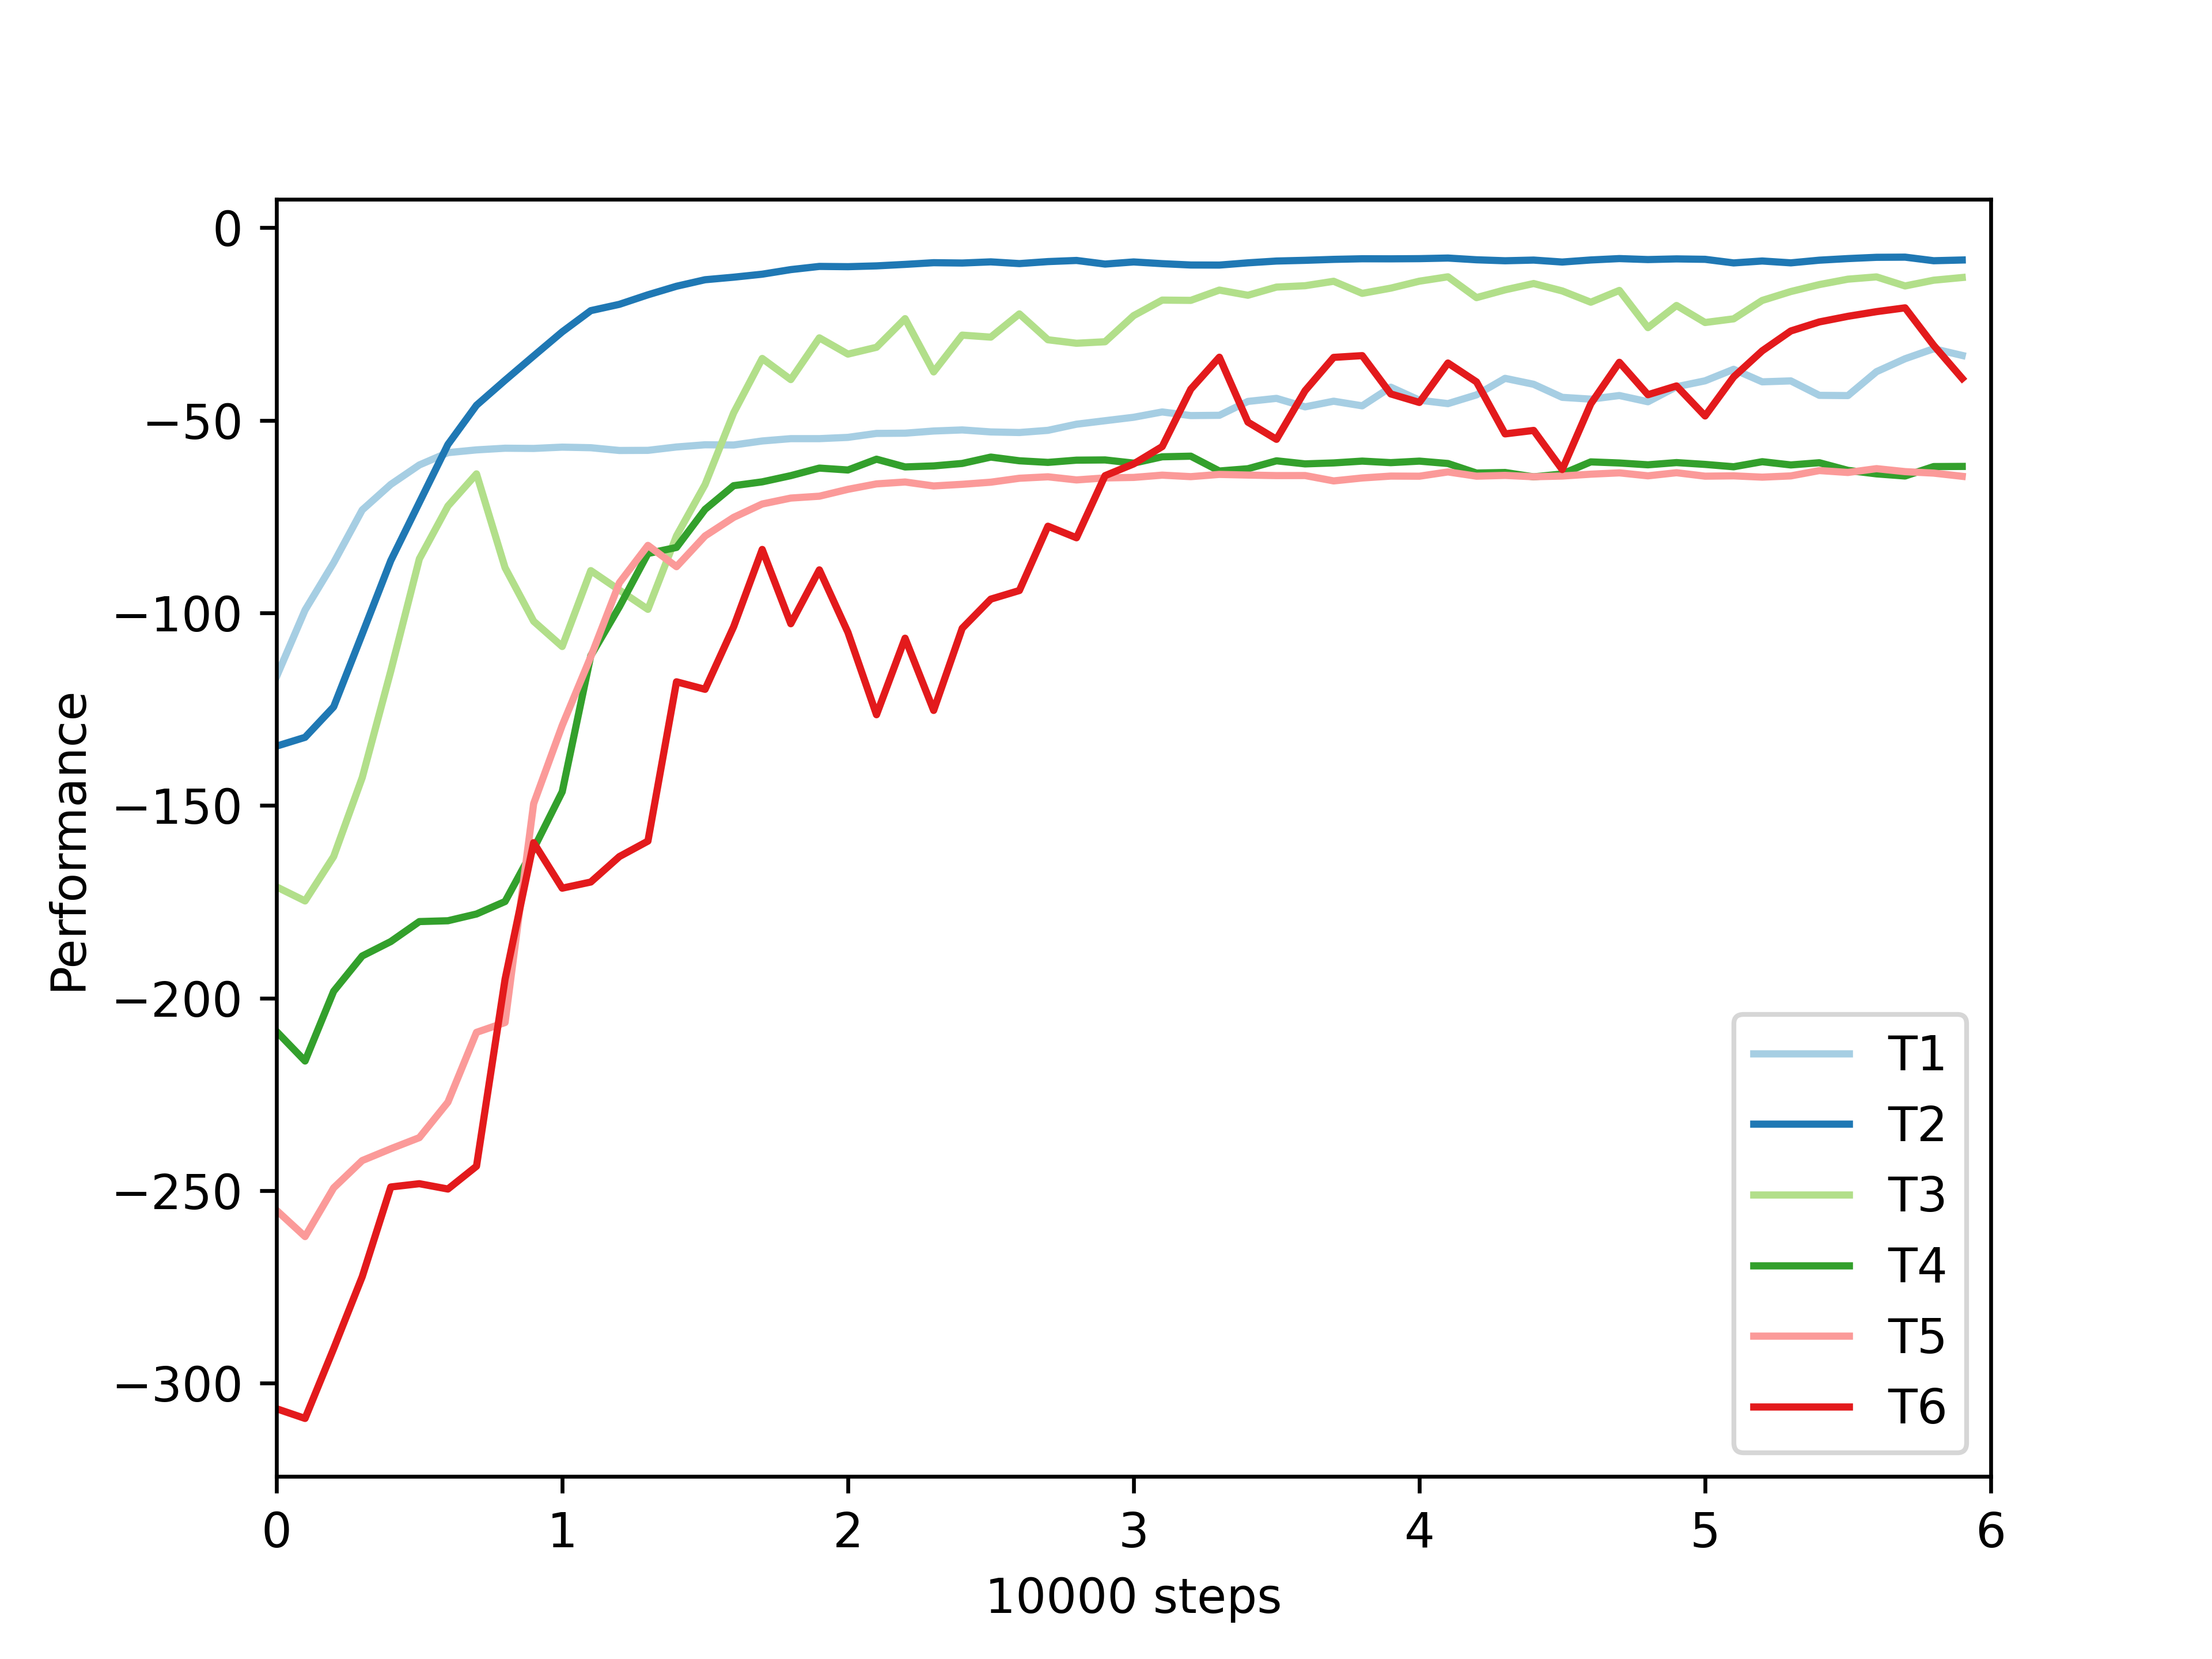}}
	\subcaptionbox{DT + EWC}
    {\includegraphics[width=0.245\linewidth]{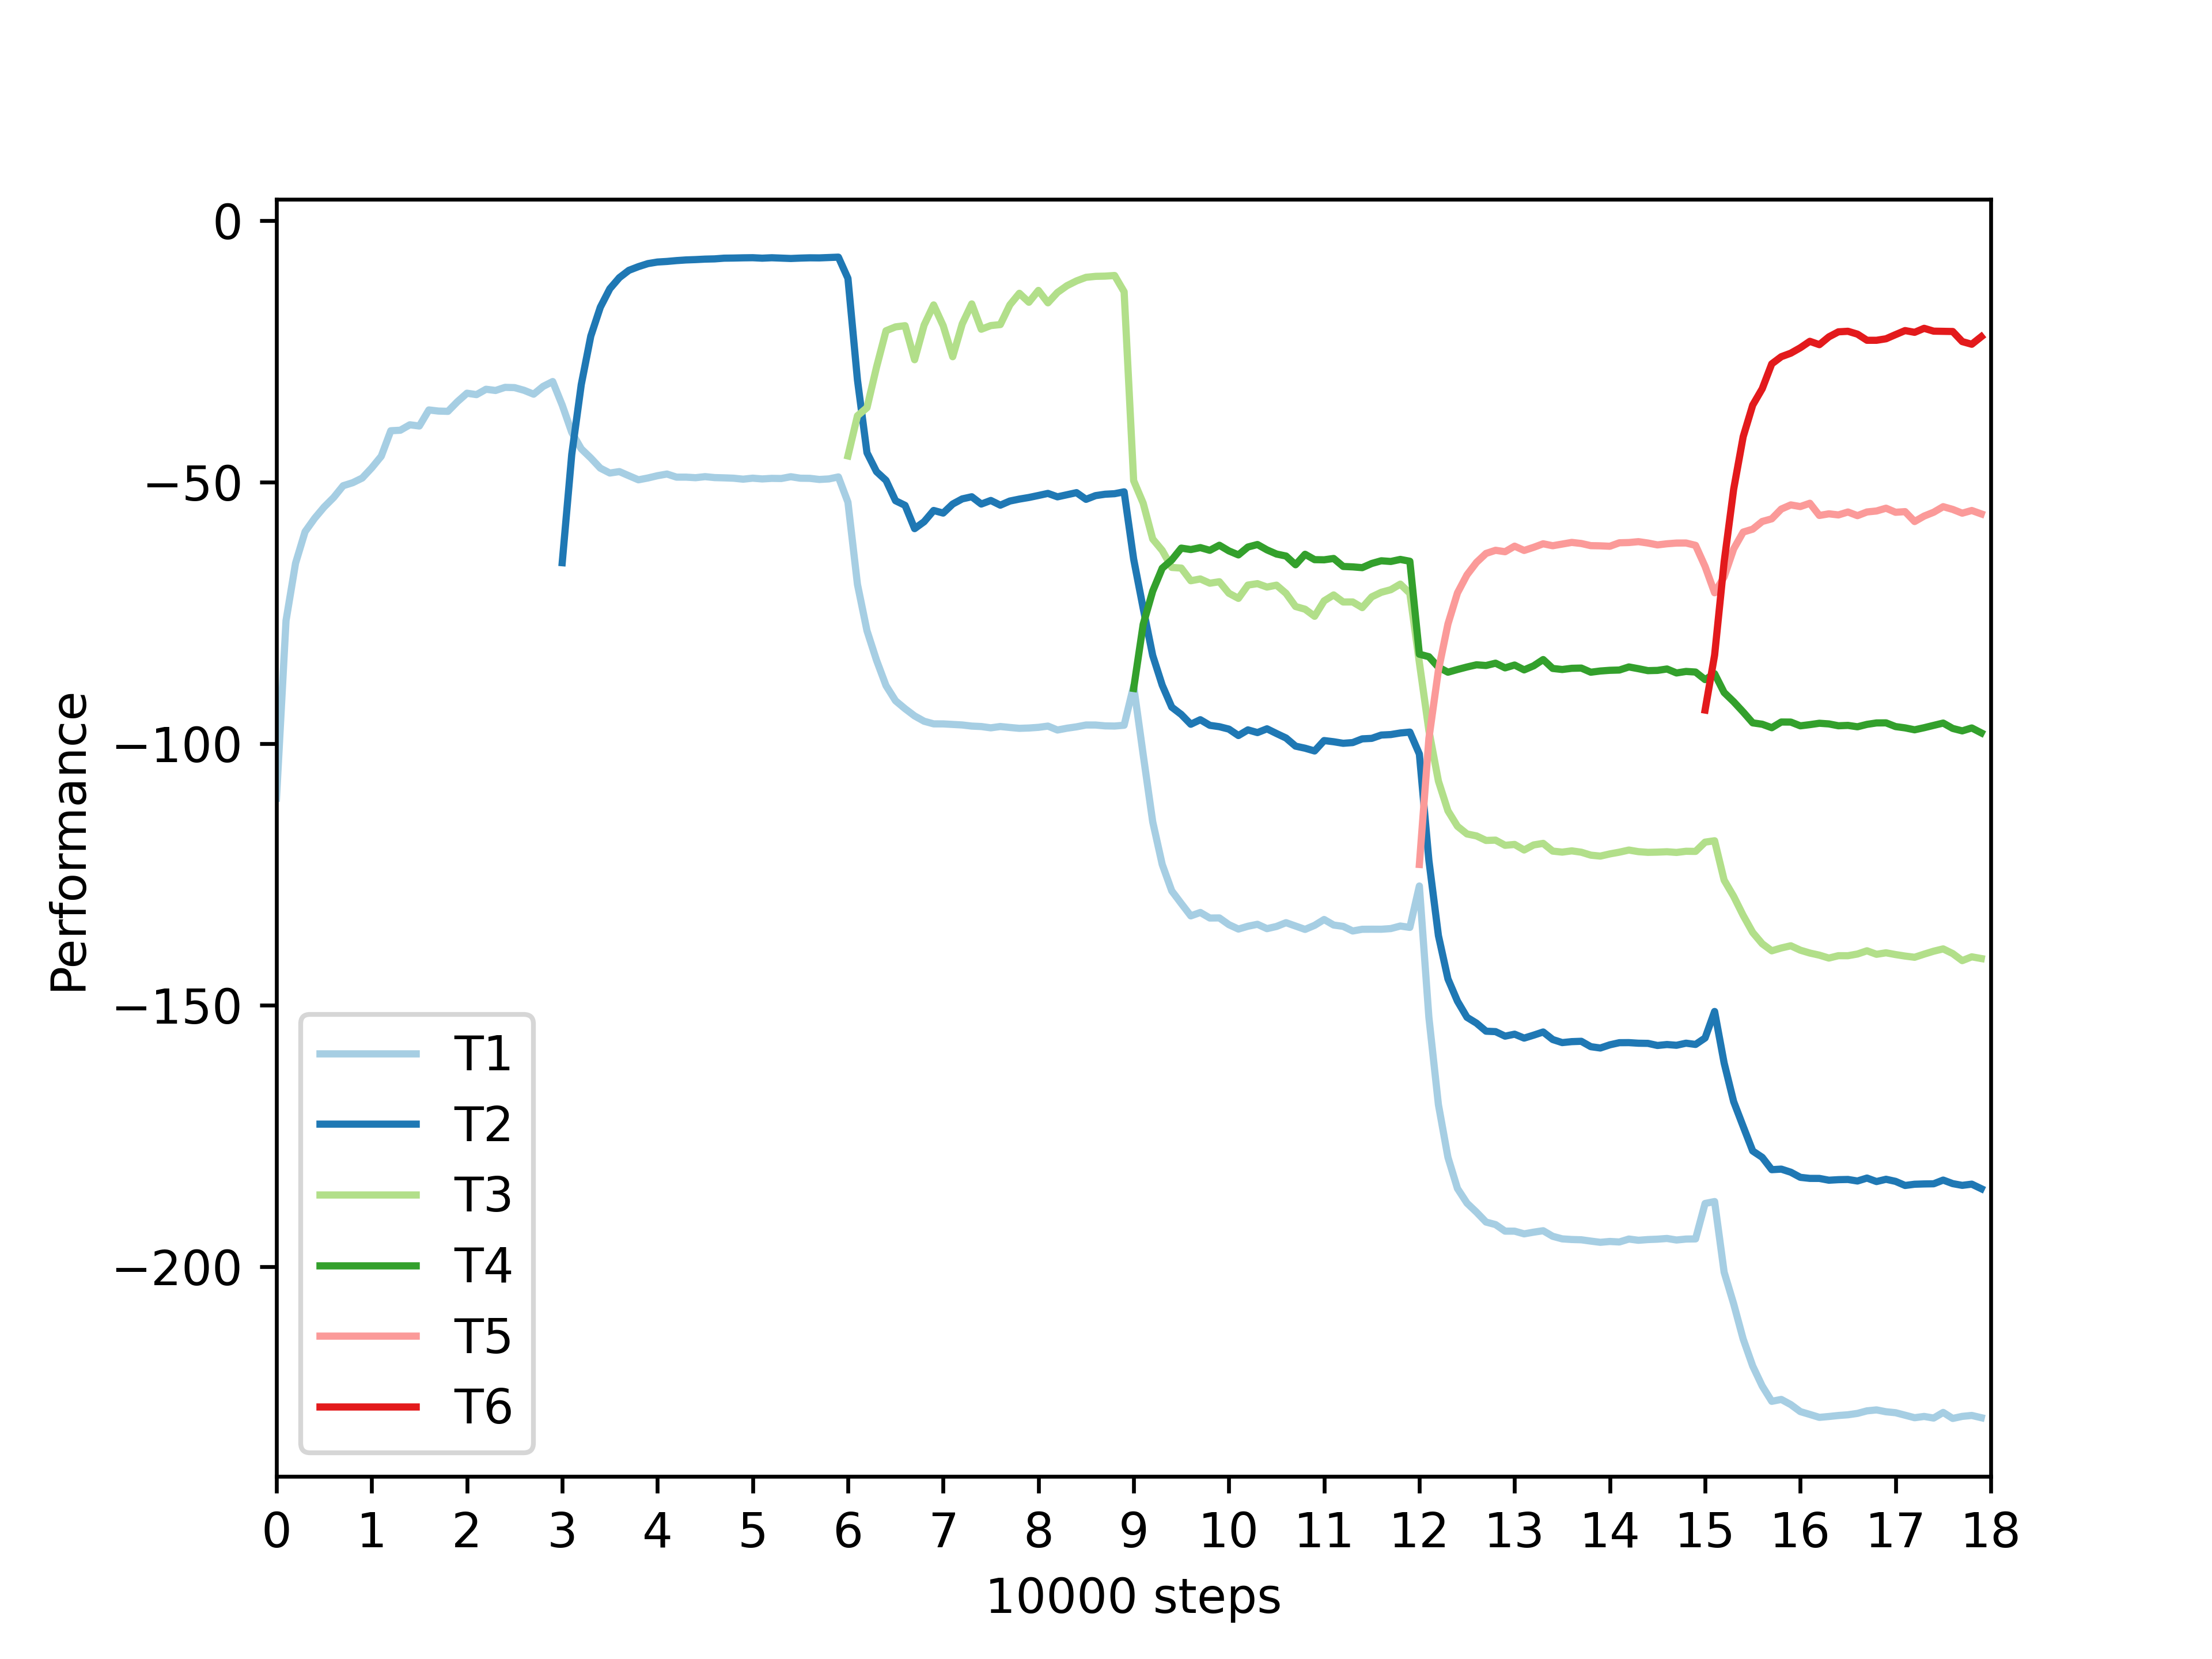}}
    \subcaptionbox{DT + SI}
    {\includegraphics[width=0.245\linewidth]{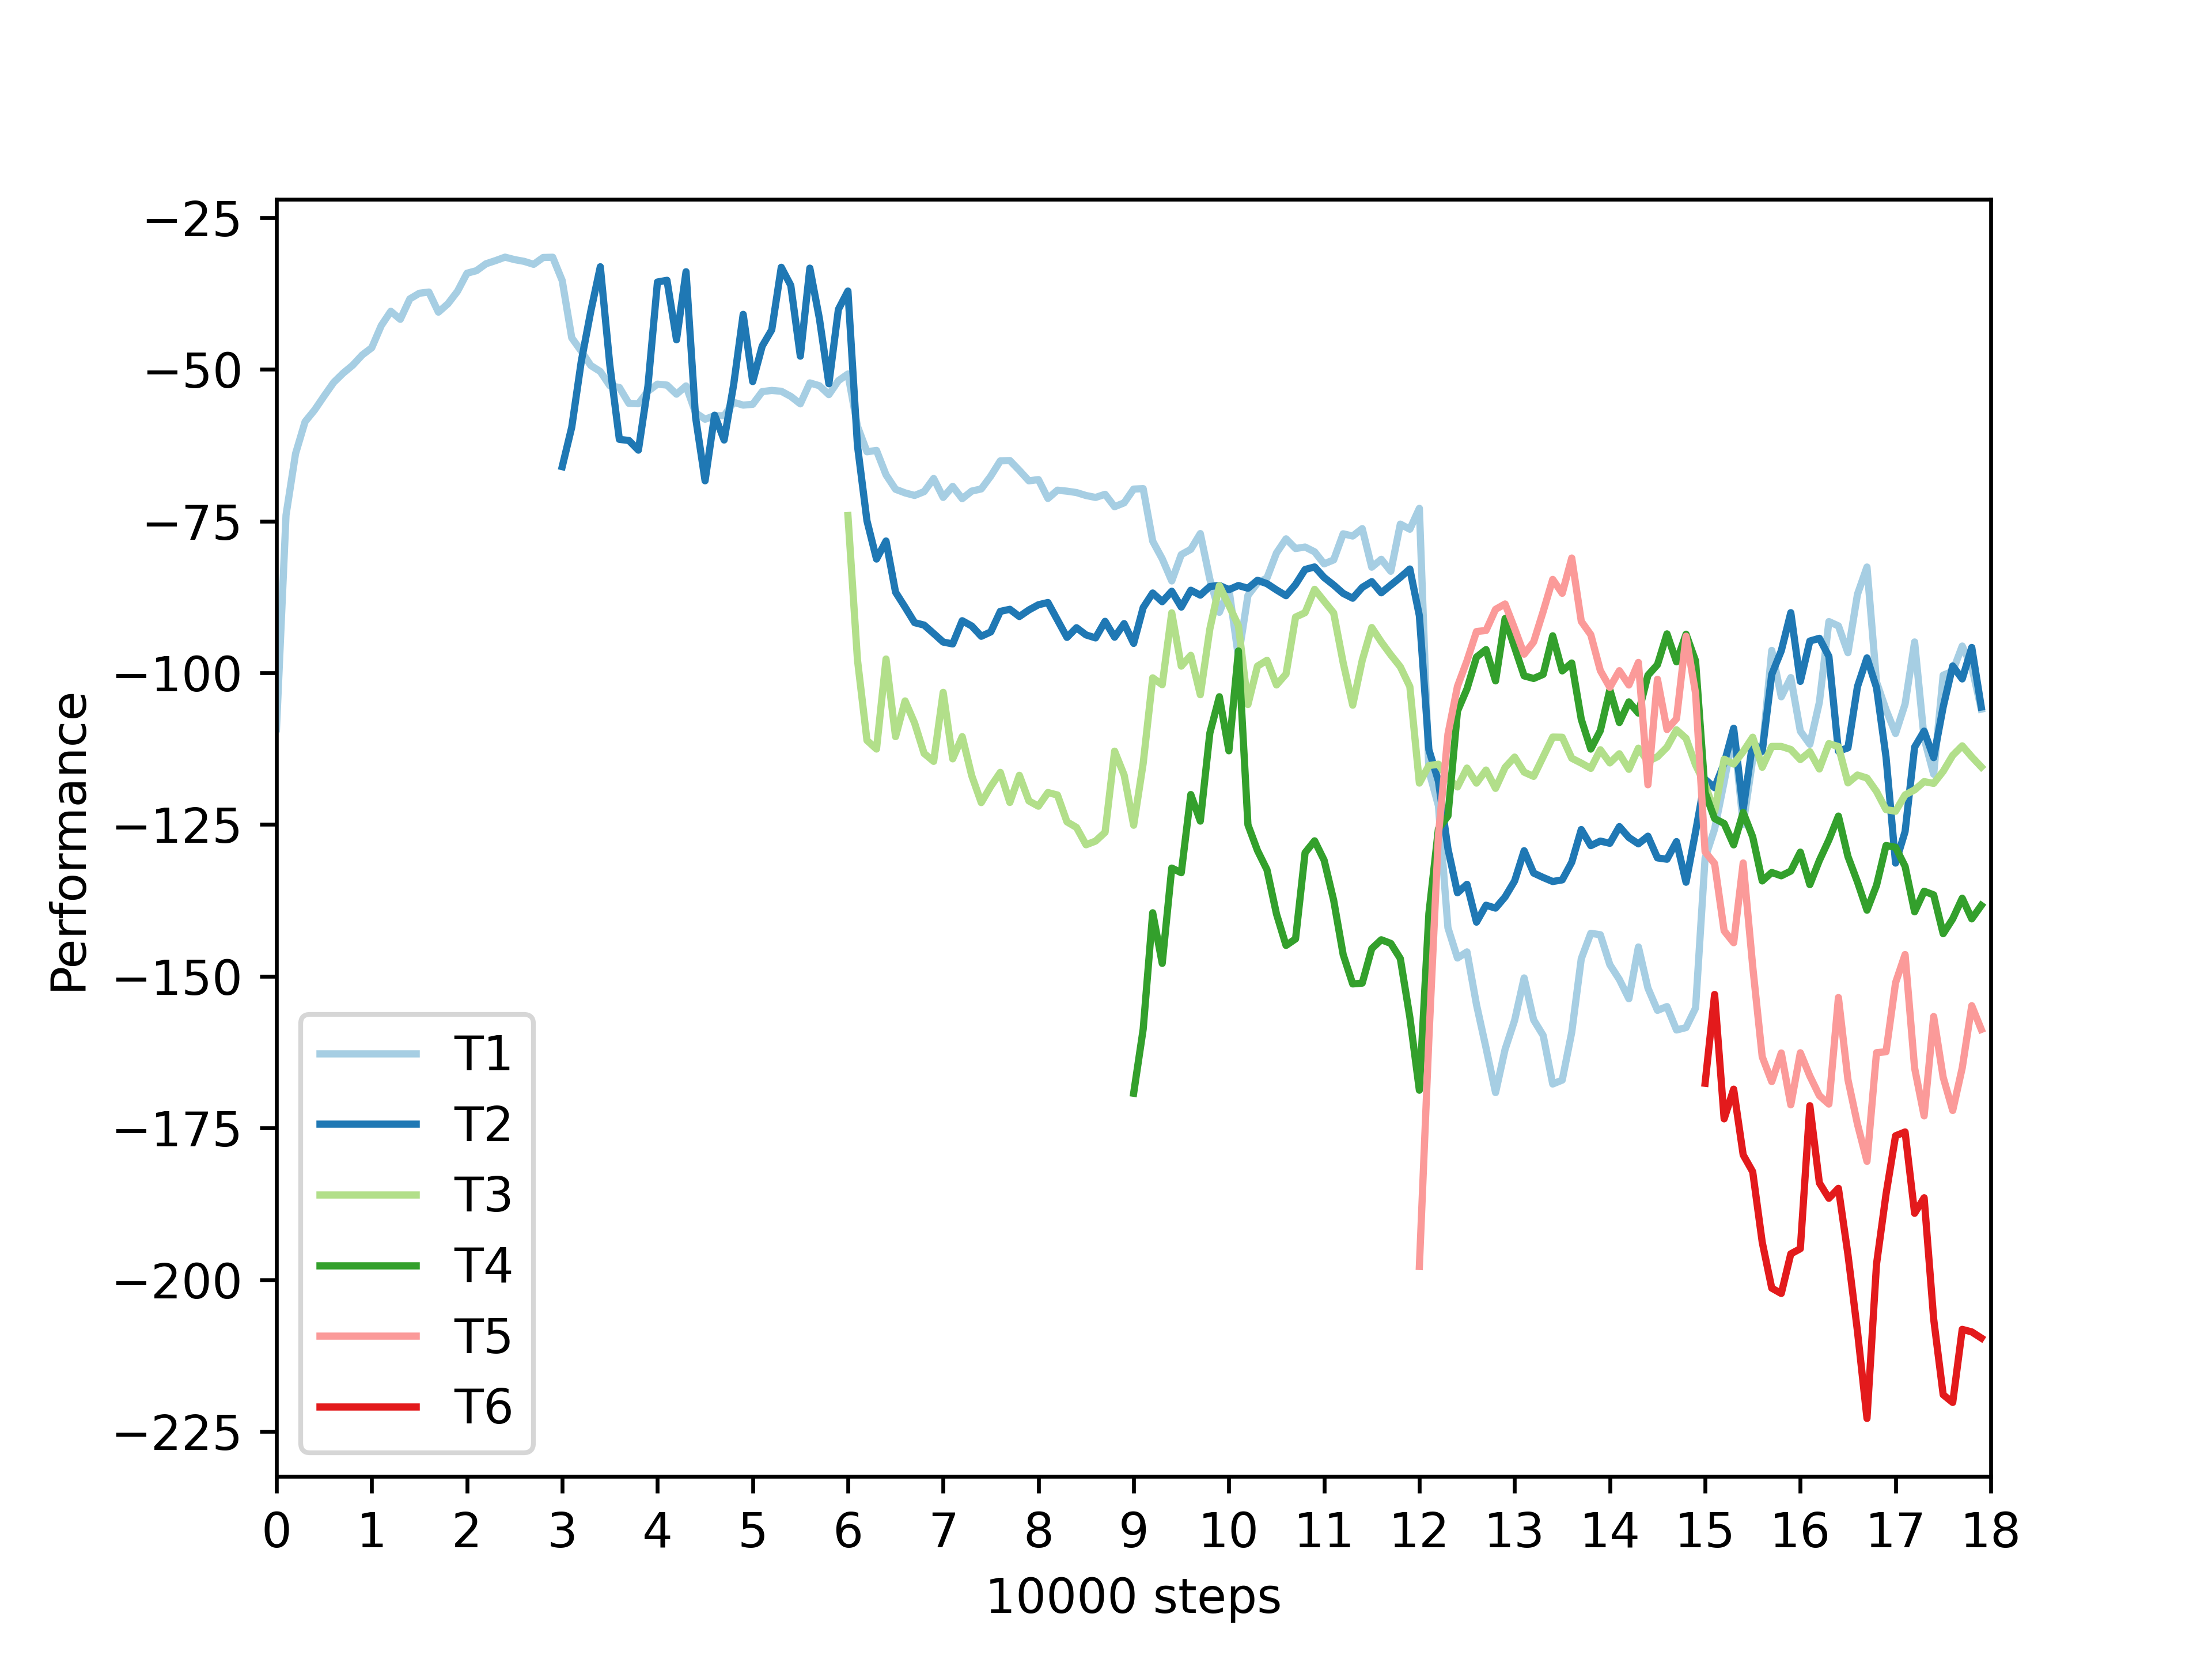}}
    \subcaptionbox{DT + GEM}
    {\includegraphics[width=0.245\linewidth]{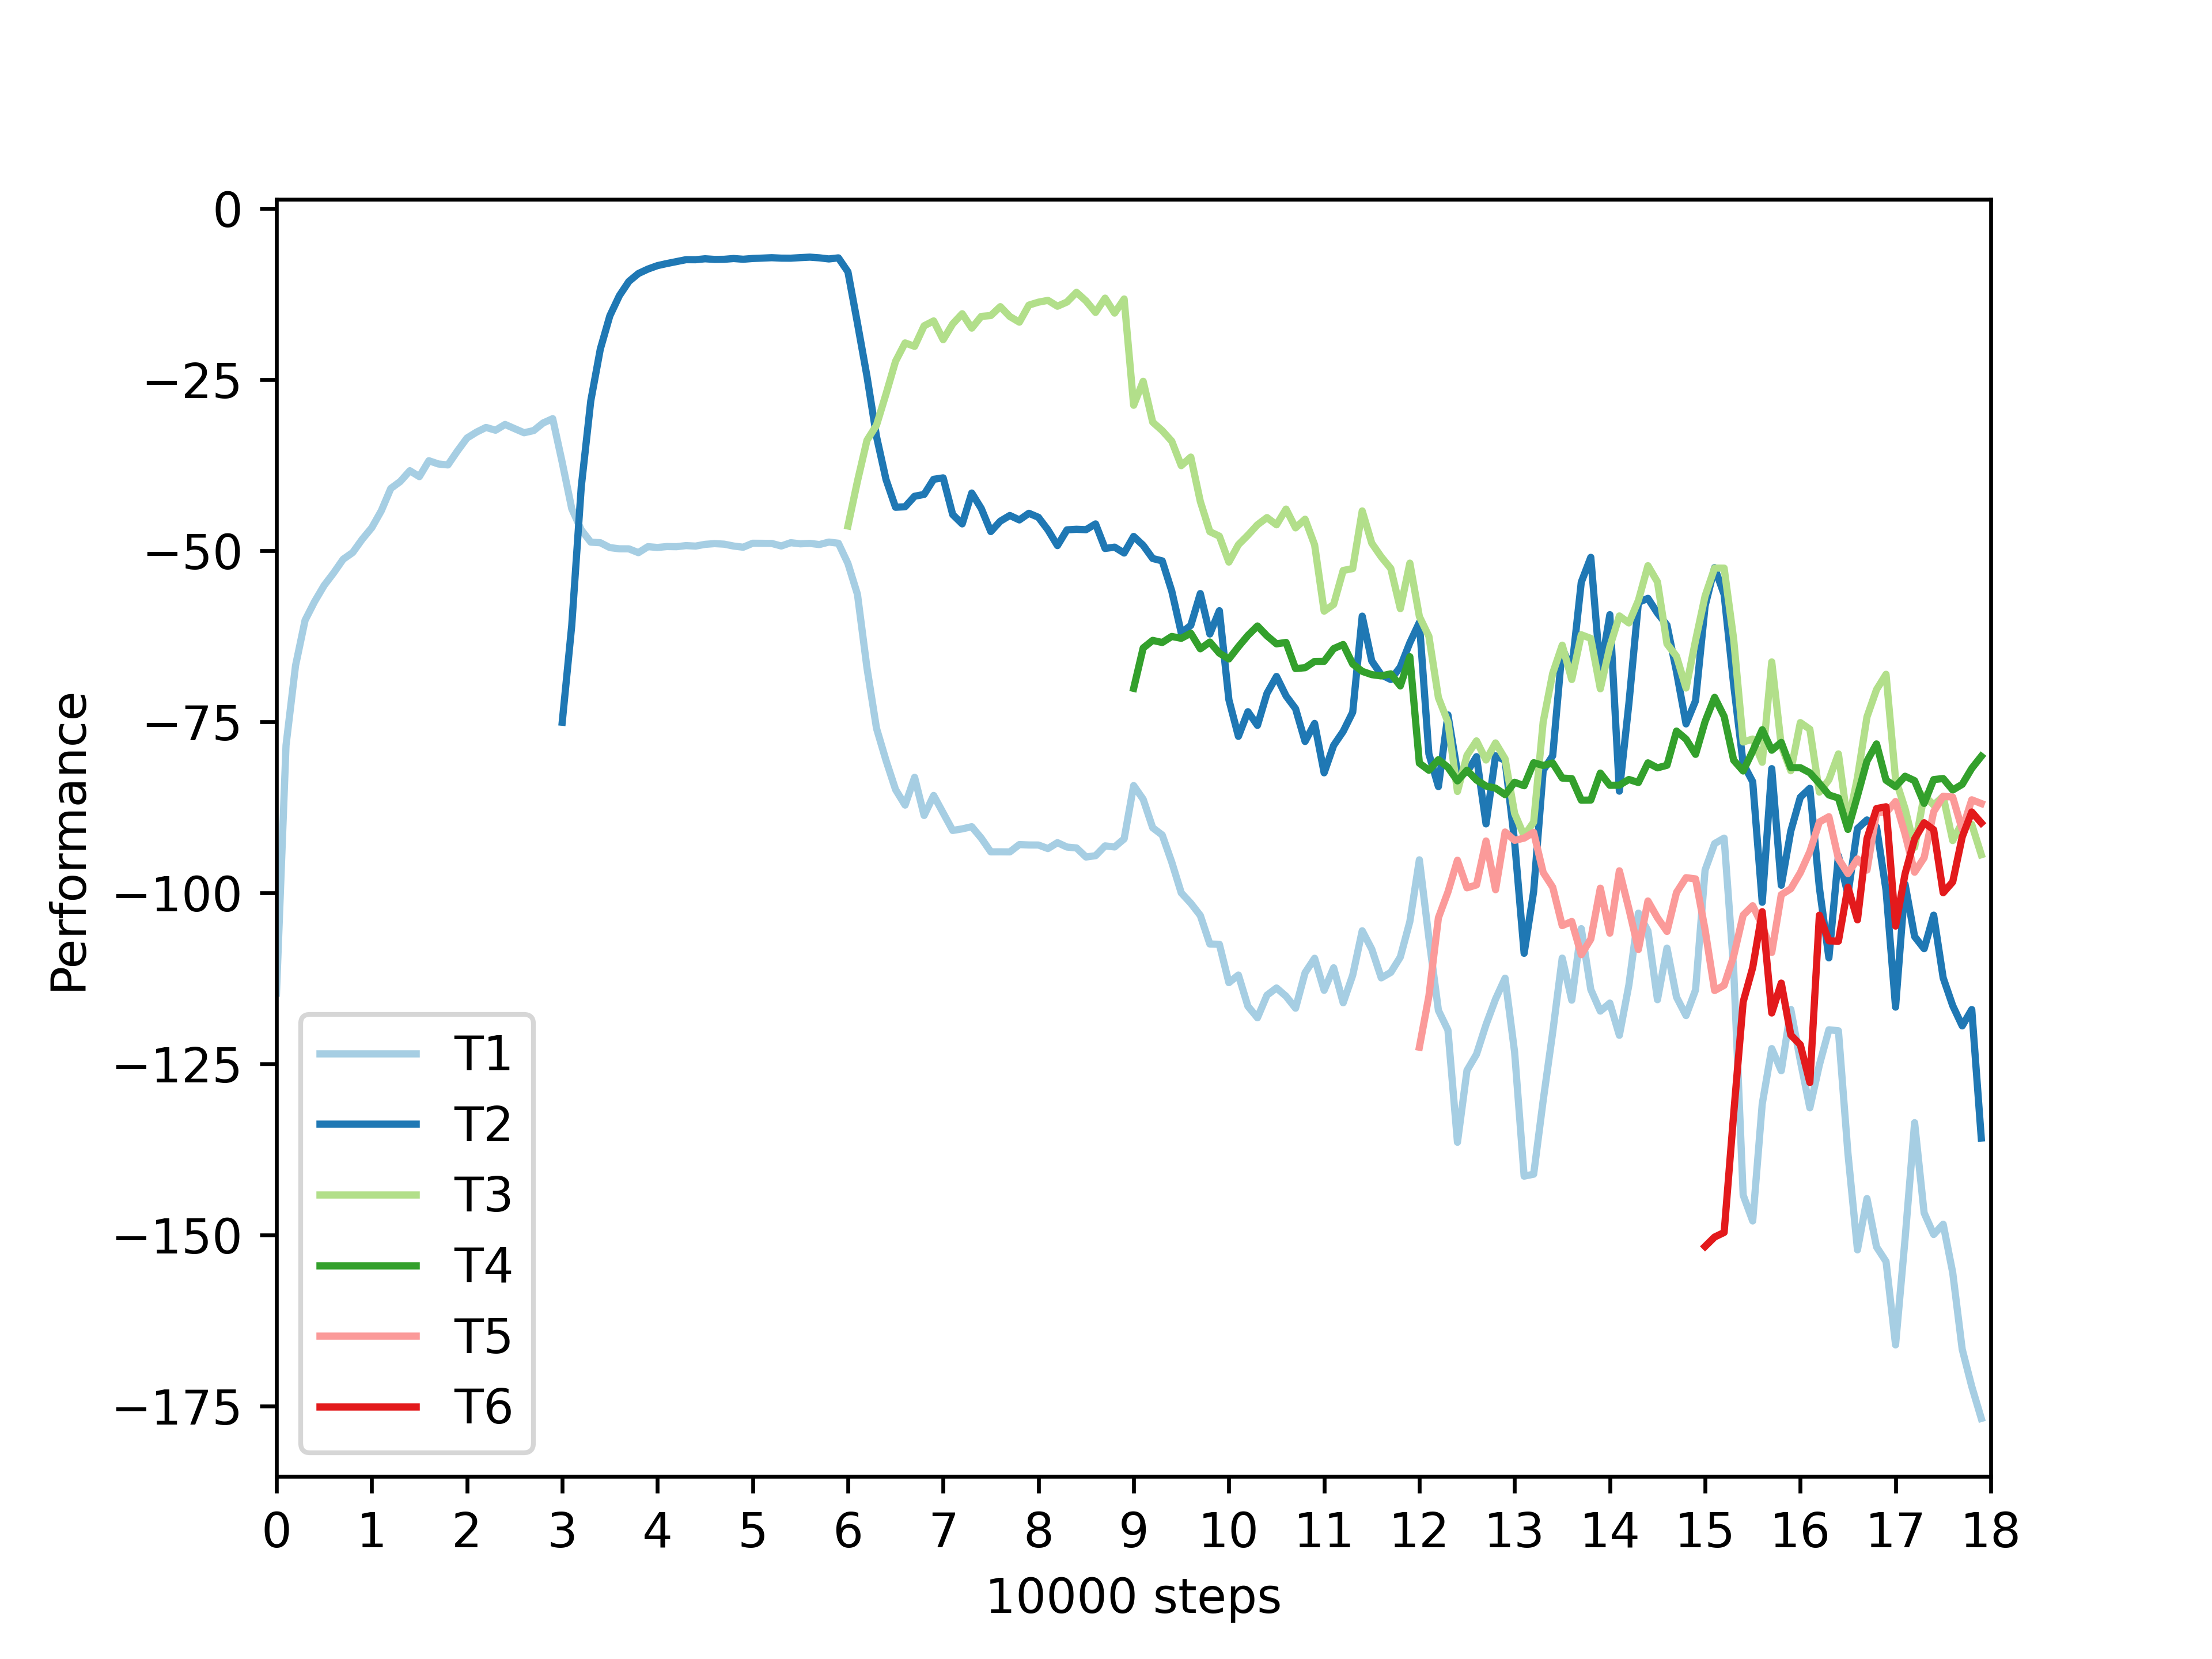}}
	
        \centering	
        \subcaptionbox{Vanilla DT}
    {\includegraphics[width=0.245\linewidth]{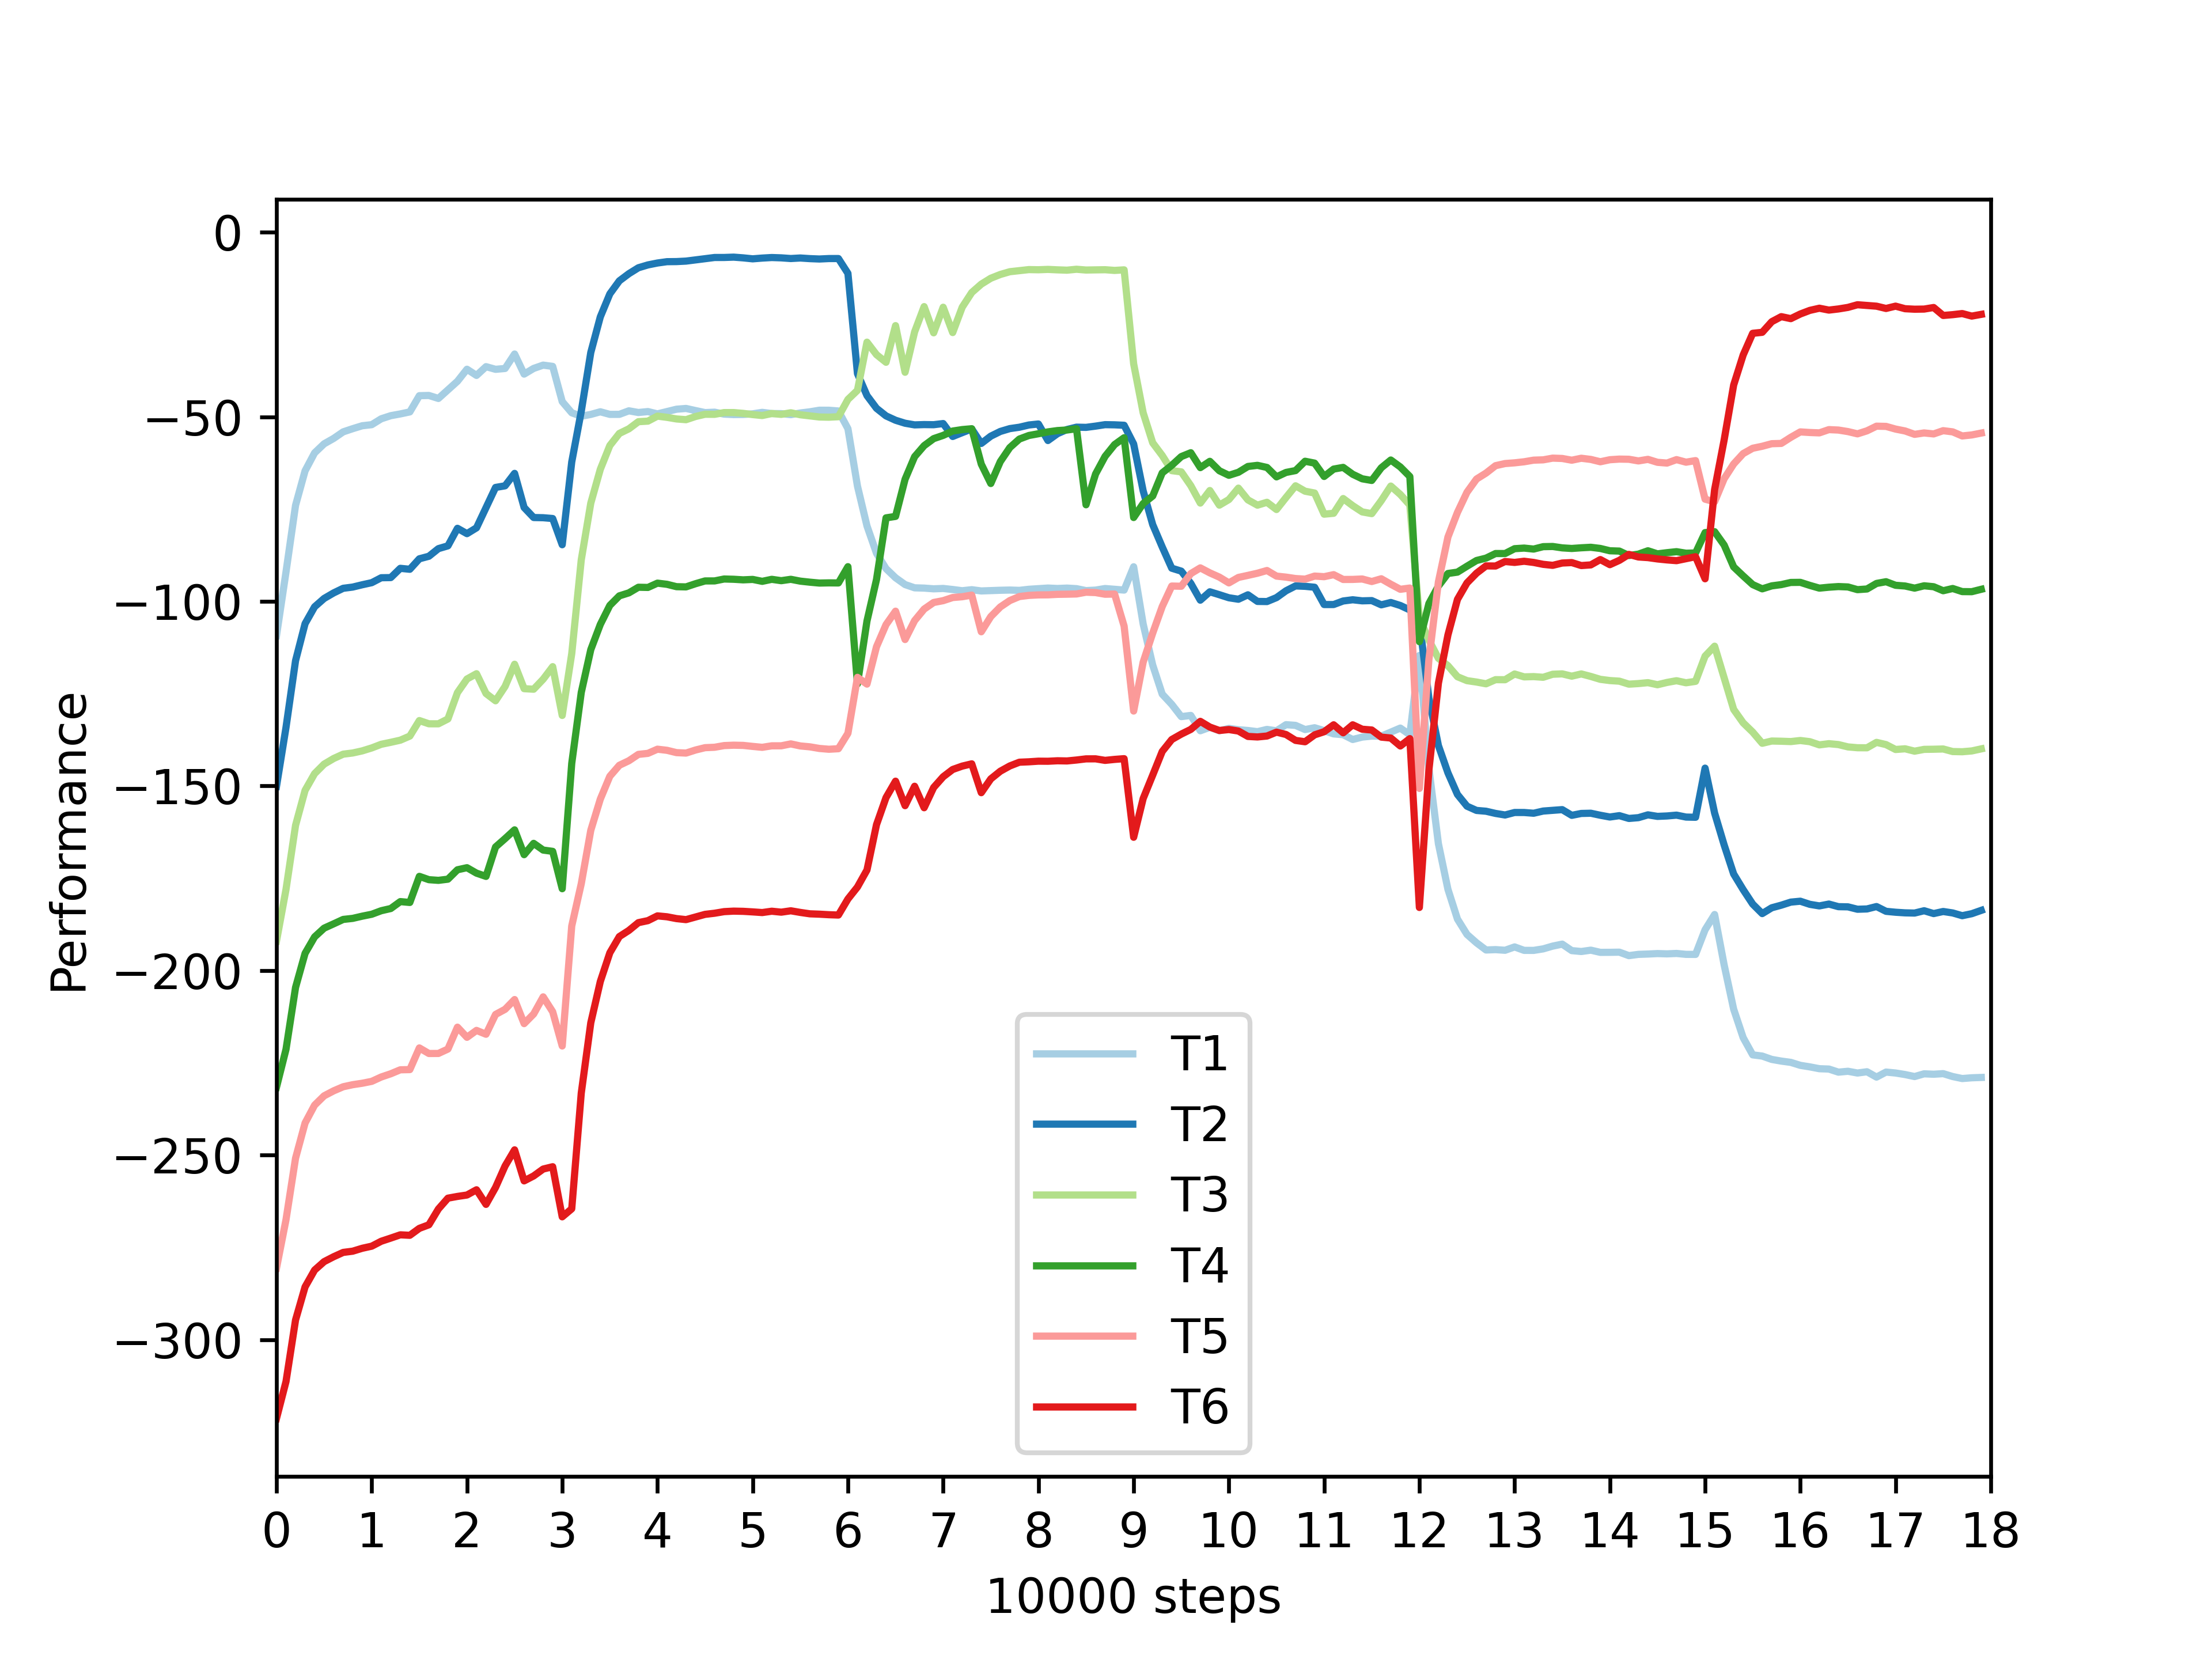}}
        \subcaptionbox{OER}
    {\includegraphics[width=0.245\linewidth]{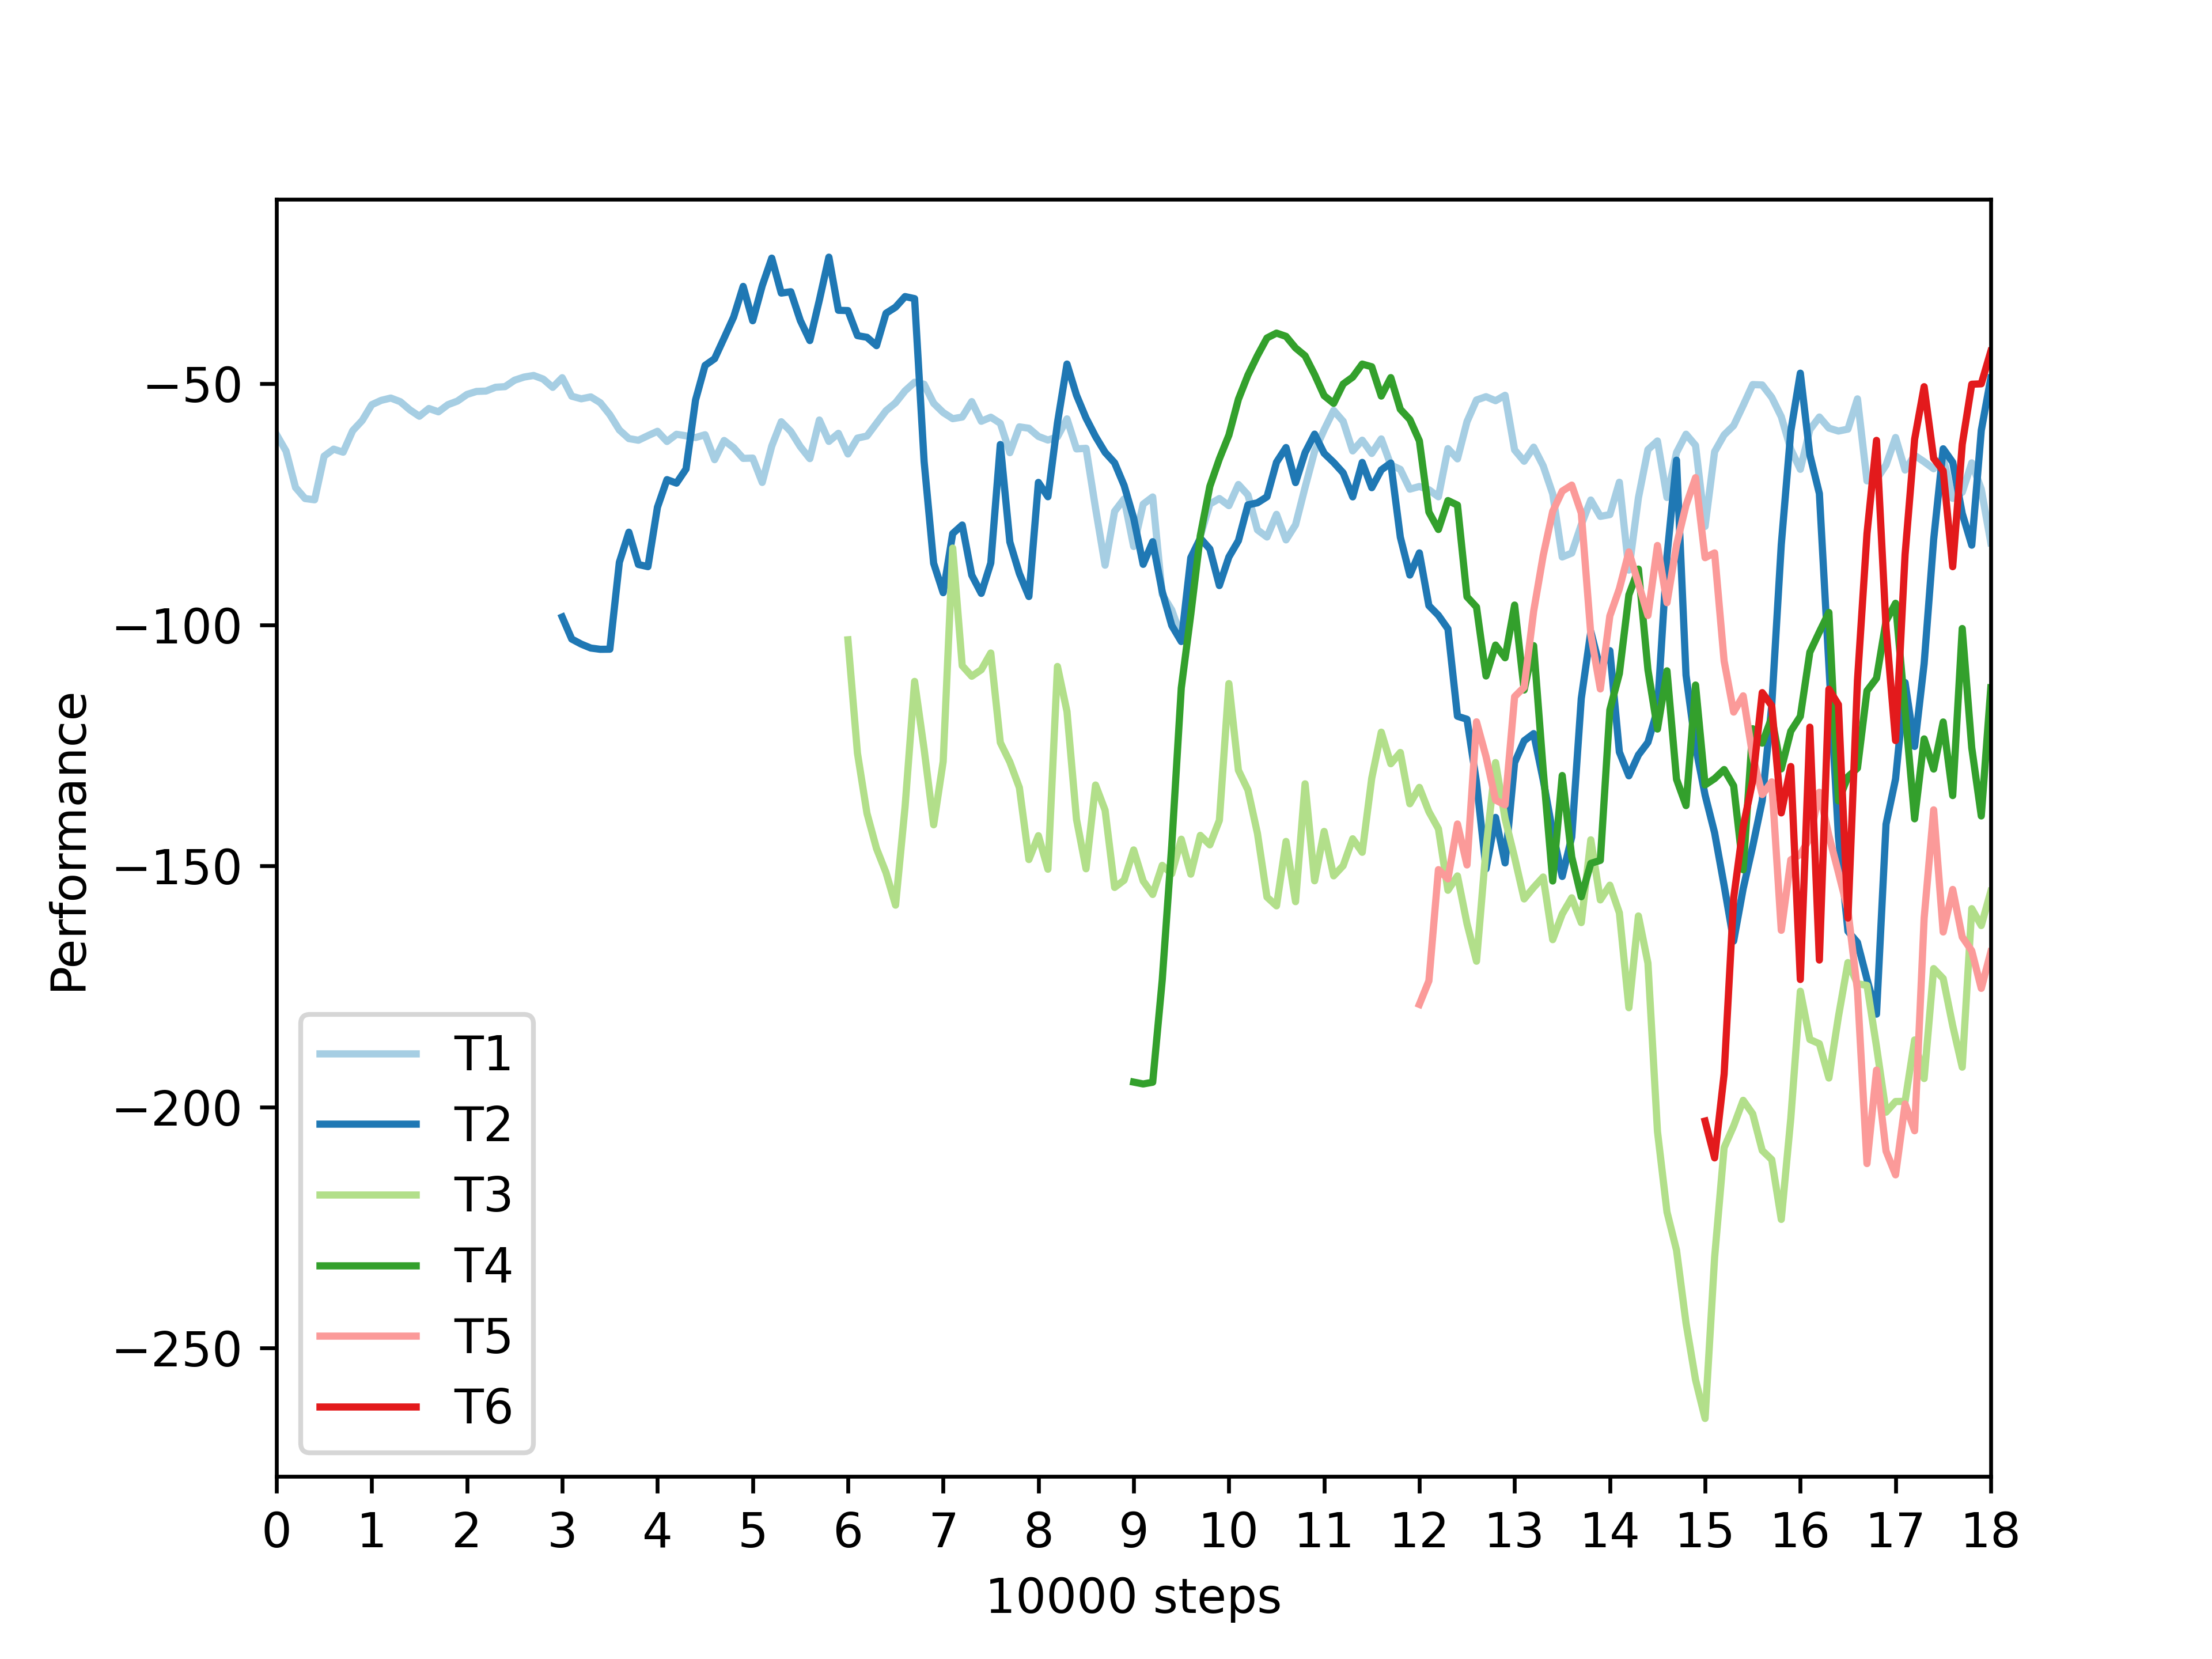}}
         \subcaptionbox{MH-DT}
    {\includegraphics[width=0.245\linewidth]{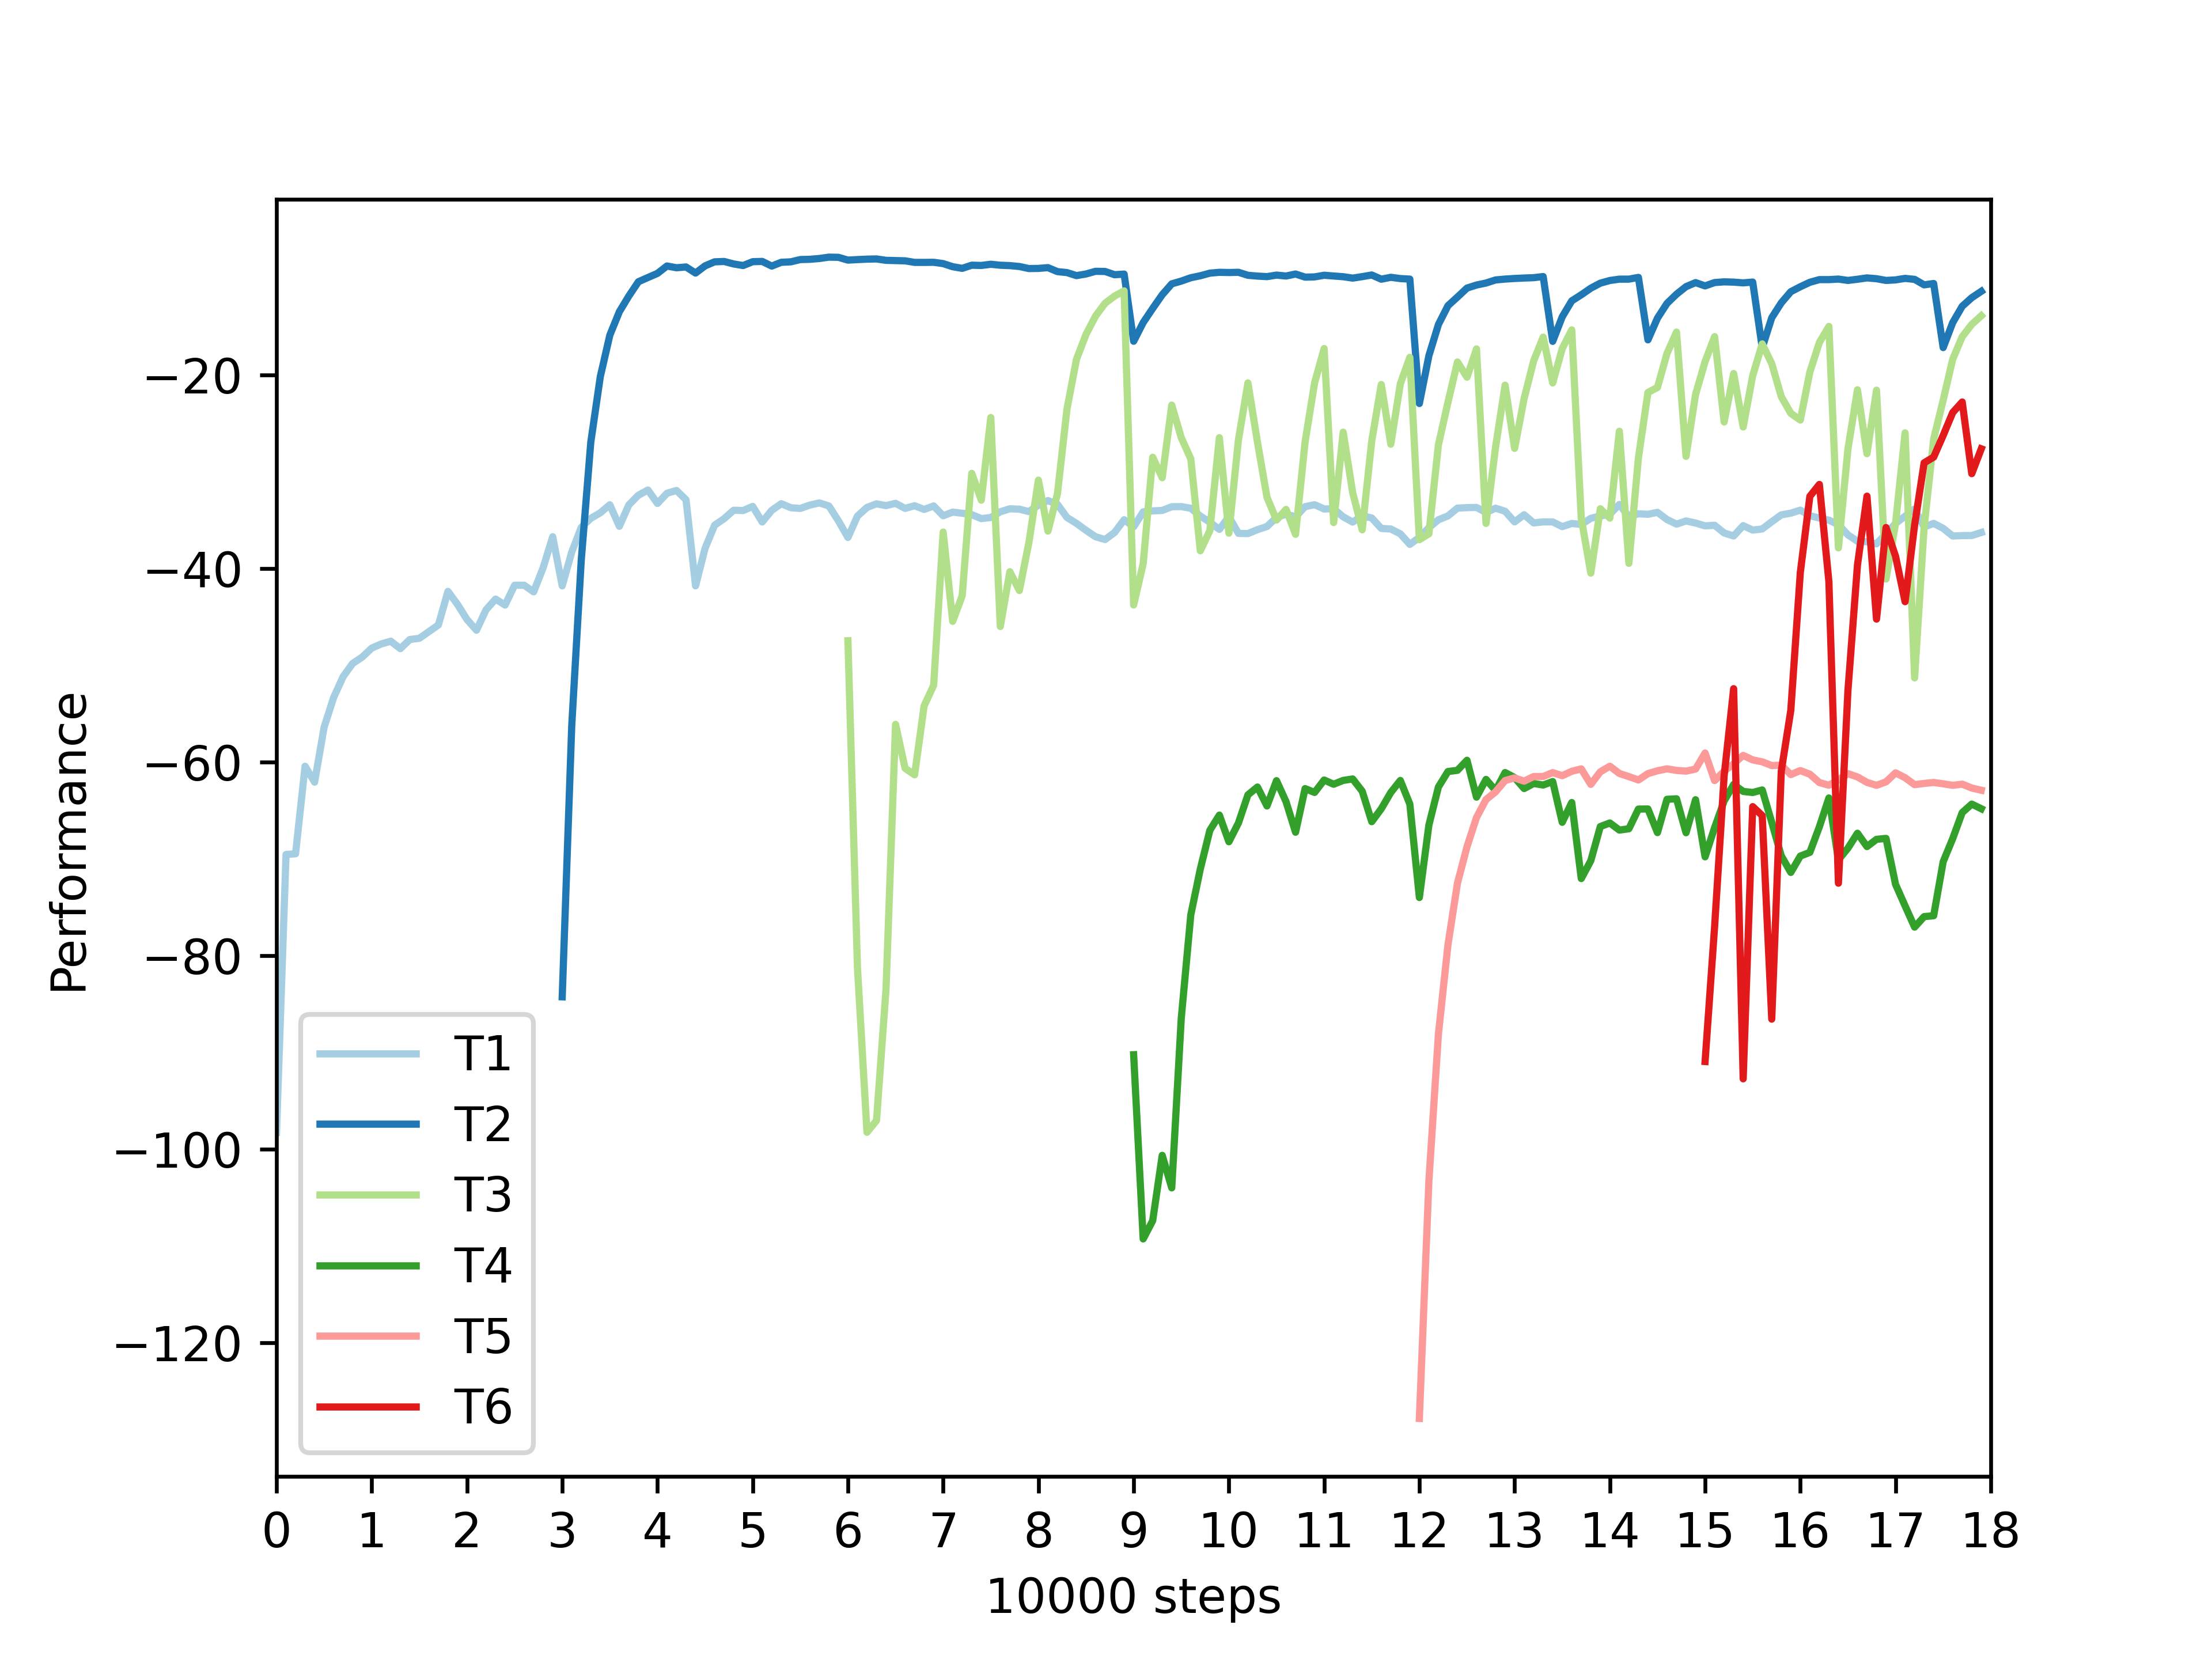}}
	\subcaptionbox{LoRA-DT}
    {\includegraphics[width=0.245\linewidth]{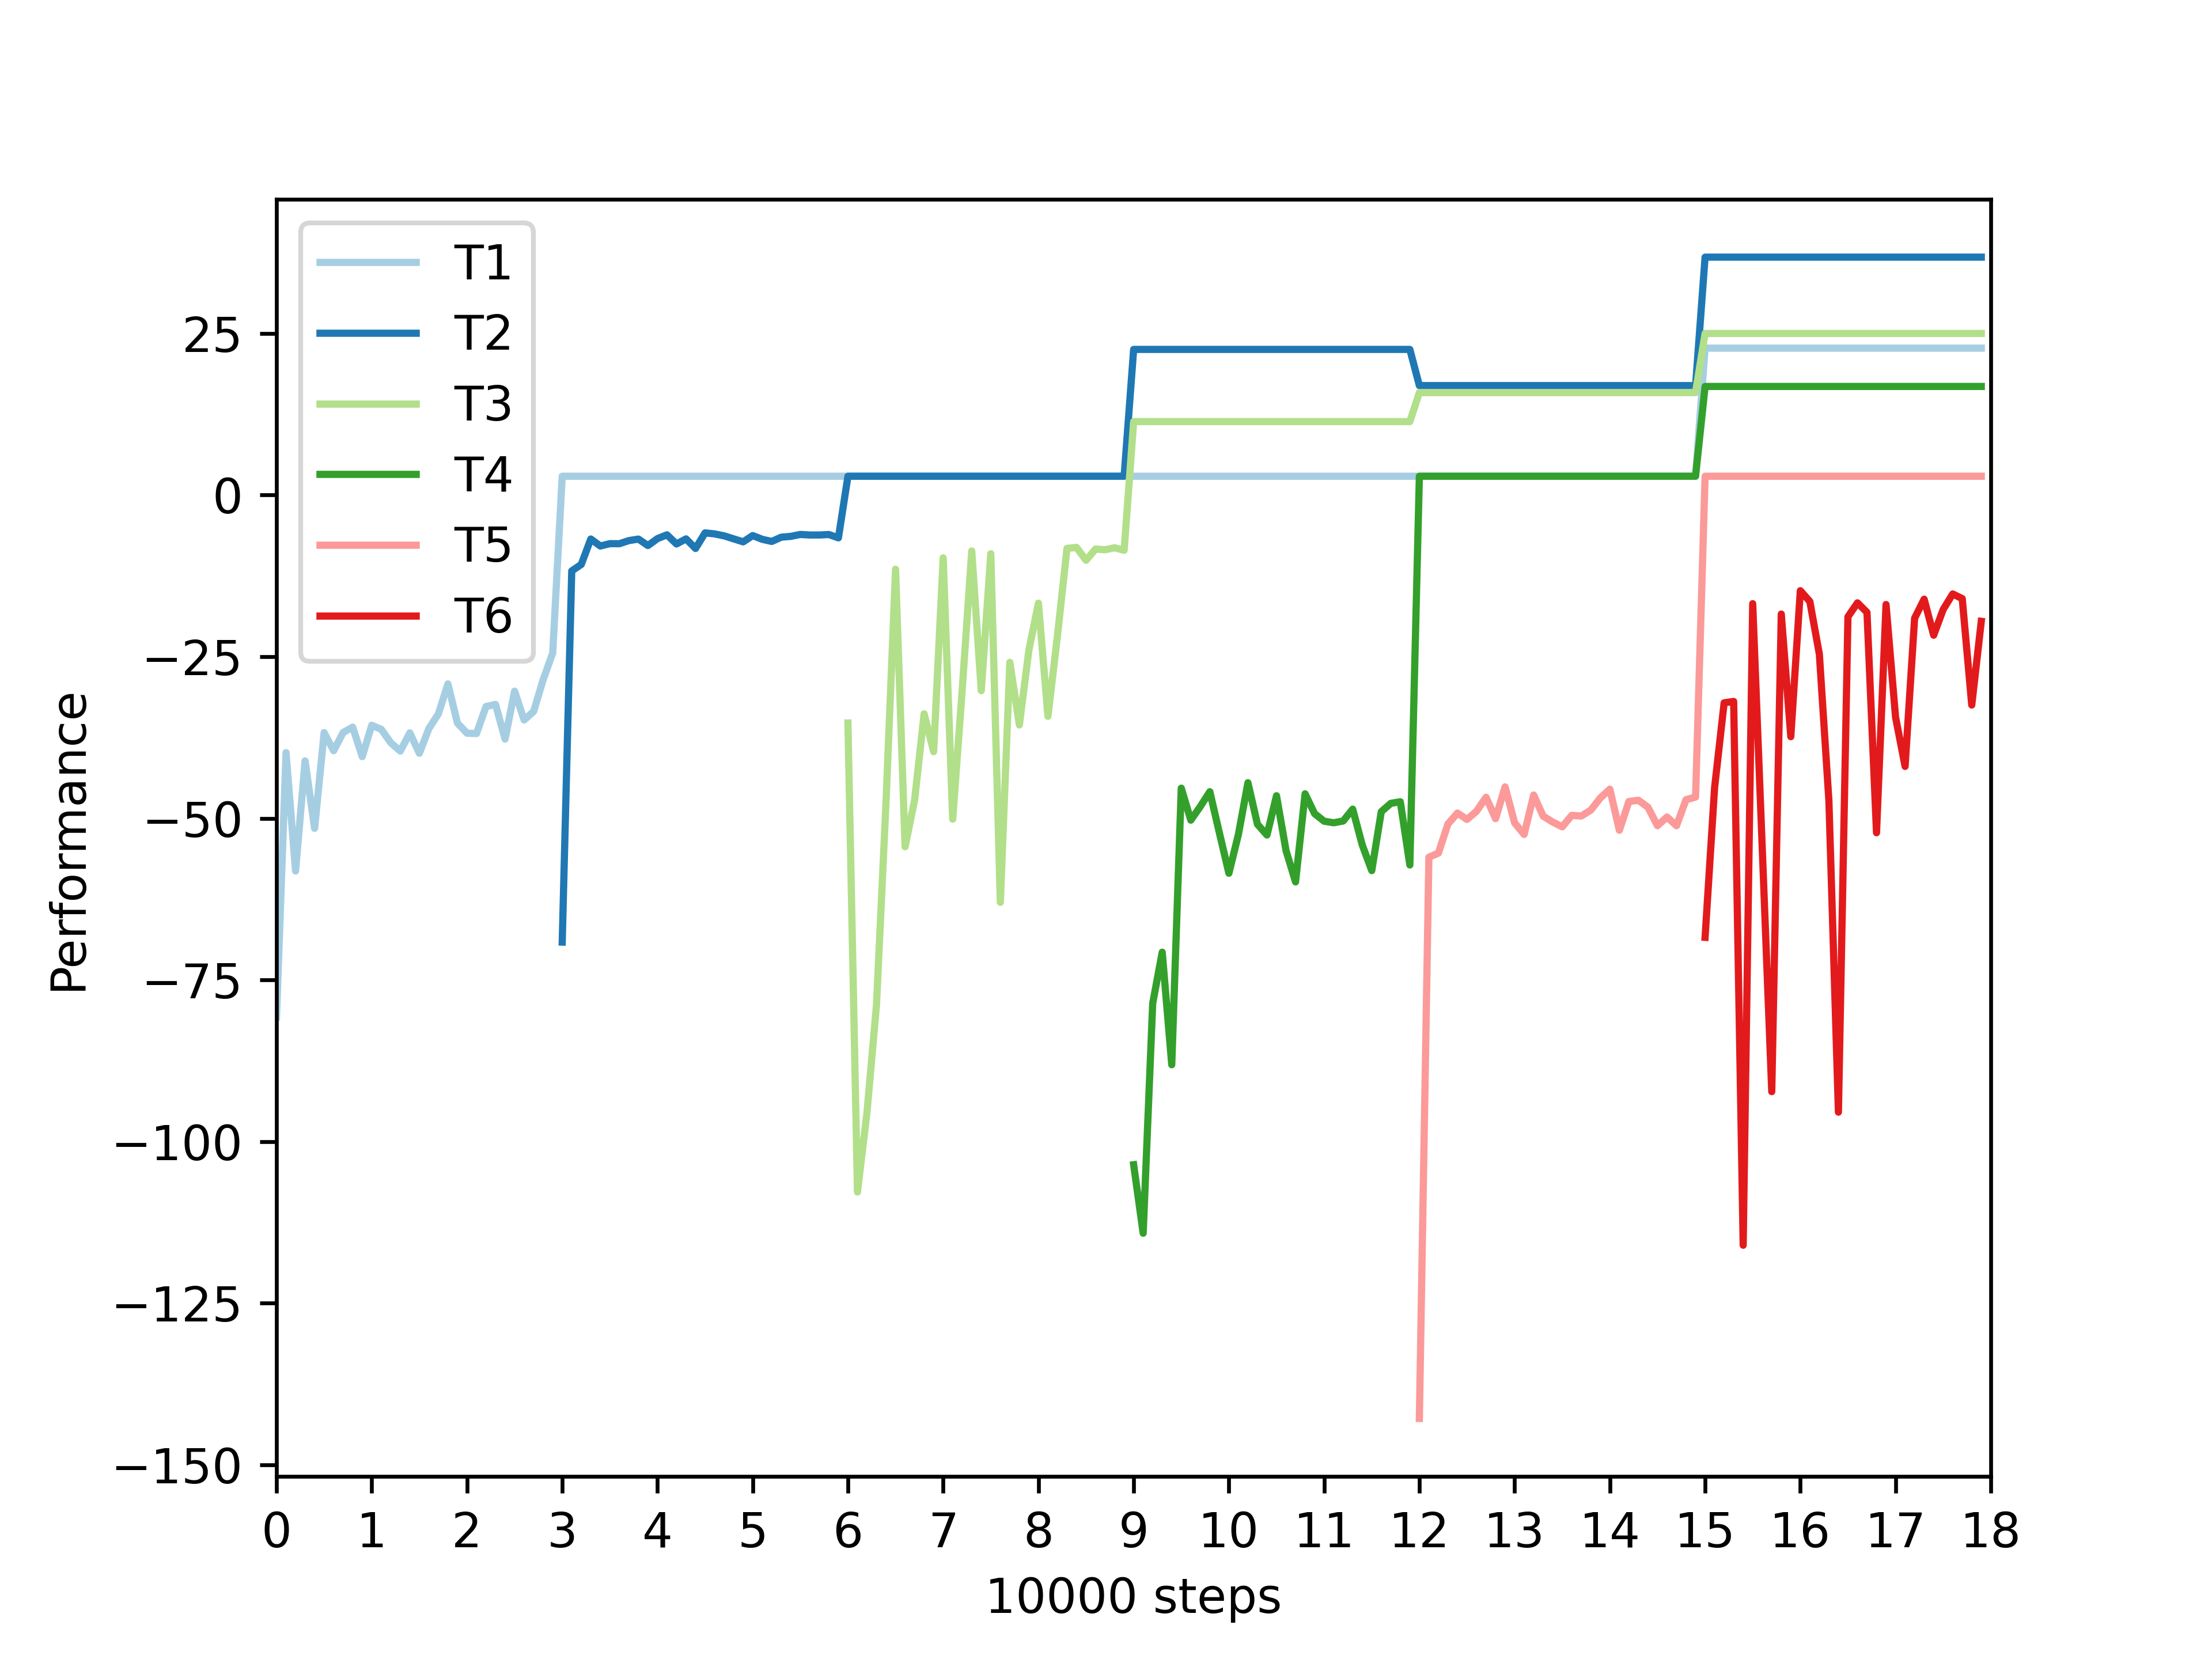}}
    \caption{Cheetah\_Vel (middle)}
\end{figure}

\begin{figure}[htbp]
	\centering
	\subcaptionbox{PDT}
    {\includegraphics[width=0.245\linewidth]{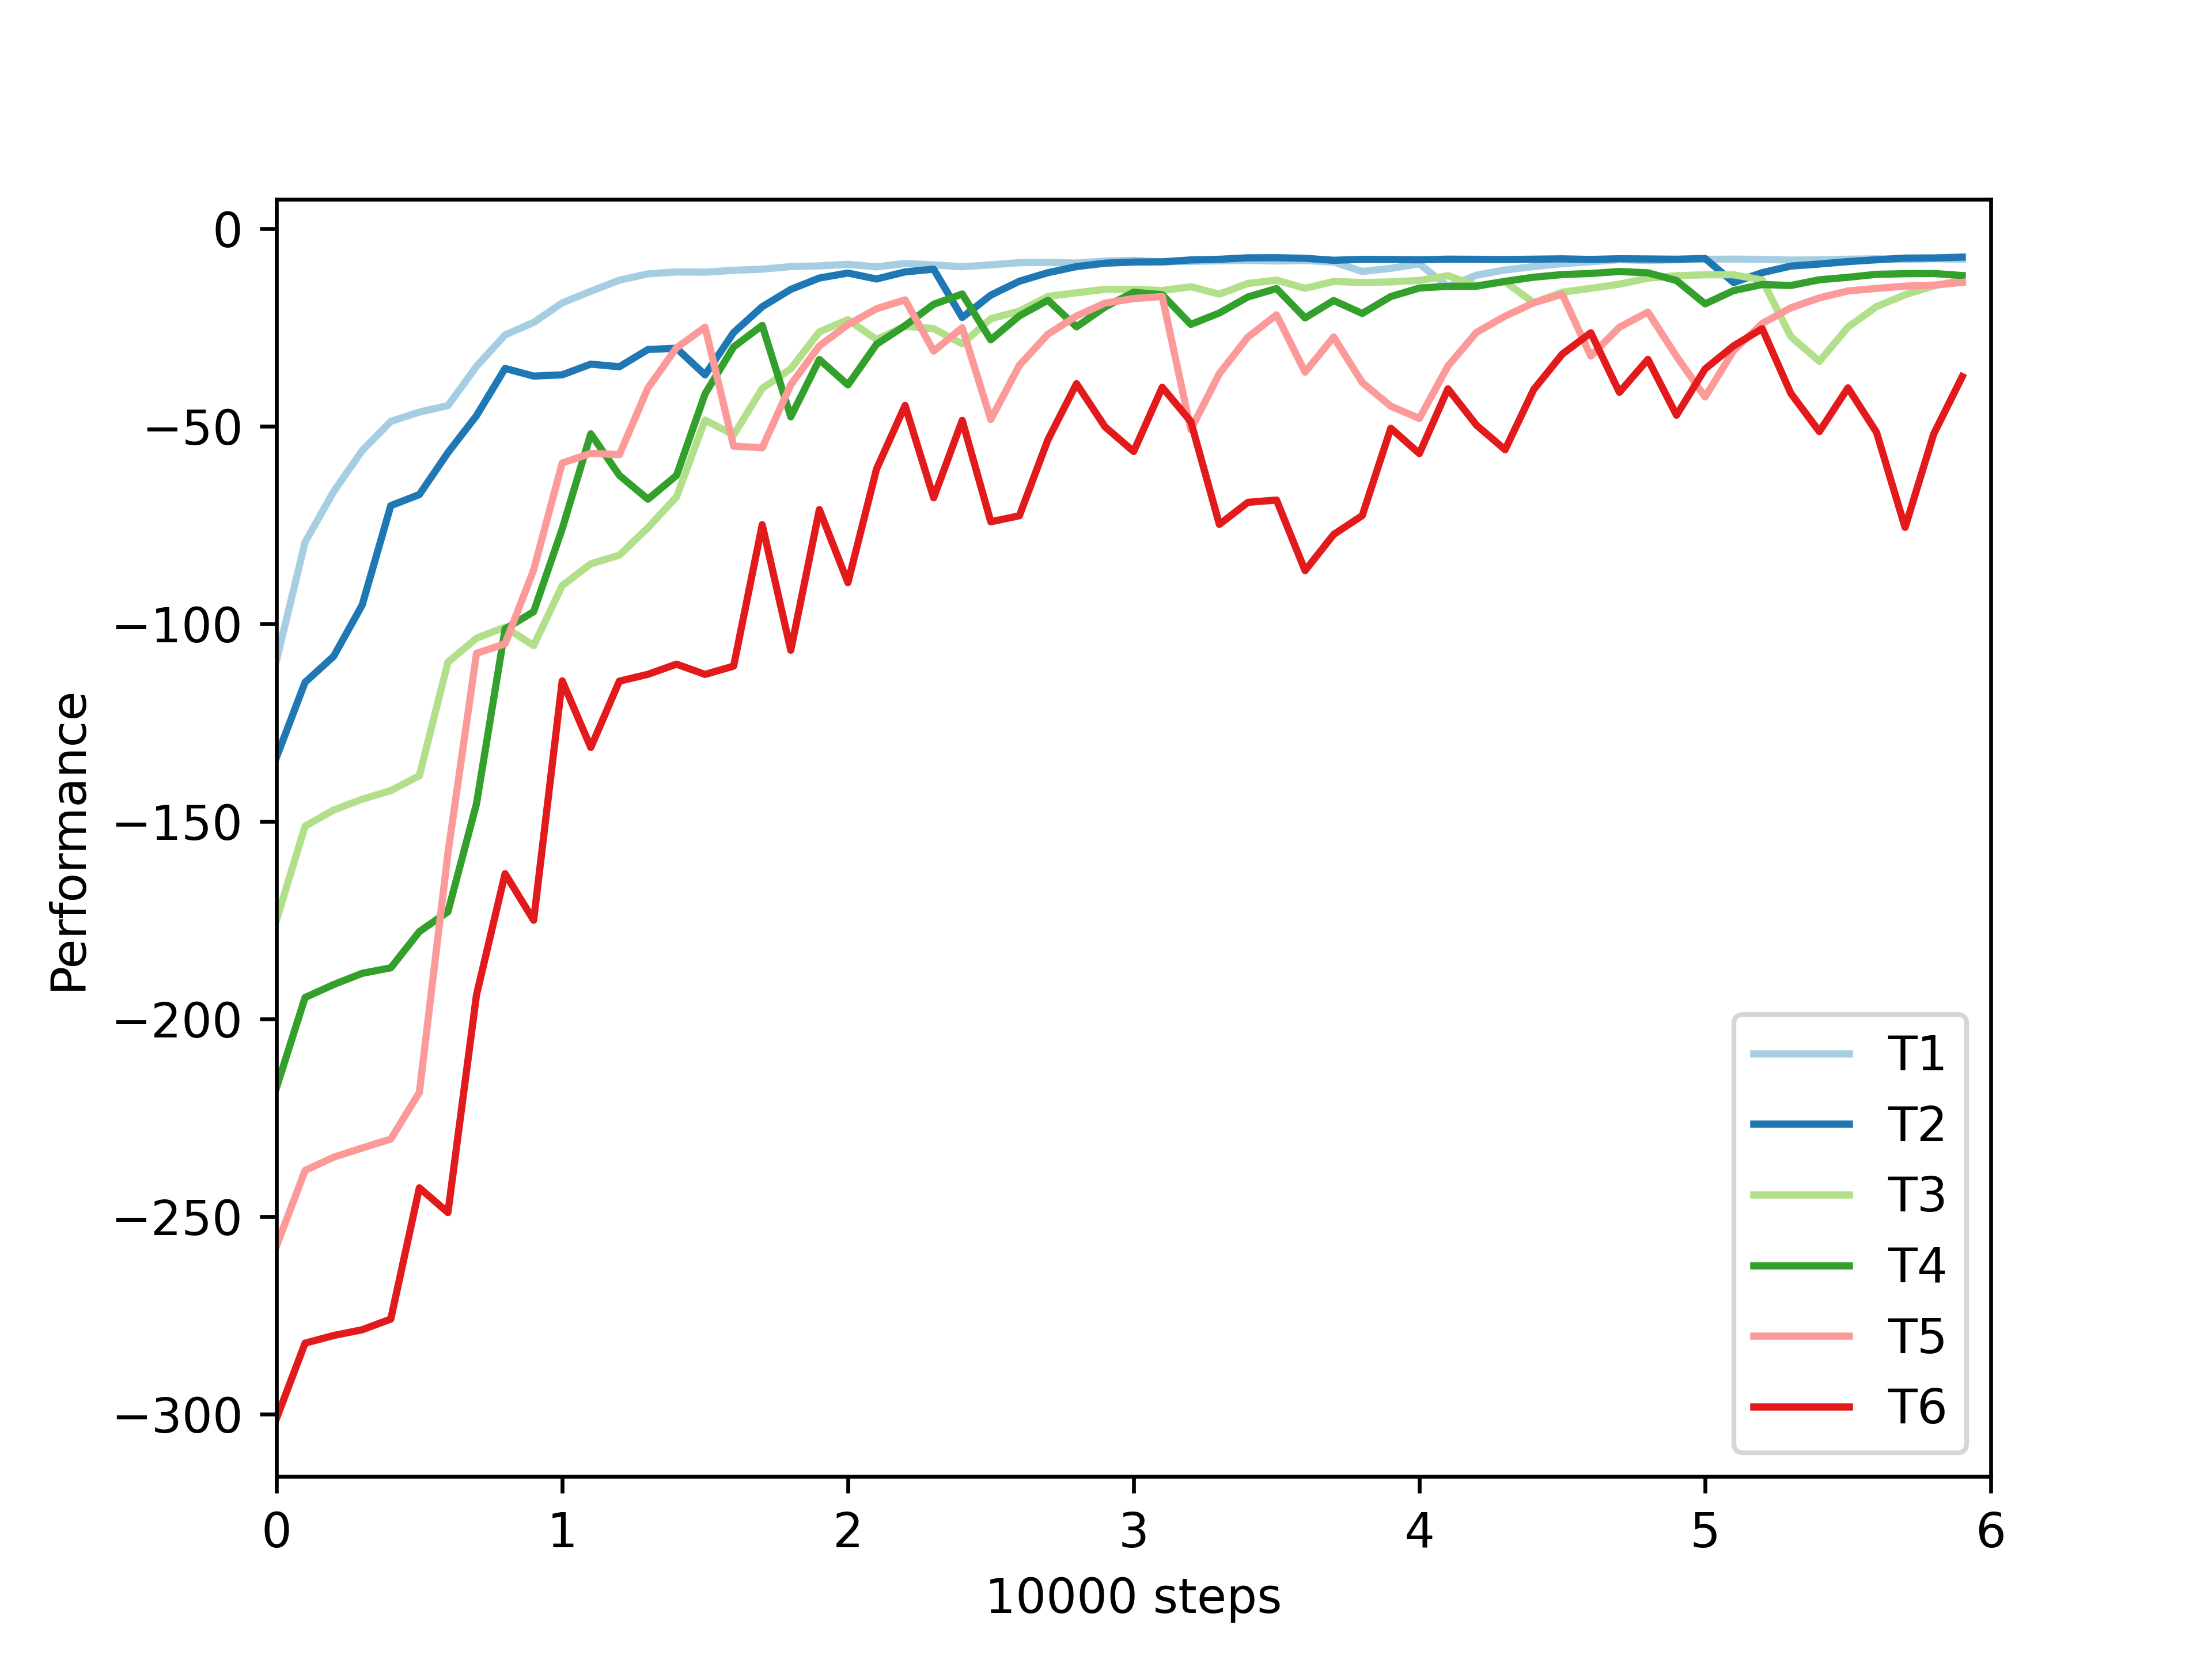}}
	\subcaptionbox{DT + EWC}
    {\includegraphics[width=0.245\linewidth]{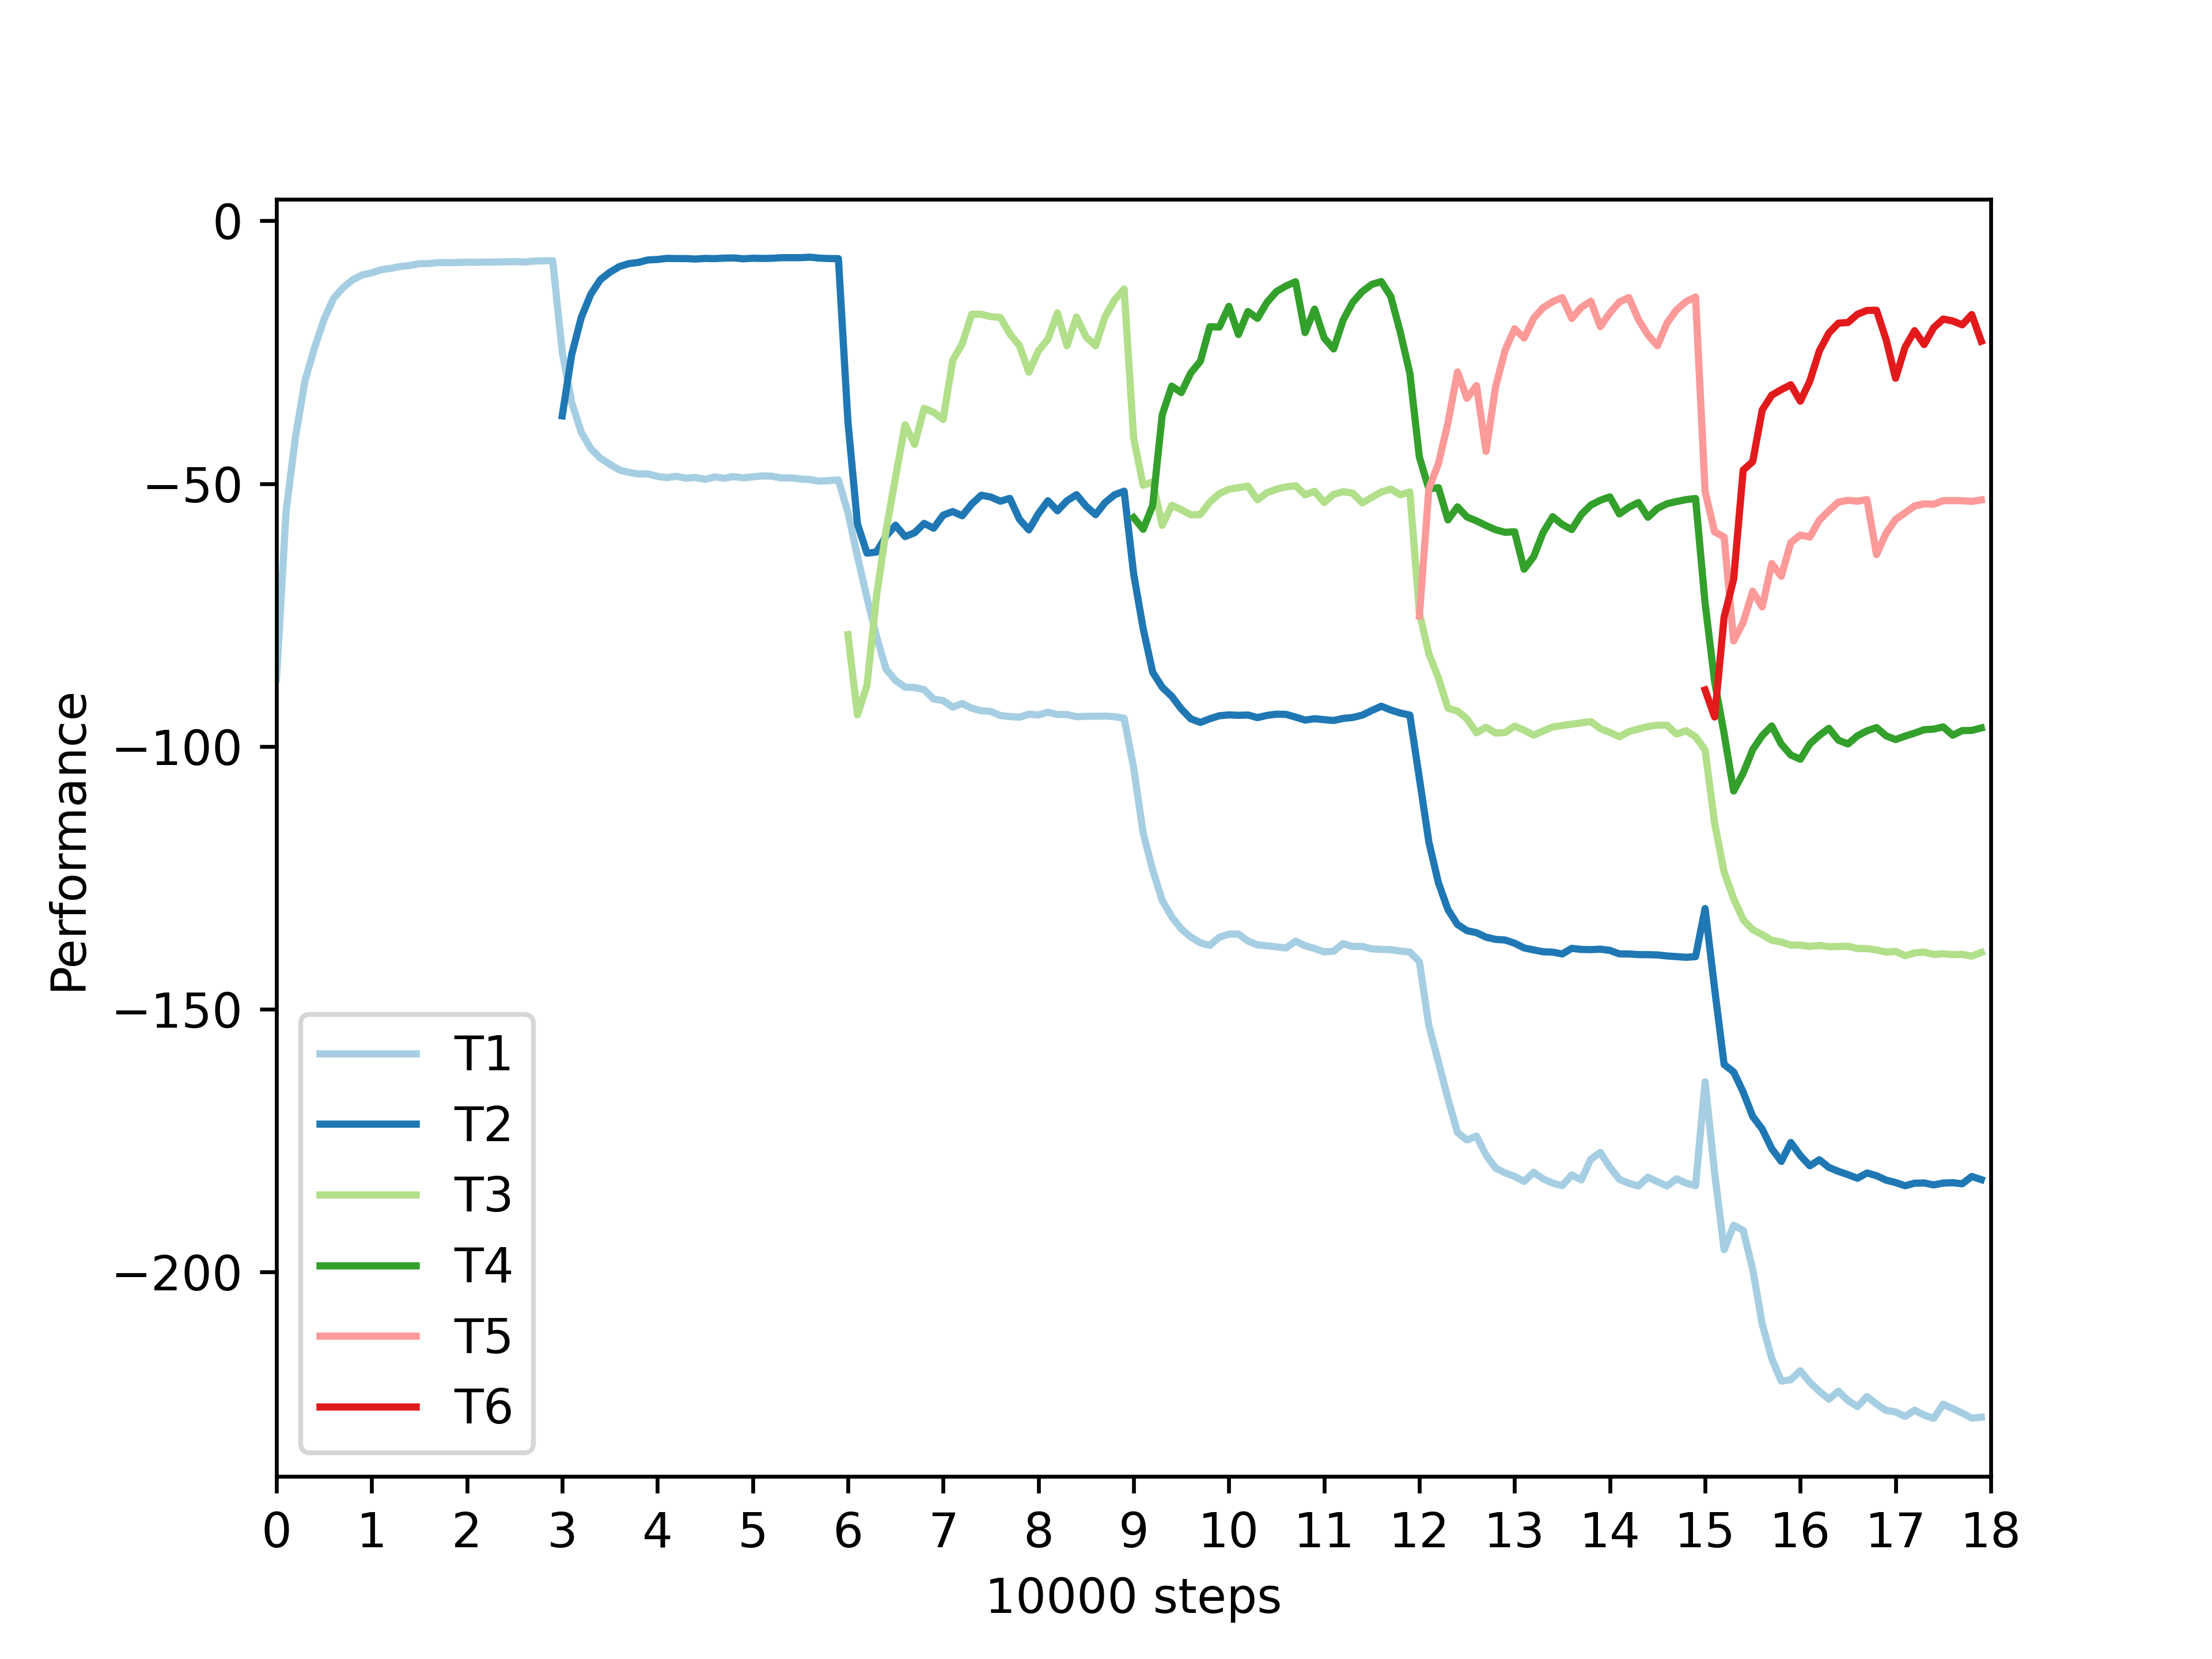}}
    \subcaptionbox{DT + SI}
    {\includegraphics[width=0.245\linewidth]{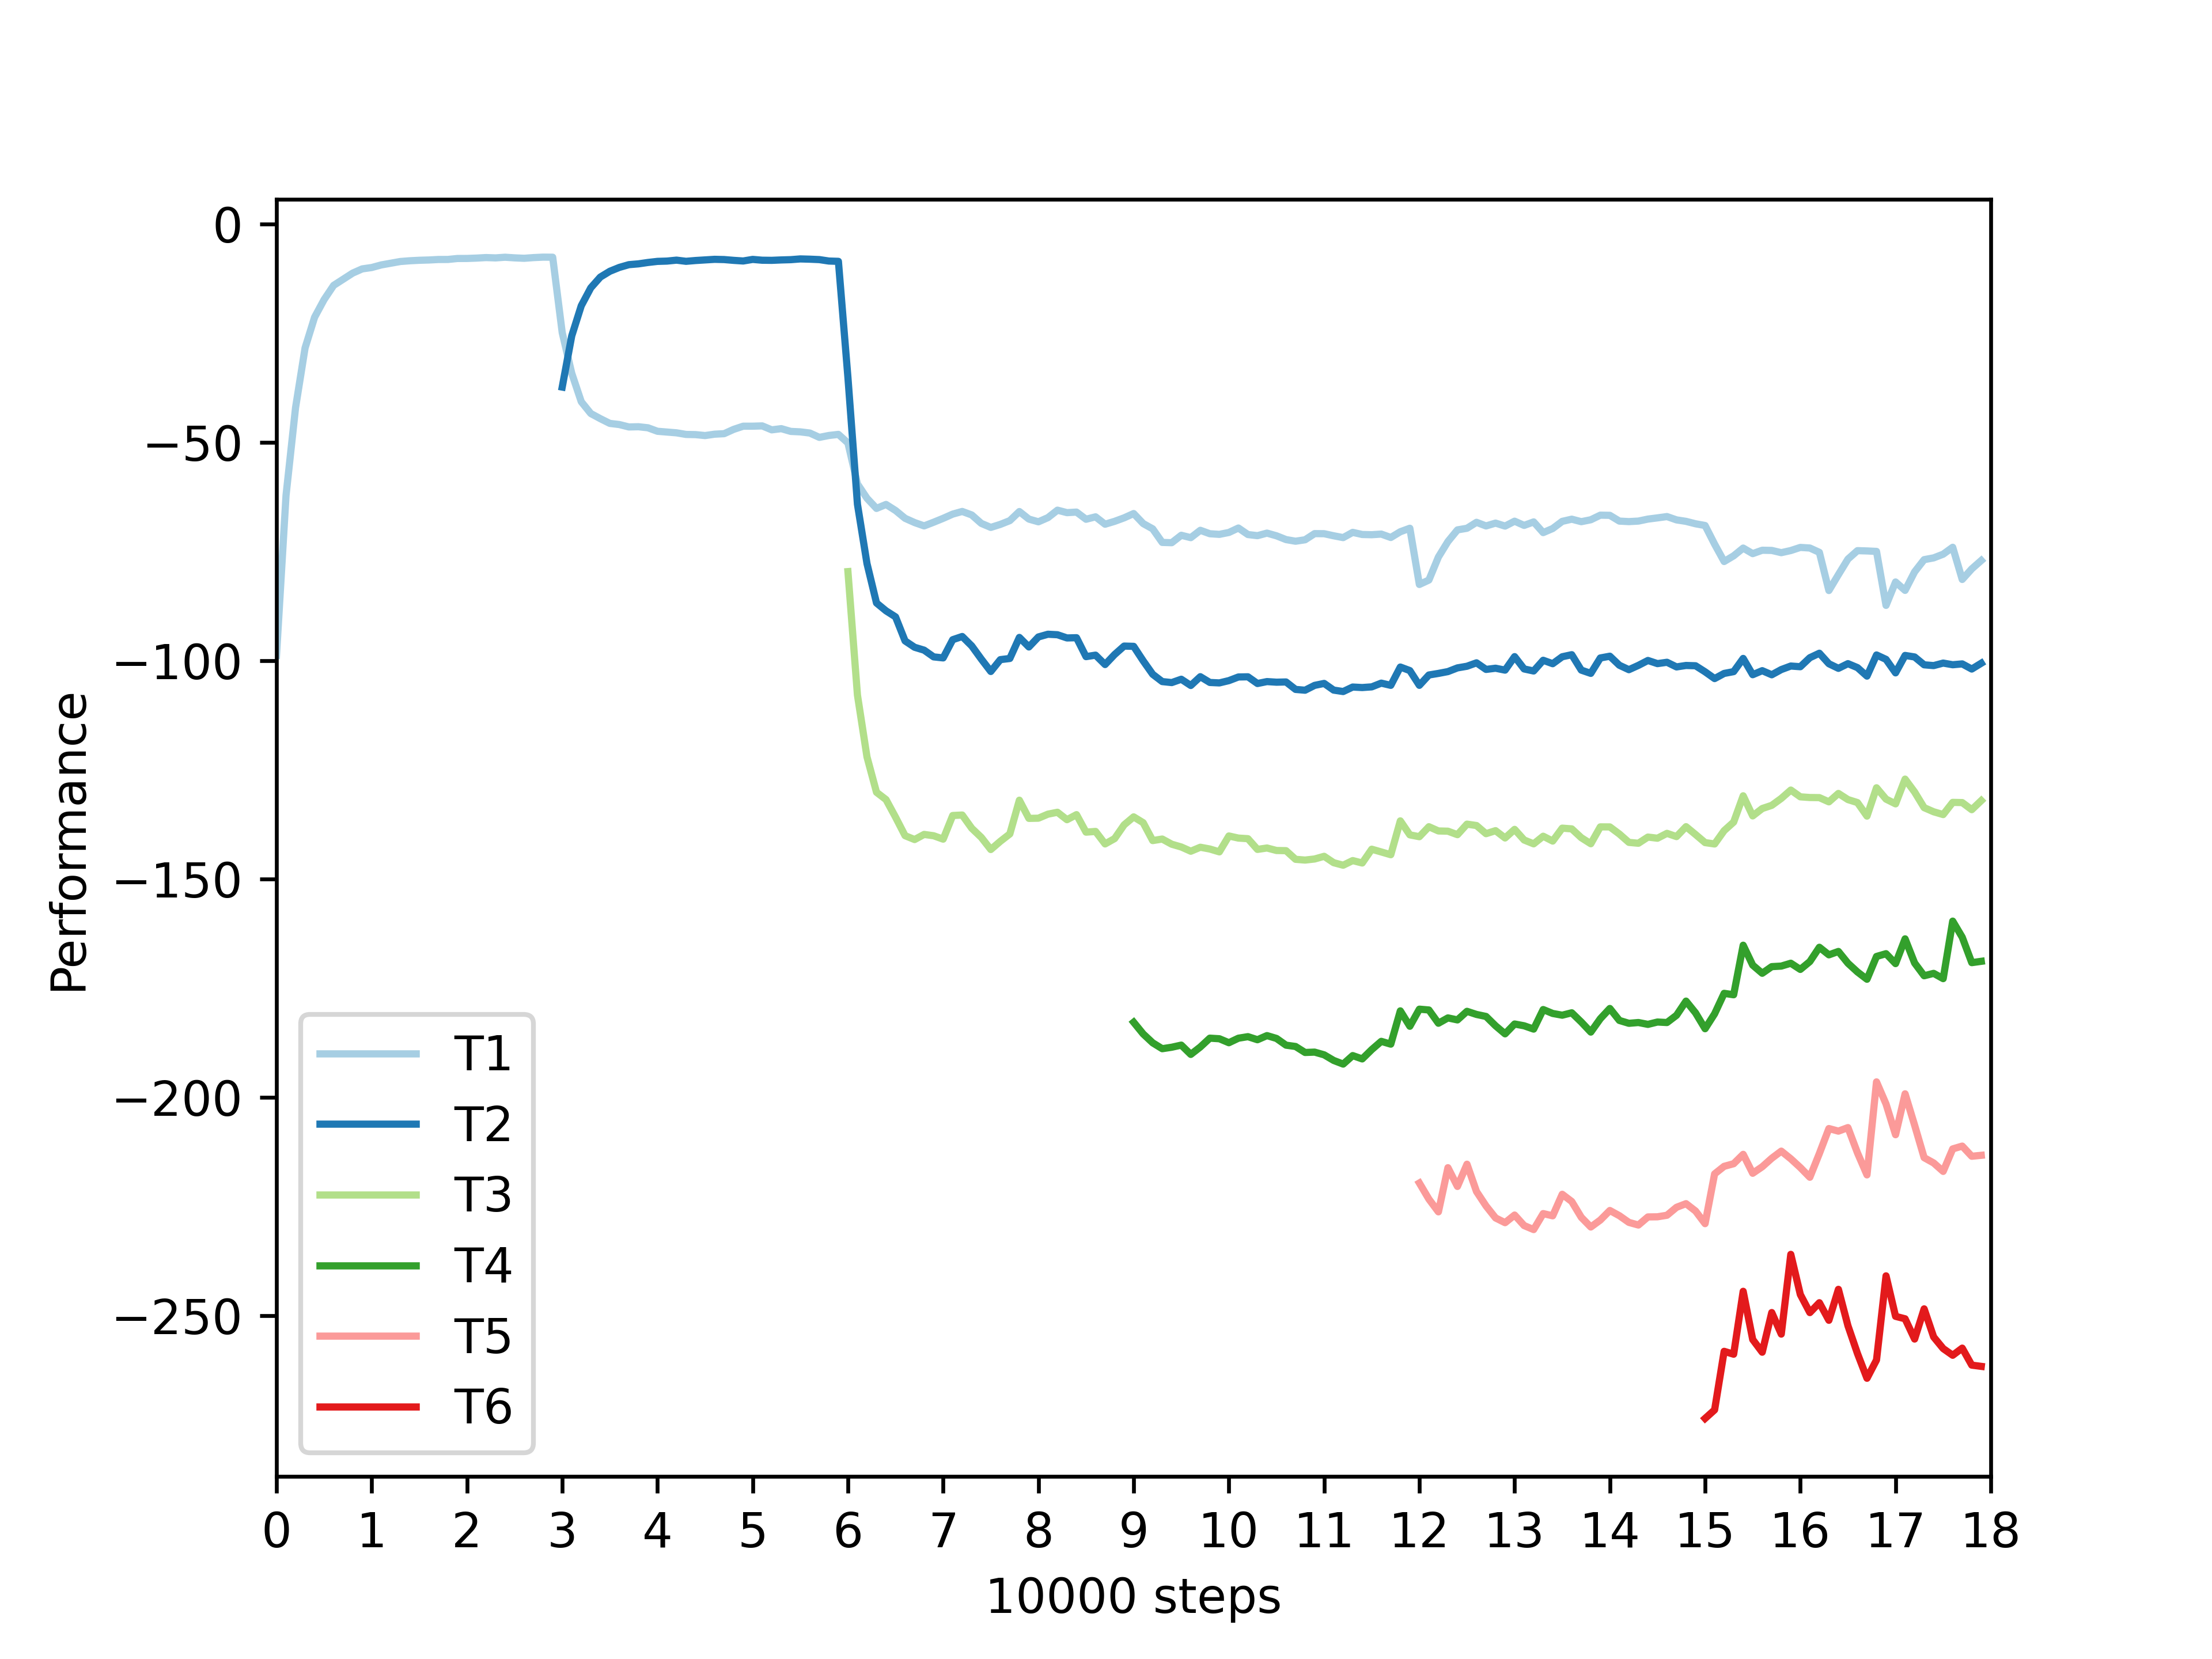}}
    \subcaptionbox{DT + GEM}
    {\includegraphics[width=0.245\linewidth]{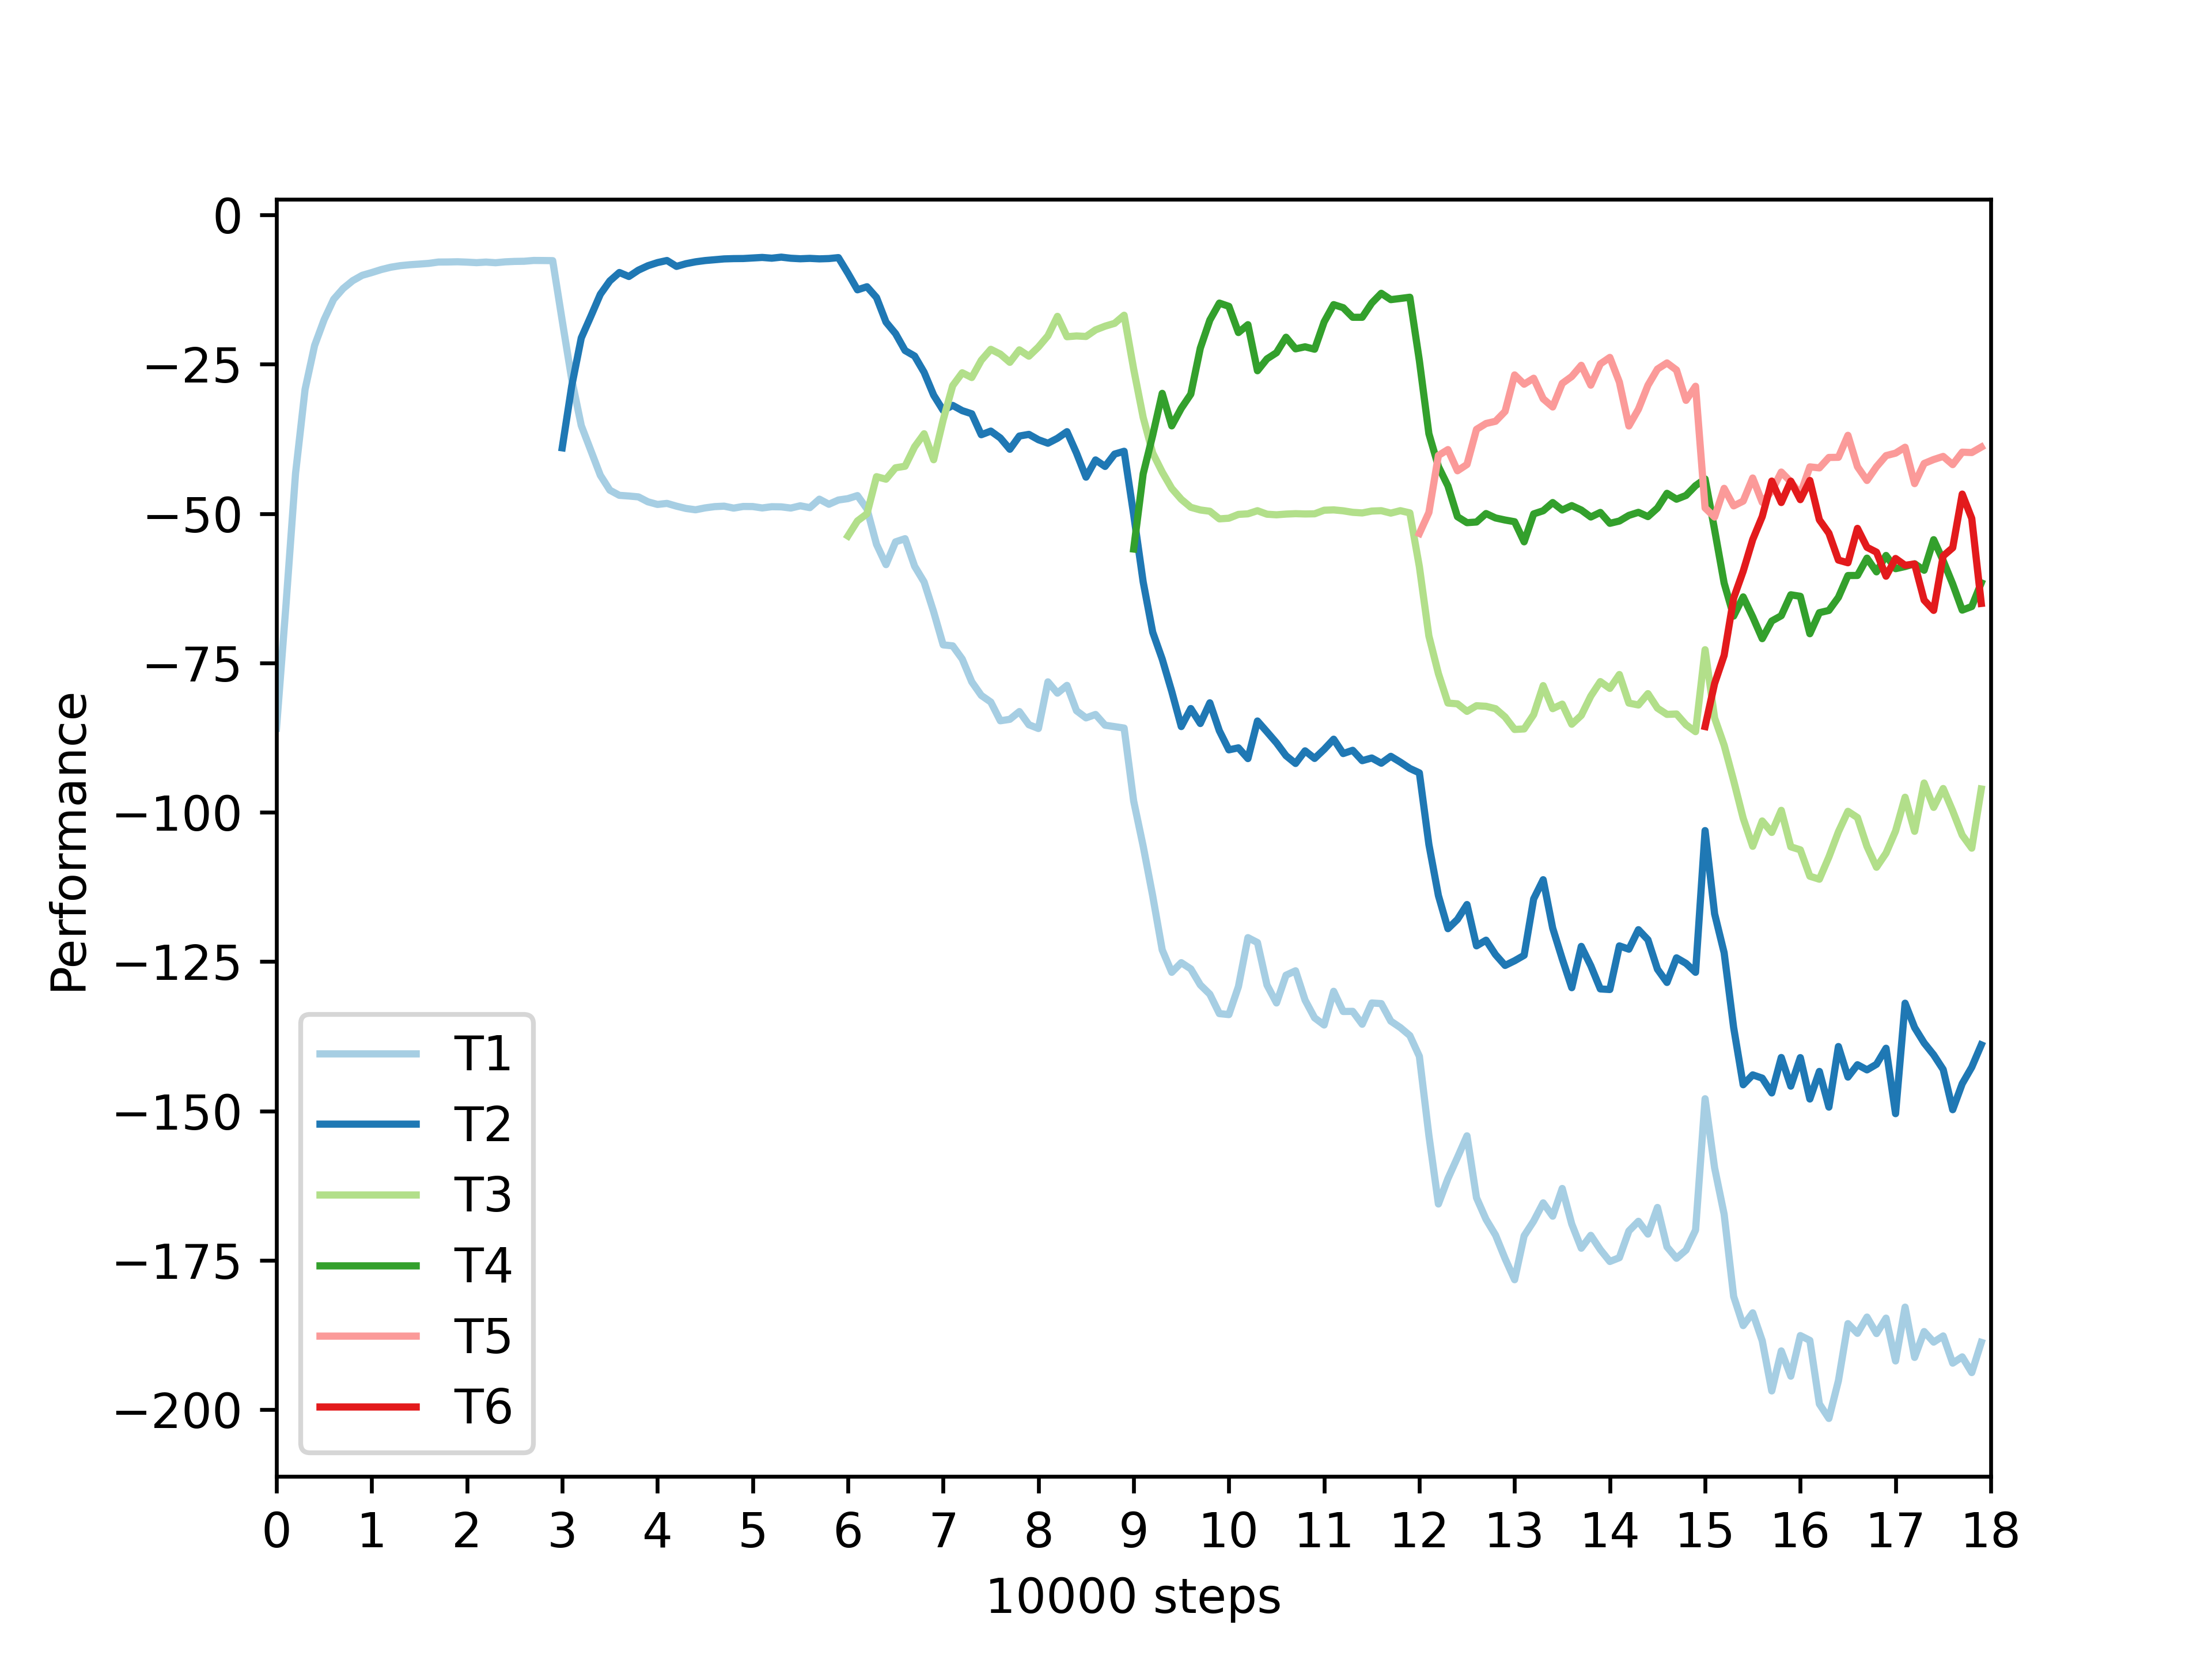}}
	
        \centering	
        \subcaptionbox{Vanilla DT}
    {\includegraphics[width=0.245\linewidth]{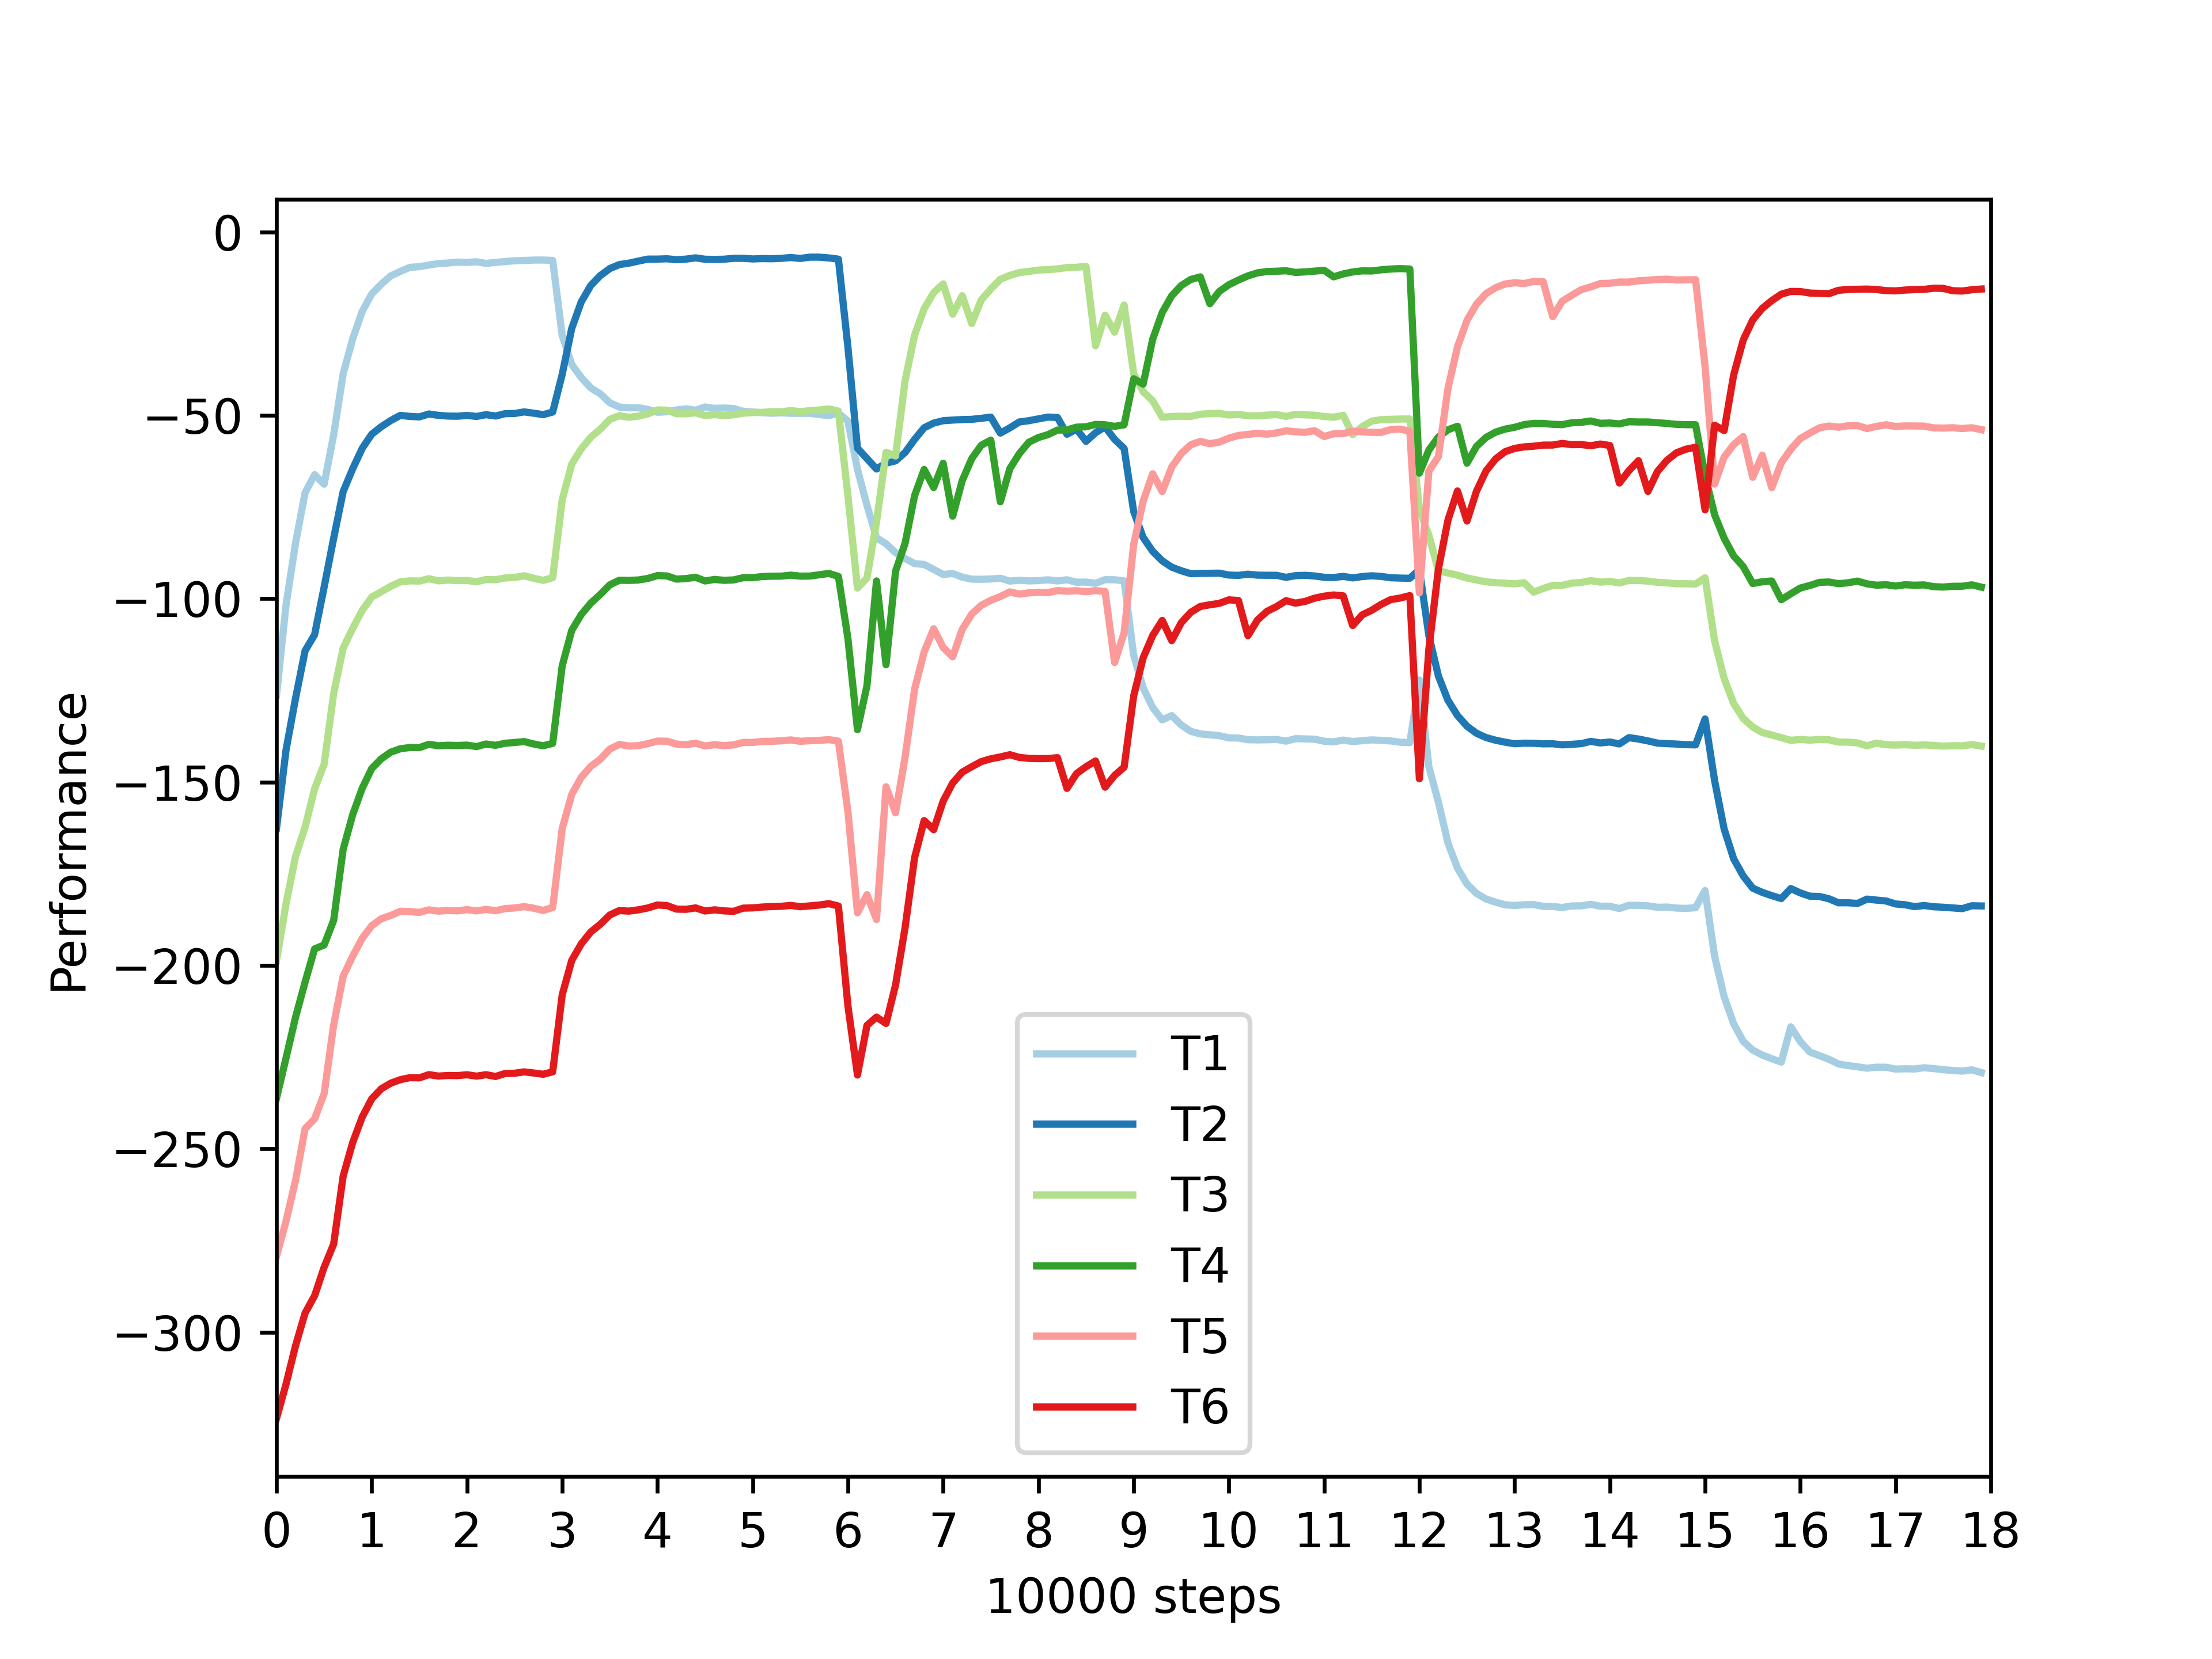}}
        \subcaptionbox{OER}
    {\includegraphics[width=0.245\linewidth]{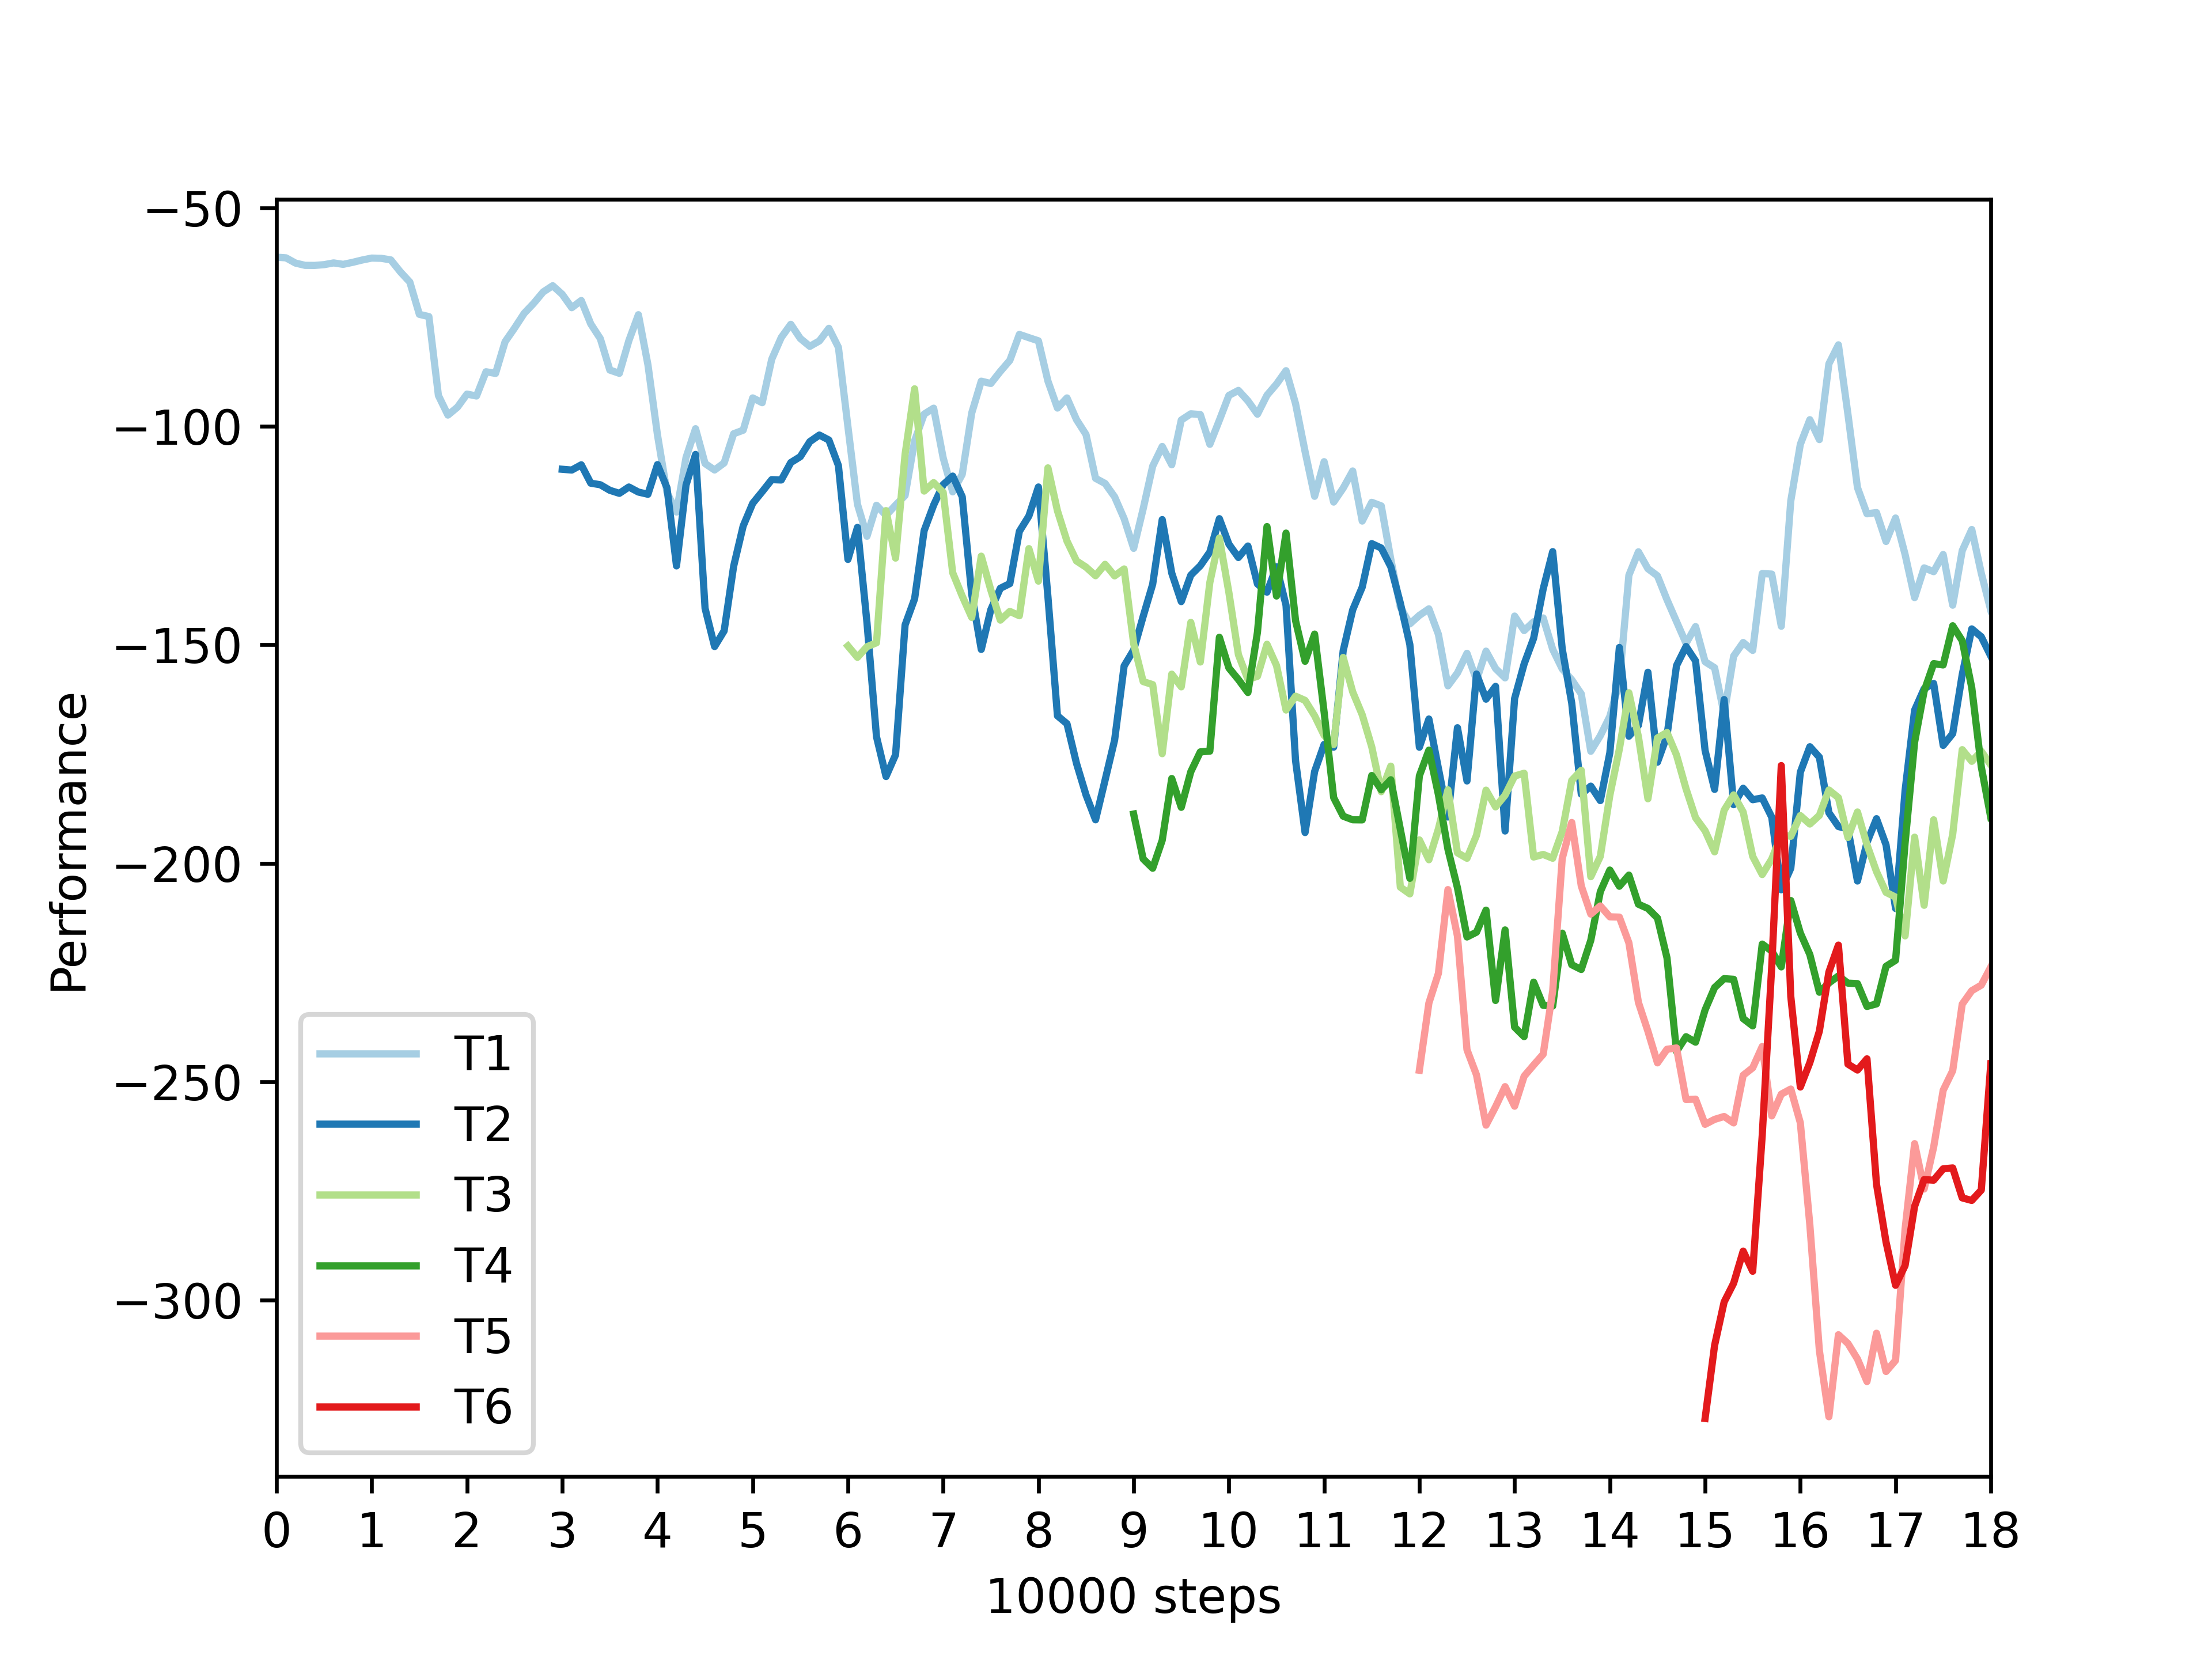}}
         \subcaptionbox{MH-DT}
    {\includegraphics[width=0.245\linewidth]{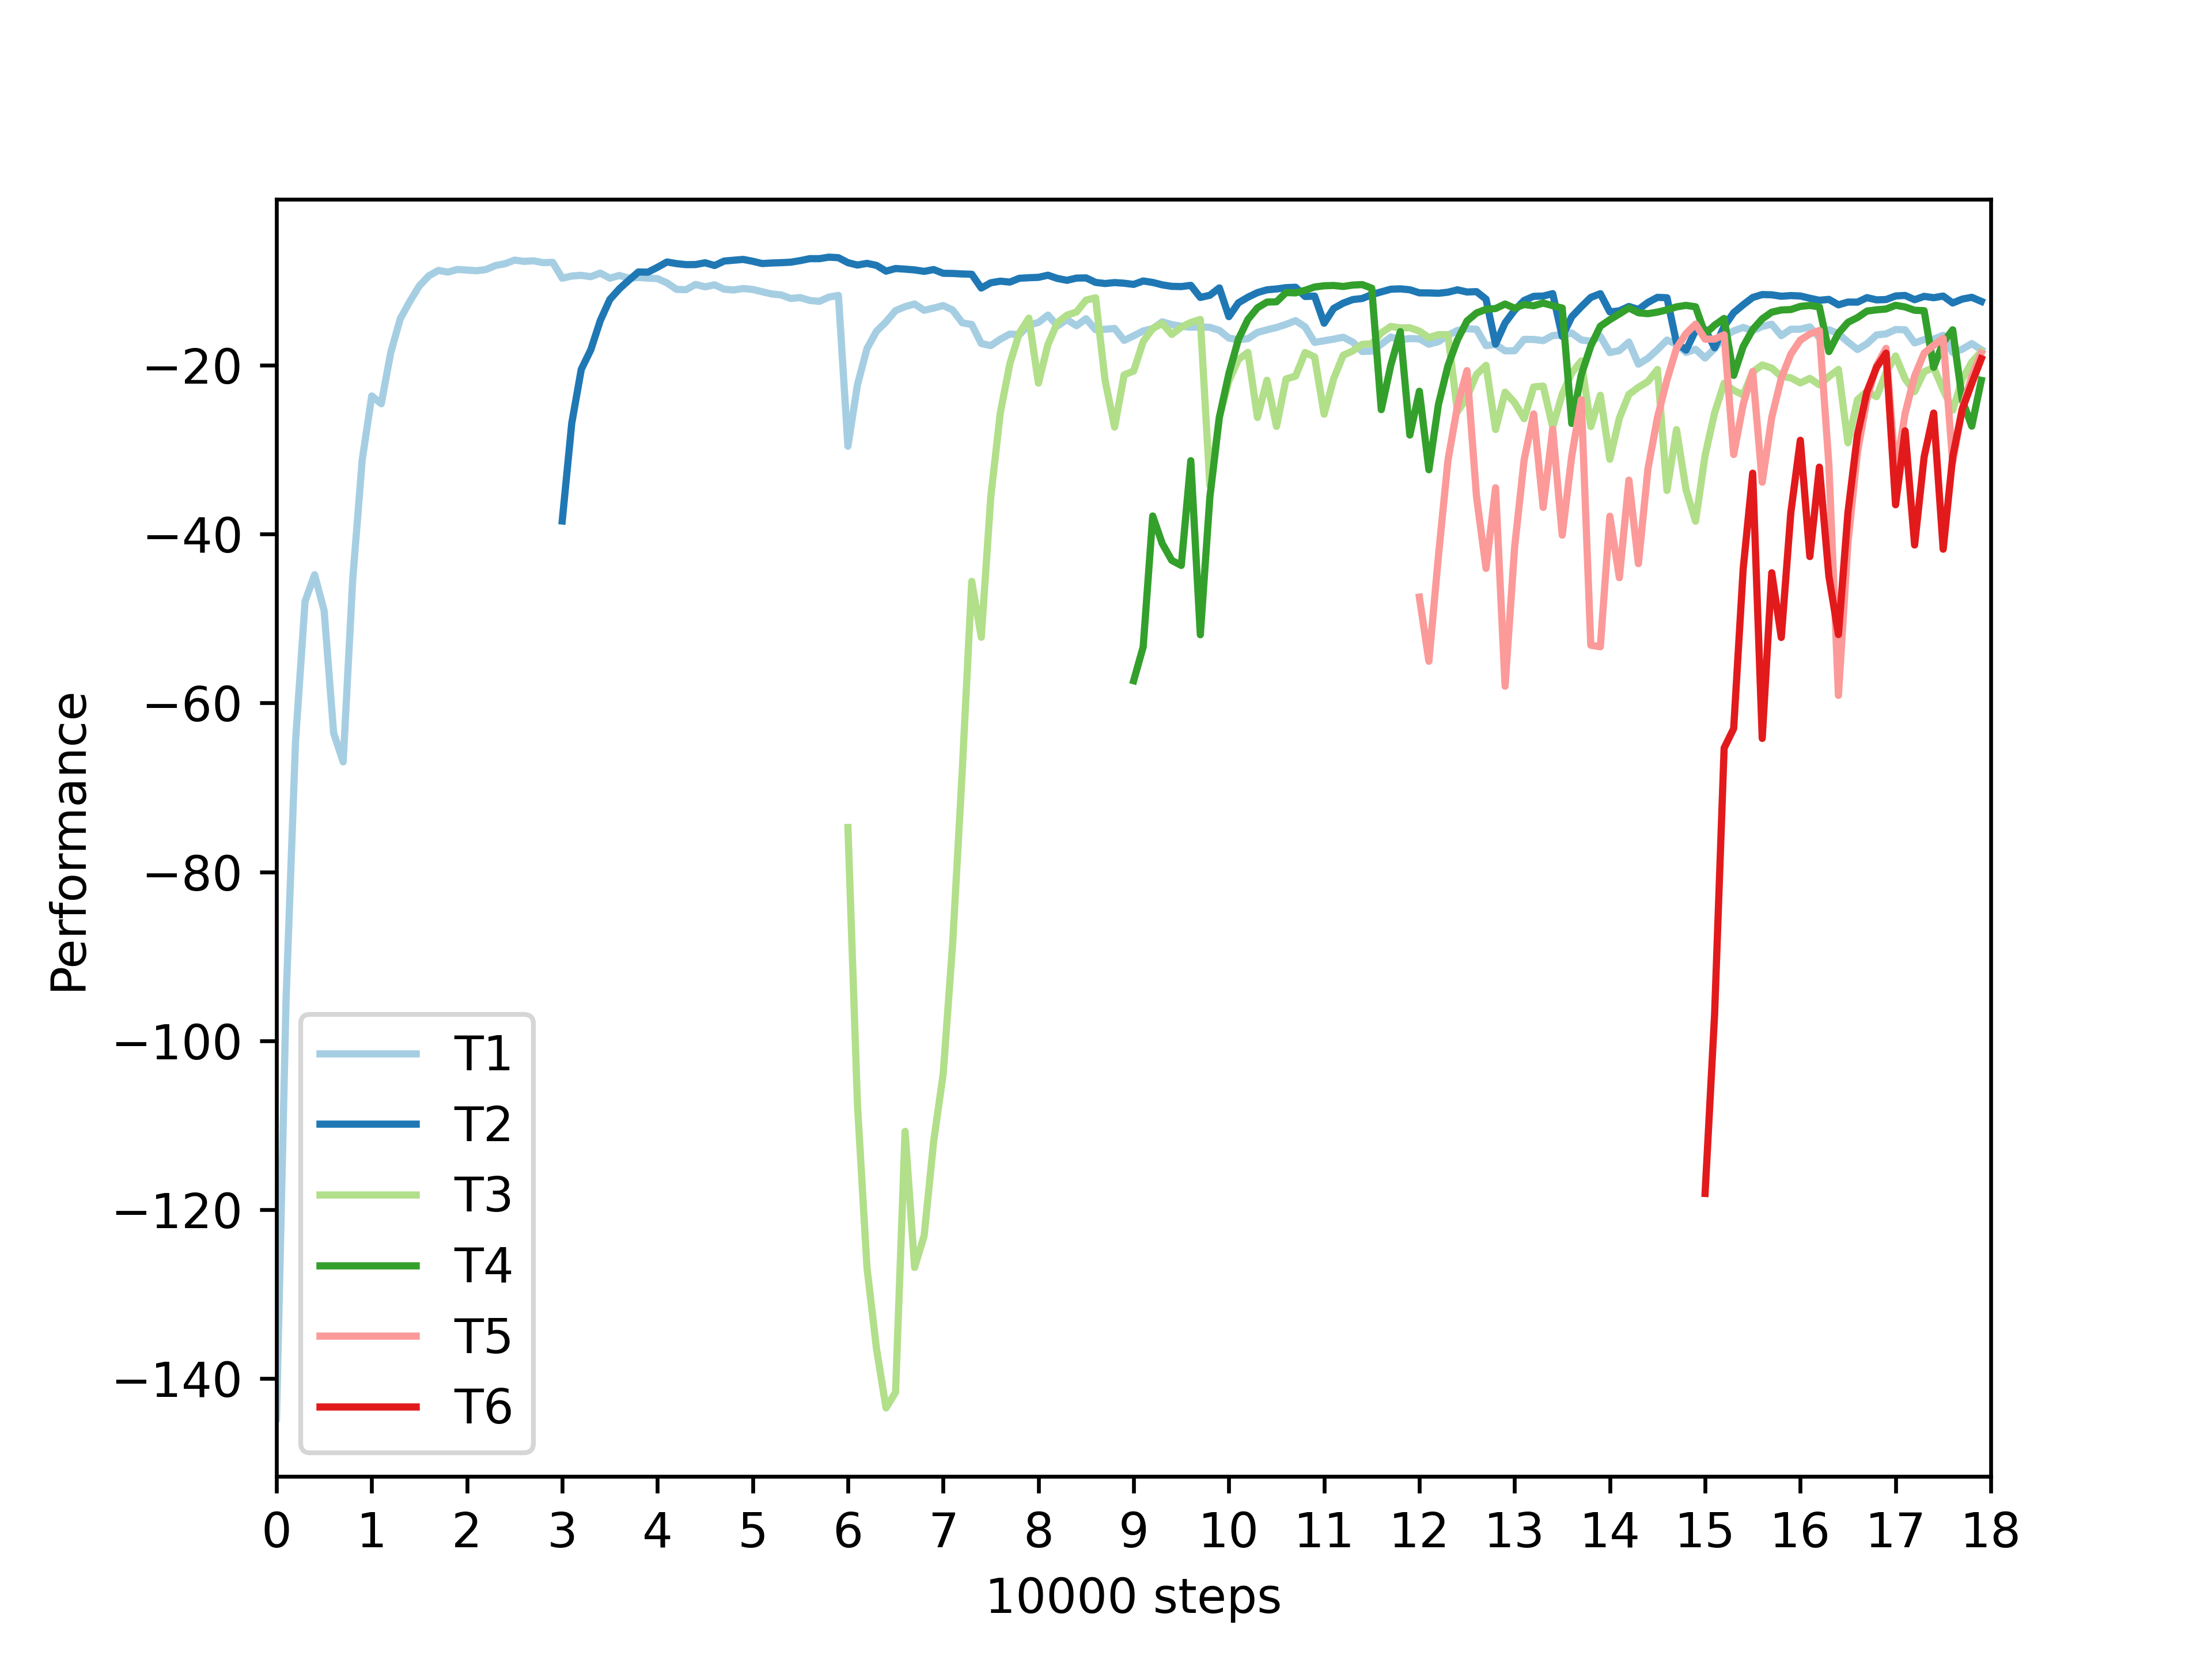}}
	\subcaptionbox{LoRA-DT}
    {\includegraphics[width=0.245\linewidth]{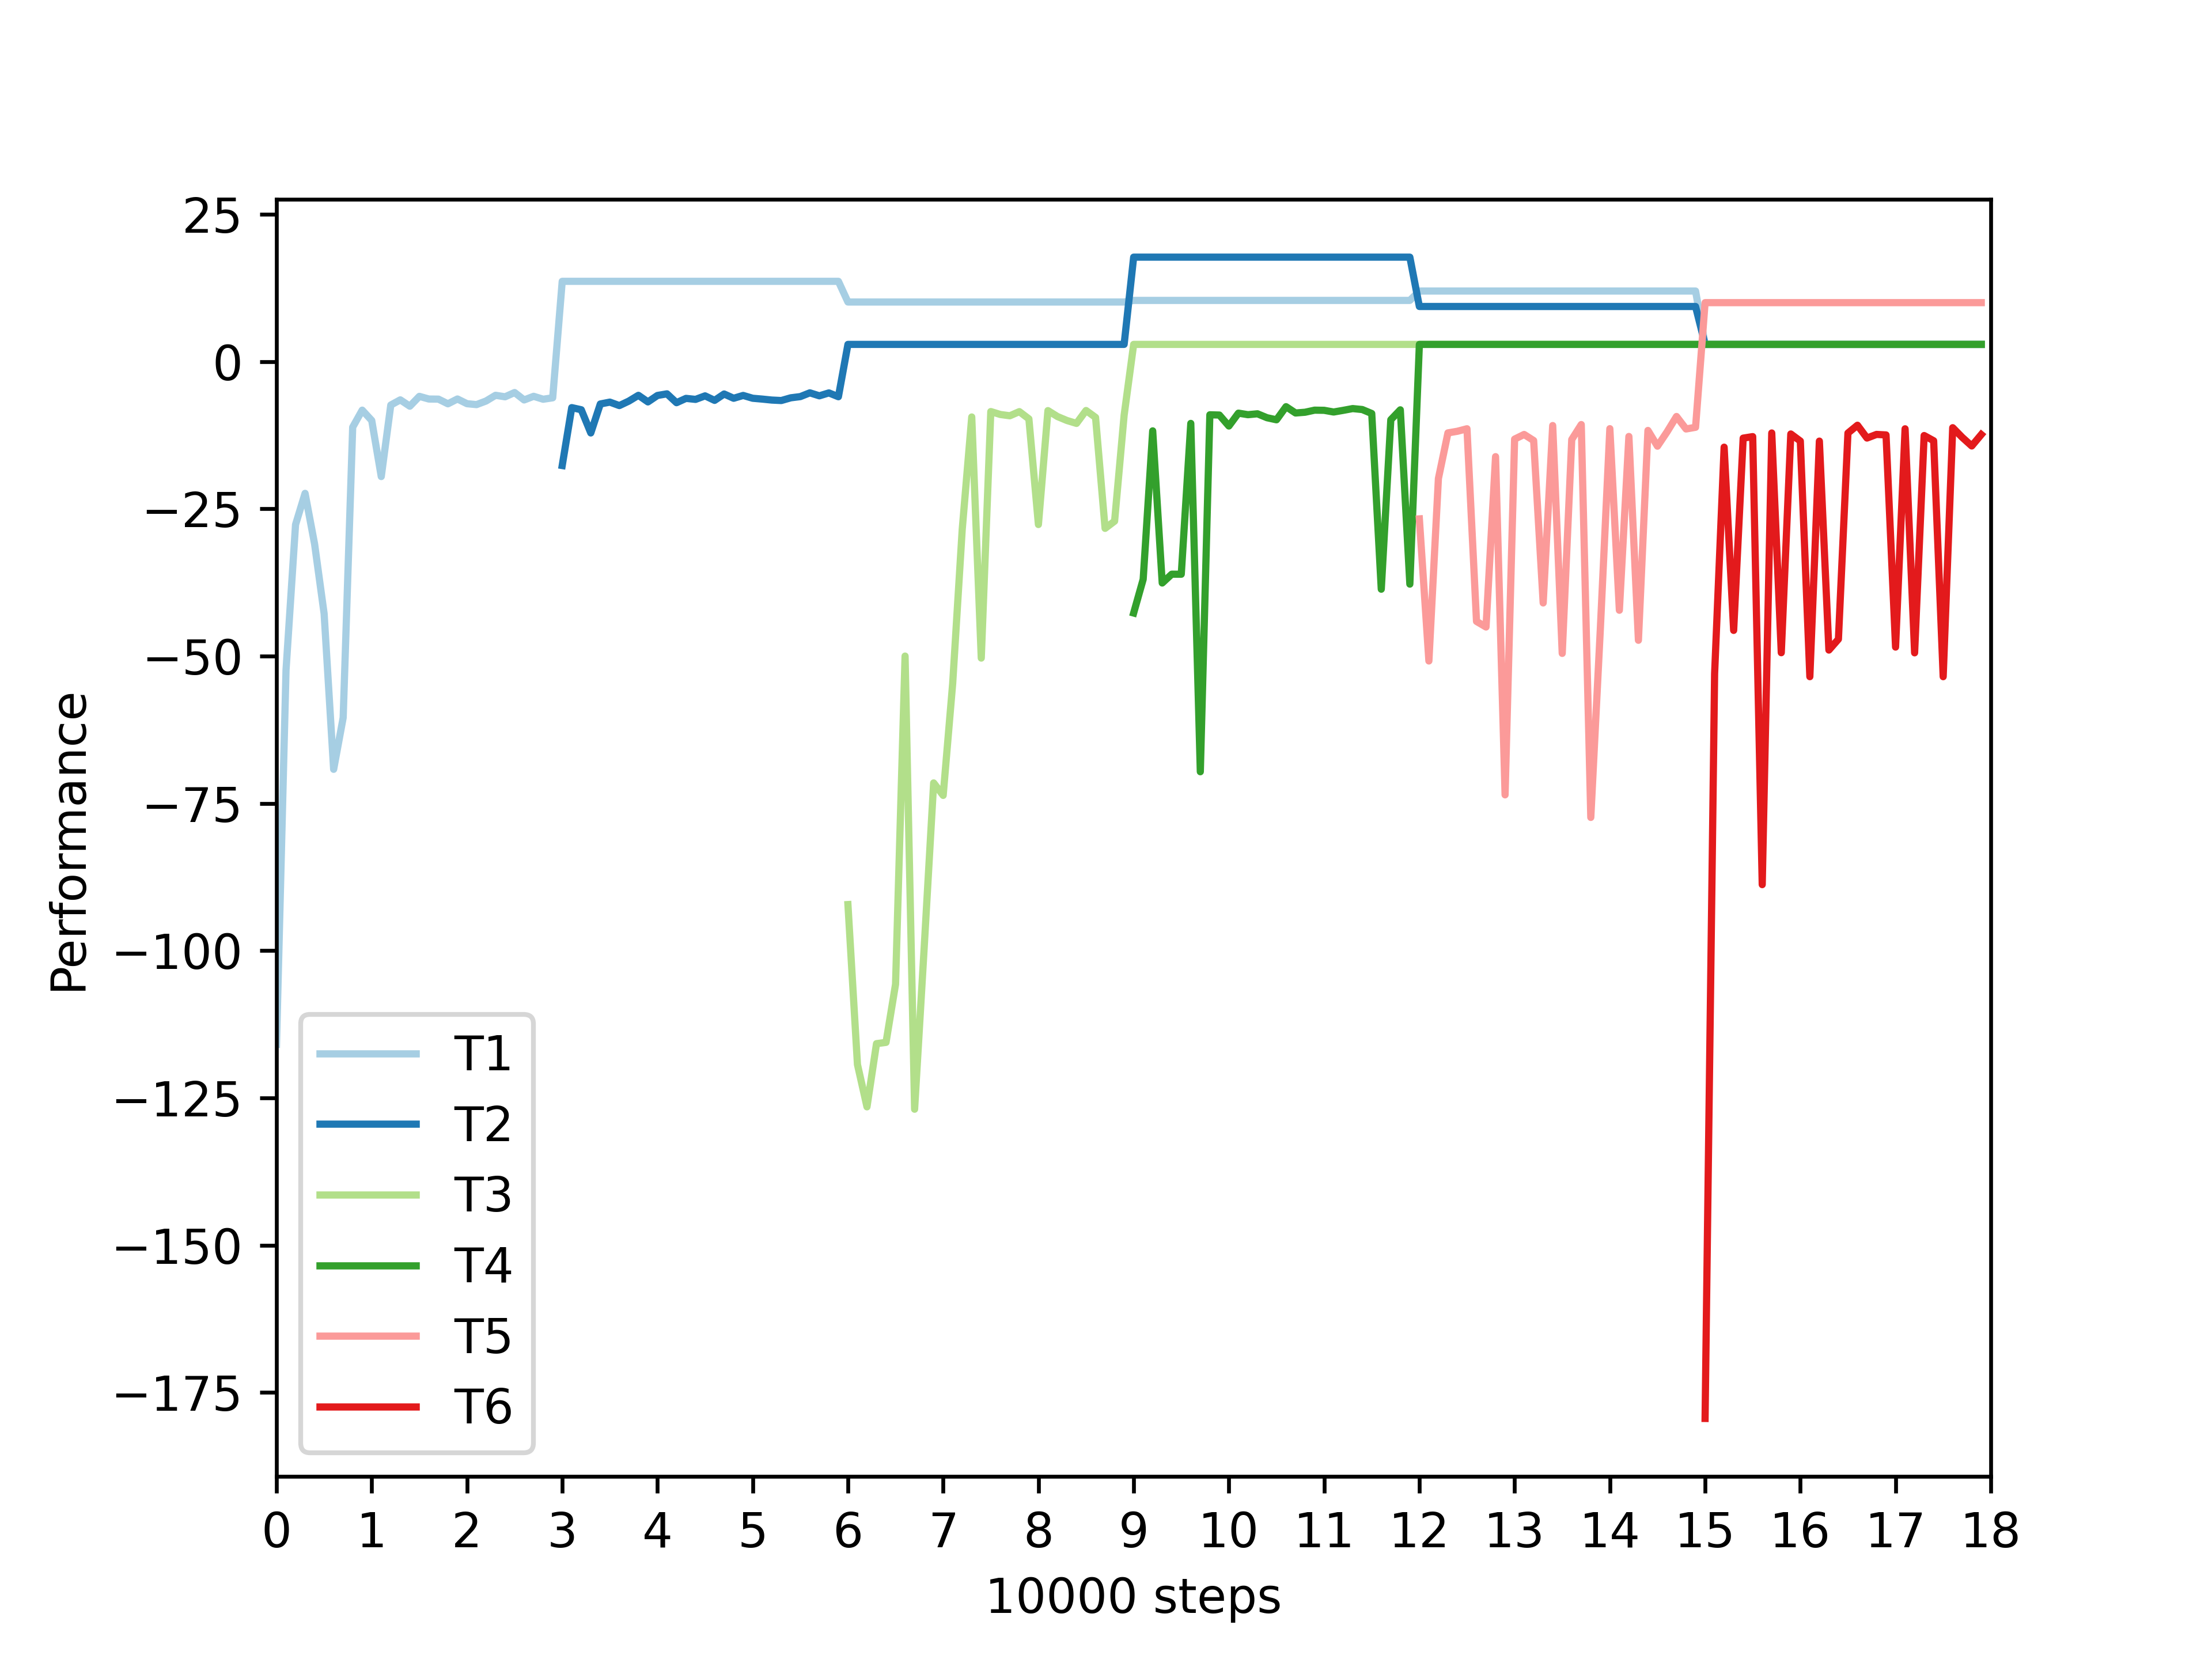}}
    \caption{Cheetah\_Vel (expert)}
\end{figure}

\begin{figure}[htbp]
	\centering
	\subcaptionbox{PDT}
    {\includegraphics[width=0.245\linewidth]{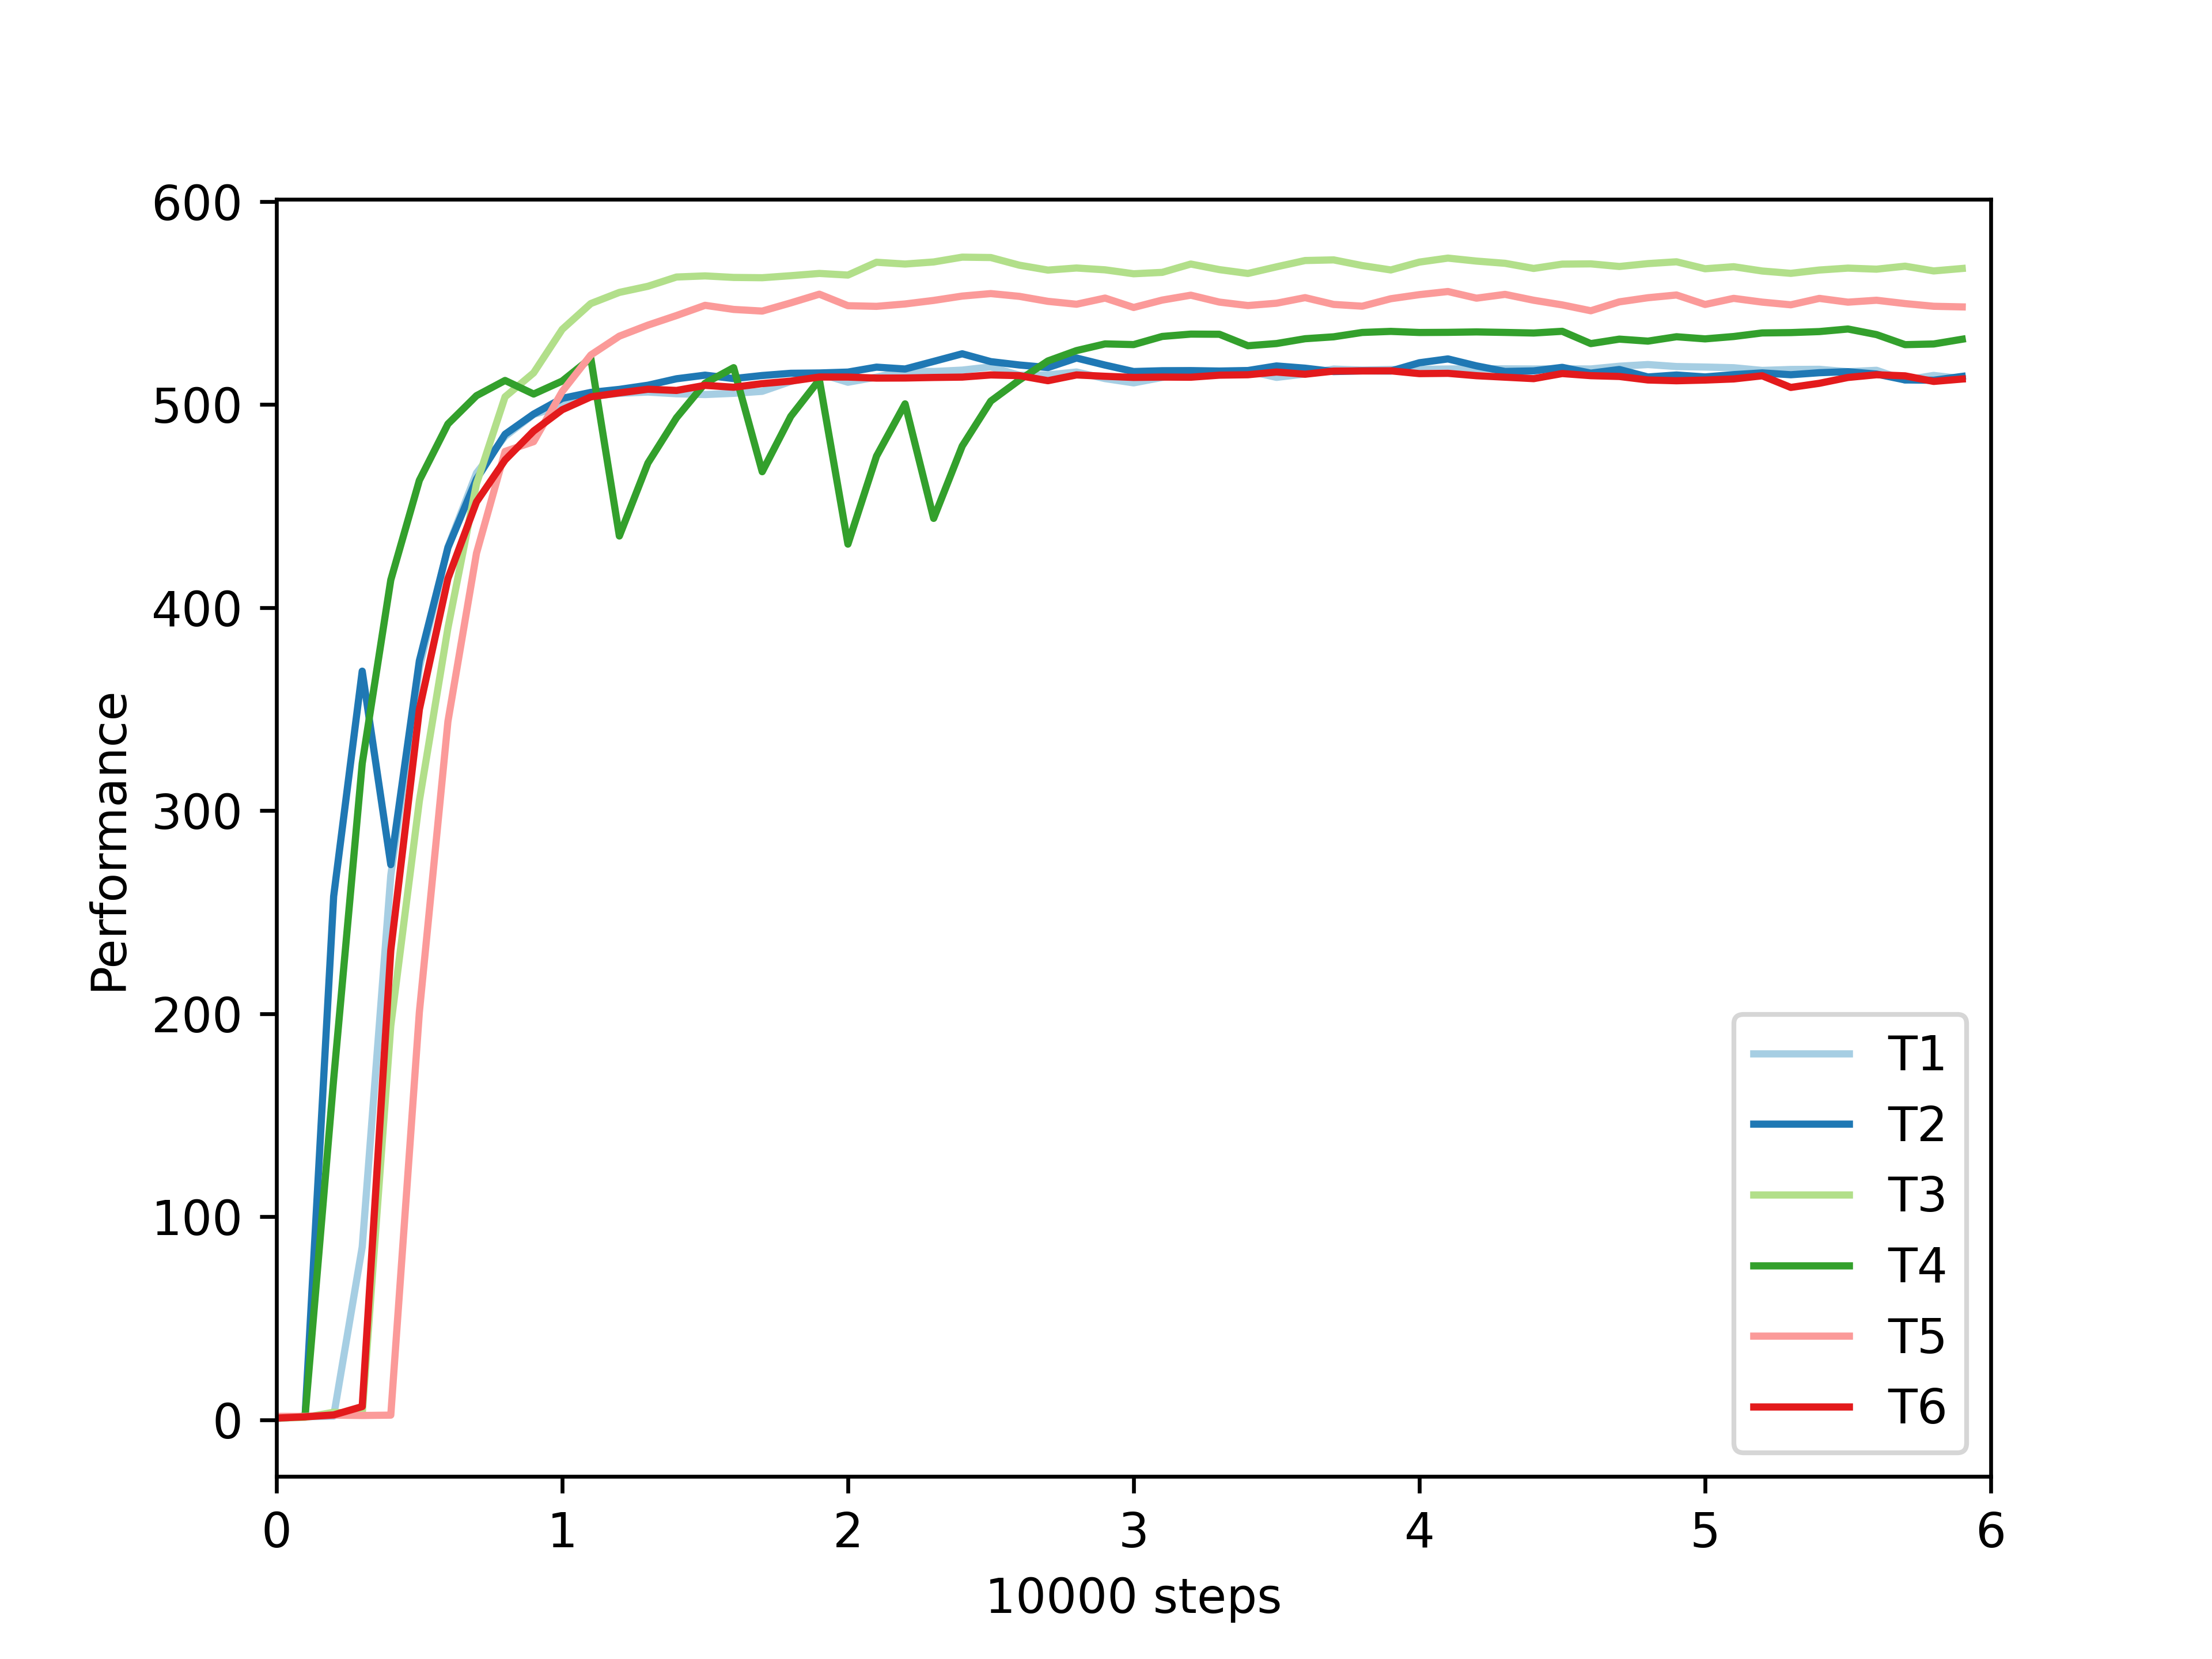}}
    \subcaptionbox{DT + EWC}
    {\includegraphics[width=0.245\linewidth]{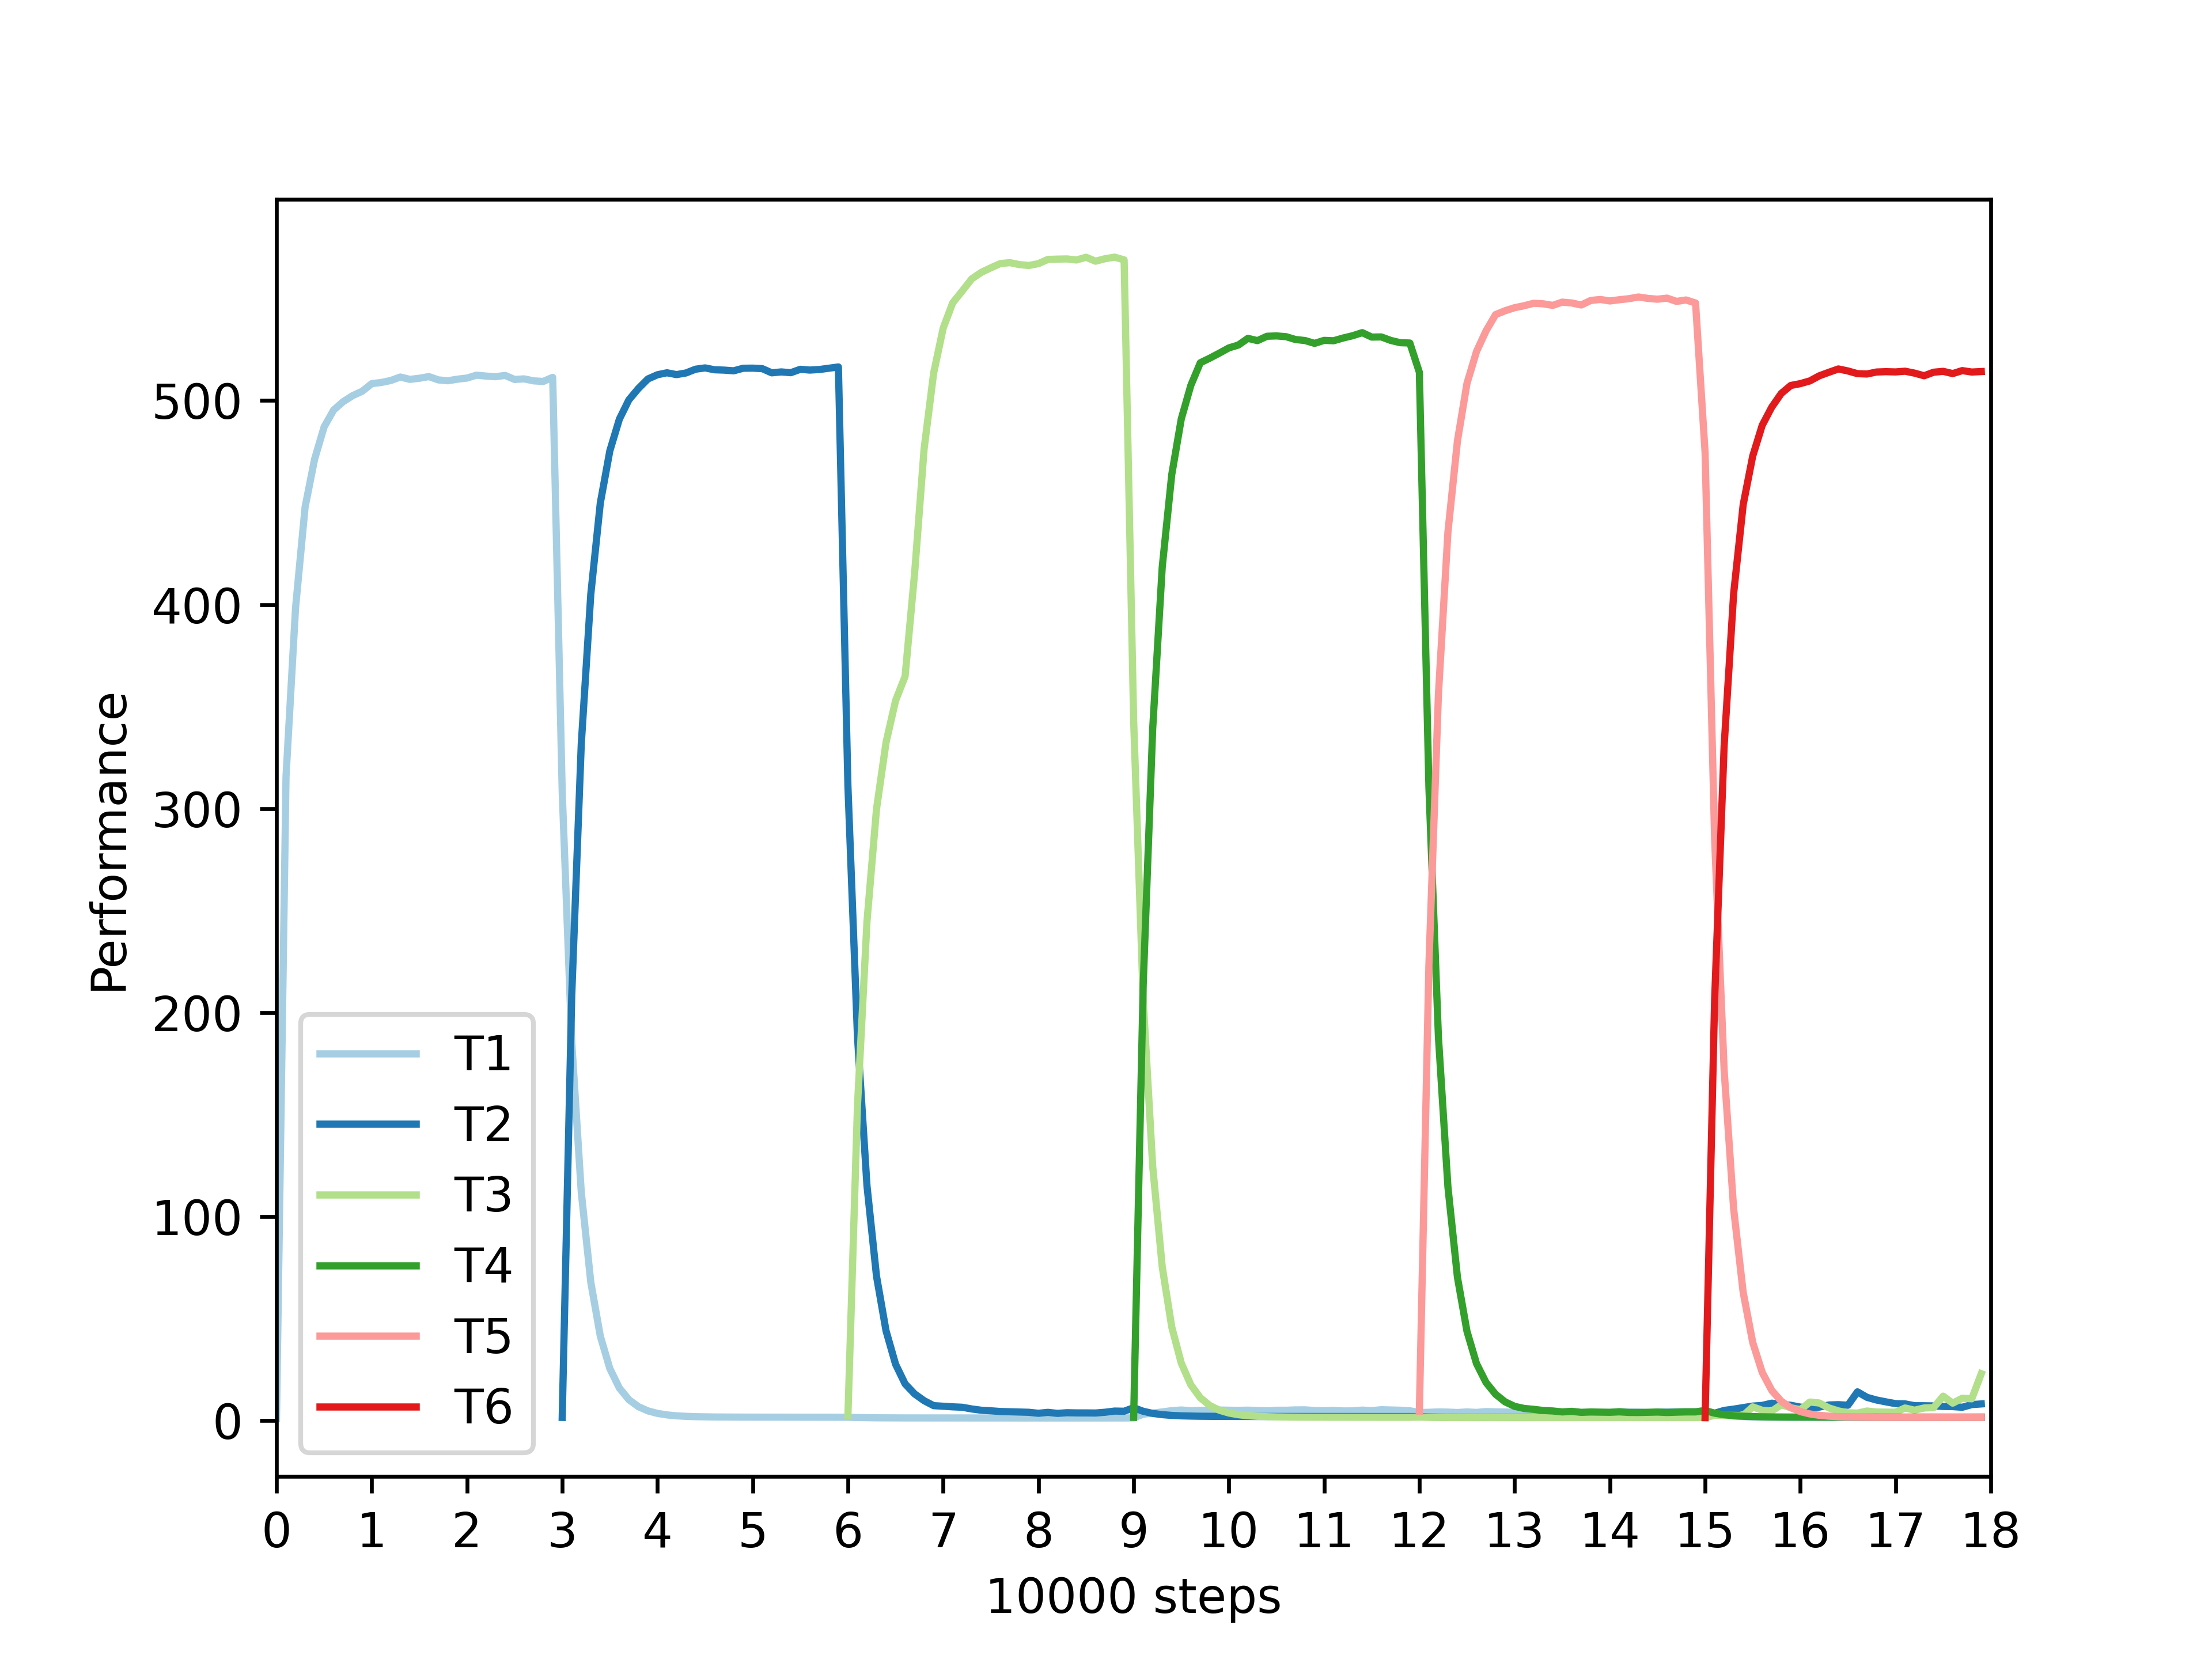}}
    \subcaptionbox{DT + SI}
    {\includegraphics[width=0.245\linewidth]{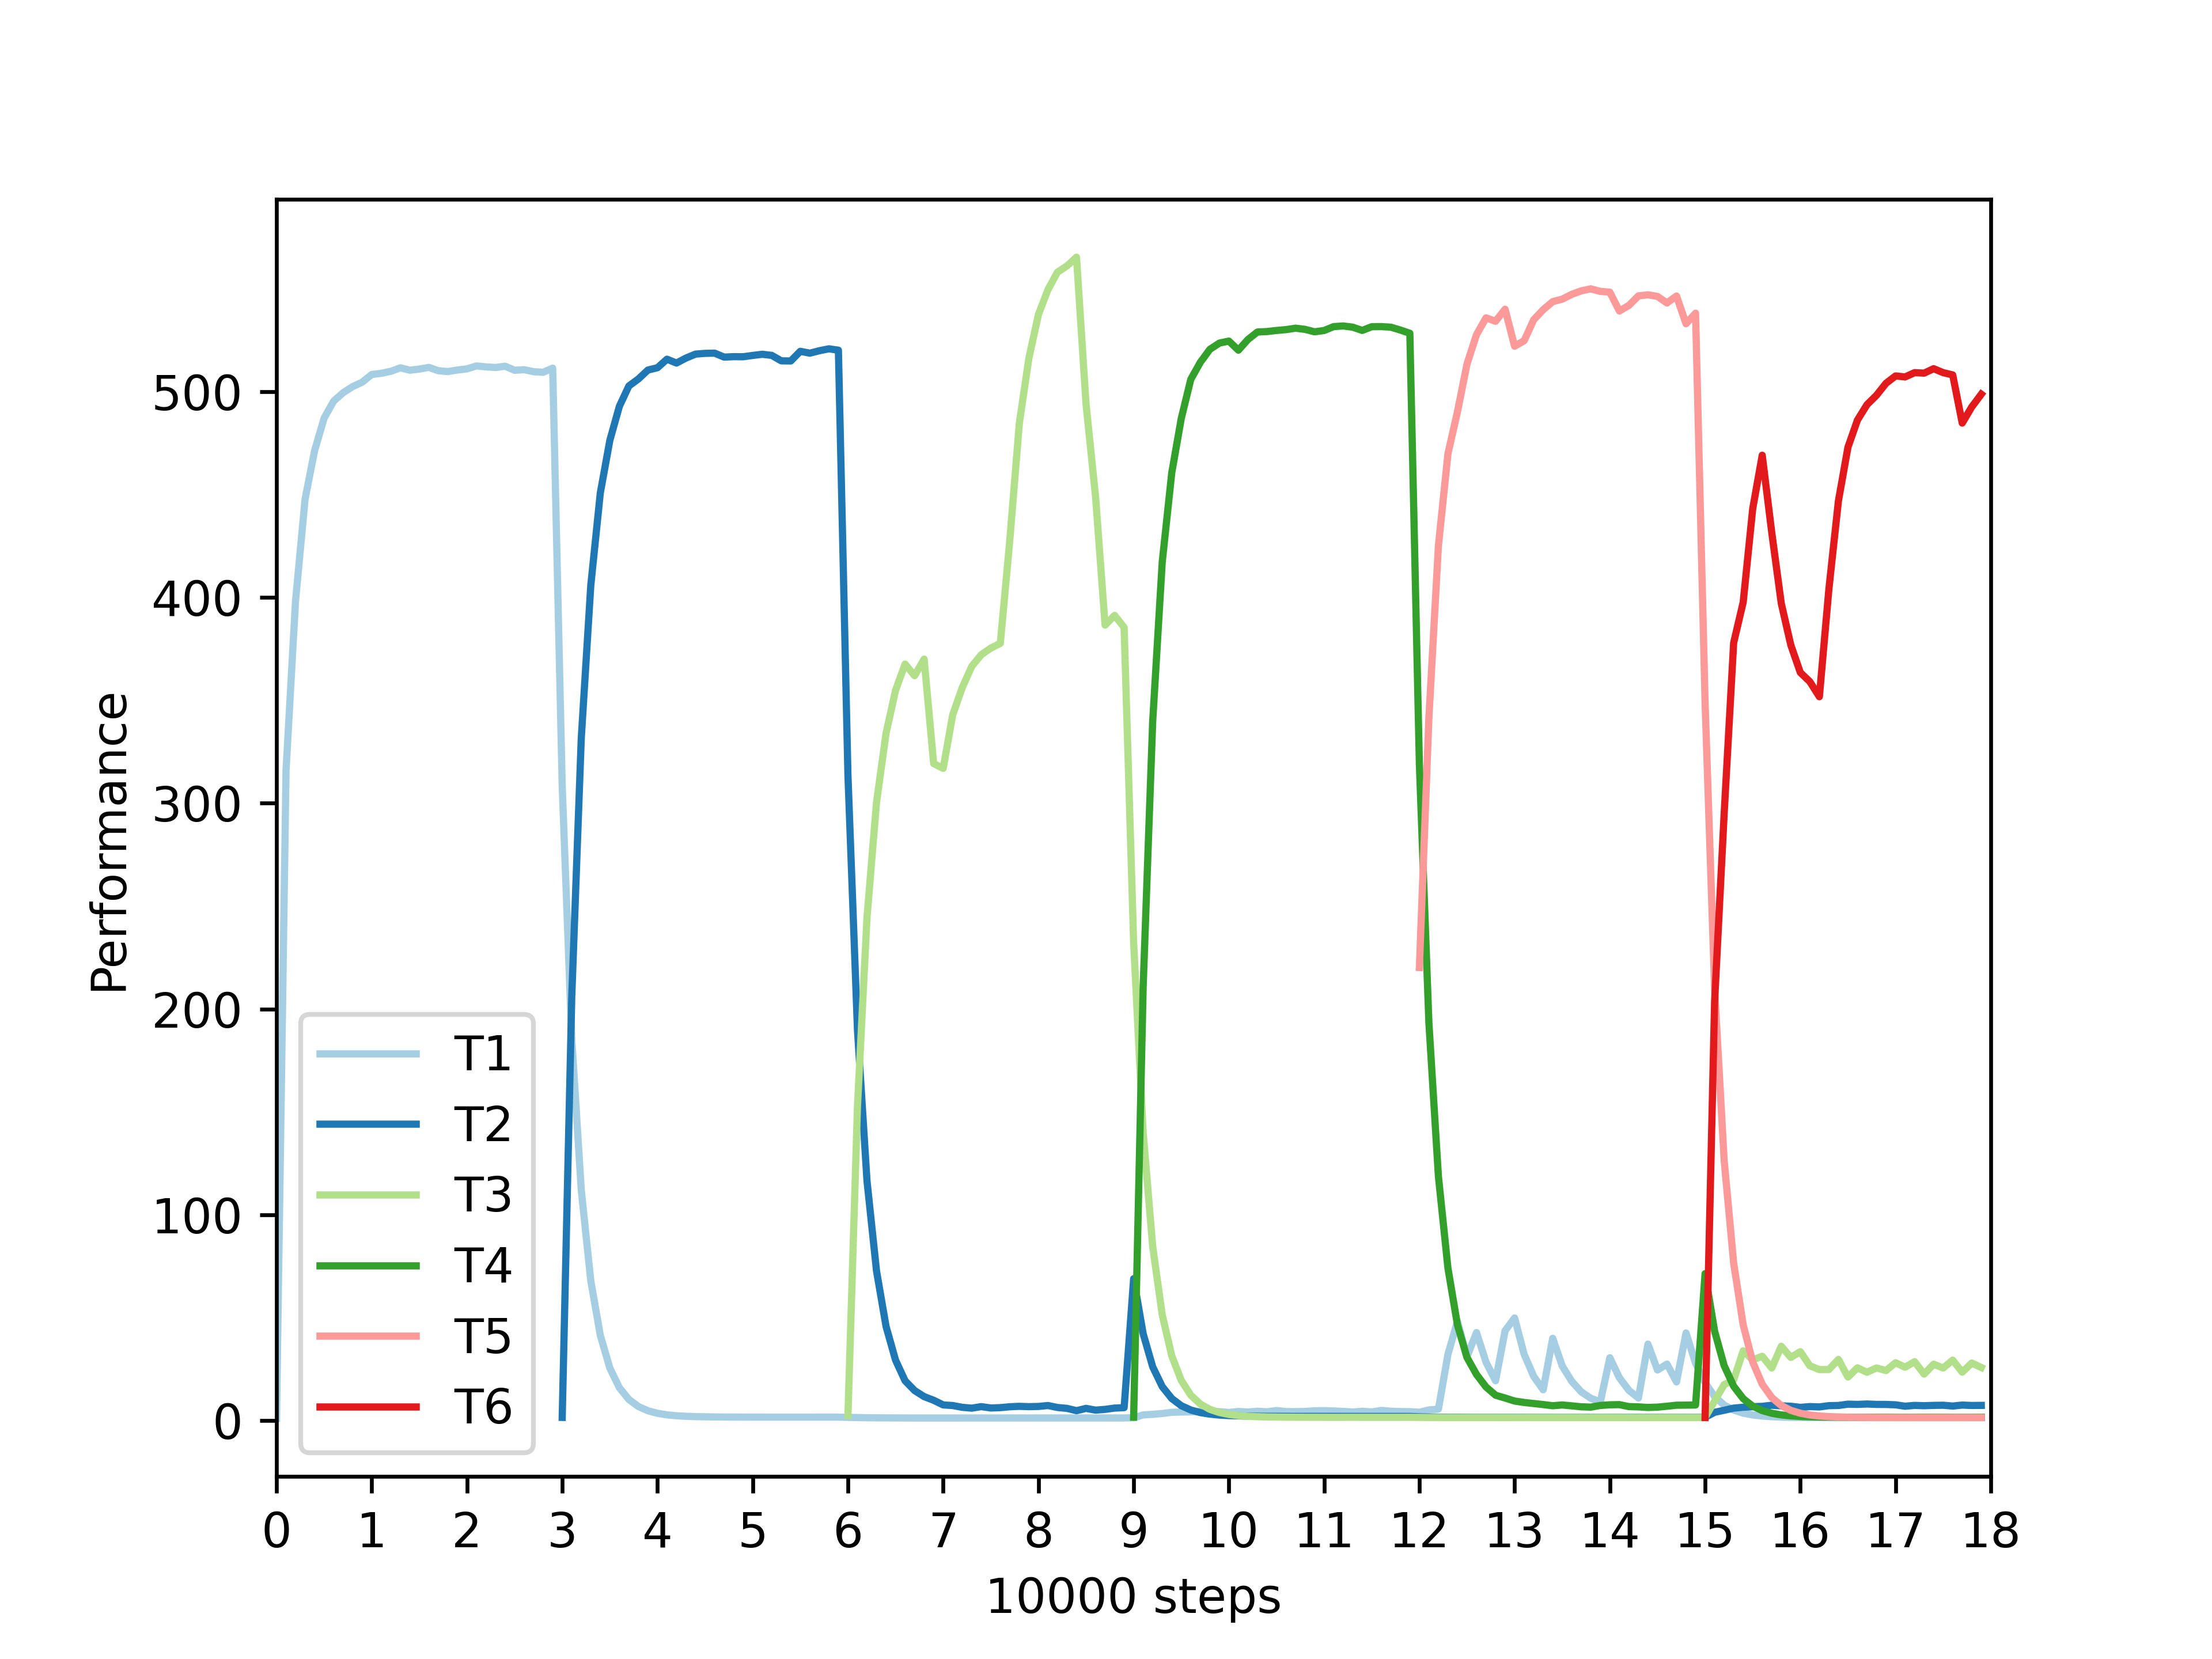}}
    \subcaptionbox{DT + GEM}
    {\includegraphics[width=0.245\linewidth]{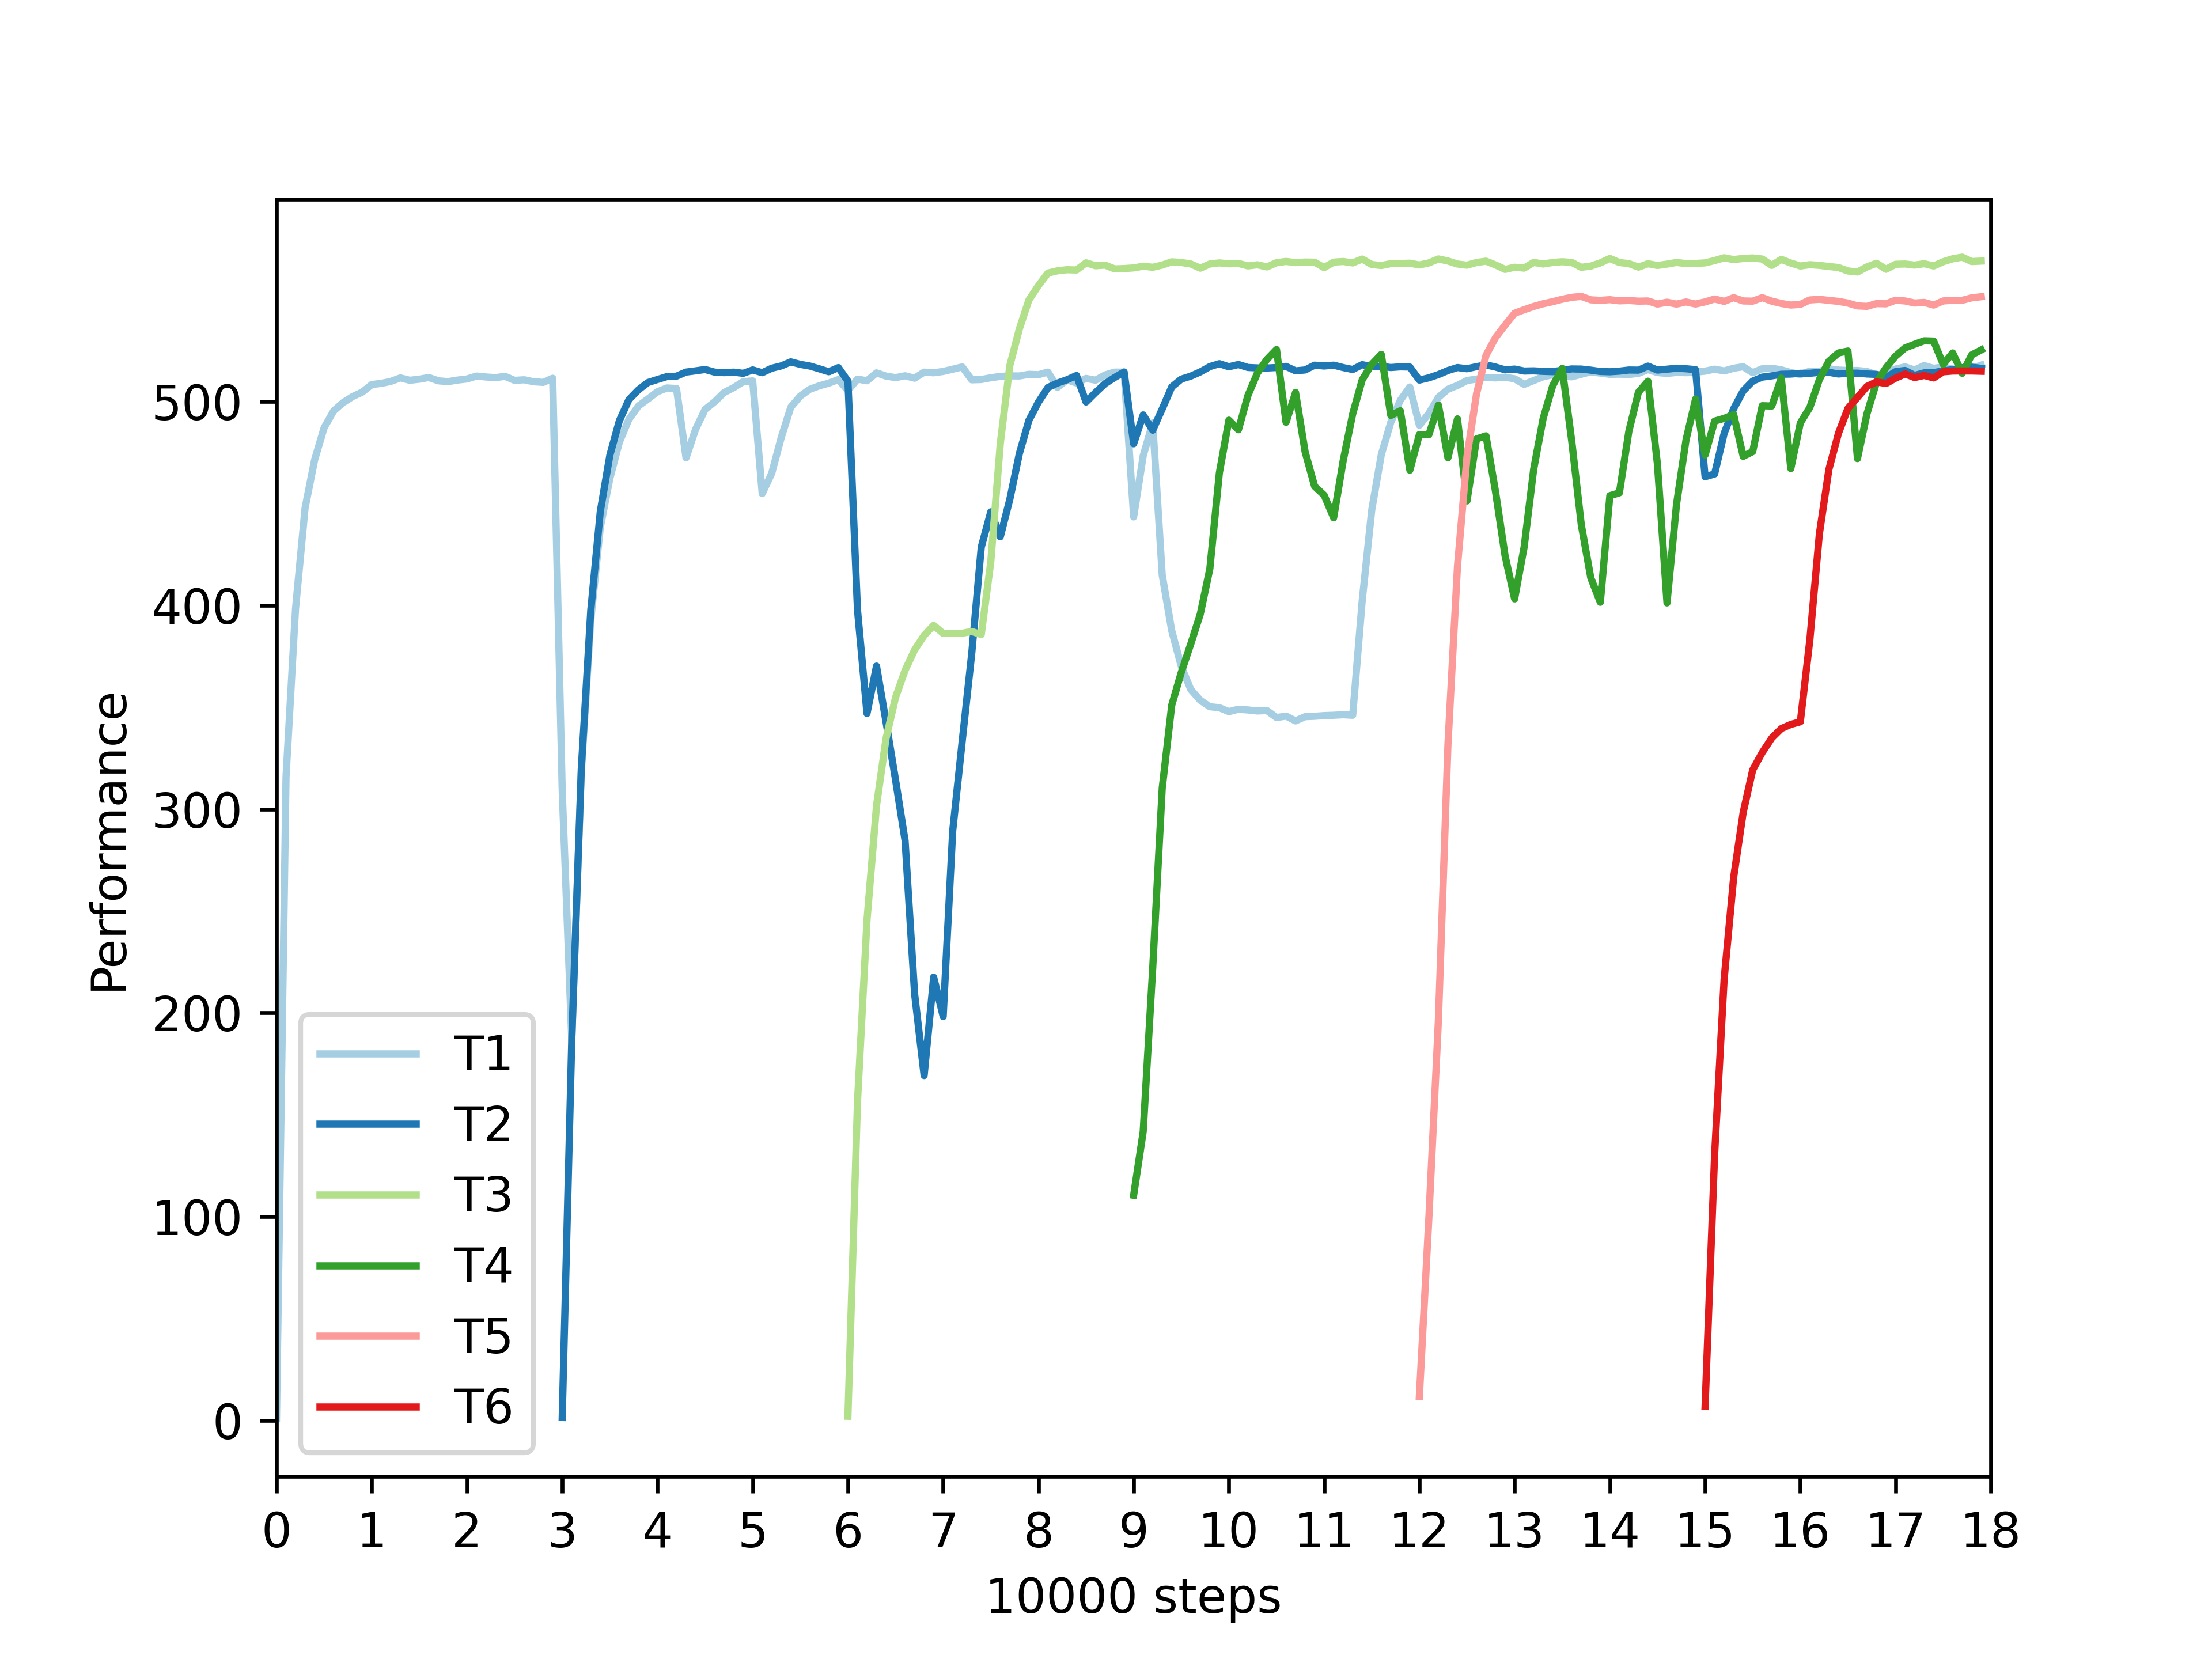}}
	
     \centering	
     \subcaptionbox{Vanilla DT}
    {\includegraphics[width=0.245\linewidth]{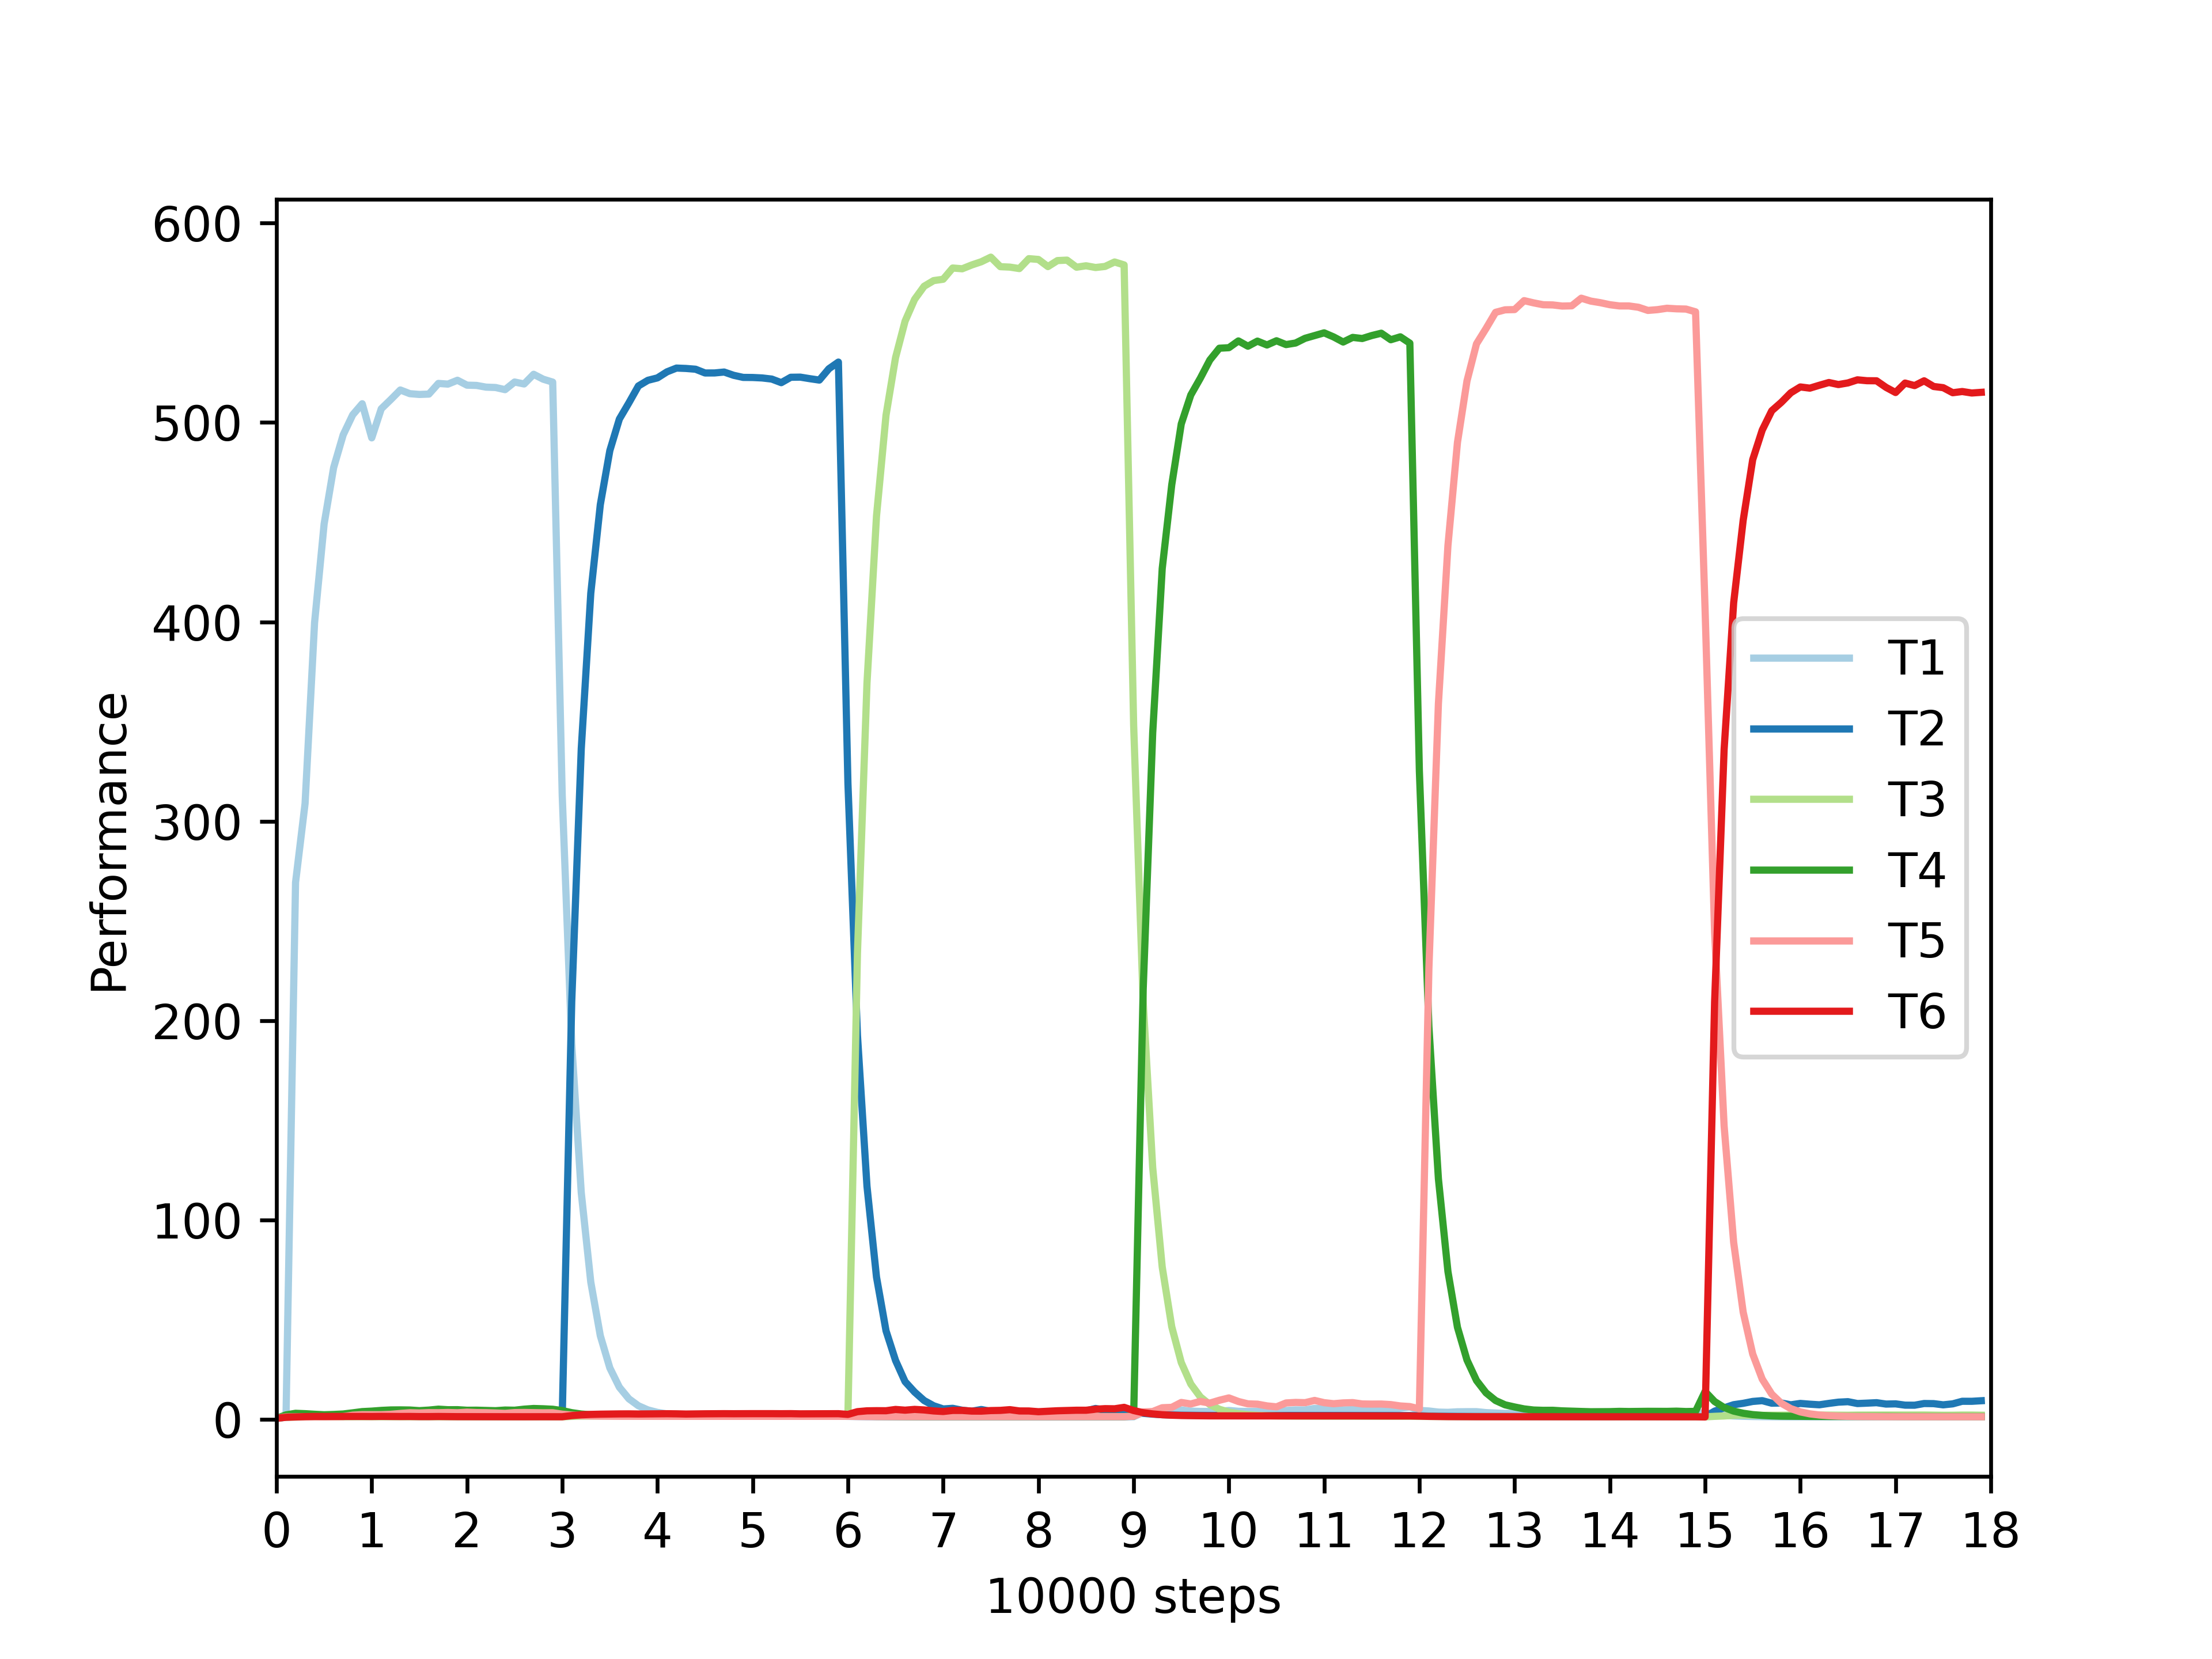}}
        \subcaptionbox{OER}
    {\includegraphics[width=0.245\linewidth]{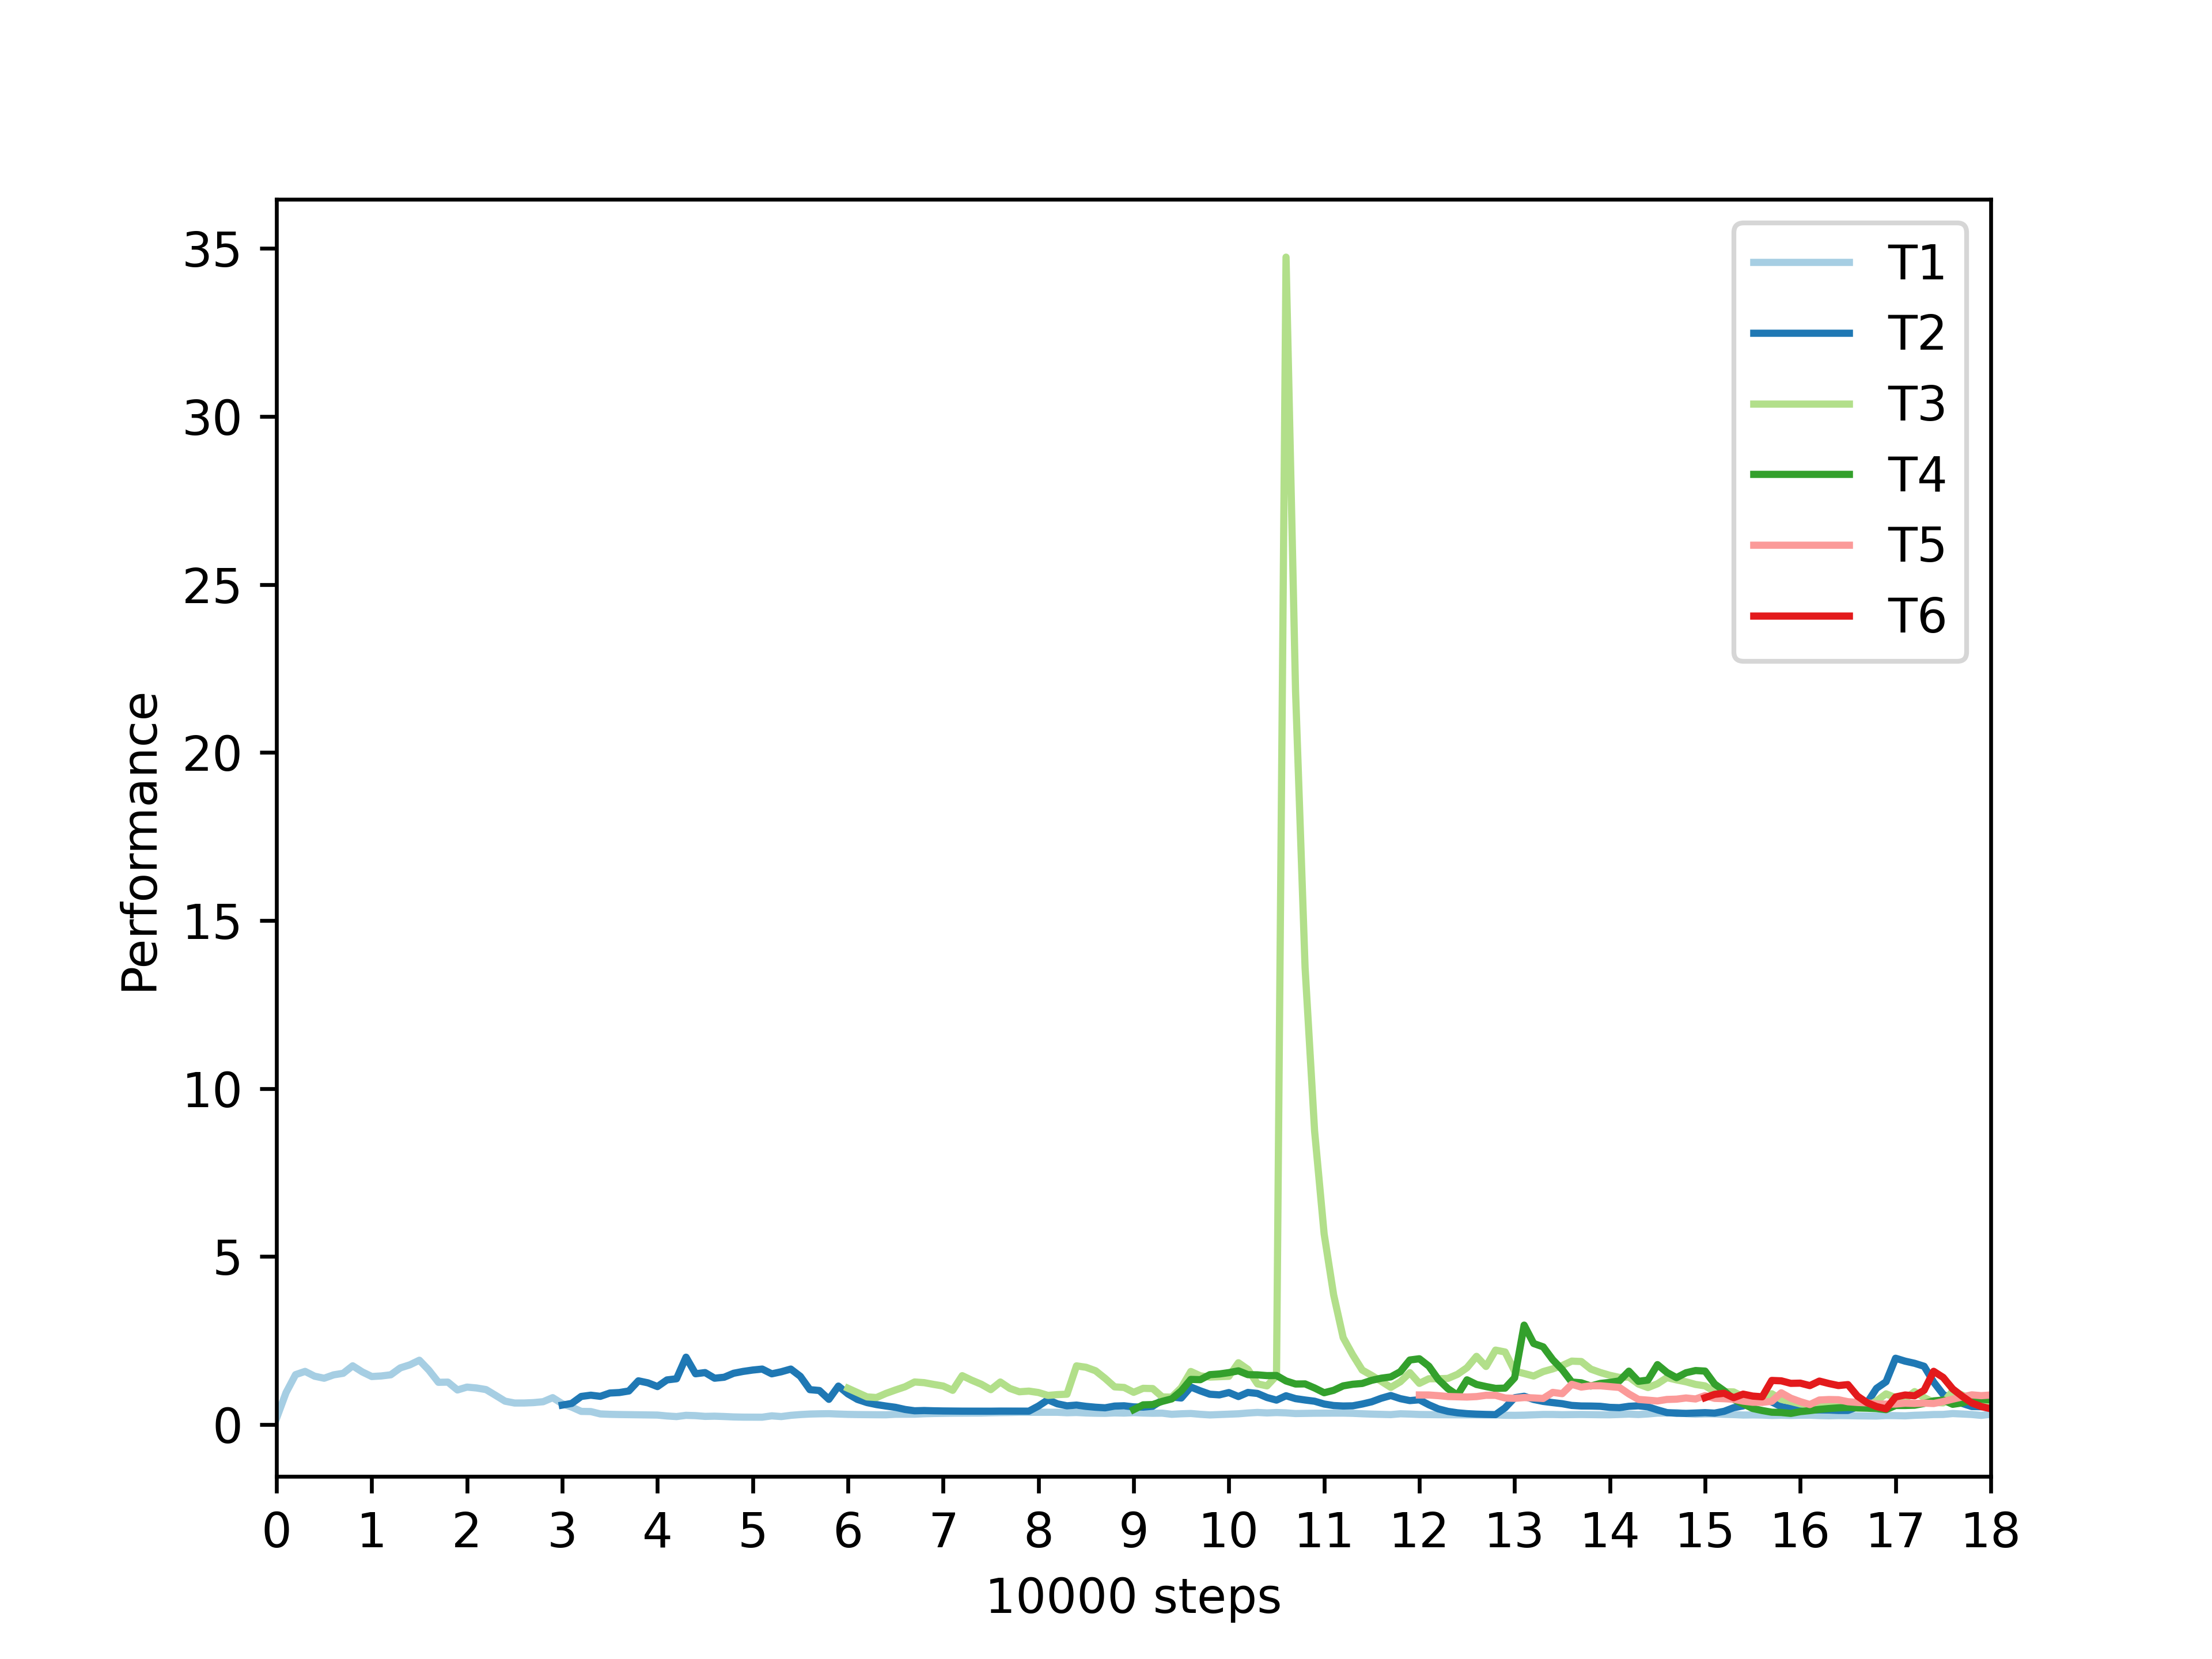}}
    \subcaptionbox{MH-DT}
    {\includegraphics[width=0.245\linewidth]{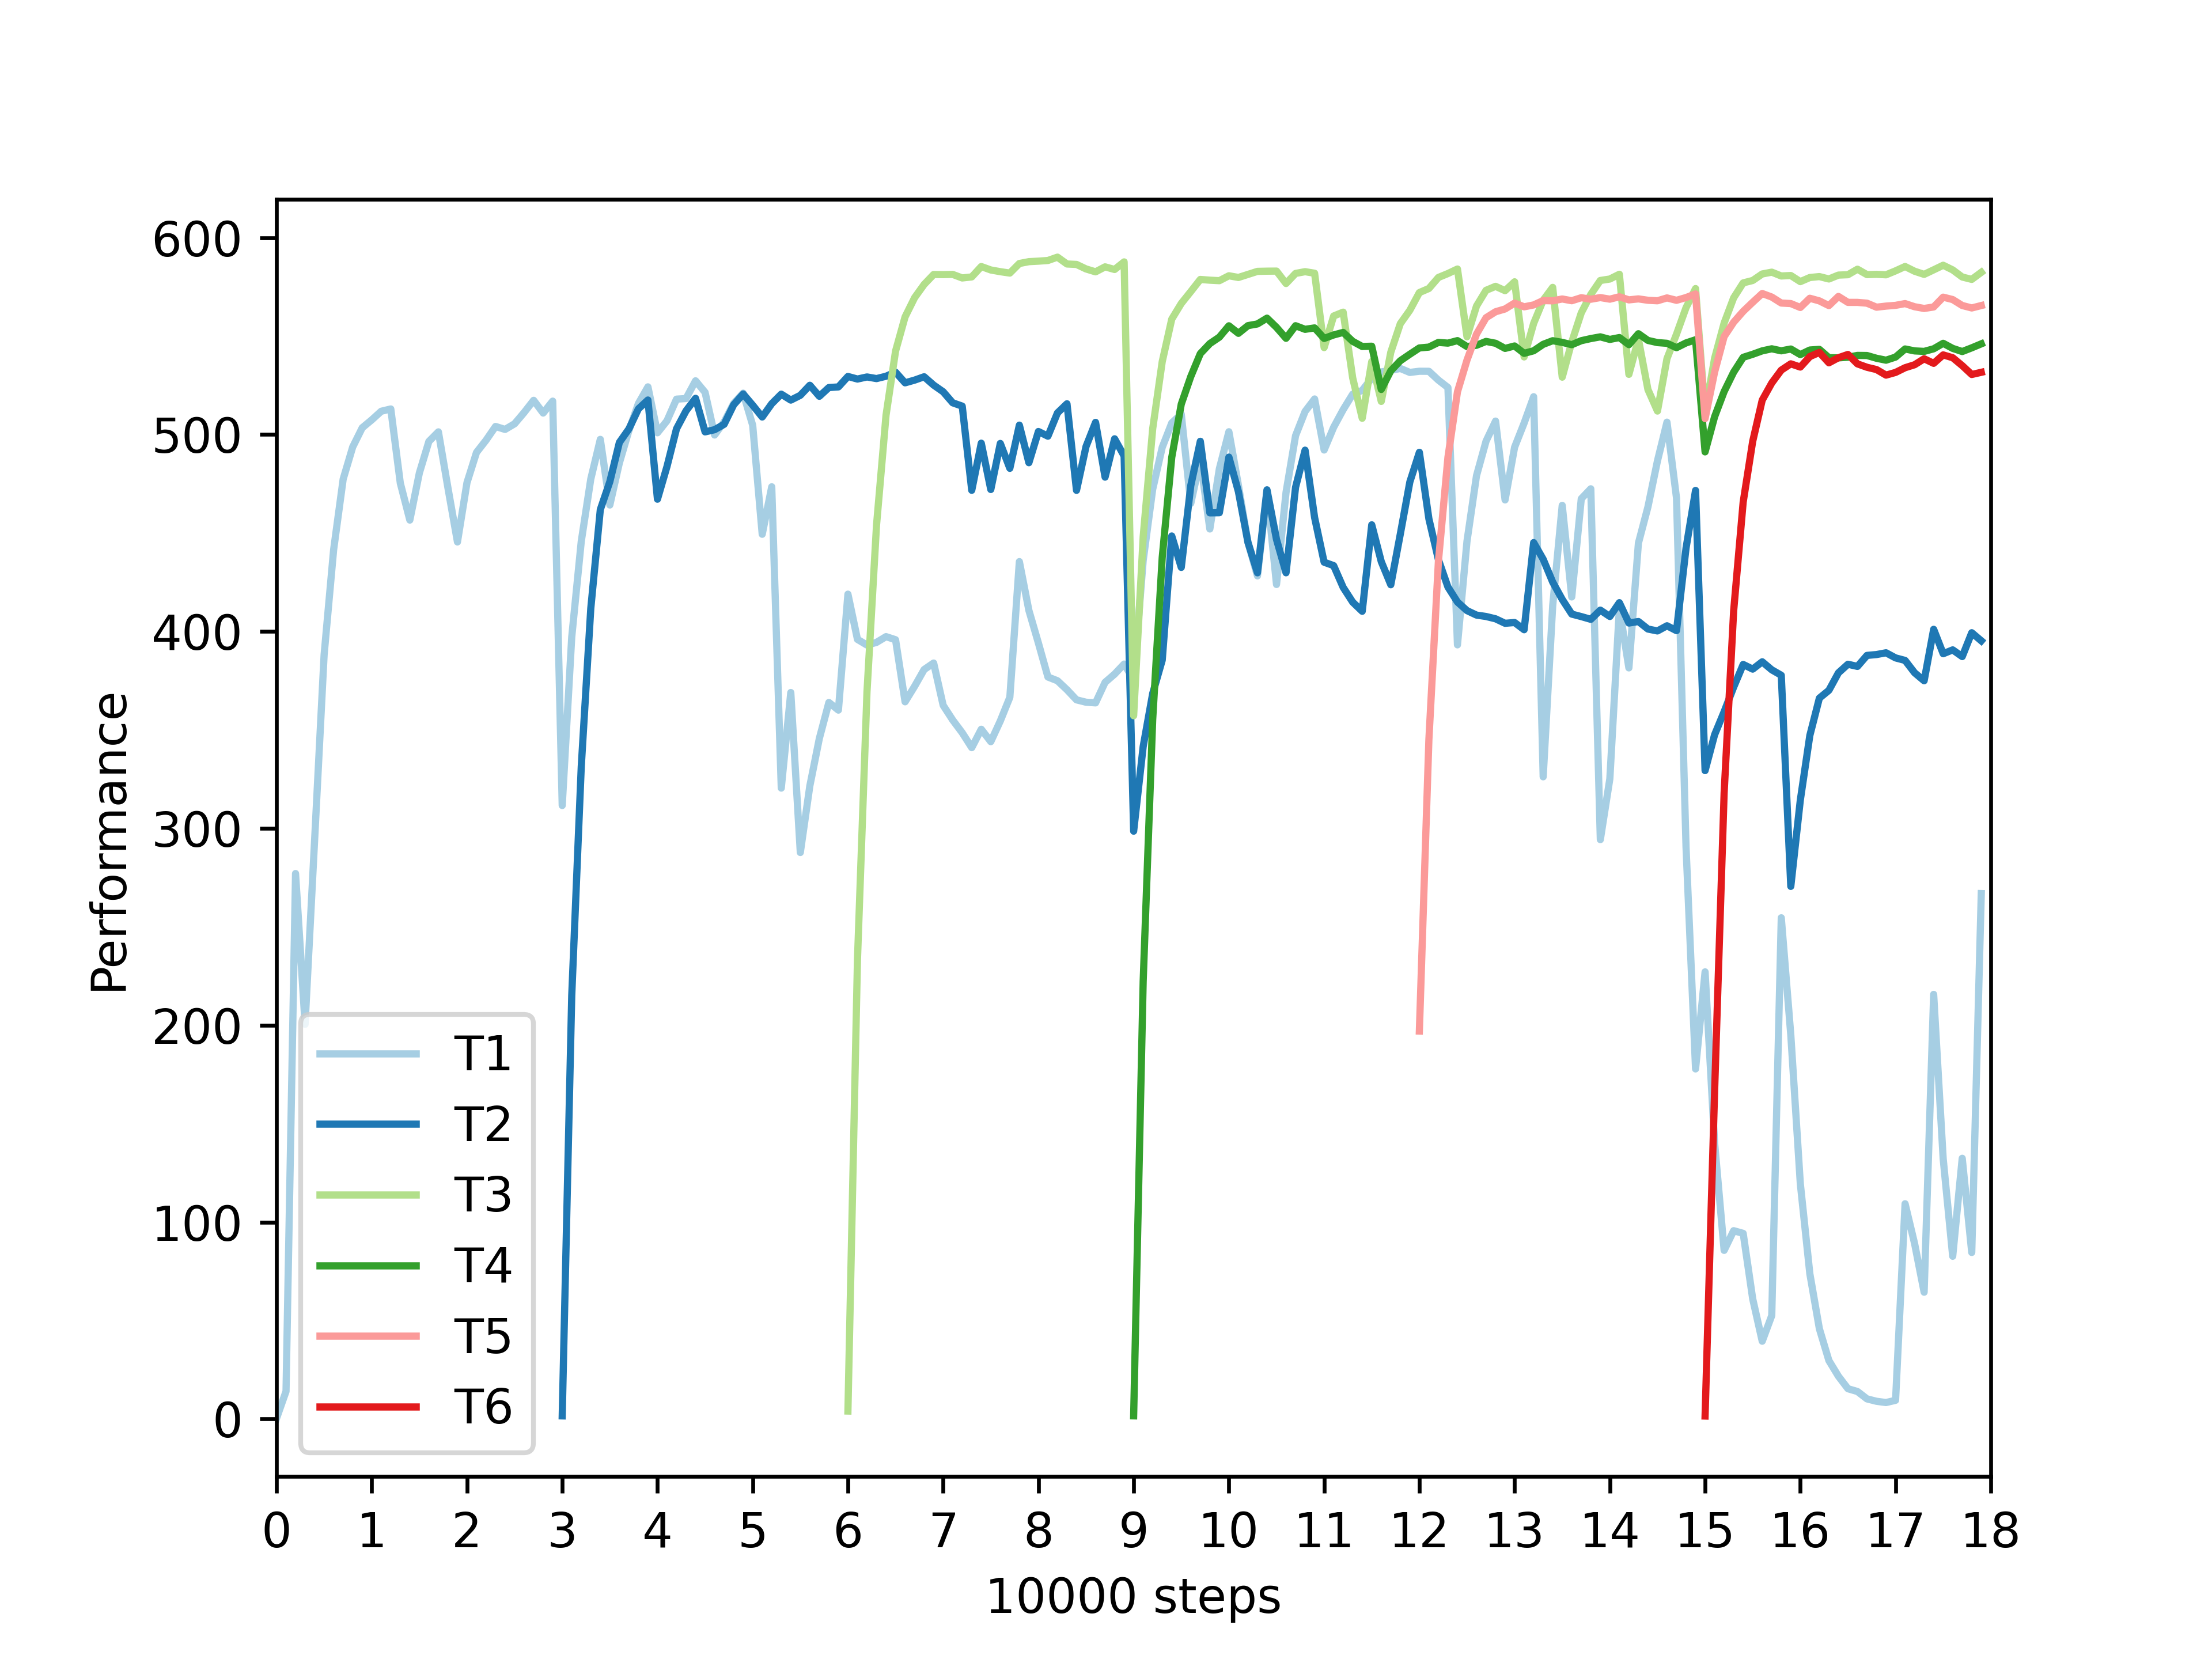}}
	\subcaptionbox{LoRA-DT}
    {\includegraphics[width=0.245\linewidth]{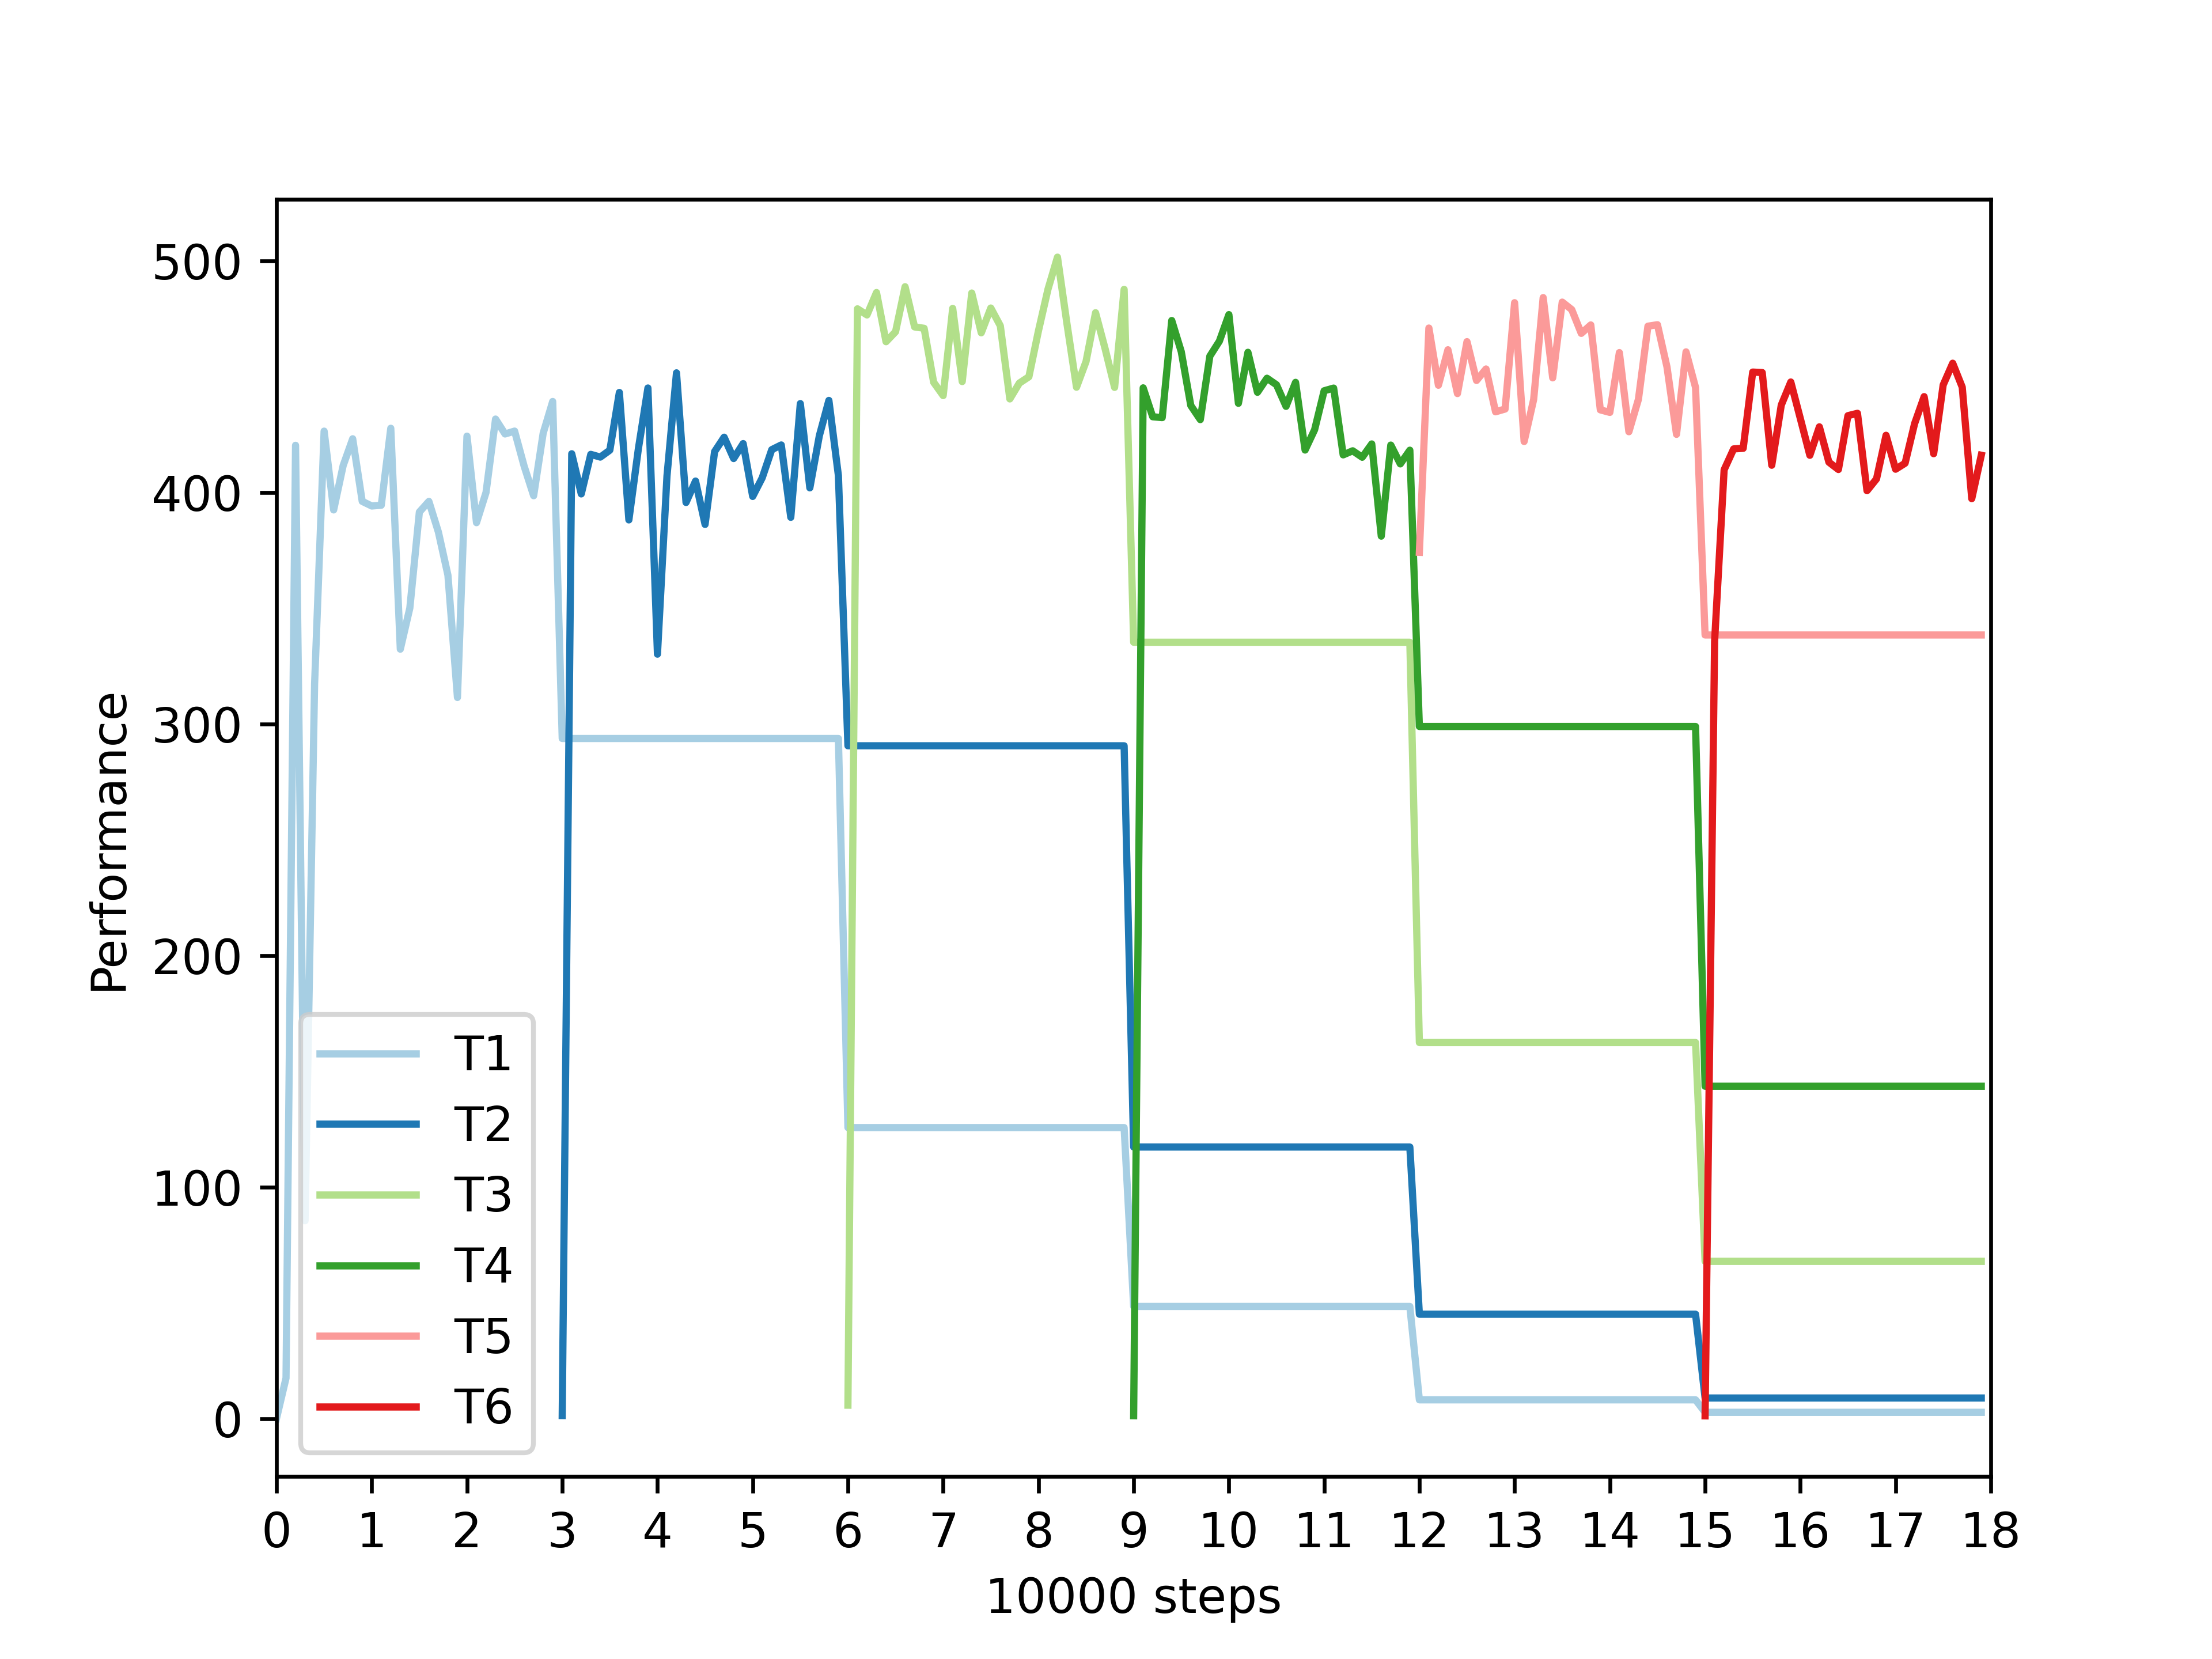}}
    \caption{ML1-pick-place-v2}
\end{figure}
